# Supplementary material for: Measuring User Experience Inclusivity in Human-AI Interaction via Five User Problem-Solving Styles
Source: arXiv:2108.00588 source file (2024-02-17)
Supplement: Supplementary file 1 [file Appendix-Demographics.tex]

\section{Participants' Demographics}
\label{app:demographics}
\begin{table}[h]
    \centering
    \begin{tabular}{p{0.15\linewidth}|p{0.4\linewidth}|p{0.06\linewidth}}
        Demographic & Category & Count\\
        \hline
        \multirow{6}{0.15\linewidth}{Age} & 18---24 years old & 125  \\
         & 25---34 years old & 422 \\
         & 35---44 years old & 259 \\
         & 45---54 years old & 138 \\
         & 55---64 years old & 58 \\
         & 65---74 years old & 14 \\
         \hline
         \multirow{7}{0.15\linewidth}{Gender} & Woman & 527 \\
         & Man & 478 \\
         & Non-Binary & 12 \\
         & Transgender & 4 \\
         & Gender Non-conforming & 2 \\
         & Declined to report & 2 \\
         & Intersex & 1 \\
         \hline
         \multirow{7}{0.15\linewidth}{Education} & Bachelors degree & 430 \\
         & Some college (no degree) & 199 \\
         & Advanced degree (MA/MS/Ph.D./M.D.) & 162 \\
         & Associates degree & 112 \\
         & At most high school & 91 \\
         & Trade/technical school & 22 \\
         \hline
         \multirow{29}{0.15\linewidth}{Employment Field} & Science/Technology/Programming & 176  \\
         & Education & 113 \\
         & Unemployed/other & 97 \\
         & Sales/Marketing & 83 \\
         & Administration/Clerical/Reception & 80 \\
         & Health care (Physical \& Mental ) & 66 \\
         & Customer service & 48 \\
         & Management (Senior/Corporate) & 42 \\
         & Arts/Leisure/Entertainment & 37 \\
         &  Operations/Logistics & 34 \\
         & Homemaker & 25 \\
         & Student & 24 \\
         & Restaurant/Food service & 24 \\
         & Construction & 23 \\
         & Social service & 21 \\
         & HR Management & 17 \\
         & Consulting & 17 \\
         & Real Estate & 15 \\
         & Production & 14 \\
         & Research & 11 \\
         & Distribution & 9 \\
         & News/Information & 9 \\
         & Advertisement/PR & 8 \\
         & Architecture/Design & 8 \\
         & Retired & 8 \\
         & Beauty/Fashion & 3\\
         & Planning (meeting, events, etc.) & 2 \\
         & Buying/Purchasing & 2 \\
         
    \end{tabular}
    \caption{Counts of participants by Age, Gender, Education, and Employment Field.}
    \label{tab:demographics}
\end{table}
