# Supplementary material for: Measuring User Experience Inclusivity in Human-AI Interaction via Five User Problem-Solving Styles
Source: arXiv:2108.00588 source file (2024-02-17)
Supplement: Supplementary file 2 [file Appendix-Vignettes.tex]

\section{Vignettes}
\label{sec:appendix-vignettes}

\begin{table}[h]
\centering
\footnotesize
\begin{tabular}{|p{0.45\linewidth}|p{0.45\linewidth}|}
\hline

\textbf{Guideline 1 Application Vignette} & \textbf{Guideline 1 Violation Vignette} \\
\hline

You are using a presentation app similar to Microsoft PowerPoint, Google Slides, Apple Keynote to make slides for a presentation.
It is called [Application AI product].
[Application AI product] has a capability called Presenter Coach that gives you feedback on your presentation skills as you practice your presentation in front of your computer.
& 

You are using a presentation app similar to Microsoft PowerPoint, Google Slides, Apple Keynote to make slides for a presentation.
It is called [Application AI product].
[Application AI product] has a capability called Presenter Coach that gives you feedback on your presentation skills as you practice your presentation in front of your computer.\\
 & \\
 
When you turn on Presenter Coach, it displays information like this: As you practice your presentation, we will give you feedback about your presentation style: how fast you speak, use of filler words (such as ``um'' and ``like''), use of inappropriate words (such as ``damn'').
&

When you turn on Presenter Coach, it displays information like this: We will help you improve your presentation style.\\
\hline

\end{tabular}

\caption{Guideline 1's vignettes for guideline application (left) and violation (right). }
    
\label{table:G1-Vignette-Appendix}

\end{table}

\begin{table}[h]
\centering
\footnotesize
\begin{tabular}{|p{0.45\linewidth}|p{0.45\linewidth}|}
\hline

\textbf{Guideline 3 Application Vignette} & \textbf{Guideline 3 Violation Vignette} \\
\hline

You are using an email application called [Application AI product].
It is similar to Gmail, Outlook, Apple Mail, etc.
[Application AI product] pops up notifications on your screen when you have new emails.

& 

You are using an email application called [Violation AI product].
It is similar to Gmail, Outlook, Apple Mail, etc.
[Violation AI product] pops up notifications on your screen when you have new emails.\\

As you use [Application AI product], you notice that [Application AI product] stops the notifications when you are busy, for example, when giving a presentation.
&

As you use [Violation AI product], you notice that [Violation AI product] pops up notifications whenever a new email arrives, regardless of your activity.\\
\hline

\end{tabular}

\caption{Guideline 3's vignettes for guideline application (left) and violation (right). }
    
\label{table:G3-Vignette-Appendix}

\end{table}

\begin{table}[h]
\centering
\footnotesize
\begin{tabular}{|p{0.45\linewidth}|p{0.45\linewidth}|}
\hline

\textbf{Guideline 4 Application Vignette} & \textbf{Guideline 4 Violation Vignette} \\
\hline

You are using a document editing app called [Application] to write documents.
It is similar to MS Word, Google Docs, Apple Pages.
It has a feature that defines meanings of acronyms.
For example, if you see an acronym such as ``CDC'' in a document, you can access an explanation of what CDC stands for (such as, Centers for Disease Control).
& 

You are using a document editing app called [Violation] to write documents.
It is similar to MS Word, Google Docs, Apple Pages.
It has a feature that defines meanings of acronyms.
For example, if you see an acronym such as ``CDC'' in a document, you can access an explanation of what CDC stands for (such as, Centers for Disease Control).\\
 & \\
 
When you highlight an acronym to see what it stands for, {[Application] shows you definitions that are used in your workplace and pertain to the topic of the current document.}
&

When you highlight an acronym to see what it stands for, {[Violation] shows you a standard list of possible definitions taken from a popular acronym dictionary.}\\
\hline

\end{tabular}

\caption{Guideline 4's vignettes for guideline application (left) and violation (right).}
    
\label{table:G4-Vignette-Appendix}

\end{table}

\begin{table}[h]
\centering
\footnotesize
\begin{tabular}{|p{0.45\linewidth}|p{0.45\linewidth}|}
\hline

\textbf{Guideline 5 Application Vignette} & \textbf{Guideline 5 Violation Vignette} \\
\hline

You are using a document editing app called [Application AI product] to write documents.
It is similar to Microsoft Word, Google Docs, Apple Pages.
[Application AI product] has a feature that makes suggestions to improve your writing style.

& 

You are using a document editing app called [Violation AI product] to write documents.
It is similar to Microsoft Word, Google Docs, Apple Pages.
[Violation AI product] has a feature that makes suggestions to improve your writing style.\\

You are writing a document, and [Application AI product] presents its suggested options by saying:

``Consider using...''
&

You are writing a document, and [Violation AI product] presents its suggested options by saying:

``You made a mistake. Replace with...''\\
\hline

\end{tabular}

\caption{Guideline 5's vignettes for guideline application (left) and violation (right). }
    
\label{table:G5-Vignette-Appendix}

\end{table}

\begin{table}[h]
\centering
\footnotesize
\begin{tabular}{|p{0.45\linewidth}|p{0.45\linewidth}|}
\hline

\textbf{Guideline 6 Application Vignette} & \textbf{Guideline 6 Violation Vignette} \\
\hline

You are using an online search engine called [Application AI product] to search for images of CEOs and doctors.

& 

You are using an online search engine called [Violation AI product] to search for images of CEOs and doctors.\\

On the first page, the search results show images of different types of people in terms of gender and skin tone, including people who look like you.
&

The search results don't show any images of women or people of color on the first page.\\
\hline

\end{tabular}

\caption{Guideline 6's vignettes for guideline application (left) and violation (right). }
    
\label{table:G6-Vignette-Appendix}

\end{table}

\begin{table}[h]
\centering
\footnotesize
\begin{tabular}{|p{0.45\linewidth}|p{0.45\linewidth}|}
\hline

\textbf{Guideline 7 Application Vignette} & \textbf{Guideline 7 Violation Vignette} \\
\hline

You are using a presentation app similar to Microsoft PowerPoint, Google Slides, Apple Keynote to make slides for a presentation.
It is called [Application AI product].
[Application AI product] has a capability called Design Helper that provides alternative design ideas.
As you work on a slide and add text and images, Design Helper automatically provides you with design suggestions for alternative layouts.

& 

You are using a presentation app similar to Microsoft PowerPoint, Google Slides, Apple Keynote to make slides for a presentation.
It is called [Violation AI product].
[Violation AI product] has a capability called Design Helper that provides alternative design ideas.
As you work on a slide and add text and images, Design Helper automatically provides you with design suggestions for alternative layouts.\\

You are working on a slide and need some design help, but Design Helper hasn't automatically popped up any design suggestions.
You click a button visible on the interface to request suggestions and they appear on the side bar.

&

You are working on a slide and need some design help, but Design Helper hasn't automatically popped up any design suggestions.
There is no button visible on the interface that you could use to request suggestions from Design Helper.\\
\hline

\end{tabular}

\caption{Guideline 7's vignettes for guideline application (left) and violation (right). }
    
\label{table:G7-Vignette-Appendix}

\end{table}

\begin{table}[h]
\centering
\footnotesize
\begin{tabular}{|p{0.45\linewidth}|p{0.45\linewidth}|}
\hline

\textbf{Guideline 8 Application Vignette} & \textbf{Guideline 8 Violation Vignette} \\
\hline

You are using a presentation app similar to Microsoft PowerPoint, Google Slides, Apple Keynote to make slides for a presentation.
It is called [Application AI product].
[Application AI product] has a capability called Design Helper that provides alternative design ideas.
As you work on a slide and add text and images, Design Helper automatically provides you with design suggestions for alternative layouts.

& 

You are using a presentation app similar to Microsoft PowerPoint, Google Slides, Apple Keynote to make slides for a presentation.
It is called [Violation AI product].
[Violation AI product] has a capability called Design Helper that provides alternative design ideas.
As you work on a slide and add text and images, Design Helper automatically provides you with design suggestions for alternative layouts.\\

You are working on a slide and Design Helper pops up, showing you some design suggestions.
You do not need any design help at this time, so you click on a button visible on screen to hide the design suggestions.

&

You are working on a slide and Design Helper pops up, showing you some design suggestions.
You do not need any design help at this time, but there is no way to hide the design suggestions.\\
\hline

\end{tabular}

\caption{Guideline 8's vignettes for guideline application (left) and violation (right). }
    
\label{table:G8-Vignette-Appendix}

\end{table}

\begin{table}[h]
\centering
\footnotesize
\begin{tabular}{|p{0.45\linewidth}|p{0.45\linewidth}|}
\hline

\textbf{Guideline 9 Application Vignette} & \textbf{Guideline 9 Violation Vignette} \\
\hline

You are using a presentation app similar to Microsoft PowerPoint, Google Slides, Apple Keynote to make slides for a presentation.
It is called [Application AI product].
[Application AI product] has a capability called Design Helper that provides alternative design ideas.
As you work on a slide and add text and images, Design Helper automatically provides you with design suggestions for alternative layouts.

& 

You are using a presentation app similar to Microsoft PowerPoint, Google Slides, Apple Keynote to make slides for a presentation.
It is called [Violation AI product].
[Violation AI product] has a capability called Design Helper that provides alternative design ideas.
As you work on a slide and add text and images, Design Helper automatically provides you with design suggestions for alternative layouts.\\

You are working on a slide and Design Helper shows you a few design suggestions.
You click one of the suggestions, and the layout is applied to the current slide.
You decide you want to make a few changes to the layout, such as resizing or repositioning the images, which you can do directly on the slide.

&

You are working on a slide and Design Helper shows you a few design suggestions.
You click one of the suggestions, and the layout is applied to the current slide.
You decide you want to make a few changes to the layout, such as resizing or repositioning the images, but you see that it does not allow you to make changes.\\
\hline

\end{tabular}

\caption{Guideline 9's vignettes for guideline application (left) and violation (right). }
    
\label{table:G9-Vignette-Appendix}

\end{table}

\begin{table}[h]
\centering
\footnotesize
\begin{tabular}{|p{0.45\linewidth}|p{0.45\linewidth}|}
\hline

\textbf{Guideline 10 Application Vignette} & \textbf{Guideline 10 Violation Vignette} \\
\hline

You are using a document editing app called [Application AI product] to write documents.
It is similar to Microsoft Word, Google Docs, Apple Pages.
[Application AI product] has a spelling assistant that can automatically detect typos.

& 

You are using a document editing app called [Violation AI product] to write documents.
It is similar to Microsoft Word, Google Docs, Apple Pages.
[Violation AI product] has a spelling assistant that can automatically detect typos.\\

You are writing a document, and you make a typo.
The spelling assistant isn't sure what word you intended to type, so it provides multiple options for you to choose from.

&

You are writing a document, and you make a typo.
The spelling assistant isn't sure what word you intended to type, so it replaces the typo with its best bet.
For example, if you type ``multipl'', it automatically replaces it with ``multiple'', even though other options might make sense--e.g., multiple, multiplex.\\
\hline

\end{tabular}

\caption{Guideline 10's vignettes for guideline application (left) and violation (right). }
    
\label{table:G10-Vignette-Appendix}

\end{table}

\begin{table}[h]
\centering
\footnotesize
\begin{tabular}{|p{0.45\linewidth}|p{0.45\linewidth}|}
\hline

\textbf{Guideline 11 Application Vignette} & \textbf{Guideline 11 Violation Vignette} \\
\hline

You are using a spreadsheet app called [Application AI product] to analyze some data.
It is similar to MS Excel, Google Sheets, Apple Numbers.
[Application AI product] has a feature that suggests charts based on the data you have in a file.
For each suggested chart, the interface shows an interesting insight that summarizes the data--for example, ``People who walk to work drink more coffee than people who drive.''

& 

You are using a spreadsheet app called [Violation AI product] to analyze some data.
It is similar to MS Excel, Google Sheets, Apple Numbers.
[Violation AI product] has a feature that suggests charts based on the data you have in a file.
For each suggested chart, the interface shows an interesting insight that summarizes the data--for example, ``People who walk to work drink more coffee than people who drive.''\\

As you use [Application AI product], you wonder how each suggested chart and insight was generated, and you notice a button under each chart that you can click to access an explanation.
&

As you use [Violation AI product], you wonder how each suggested chart and insight was generated but are unable to access an explanation.\\
\hline

\end{tabular}

\caption{Guideline 11's vignettes for guideline application (left) and violation (right). }
    
\label{table:G11-Vignette-Appendix}

\end{table}

\begin{table}[h]
\centering
\footnotesize
\begin{tabular}{|p{0.45\linewidth}|p{0.45\linewidth}|}
\hline

\textbf{Guideline 12 Application Vignette} & \textbf{Guideline 12 Violation Vignette} \\
\hline

You are using an email application called [Application AI product].
It is similar to Gmail, Outlook, Apple Mail, etc.

& 

You are using an email application called [Violation AI product].
It is similar to Gmail, Outlook, Apple Mail, etc.\\

When attaching a file, [Application AI product] shows a list of recent files you worked on to choose from, along with a file explorer you can use to navigate to other files not in the list.
&

When attaching a file, [Violation AI product] opens a file explorer window you can use to navigate to files.\\
\hline

\end{tabular}

\caption{Guideline 12's vignettes for guideline application (left) and violation (right). }
    
\label{table:G12-Vignette-Appendix}

\end{table}

\begin{table}[h]
\centering
\footnotesize
\begin{tabular}{|p{0.45\linewidth}|p{0.45\linewidth}|}
\hline

\textbf{Guideline 13 Application Vignette} & \textbf{Guideline 13 Violation Vignette} \\
\hline

You are using a presentation app similar to Microsoft PowerPoint, Google Slides, Apple Keynote to make slides for a presentation.
It is called [Application AI product].
[Application AI product] has a capability called Design Helper that provides alternative design ideas.
As you work on a slide and add text and images, Design Helper automatically provides you with design suggestions for alternative layouts.

& 

You are using a presentation app similar to Microsoft PowerPoint, Google Slides, Apple Keynote to make slides for a presentation.
It is called [Violation AI product].
[Violation AI product] has a capability called Design Helper that provides alternative design ideas.
As you work on a slide and add text and images, Design Helper automatically provides you with design suggestions for alternative layouts.\\

As you make slides, you pick from the design suggestions offered by Design Helper.
You usually pick designs that feature the color blue.
After using [Application AI product] a few times, you notice it has learned your preferences and now features blue designs prominently.

&

As you make slides, you pick from the design suggestions offered by Design Helper.
You usually pick designs that feature the color blue.
After using [Violation AI product] a few times, you notice it has not learned your preferences, and blue designs appear in the same place among the suggested designs as the first time you used it.\\
\hline

\end{tabular}

\caption{Guideline 13's vignettes for guideline application (left) and violation (right). }
    
\label{table:G13-Vignette-Appendix}

\end{table}

\begin{table}[h]
\centering
\footnotesize
\begin{tabular}{|p{0.45\linewidth}|p{0.45\linewidth}|}
\hline

\textbf{Guideline 14 Application Vignette} & \textbf{Guideline 14 Violation Vignette} \\
\hline

You are using a document editing app similar to Microsoft Word, Google Docs, Apple Pages, called [Application AI product]

& 

You are using a document editing app similar to Microsoft Word, Google Docs, Apple Pages, called [Violation AI product]\\

As you work on a document, the app automatically updates a small dedicated part of the menu bar at the top right, based on what functionality it thinks you'll need next.
The rest of the menu bar never changes.

&

As you work on a document, the app automatically updates the entire menu bar at the top based on what functionality it thinks you'll need next.\\
\hline

\end{tabular}

\caption{Guideline 14's vignettes for guideline application (left) and violation (right). }
    
\label{table:G14-Vignette-Appendix}

\end{table}

\begin{table}[h]
\centering
\footnotesize
\begin{tabular}{|p{0.45\linewidth}|p{0.45\linewidth}|}
\hline

\textbf{Guideline 15 Application Vignette} & \textbf{Guideline 15 Violation Vignette} \\
\hline

You are using a spreadsheet app called [Application AI product] to analyze some data.
It is similar to MS Excel, Google Sheets, Apple Numbers.
[Application AI product] has a feature that suggests charts based on the data you have in a file.

& 

You are using a spreadsheet app called [Violation AI product] to analyze some data.
It is similar to MS Excel, Google Sheets, Apple Numbers.
[Violation AI product] has a feature that suggests charts based on the data you have in a file.\\

Below each suggested chart, [Application AI product] shows buttons you can use to provide feedback as to whether that suggestion is useful to you or not.
&

[Violation AI product] does not have a way for you to provide feedback as to whether any suggestion is useful to you or not.\\
\hline

\end{tabular}

\caption{Guideline 15's vignettes for guideline application (left) and violation (right). }
    
\label{table:G15-Vignette-Appendix}

\end{table}

\begin{table}[h]
\centering
\footnotesize
\begin{tabular}{|p{0.45\linewidth}|p{0.45\linewidth}|}
\hline

\textbf{Guideline 17 Application Vignette} & \textbf{Guideline 17 Violation Vignette} \\
\hline

You are using an email application called [Application AI product].
It is similar to Gmail, Outlook, Apple Mail, etc.
[Application AI product] can automatically sort your emails into 2 categories: \textit{important} email and \textit{other} emails.

& 

You are using an email application called [Violation AI product].
It is similar to Gmail, Outlook, Apple Mail, etc.
[Violation AI product] can automatically sort your emails into 2 categories: \textit{important} email and \textit{other} emails.\\

As you use [Application AI product], you notice that emails from some important people (e.g., your boss, your mom) are not being marked as \textit{important}.
[Application AI product] provides a setting where you can enter the names of specific people to make sure they are always marked as \textit{important} going forward.
&

As you use [Violation AI product], you notice that emails from some important people (e.g., your boss, your mom) are not being marked as \textit{important}.
Going forward, you periodically check the \textit{other} email category to make sure you are not missing emails from those \textit{important} people.\\
\hline

\end{tabular}

\caption{Guideline 17's vignettes for guideline application (left) and violation (right). }
    
\label{table:G17-Vignette-Appendix}

\end{table}

\begin{table}[h]
\centering
\footnotesize
\begin{tabular}{|p{0.45\linewidth}|p{0.45\linewidth}|}
\hline

\textbf{Guideline 18 Application Vignette} & \textbf{Guideline 18 Violation Vignette} \\
\hline

You are using an email application called [Application AI product].
It is similar to Gmail, Outlook, Apple Mail, etc.
[Application AI product] can automatically sort your emails into 2 categories: \textit{important} email and \textit{other} emails.

& 

You are using an email application called [Violation AI product].
It is similar to Gmail, Outlook, Apple Mail, etc.
[Violation AI product] can automatically sort your emails into 2 categories: \textit{important} email and \textit{other} emails.\\

Occasionally, [Application AI product] improves the way it sorts emails into \textit{important} and \textit{other}.
For example, one day it informs you that:

\begin{itemize}
    \item ``From now on, emails Sarah [your boss] will always appear in the important category and emails from Local News [some mailing lists] will no longer appear the important category.''
\end{itemize}
&

Occasionally, [Violation AI product] improves the way it sorts emails into \textit{important} and \textit{other}.
For example, as you use it, you notice that emails from your boss start to appear in the important category when they didn't always before and emails from some mailing lists no longer seem to appear in the important category.\\
\hline

\end{tabular}

\caption{Guideline 18's vignettes for guideline application (left) and violation (right). }
    
\label{table:G18-Vignette-Appendix}

\end{table}

\clearpage
