# Supplementary material for: Measuring User Experience Inclusivity in Human-AI Interaction via Five User Problem-Solving Styles
Source: arXiv:2108.00588 source file (2024-02-17)
Supplement: Supplementary file 3 [file Learn-Appendix.tex]

%Guideline 1 ------------------------------
\begin{table}[]
    \centering
    \begin{tabular}{cc|cc|cc|cc|cc}
    \multicolumn{2}{c|}{\includegraphics[width = 0.16\columnwidth]{assets/05-All-BoxPlots/01-G1/Learn/G1-Feel-In-Control-LEARN.png}} &
    \multicolumn{2}{c|}{\includegraphics[width = 0.16\columnwidth]{assets/05-All-BoxPlots/01-G1/Learn/G1-Feel-Secure-LEARN.png}} &
    \multicolumn{2}{c|}{\includegraphics[width = 0.16\columnwidth]{assets/05-All-BoxPlots/01-G1/Learn/G1-Feel-Adequate-LEARN.png}} &
    \multicolumn{2}{c|}{\includegraphics[width = 0.16\columnwidth]{assets/05-All-BoxPlots/01-G1/Learn/G1-Feel-Certain-LEARN.png}} &
    \multicolumn{2}{c}{\includegraphics[width = 0.16\columnwidth]{assets/05-All-BoxPlots/01-G1/Learn/G1-Feel-Productive-LEARN.png}}
    \\
    \hline
    \hline
    \multicolumn{2}{c|}{\includegraphics[width = 0.16\columnwidth]{assets/05-All-BoxPlots/01-G1/Learn/G1-Perceived-Useful-LEARN.png}} &
    \multicolumn{2}{c|}{\includegraphics[width = 0.16\columnwidth]{assets/05-All-BoxPlots/01-G1/Learn/G1-Not-Suspicious-LEARN.png}} &
    \multicolumn{2}{c|}{\includegraphics[width = 0.16\columnwidth]{assets/05-All-BoxPlots/01-G1/Learn/G1-Not-Harmful-LEARN.png}} &
    \multicolumn{2}{c|}{\includegraphics[width = 0.16\columnwidth]{assets/05-All-BoxPlots/01-G1/Learn/G1-Product-Reliable-LEARN.png}} &
    \multicolumn{2}{c}{\includegraphics[width = 0.16\columnwidth]{assets/05-All-BoxPlots/01-G1/Learn/G1-Trust-Product-LEARN.png}}
    \end{tabular}
    
    \caption{Guideline 1 participants' ratings for all dependent variables, disaggregated by participants' learning styles: by process vs. by tinkering.
	%For the disaggregated data, notice how large the distances between the average rating are when the guideline is applied.
	Table~\ref{tab:G1-Learn-Stats-Appendix} below provides the statistics (where applicable).
}
    \label{fig:Learn-G1-Appendix}
\end{table}

\begin{table}[h]

%\framebox[\linewidth]{For Measuring!}
\centering
\footnotesize

    \begin{tabular}{p{0.22\columnwidth}|c|c|c|c|c|c}
    
    \rowcolor{LightGray}\multicolumn{7}{c}{\textbf{Violation AI Product}}\\
    \hline
    \textbf{Dependent}  & \textbf{Distance b/w} &  &  & & \textbf{Bonferroni} &  \\
    \textbf{variable} & \textbf{Means} &  \textbf{df} &  \textbf{t-val} &   \textbf{p-value}  & \textbf{correction} & \textbf{Cohen's \textit{d}} \\
    \hline
    
    I would feel in control & - - - & - &  - - - & - - - & - - - & - - -\\
    \hline
    
    I would feel secure & - - - & - &  - - - & - - - & - - - & - - - \\
    \hline
    
    I would feel adequate & - - - & - &  - - - & - - - & - - - & - - - \\
    \hline
    
    I would feel certain & - - - & - &  - - - & - - - & - - - & - - - \\
    \hline
    
    I would feel productive & - - - & - &  - - - & - - - & - - - & - - -  \\
    \hline
    \hline
    
    I perceived it as useful &  - - - & - &  - - - & - - - & - - - & - - -  \\
    \hline
    
    I would not be suspicious & - - - & - &  - - - & - - - & - - - & - - -  \\
    \hline
    
    It would not be harmful & - - - & - &  - - - & - - - & - - - & - - -  \\
    \hline
    
    I find the product reliable & - - - & - &  - - - & - - - & - - - & - - -  \\
    \hline
    
    I would trust the product & - - - & - &  - - - & - - - & - - - & - - - \\
    \hline

    \rowcolor{LightGray}\multicolumn{7}{c}{\textbf{Application AI Product}}\\
    \hline
    \textbf{Dependent}  & \textbf{Distance b/w} &  &  & & \textbf{Bonferroni} &  \\
    \textbf{variable} & \textbf{Means} &  \textbf{df} &  \textbf{t-val} &   \textbf{p-value}  & \textbf{correction} & \textbf{Cohen's \textit{d}} \\
    \hline
    
    I would feel in control & - - - & - &  - - - & - - - & - - - & - - -  \\
    \hline
    
    I would feel secure & - - - & - &  - - - & - - - & - - - & - - - \\
    \hline
    
    I would feel adequate & - - - & - &  - - - & - - - & - - - & - - - \\
    \hline
    
    I would feel certain & - - - & - &  - - - & - - - & - - - & - - - \\
    \hline
    
    I would feel productive & - - - & - &  - - - & - - - & - - - & - - -   \\
    \hline
    \hline
    
    I perceived it as useful &  - - - & - &  - - - & - - - & - - - & - - -  \\
    \hline
    
    I would not be suspicious & - - - & - &  - - - & - - - & - - - & - - -  \\
    \hline
    
    It would not be harmful & - - - & - &  - - - & - - - & - - - & - - -  \\
    \hline
    
    I find the product reliable & - - - & - &  - - - & - - - & - - - & - - - \\
    \hline
    
    I would trust the product & - - - & - &  - - - & - - - & - - - & - - -

    \end{tabular}

    \caption{Guideline 1's t-test results %(\checkmark if Welch's t-test) 
    for the ``by process'' learning style vs. the ``by tinkering'' learning style participants' average ratings of the independent Violation AI product (top) and Application AI product (bottom), for all 10 dependent variables.
    If dashes (- - -) are present, no statistical test was performed.
    If the number of tests exceeded 5 for each product, Bonferroni correction applied by multiplying p-values by the number of tests performed.
    }
    \label{tab:G1-Learn-Stats-Appendix}
    
    % \FIXME{MMB@AAA: FYI, I took the \checkmark s out and replaced them with plain text, because the \checkmark vs blank visually stood out so much, I kept mis-seeing it as saying only those 4 rows were signif. or important.\\
    % AAA@MMB: Redid it with Y/N. The Welch's t and t were cluttering up the table too much.\\
    % MMB@AAA: I actually prefer the spelled-out way.  Visually, the table layout now screams WELCHES IS GOOD, and draws attention away from all other columns.  Meta-comment: it might help if you forced yourself to look at this paper with a reader hat on.}

\end{table}

\clearpage
%---------------------------------------------------- End Guideline 1

%Guideline 3 ------------------------------
\begin{table}[]
    \centering
    \begin{tabular}{cc|cc|cc|cc|cc}
    \multicolumn{2}{c|}{\includegraphics[width = 0.16\columnwidth]{assets/05-All-BoxPlots/02-G3/Learn/G3-Feel-In-Control-LEARN.png}} &
    \multicolumn{2}{c|}{\includegraphics[width = 0.16\columnwidth]{assets/05-All-BoxPlots/02-G3/Learn/G3-Feel-Secure-LEARN.png}} &
    \multicolumn{2}{c|}{\includegraphics[width = 0.16\columnwidth]{assets/05-All-BoxPlots/02-G3/Learn/G3-Feel-Adequate-LEARN.png}} &
    \multicolumn{2}{c|}{\includegraphics[width = 0.16\columnwidth]{assets/05-All-BoxPlots/02-G3/Learn/G3-Feel-Certain-LEARN.png}} &
    \multicolumn{2}{c}{\includegraphics[width = 0.16\columnwidth]{assets/05-All-BoxPlots/02-G3/Learn/G3-Feel-Productive-LEARN.png}}
    \\
    \hline
    \hline
    \multicolumn{2}{c|}{\includegraphics[width = 0.16\columnwidth]{assets/05-All-BoxPlots/02-G3/Learn/G3-Perceived-Useful-LEARN.png}} &
    \multicolumn{2}{c|}{\includegraphics[width = 0.16\columnwidth]{assets/05-All-BoxPlots/02-G3/Learn/G3-Not-Suspicious-LEARN.png}} &
    \multicolumn{2}{c|}{\includegraphics[width = 0.16\columnwidth]{assets/05-All-BoxPlots/02-G3/Learn/G3-Not-Harmful-LEARN.png}} &
    \multicolumn{2}{c|}{\includegraphics[width = 0.16\columnwidth]{assets/05-All-BoxPlots/02-G3/Learn/G3-Product-Reliable-LEARN.png}} &
    \multicolumn{2}{c}{\includegraphics[width = 0.16\columnwidth]{assets/05-All-BoxPlots/02-G3/Learn/G3-Trust-Product-LEARN.png}}
    \end{tabular}
    
    \caption{Guideline 3 participants' ratings for all dependent variables, disaggregated by participants' learning styles: by process vs. by tinkering.
	%For the disaggregated data, notice how large the distances between the average rating are when the guideline is applied.
	Table~\ref{tab:G3-Learn-Stats-Appendix} below provides the statistics (where applicable).
}
    \label{fig:Learn-G3-Appendix}
\end{table}

\begin{table}[h]

%\framebox[\linewidth]{For Measuring!}
\centering
\footnotesize

    \begin{tabular}{p{0.22\columnwidth}|c|c|c|c|c|c}
    
    \rowcolor{LightGray}\multicolumn{7}{c}{\textbf{Violation AI Product}}\\
    \hline
    \textbf{Dependent}  & \textbf{Distance b/w} &  &  & & \textbf{Bonferroni} &  \\
    \textbf{variable} & \textbf{Means} &  \textbf{df} &  \textbf{t-val} &   \textbf{p-value}  & \textbf{correction} & \textbf{Cohen's \textit{d}} \\
    \hline
    
    I would feel in control & - - - & - &  - - - & - - - & - - - & - - -\\
    \hline
    
    I would feel secure & - - - & - &  - - - & - - - & - - - & - - - \\
    \hline
    
    I would feel adequate & - - - & - &  - - - & - - - & - - - & - - - \\
    \hline
    
    I would feel certain & - - - & - &  - - - & - - - & - - - & - - - \\
    \hline
    
    I would feel productive & - - - & - &  - - - & - - - & - - - & - - -  \\
    \hline
    \hline
    
    I perceived it as useful &  - - - & - &  - - - & - - - & - - - & - - -  \\
    \hline
    
    I would not be suspicious & .6598 & 64 &  2.0925 & \cellcolor{TimBlueQuote}.0404 & - - - & .5212  \\
    \hline
    
    It would not be harmful & - - - & - &  - - - & - - - & - - - & - - -  \\
    \hline
    
    I find the product reliable & - - - & - &  - - - & - - - & - - - & - - -  \\
    \hline
    
    I would trust the product & - - - & - &  - - - & - - - & - - - & - - - \\
    \hline

    \rowcolor{LightGray}\multicolumn{7}{c}{\textbf{Application AI Product}}\\
    \hline
    \textbf{Dependent}  & \textbf{Distance b/w} &  &  & & \textbf{Bonferroni} &  \\
    \textbf{variable} & \textbf{Means} &  \textbf{df} &  \textbf{t-val} &   \textbf{p-value}  & \textbf{correction} & \textbf{Cohen's \textit{d}} \\
    \hline
    
    I would feel in control & - - - & - &  - - - & - - - & - - - & - - -  \\
    \hline
    
    I would feel secure & - - - & - &  - - - & - - - & - - - & - - - \\
    \hline
    
    I would feel adequate & - - - & - &  - - - & - - - & - - - & - - - \\
    \hline
    
    I would feel certain & - - - & - &  - - - & - - - & - - - & - - - \\
    \hline
    
    I would feel productive & - - - & - &  - - - & - - - & - - - & - - -   \\
    \hline
    \hline
    
    I perceived it as useful &  - - - & - &  - - - & - - - & - - - & - - -  \\
    \hline
    
    I would not be suspicious & - - - & - &  - - - & - - - & - - - & - - -  \\
    \hline
    
    It would not be harmful & - - - & - &  - - - & - - - & - - - & - - -  \\
    \hline
    
    I find the product reliable & - - - & - &  - - - & - - - & - - - & - - - \\
    \hline
    
    I would trust the product & - - - & - &  - - - & - - - & - - - & - - -

    \end{tabular}

    \caption{Guideline 3's t-test results %(\checkmark if Welch's t-test) 
    for the ``by process'' learning style vs. the ``by tinkering'' learning style participants' average ratings of the independent Violation AI product (top) and Application AI product (bottom), for all 10 dependent variables.
    If dashes (- - -) are present, no statistical test was performed.
    If the number of tests exceeded 5 for each product, Bonferroni correction applied by multiplying p-values by the number of tests performed.
    }
    \label{tab:G3-Learn-Stats-Appendix}
    
    % \FIXME{MMB@AAA: FYI, I took the \checkmark s out and replaced them with plain text, because the \checkmark vs blank visually stood out so much, I kept mis-seeing it as saying only those 4 rows were signif. or important.\\
    % AAA@MMB: Redid it with Y/N. The Welch's t and t were cluttering up the table too much.\\
    % MMB@AAA: I actually prefer the spelled-out way.  Visually, the table layout now screams WELCHES IS GOOD, and draws attention away from all other columns.  Meta-comment: it might help if you forced yourself to look at this paper with a reader hat on.}

\end{table}

\clearpage
%---------------------------------------------------- End Guideline 3

%Begin Guideline 4----------------------------------------------------

\begin{table}[]
    \centering
    \begin{tabular}{cc|cc|cc|cc|cc}
    \multicolumn{2}{c|}{\includegraphics[width = 0.16\columnwidth]{assets/05-All-BoxPlots/03-G4/Learn/G4-Feel-In-Control-LEARN.png}} &
    \multicolumn{2}{c|}{\includegraphics[width = 0.16\columnwidth]{assets/05-All-BoxPlots/03-G4/Learn/G4-Feel-Secure-LEARN.png}} &
    \multicolumn{2}{c|}{\includegraphics[width = 0.16\columnwidth]{assets/05-All-BoxPlots/03-G4/Learn/G4-Feel-Adequate-LEARN.png}} &
    \multicolumn{2}{c|}{\includegraphics[width = 0.16\columnwidth]{assets/05-All-BoxPlots/03-G4/Learn/G4-Feel-Certain-LEARN.png}} &
    \multicolumn{2}{c}{\includegraphics[width = 0.16\columnwidth]{assets/05-All-BoxPlots/03-G4/Learn/G4-Feel-Productive-LEARN.png}}
    \\
    \hline
    \hline
    \multicolumn{2}{c|}{\includegraphics[width = 0.16\columnwidth]{assets/05-All-BoxPlots/03-G4/Learn/G4-Perceived-Useful-LEARN.png}} &
    \multicolumn{2}{c|}{\includegraphics[width = 0.16\columnwidth]{assets/05-All-BoxPlots/03-G4/Learn/G4-Not-Suspicious-LEARN.png}} &
    \multicolumn{2}{c|}{\includegraphics[width = 0.16\columnwidth]{assets/05-All-BoxPlots/03-G4/Learn/G4-Not-Harmful-LEARN.png}} &
    \multicolumn{2}{c|}{\includegraphics[width = 0.16\columnwidth]{assets/05-All-BoxPlots/03-G4/Learn/G4-Product-Reliable-LEARN.png}} &
    \multicolumn{2}{c}{\includegraphics[width = 0.16\columnwidth]{assets/05-All-BoxPlots/03-G4/Learn/G4-Trust-Product-LEARN.png}}
    \end{tabular}
    
    \caption{Guideline 4 participants' ratings for all dependent variables, disaggregated by participants' learning styles: by process vs. by tinkering.
	%For the disaggregated data, notice how large the distances between the average rating are when the guideline is applied.
	Table~\ref{tab:G4-Learn-Stats-Appendix} below provides the statistics (where applicable).
}
    \label{fig:Learn-G4-Appendix}
\end{table}

\begin{table}[h]

%\framebox[\linewidth]{For Measuring!}
\centering
\footnotesize

    \begin{tabular}{p{0.22\columnwidth}|c|c|c|c|c|c}
    
    \rowcolor{LightGray}\multicolumn{7}{c}{\textbf{Violation AI Product}}\\
    \hline
    \textbf{Dependent}  & \textbf{Distance b/w} &  &  & & \textbf{Bonferroni} &  \\
    \textbf{variable} & \textbf{Means} &  \textbf{df} &  \textbf{t-val} &   \textbf{p-value}  & \textbf{correction} & \textbf{Cohen's \textit{d}} \\
    \hline
    
    I would feel in control & - - - & - &  - - - & - - - & - - - & - - - \\
    \hline
    
    I would feel secure & - - - & - &  - - - & - - - & - - - & - - - \\
    \hline
    
    I would feel adequate & - - - & - &  - - - & - - - & - - - & - - - \\
    \hline
    
    I would feel certain & - - - & - &  - - - & - - - & - - - & - - - \\
    \hline
    
    I would feel productive & - - - & - &  - - - & - - - & - - - & - - -  \\
    \hline
    \hline
    
    I perceived it as useful &  0.4757 & 62  & 1.5241 & .1326 & - - -  & .3879 \\
    \hline
    
    I would not be suspicious & - - - & - &  - - - & - - - & - - - & - - -  \\
    \hline
    
    It would not be harmful & 0.6014 & 63  & 2.239  & \cellcolor{AbiOrangeQuote}.0287  & - - -   & .5636  \\
    \hline
    
    I find the product reliable & - - - & - &  - - - & - - - & - - - & - - -  \\
    \hline
    
    I would trust the product & - - - & - &  - - - & - - - & - - - & - - - \\
    \hline

    \rowcolor{LightGray}\multicolumn{7}{c}{\textbf{Application AI Product}}\\
    \hline
    \textbf{Dependent}  & \textbf{Distance b/w} &  &  & & \textbf{Bonferroni} &  \\
    \textbf{variable} & \textbf{Means} &  \textbf{df} &  \textbf{t-val} &   \textbf{p-value}  & \textbf{correction} & \textbf{Cohen's \textit{d}} \\
    \hline
    
    I would feel in control & - - - & - &  - - -  &  - - -  & - - -  & - - -  \\
    \hline
    
    I would feel secure & - - - & - &  - - - & - - - & - - - & - - - \\
    \hline
    
    I would feel adequate & - - - & - &  - - - & - - - & - - - & - - - \\
    \hline
    
    I would feel certain & 0.9581 &  63 & 2.3906 & \cellcolor{AbiOrangeQuote}{.0198} & - - - & .6017 \\
    \hline
    
    I would feel productive & .6628 & 63  & 2.7159  & \cellcolor{AbiOrangeQuote} .0085  &  - - - & .6836   \\
    \hline
    \hline
    
    I perceived it as useful &  0.7310 & 63  & 2.7220  &  \cellcolor{AbiOrangeQuote} .0084  & - - -   & .6851   \\
    \hline
    
    I would not be suspicious & - - - & - &  - - - & - - - & - - - & - - -   \\
    \hline
    
    It would not be harmful & 0.3596 & 63  & 1.1400  & .2586  &  - - -  & .2869  \\
    \hline
    
    I find the product reliable & - - - & - &  - - - & - - - & - - - & - - - \\
    \hline
    
    I would trust the product & - - - & - &  - - - & - - - & - - - & - - -

    \end{tabular}

    \caption{Guideline 4's t-test results %(\checkmark if Welch's t-test) 
    for the ``by process'' learning style vs. the ``by tinkering'' learning style participants' average ratings of the independent Violation AI product (top) and Application AI product (bottom), for all 10 dependent variables.
    If dashes (- - -) are present, no statistical test was performed.
    If the number of tests exceeded 5 for each product, Bonferroni correction applied by multiplying p-values by the number of tests performed.
    }
    \label{tab:G4-Learn-Stats-Appendix}
\end{table}

%---------------------------------------------------- End Guideline 4

\clearpage

%Begin Guideline 5----------------------------------------------------

\begin{table}[]
    \centering
    \begin{tabular}{cc|cc|cc|cc|cc}
    \multicolumn{2}{c|}{\includegraphics[width = 0.16\columnwidth]{assets/05-All-BoxPlots/04-G5/Learn/G5-Feel-In-Control-LEARN.png}} &
    \multicolumn{2}{c|}{\includegraphics[width = 0.16\columnwidth]{assets/05-All-BoxPlots/04-G5/Learn/G5-Feel-Secure-LEARN.png}} &
    \multicolumn{2}{c|}{\includegraphics[width = 0.16\columnwidth]{assets/05-All-BoxPlots/04-G5/Learn/G5-Feel-Adequate-LEARN.png}} &
    \multicolumn{2}{c|}{\includegraphics[width = 0.16\columnwidth]{assets/05-All-BoxPlots/04-G5/Learn/G5-Feel-Certain-LEARN.png}} &
    \multicolumn{2}{c}{\includegraphics[width = 0.16\columnwidth]{assets/05-All-BoxPlots/04-G5/Learn/G5-Feel-Productive-LEARN.png}}
    \\
    \hline
    \hline
    \multicolumn{2}{c|}{\includegraphics[width = 0.16\columnwidth]{assets/05-All-BoxPlots/04-G5/Learn/G5-Perceived-Useful-LEARN.png}} &
    \multicolumn{2}{c|}{\includegraphics[width = 0.16\columnwidth]{assets/05-All-BoxPlots/04-G5/Learn/G5-Not-Suspicious-LEARN.png}} &
    \multicolumn{2}{c|}{\includegraphics[width = 0.16\columnwidth]{assets/05-All-BoxPlots/04-G5/Learn/G5-Not-Harmful-LEARN.png}} &
    \multicolumn{2}{c|}{\includegraphics[width = 0.16\columnwidth]{assets/05-All-BoxPlots/04-G5/Learn/G5-Product-Reliable-LEARN.png}} &
    \multicolumn{2}{c}{\includegraphics[width = 0.16\columnwidth]{assets/05-All-BoxPlots/04-G5/Learn/G5-Trust-Product-LEARN.png}}
    \end{tabular}
    
    \caption{Guideline 5 participants' ratings for all dependent variables, disaggregated by participants' learning styles: by process vs. by tinkering.
	%For the disaggregated data, notice how large the distances between the average rating are when the guideline is applied.
	Table~\ref{tab:G5-Learn-Stats-Appendix} below provides the statistics (where applicable).
}
    \label{fig:Learn-G5-Appendix}
\end{table}

\begin{table}[h]

%\framebox[\linewidth]{For Measuring!}
\centering
\footnotesize

    \begin{tabular}{p{0.22\columnwidth}|c|c|c|c|c|c}
    
    \rowcolor{LightGray}\multicolumn{7}{c}{\textbf{Violation AI Product}}\\
    \hline
    \textbf{Dependent}  & \textbf{Distance b/w} &  &  & & \textbf{Bonferroni} &  \\
    \textbf{variable} & \textbf{Means} &  \textbf{df} &  \textbf{t-val} &   \textbf{p-value}  & \textbf{correction} & \textbf{Cohen's \textit{d}} \\
    \hline
    
    I would feel in control & - - - & - &  - - - & - - - & - - - & - - - \\
    \hline
    
    I would feel secure & - - - & - &  - - - & - - - & - - - & - - - \\
    \hline
    
    I would feel adequate & - - - & - &  - - - & - - - & - - - & - - - \\
    \hline
    
    I would feel certain & - - - & - &  - - - & - - - & - - - & - - - \\
    \hline
    
    I would feel productive & .3285 & 67 &  0.9671 & .3370 & - - - & .2335  \\
    \hline
    \hline
    
    I perceived it as useful &  .4907 & 67 &  1.3401 & .1847 & - - - & .3235  \\
    \hline
    
    I would not be suspicious & - - - & - &  - - - & - - - & - - - & - - -  \\
    \hline
    
    It would not be harmful & - - - & - &  - - - & - - - & - - - & - - -  \\
    \hline
    
    I find the product reliable & - - - & - &  - - - & - - - & - - - & - - -  \\
    \hline
    
    I would trust the product & - - - & - &  - - - & - - - & - - - & - - - \\
    \hline

    \rowcolor{LightGray}\multicolumn{7}{c}{\textbf{Application AI Product}}\\
    \hline
    \textbf{Dependent}  & \textbf{Distance b/w} &  &  & & \textbf{Bonferroni} &  \\
    \textbf{variable} & \textbf{Means} &  \textbf{df} &  \textbf{t-val} &   \textbf{p-value}  & \textbf{correction} & \textbf{Cohen's \textit{d}} \\
    \hline
    
    I would feel in control & - - - & - &  - - - & - - - & - - - & - - -  \\
    \hline
    
    I would feel secure & - - - & - &  - - - & - - - & - - - & - - - \\
    \hline
    
    I would feel adequate & - - - & - &  - - - & - - - & - - - & - - - \\
    \hline
    
    I would feel certain & - - - & - &  - - - & - - - & - - - & - - - \\
    \hline
    
    I would feel productive & 0.7249 & 65 &  2.1491 & \cellcolor{TimBlueQuote}.0354 & - - - & .5266 \\
    \hline
    \hline
    
    I perceived it as useful &  - - - & - &  - - - & - - - & - - - & - - -   \\
    \hline
    
    I would not be suspicious & - - - & - &  - - - & - - - & - - - & - - -   \\
    \hline
    
    It would not be harmful & - - - & - &  - - - & - - - & - - - & - - -  \\
    \hline
    
    I find the product reliable & - - - & - &  - - - & - - - & - - - & - - - \\
    \hline
    
    I would trust the product & - - - & - &  - - - & - - - & - - - & - - -

    \end{tabular}

    \caption{Guideline 5's t-test results %(\checkmark if Welch's t-test) 
    for the ``by process'' learning style vs. the ``by tinkering'' learning style participants' average ratings of the independent Violation AI product (top) and Application AI product (bottom), for all 10 dependent variables.
    If dashes (- - -) are present, no statistical test was performed.
    If the number of tests exceeded 5 for each product, Bonferroni correction applied by multiplying p-values by the number of tests performed.
    }
    \label{tab:G5-Learn-Stats-Appendix}
\end{table}

%---------------------------------------------------- End Guideline 5

\clearpage

%Begin Guideline 6----------------------------------------------------

\begin{table}[]
    \centering
    \begin{tabular}{cc|cc|cc|cc|cc}
    \multicolumn{2}{c|}{\includegraphics[width = 0.16\columnwidth]{assets/05-All-BoxPlots/05-G6/Learn/G6-Feel-In-Control-LEARN.png}} &
    \multicolumn{2}{c|}{\includegraphics[width = 0.16\columnwidth]{assets/05-All-BoxPlots/05-G6/Learn/G6-Feel-Secure-LEARN.png}} &
    \multicolumn{2}{c|}{\includegraphics[width = 0.16\columnwidth]{assets/05-All-BoxPlots/05-G6/Learn/G6-Feel-Adequate-LEARN.png}} &
    \multicolumn{2}{c|}{\includegraphics[width = 0.16\columnwidth]{assets/05-All-BoxPlots/05-G6/Learn/G6-Feel-Certain-LEARN.png}} &
    \multicolumn{2}{c}{\includegraphics[width = 0.16\columnwidth]{assets/05-All-BoxPlots/05-G6/Learn/G6-Feel-Productive-LEARN.png}}
    \\
    \hline
    \hline
    \multicolumn{2}{c|}{\includegraphics[width = 0.16\columnwidth]{assets/05-All-BoxPlots/05-G6/Learn/G6-Perceived-Useful-LEARN.png}} &
    \multicolumn{2}{c|}{\includegraphics[width = 0.16\columnwidth]{assets/05-All-BoxPlots/05-G6/Learn/G6-Not-Suspicious-LEARN.png}} &
    \multicolumn{2}{c|}{\includegraphics[width = 0.16\columnwidth]{assets/05-All-BoxPlots/05-G6/Learn/G6-Not-Harmful-LEARN.png}} &
    \multicolumn{2}{c|}{\includegraphics[width = 0.16\columnwidth]{assets/05-All-BoxPlots/05-G6/Learn/G6-Product-Reliable-LEARN.png}} &
    \multicolumn{2}{c}{\includegraphics[width = 0.16\columnwidth]{assets/05-All-BoxPlots/05-G6/Learn/G6-Trust-Product-LEARN.png}}
    \end{tabular}
    
    \caption{Guideline 6 participants' ratings for all dependent variables, disaggregated by participants' learning styles: by process vs. by tinkering.
	%For the disaggregated data, notice how large the distances between the average rating are when the guideline is applied.
	Table~\ref{tab:G6-Learn-Stats-Appendix} below provides the statistics (where applicable).
}
    \label{fig:Learn-G6-Appendix}
\end{table}

\begin{table}[h]

%\framebox[\linewidth]{For Measuring!}
\centering
\footnotesize

    \begin{tabular}{p{0.22\columnwidth}|c|c|c|c|c|c}
    
    \rowcolor{LightGray}\multicolumn{7}{c}{\textbf{Violation AI Product}}\\
    \hline
    \textbf{Dependent}  & \textbf{Distance b/w} &  &  & & \textbf{Bonferroni} &  \\
    \textbf{variable} & \textbf{Means} &  \textbf{df} &  \textbf{t-val} &   \textbf{p-value}  & \textbf{correction} & \textbf{Cohen's \textit{d}} \\
    \hline
    
    I would feel in control & 0.7759 & 59 &  1.9802 & .0524 & - - - & .5077 \\
    \hline
    
    I would feel secure & 0.6333 & 60 &  1.8450 & .0700 & - - - & .4689 \\
    \hline
    
    I would feel adequate & 0.9176 & 62 &  1.8017 & .0765 & - - - & .4513 \\
    \hline
    
    I would feel certain & - - - & - &  - - - & - - - & - - - & - - - \\
    \hline
    
    I would feel productive & - - - & - &  - - - & - - - & - - - & - - -    \\
    \hline
    \hline
    
    I perceived it as useful &  - - - & - &  - - - & - - - & - - - & - - -   \\
    \hline
    
    I would not be suspicious & - - - & - &  - - - & - - - & - - - & - - -   \\
    \hline
    
    It would not be harmful & - - - & - &  - - - & - - - & - - - & - - -  \\
    \hline
    
    I find the product reliable & 0.9667 & 62 &  2.0170 & \cellcolor{AbiOrangeQuote}.0480 & - - - & .5052 \\
    \hline
    
    I would trust the product & - - - & - &  - - - & - - - & - - - & - - - \\
    \hline

    \rowcolor{LightGray}\multicolumn{7}{c}{\textbf{Application AI Product}}\\
    \hline
    \textbf{Dependent}  & \textbf{Distance b/w} &  &  & & \textbf{Bonferroni} &  \\
    \textbf{variable} & \textbf{Means} &  \textbf{df} &  \textbf{t-val} &   \textbf{p-value}  & \textbf{correction} & \textbf{Cohen's \textit{d}} \\
    \hline
    
    I would feel in control & - - - & - &  - - - & - - - & - - - & - - -  \\
    \hline
    
    I would feel secure & - - - & - &  - - - & - - - & - - - & - - - \\
    \hline
    
    I would feel adequate & - - - & - &  - - - & - - - & - - - & - - - \\
    \hline
    
    I would feel certain & - - - & - &  - - - & - - - & - - - & - - - \\
    \hline
    
    I would feel productive & - - - & - &  - - - & - - - & - - - & - - -    \\
    \hline
    \hline
    
    I perceived it as useful &  - - - & - &  - - - & - - - & - - - & - - -   \\
    \hline
    
    I would not be suspicious & - - - & - &  - - - & - - - & - - - & - - -   \\
    \hline
    
    It would not be harmful & - - - & - &  - - - & - - - & - - - & - - -  \\
    \hline
    
    I find the product reliable & - - - & - &  - - - & - - - & - - - & - - - \\
    \hline
    
    I would trust the product & - - - & - &  - - - & - - - & - - - & - - -

    \end{tabular}

    \caption{Guideline 6's t-test results %(\checkmark if Welch's t-test) 
    for the ``by process'' learning style vs. the ``by tinkering'' learning style participants' average ratings of the independent Violation AI product (top) and Application AI product (bottom), for all 10 dependent variables.
    If dashes (- - -) are present, no statistical test was performed.
    If the number of tests exceeded 5 for each product, Bonferroni correction applied by multiplying p-values by the number of tests performed.
    }
    \label{tab:G6-Learn-Stats-Appendix}
\end{table}

%---------------------------------------------------- End Guideline 6

\clearpage

%Begin Guideline 7----------------------------------------------------

\begin{table}[]
    \centering
    \begin{tabular}{cc|cc|cc|cc|cc}
    \multicolumn{2}{c|}{\includegraphics[width = 0.16\columnwidth]{assets/05-All-BoxPlots/06-G7/Learn/G7-Feel-In-Control-LEARN.png}} &
    \multicolumn{2}{c|}{\includegraphics[width = 0.16\columnwidth]{assets/05-All-BoxPlots/06-G7/Learn/G7-Feel-Secure-LEARN.png}} &
    \multicolumn{2}{c|}{\includegraphics[width = 0.16\columnwidth]{assets/05-All-BoxPlots/06-G7/Learn/G7-Feel-Adequate-LEARN.png}} &
    \multicolumn{2}{c|}{\includegraphics[width = 0.16\columnwidth]{assets/05-All-BoxPlots/06-G7/Learn/G7-Feel-Certain-LEARN.png}} &
    \multicolumn{2}{c}{\includegraphics[width = 0.16\columnwidth]{assets/05-All-BoxPlots/06-G7/Learn/G7-Feel-Productive-LEARN.png}}
    \\
    \hline
    \hline
    \multicolumn{2}{c|}{\includegraphics[width = 0.16\columnwidth]{assets/05-All-BoxPlots/06-G7/Learn/G7-Perceived-Useful-LEARN.png}} &
    \multicolumn{2}{c|}{\includegraphics[width = 0.16\columnwidth]{assets/05-All-BoxPlots/06-G7/Learn/G7-Not-Suspicious-LEARN.png}} &
    \multicolumn{2}{c|}{\includegraphics[width = 0.16\columnwidth]{assets/05-All-BoxPlots/06-G7/Learn/G7-Not-Harmful-LEARN.png}} &
    \multicolumn{2}{c|}{\includegraphics[width = 0.16\columnwidth]{assets/05-All-BoxPlots/06-G7/Learn/G7-Product-Reliable-LEARN.png}} &
    \multicolumn{2}{c}{\includegraphics[width = 0.16\columnwidth]{assets/05-All-BoxPlots/06-G7/Learn/G7-Trust-Product-LEARN.png}}
    \end{tabular}
    
    \caption{Guideline 7 participants' ratings for all dependent variables, disaggregated by participants' learning styles: by process vs. by tinkering.
	%For the disaggregated data, notice how large the distances between the average rating are when the guideline is applied.
	Table~\ref{tab:G7-Learn-Stats-Appendix} below provides the statistics (where applicable).
}
    \label{fig:Learn-G7-Appendix}
\end{table}

\begin{table}[h]

%\framebox[\linewidth]{For Measuring!}
\centering
\footnotesize

    \begin{tabular}{p{0.22\columnwidth}|c|c|c|c|c|c}
    
    \rowcolor{LightGray}\multicolumn{7}{c}{\textbf{Violation AI Product}}\\
    \hline
    \textbf{Dependent}  & \textbf{Distance b/w} &  &  & & \textbf{Bonferroni} &  \\
    \textbf{variable} & \textbf{Means} &  \textbf{df} &  \textbf{t-val} &   \textbf{p-value}  & \textbf{correction} & \textbf{Cohen's \textit{d}} \\
    \hline
    
    I would feel in control & - - - & - &  - - - & - - - & - - - & - - - \\
    \hline
    
    I would feel secure & - - - & - &  - - - & - - - & - - - & - - - \\
    \hline
    
    I would feel adequate & - - - & - &  - - - & - - - & - - - & - - - \\
    \hline
    
    I would feel certain & - - - & - &  - - - & - - - & - - - & - - - \\
    \hline
    
    I would feel productive & - - - & - &  - - - & - - - & - - - & - - -  \\
    \hline
    \hline
    
    I perceived it as useful &  - - - & - &  - - - & - - - & - - - & - - -  \\
    \hline
    
    I would not be suspicious & - - - & - &  - - - & - - - & - - - & - - -  \\
    \hline
    
    It would not be harmful & - - - & - &  - - - & - - - & - - - & - - -  \\
    \hline
    
    I find the product reliable & - - - & - &  - - - & - - - & - - - & - - -  \\
    \hline
    
    I would trust the product & 0.5881 & 56 &  1.7277 & .0896 & - - - & .4540 \\
    \hline

    \rowcolor{LightGray}\multicolumn{7}{c}{\textbf{Application AI Product}}\\
    \hline
    \textbf{Dependent}  & \textbf{Distance b/w} &  &  & & \textbf{Bonferroni} &  \\
    \textbf{variable} & \textbf{Means} &  \textbf{df} &  \textbf{t-val} &   \textbf{p-value}  & \textbf{correction} & \textbf{Cohen's \textit{d}} \\
    \hline
    
    I would feel in control & - - - & - &  - - - & - - - & - - - & - - -  \\
    \hline
    
    I would feel secure & - - - & - &  - - - & - - - & - - - & - - - \\
    \hline
    
    I would feel adequate & - - -  & - &  - - - & - - - & - - - & - - - \\
    \hline
    
    I would feel certain & - - - & - &  - - - & - - - & - - - & - - - \\
    \hline
    
    I would feel productive & - - - & - &  - - - & - - - & - - - & - - -    \\
    \hline
    \hline
    
    I perceived it as useful &  - - - & - &  - - - & - - - & - - - & - - -   \\
    \hline
    
    I would not be suspicious & - - - & - &  - - - & - - - & - - - & - - -   \\
    \hline
    
    It would not be harmful & - - - & - &  - - - & - - - & - - - & - - -  \\
    \hline
    
    I find the product reliable & - - - & - &  - - - & - - - & - - - & - - - \\
    \hline
    
    I would trust the product & - - - & - &  - - - & - - - & - - - & - - -

    \end{tabular}

    \caption{Guideline 7's t-test results %(\checkmark if Welch's t-test) 
    for the ``by process'' learning style vs. the ``by tinkering'' learning style participants' average ratings of the independent Violation AI product (top) and Application AI product (bottom), for all 10 dependent variables.
    If dashes (- - -) are present, no statistical test was performed.
    If the number of tests exceeded 5 for each product, Bonferroni correction applied by multiplying p-values by the number of tests performed.
    }
    \label{tab:G7-Learn-Stats-Appendix}
\end{table}

%---------------------------------------------------- End Guideline 7

\clearpage

%Begin Guideline 8----------------------------------------------------

\begin{table}[]
    \centering
    \begin{tabular}{cc|cc|cc|cc|cc}
    \multicolumn{2}{c|}{\includegraphics[width = 0.16\columnwidth]{assets/05-All-BoxPlots/07-G8/Learn/G8-Feel-In-Control-LEARN.png}} &
    \multicolumn{2}{c|}{\includegraphics[width = 0.16\columnwidth]{assets/05-All-BoxPlots/07-G8/Learn/G8-Feel-Secure-LEARN.png}} &
    \multicolumn{2}{c|}{\includegraphics[width = 0.16\columnwidth]{assets/05-All-BoxPlots/07-G8/Learn/G8-Feel-Adequate-LEARN.png}} &
    \multicolumn{2}{c|}{\includegraphics[width = 0.16\columnwidth]{assets/05-All-BoxPlots/07-G8/Learn/G8-Feel-Certain-LEARN.png}} &
    \multicolumn{2}{c}{\includegraphics[width = 0.16\columnwidth]{assets/05-All-BoxPlots/07-G8/Learn/G8-Feel-Productive-LEARN.png}}
    \\
    \hline
    \hline
    \multicolumn{2}{c|}{\includegraphics[width = 0.16\columnwidth]{assets/05-All-BoxPlots/07-G8/Learn/G8-Perceived-Useful-LEARN.png}} &
    \multicolumn{2}{c|}{\includegraphics[width = 0.16\columnwidth]{assets/05-All-BoxPlots/07-G8/Learn/G8-Not-Suspicious-LEARN.png}} &
    \multicolumn{2}{c|}{\includegraphics[width = 0.16\columnwidth]{assets/05-All-BoxPlots/07-G8/Learn/G8-Not-Harmful-LEARN.png}} &
    \multicolumn{2}{c|}{\includegraphics[width = 0.16\columnwidth]{assets/05-All-BoxPlots/07-G8/Learn/G8-Product-Reliable-LEARN.png}} &
    \multicolumn{2}{c}{\includegraphics[width = 0.16\columnwidth]{assets/05-All-BoxPlots/07-G8/Learn/G8-Trust-Product-LEARN.png}}
    \end{tabular}
    
    \caption{Guideline 8 participants' ratings for all dependent variables, disaggregated by participants' learning styles: by process vs. by tinkering.
	%For the disaggregated data, notice how large the distances between the average rating are when the guideline is applied.
	Table~\ref{tab:G8-Learn-Stats-Appendix} below provides the statistics (where applicable).
}
    \label{fig:Learn-G8-Appendix}
\end{table}

\begin{table}[h]

%\framebox[\linewidth]{For Measuring!}
\centering
\footnotesize

    \begin{tabular}{p{0.22\columnwidth}|c|c|c|c|c|c}
    
    \rowcolor{LightGray}\multicolumn{7}{c}{\textbf{Violation AI Product}}\\
    \hline
    \textbf{Dependent}  & \textbf{Distance b/w} &  &  & & \textbf{Bonferroni} &  \\
    \textbf{variable} & \textbf{Means} &  \textbf{df} &  \textbf{t-val} &   \textbf{p-value}  & \textbf{correction} & \textbf{Cohen's \textit{d}} \\
    \hline
    
    I would feel in control & - - - & - &  - - - & - - - & - - - & - - - \\
    \hline
    
    I would feel secure & - - - & - &  - - - & - - - & - - - & - - - \\
    \hline
    
    I would feel adequate & - - - & - &  - - - & - - - & - - - & - - - \\
    \hline
    
    I would feel certain & - - - & - &  - - - & - - - & - - - & - - - \\
    \hline
    
    I would feel productive & - - - & - &  - - - & - - - & - - - & - - -  \\
    \hline
    \hline
    
    I perceived it as useful &  0.7251 & 55 &  1.8991 & .0628 & - - - & .4539  \\
    \hline
    
    I would not be suspicious & - - - & - &  - - - & - - - & - - - & - - - \\
    \hline
    
    It would not be harmful & - - - & - &  - - - & - - - & - - - & - - -  \\
    \hline
    
    I find the product reliable & - - - & - &  - - - & - - - & - - - & - - -  \\
    \hline
    
    I would trust the product & - - - & - &  - - - & - - - & - - - & - - - \\
    \hline

    \rowcolor{LightGray}\multicolumn{7}{c}{\textbf{Application AI Product}}\\
    \hline
    \textbf{Dependent}  & \textbf{Distance b/w} &  &  & & \textbf{Bonferroni} &  \\
    \textbf{variable} & \textbf{Means} &  \textbf{df} &  \textbf{t-val} &   \textbf{p-value}  & \textbf{correction} & \textbf{Cohen's \textit{d}} \\
    \hline
    
    I would feel in control & - - -& - &  - - - & - - - & - - - & - - -  \\
    \hline
    
    I would feel secure & - - - & - &  - - - & - - - & - - - & - - - \\
    \hline
    
    I would feel adequate & - - -  & - &  - - - & - - - & - - - & - - - \\
    \hline
    
    I would feel certain & - - - & - &  - - - & - - - & - - - & - - - \\
    \hline
    
    I would feel productive & - - - & - &  - - - & - - - & - - - & - - -    \\
    \hline
    \hline
    
    I perceived it as useful &  - - - & - &  - - - & - - - & - - - & - - -   \\
    \hline
    
    I would not be suspicious & - - - & - &  - - - & - - - & - - - & - - -   \\
    \hline
    
    It would not be harmful & - - - & - &  - - - & - - - & - - - & - - -  \\
    \hline
    
    I find the product reliable & - - - & - &  - - - & - - - & - - - & - - - \\
    \hline
    
    I would trust the product & - - - & - &  - - - & - - - & - - - & - - -

    \end{tabular}

    \caption{Guideline 8's t-test results %(\checkmark if Welch's t-test) 
    for the ``by process'' learning style vs. the ``by tinkering'' learning style participants' average ratings of the independent Violation AI product (top) and Application AI product (bottom), for all 10 dependent variables.
    If dashes (- - -) are present, no statistical test was performed.
    If the number of tests exceeded 5 for each product, Bonferroni correction applied by multiplying p-values by the number of tests performed.
    }
    \label{tab:G8-Learn-Stats-Appendix}
\end{table}
\clearpage
%---------------------------------------------------- End Guideline 8

%Begin Guideline 9----------------------------------------------------

\begin{table}[]
    \centering
    \begin{tabular}{cc|cc|cc|cc|cc}
    \multicolumn{2}{c|}{\includegraphics[width = 0.16\columnwidth]{assets/05-All-BoxPlots/08-G9/Learn/G9-Feel-In-Control-LEARN.png}} &
    \multicolumn{2}{c|}{\includegraphics[width = 0.16\columnwidth]{assets/05-All-BoxPlots/08-G9/Learn/G9-Feel-Secure-LEARN.png}} &
    \multicolumn{2}{c|}{\includegraphics[width = 0.16\columnwidth]{assets/05-All-BoxPlots/08-G9/Learn/G9-Feel-Adequate-LEARN.png}} &
    \multicolumn{2}{c|}{\includegraphics[width = 0.16\columnwidth]{assets/05-All-BoxPlots/08-G9/Learn/G9-Feel-Certain-LEARN.png}} &
    \multicolumn{2}{c}{\includegraphics[width = 0.16\columnwidth]{assets/05-All-BoxPlots/08-G9/Learn/G9-Feel-Productive-LEARN.png}}
    \\
    \hline
    \hline
    \multicolumn{2}{c|}{\includegraphics[width = 0.16\columnwidth]{assets/05-All-BoxPlots/08-G9/Learn/G9-Perceived-Useful-LEARN.png}} &
    \multicolumn{2}{c|}{\includegraphics[width = 0.16\columnwidth]{assets/05-All-BoxPlots/08-G9/Learn/G9-Not-Suspicious-LEARN.png}} &
    \multicolumn{2}{c|}{\includegraphics[width = 0.16\columnwidth]{assets/05-All-BoxPlots/08-G9/Learn/G9-Not-Harmful-LEARN.png}} &
    \multicolumn{2}{c|}{\includegraphics[width = 0.16\columnwidth]{assets/05-All-BoxPlots/08-G9/Learn/G9-Product-Reliable-LEARN.png}} &
    \multicolumn{2}{c}{\includegraphics[width = 0.16\columnwidth]{assets/05-All-BoxPlots/08-G9/Learn/G9-Trust-Product-LEARN.png}}
    \end{tabular}
    
    \caption{Guideline 9 participants' ratings for all dependent variables, disaggregated by participants' learning styles: by process vs. by tinkering.
	%For the disaggregated data, notice how large the distances between the average rating are when the guideline is applied.
	Table~\ref{tab:G9-Learn-Stats-Appendix} below provides the statistics (where applicable).
}
    \label{fig:Learn-G9-Appendix}
\end{table}

\begin{table}[h]

%\framebox[\linewidth]{For Measuring!}
\centering
\footnotesize

    \begin{tabular}{p{0.22\columnwidth}|c|c|c|c|c|c}
    
    \rowcolor{LightGray}\multicolumn{7}{c}{\textbf{Violation AI Product}}\\
    \hline
    \textbf{Dependent}  & \textbf{Distance b/w} &  &  & & \textbf{Bonferroni} &  \\
    \textbf{variable} & \textbf{Means} &  \textbf{df} &  \textbf{t-val} &   \textbf{p-value}  & \textbf{correction} & \textbf{Cohen's \textit{d}} \\
    \hline
    
    I would feel in control & - - - & - &  - - - & - - - & - - - & - - - \\
    \hline
    
    I would feel secure & - - - & - &  - - - & - - - & - - - & - - - \\
    \hline
    
    I would feel adequate & - - - & - &  - - - & - - - & - - - & - - - \\
    \hline
    
    I would feel certain & - - - & - &  - - - & - - - & - - - & - - - \\
    \hline
    
    I would feel productive & - - - & - &  - - - & - - - & - - - & - - -  \\
    \hline
    \hline
    
    I perceived it as useful &  - - - & - &  - - - & - - - & - - - & - - -  \\
    \hline
    
    I would not be suspicious & - - - & - &  - - - & - - - & - - - & - - - \\
    \hline
    
    It would not be harmful & - - - & - &  - - - & - - - & - - - & - - -  \\
    \hline
    
    I find the product reliable & - - - & - &  - - - & - - - & - - - & - - -  \\
    \hline
    
    I would trust the product & - - - & - &  - - - & - - - & - - - & - - - \\
    \hline

    \rowcolor{LightGray}\multicolumn{7}{c}{\textbf{Application AI Product}}\\
    \hline
    \textbf{Dependent}  & \textbf{Distance b/w} &  &  & & \textbf{Bonferroni} &  \\
    \textbf{variable} & \textbf{Means} &  \textbf{df} &  \textbf{t-val} &   \textbf{p-value}  & \textbf{correction} & \textbf{Cohen's \textit{d}} \\
    \hline
    
    I would feel in control & - - - & - &  - - - & - - - & - - - & - - -  \\
    \hline
    
    I would feel secure & - - - & - &  - - - & - - - & - - - & - - - \\
    \hline
    
    I would feel adequate & - - -  & - &  - - - & - - - & - - - & - - - \\
    \hline
    
    I would feel certain & - - - & - &  - - - & - - - & - - - & - - - \\
    \hline
    
    I would feel productive & - - - & - &  - - - & - - - & - - - & - - -    \\
    \hline
    \hline
    
    I perceived it as useful &  - - - & - &  - - - & - - - & - - - & - - -   \\
    \hline
    
    I would not be suspicious & - - - & - &  - - - & - - - & - - - & - - -   \\
    \hline
    
    It would not be harmful & - - - & - &  - - - & - - - & - - - & - - -  \\
    \hline
    
    I find the product reliable & - - - & - &  - - - & - - - & - - - & - - - \\
    \hline
    
    I would trust the product & - - - & - &  - - - & - - - & - - - & - - -

    \end{tabular}

    \caption{Guideline 9's t-test results %(\checkmark if Welch's t-test) 
    for the ``by process'' learning style vs. the ``by tinkering'' learning style participants' average ratings of the independent Violation AI product (top) and Application AI product (bottom), for all 10 dependent variables.
    If dashes (- - -) are present, no statistical test was performed.
    If the number of tests exceeded 5 for each product, Bonferroni correction applied by multiplying p-values by the number of tests performed.
    }
    \label{tab:G9-Learn-Stats-Appendix}
\end{table}
\clearpage
%---------------------------------------------------- End Guideline 9

%Begin Guideline 10----------------------------------------------------

\begin{table}[]
    \centering
    \begin{tabular}{cc|cc|cc|cc|cc}
    \multicolumn{2}{c|}{\includegraphics[width = 0.16\columnwidth]{assets/05-All-BoxPlots/09-G10/Learn/G10-Feel-In-Control-LEARN.png}} &
    \multicolumn{2}{c|}{\includegraphics[width = 0.16\columnwidth]{assets/05-All-BoxPlots/09-G10/Learn/G10-Feel-Secure-LEARN.png}} &
    \multicolumn{2}{c|}{\includegraphics[width = 0.16\columnwidth]{assets/05-All-BoxPlots/09-G10/Learn/G10-Feel-Adequate-LEARN.png}} &
    \multicolumn{2}{c|}{\includegraphics[width = 0.16\columnwidth]{assets/05-All-BoxPlots/09-G10/Learn/G10-Feel-Certain-LEARN.png}} &
    \multicolumn{2}{c}{\includegraphics[width = 0.16\columnwidth]{assets/05-All-BoxPlots/09-G10/Learn/G10-Feel-Productive-LEARN.png}}
    \\
    \hline
    \hline
    \multicolumn{2}{c|}{\includegraphics[width = 0.16\columnwidth]{assets/05-All-BoxPlots/09-G10/Learn/G10-Perceived-Useful-LEARN.png}} &
    \multicolumn{2}{c|}{\includegraphics[width = 0.16\columnwidth]{assets/05-All-BoxPlots/09-G10/Learn/G10-Not-Suspicious-LEARN.png}} &
    \multicolumn{2}{c|}{\includegraphics[width = 0.16\columnwidth]{assets/05-All-BoxPlots/09-G10/Learn/G10-Not-Harmful-LEARN.png}} &
    \multicolumn{2}{c|}{\includegraphics[width = 0.16\columnwidth]{assets/05-All-BoxPlots/09-G10/Learn/G10-Product-Reliable-LEARN.png}} &
    \multicolumn{2}{c}{\includegraphics[width = 0.16\columnwidth]{assets/05-All-BoxPlots/09-G10/Learn/G10-Trust-Product-LEARN.png}}
    \end{tabular}
    
    \caption{Guideline 10 participants' ratings for all dependent variables, disaggregated by participants' learning styles: by process vs. by tinkering.
	%For the disaggregated data, notice how large the distances between the average rating are when the guideline is applied.
	Table~\ref{tab:G10-Learn-Stats-Appendix} below provides the statistics (where applicable).
}
    \label{fig:Learn-G10-Appendix}
\end{table}

\begin{table}[h]

%\framebox[\linewidth]{For Measuring!}
\centering
\footnotesize

    \begin{tabular}{p{0.22\columnwidth}|c|c|c|c|c|c}
    
    \rowcolor{LightGray}\multicolumn{7}{c}{\textbf{Violation AI Product}}\\
    \hline
    \textbf{Dependent}  & \textbf{Distance b/w} &  &  & & \textbf{Bonferroni} &  \\
    \textbf{variable} & \textbf{Means} &  \textbf{df} &  \textbf{t-val} &   \textbf{p-value}  & \textbf{correction} & \textbf{Cohen's \textit{d}} \\
    \hline
    
    I would feel in control & - - - & - &  - - - & - - - & - - - & - - - \\
    \hline
    
    I would feel secure & - - - & - &  - - - & - - - & - - - & - - - \\
    \hline
    
    I would feel adequate & - - - & - &  - - - & - - - & - - - & - - - \\
    \hline
    
    I would feel certain & - - - & - &  - - - & - - - & - - - & - - - \\
    \hline
    
    I would feel productive & - - - & - &  - - - & - - - & - - - & - - -  \\
    \hline
    \hline
    
    I perceived it as useful &  - - - & - &  - - - & - - - & - - - & - - -  \\
    \hline
    
    I would not be suspicious & 0.9886 & 63 &  2.0187 & \cellcolor{AbiOrangeQuote}.0478 & - - - & .5013 \\
    \hline
    
    It would not be harmful & - - - & - &  - - - & - - - & - - - & - - -  \\
    \hline
    
    I find the product reliable & - - - & - &  - - - & - - - & - - - & - - -  \\
    \hline
    
    I would trust the product & - - - & - &  - - - & - - - & - - - & - - - \\
    \hline

    \rowcolor{LightGray}\multicolumn{7}{c}{\textbf{Application AI Product}}\\
    \hline
    \textbf{Dependent}  & \textbf{Distance b/w} &  &  & & \textbf{Bonferroni} &  \\
    \textbf{variable} & \textbf{Means} &  \textbf{df} &  \textbf{t-val} &   \textbf{p-value}  & \textbf{correction} & \textbf{Cohen's \textit{d}} \\
    \hline
    
    I would feel in control & - - - & - &  - - - & - - - & - - - & - - -  \\
    \hline
    
    I would feel secure & - - - & - &  - - - & - - - & - - - & - - - \\
    \hline
    
    I would feel adequate & - - -  & - &  - - - & - - - & - - - & - - - \\
    \hline
    
    I would feel certain & - - - & - &  - - - & - - - & - - - & - - - \\
    \hline
    
    I would feel productive & - - - & - &  - - - & - - - & - - - & - - -   \\
    \hline
    \hline
    
    I perceived it as useful &  - - - & - &  - - - & - - - & - - - & - - -   \\
    \hline
    
    I would not be suspicious & - - - & - &  - - - & - - - & - - - & - - -   \\
    \hline
    
    It would not be harmful & - - - & - &  - - - & - - - & - - - & - - -  \\
    \hline
    
    I find the product reliable & - - - & - &  - - - & - - - & - - - & - - - \\
    \hline
    
    I would trust the product & - - - & - &  - - - & - - - & - - - & - - -

    \end{tabular}

    \caption{Guideline 10's t-test results %(\checkmark if Welch's t-test) 
    for the ``by process'' learning style vs. the ``by tinkering'' learning style participants' average ratings of the independent Violation AI product (top) and Application AI product (bottom), for all 10 dependent variables.
    If dashes (- - -) are present, no statistical test was performed.
    If the number of tests exceeded 5 for each product, Bonferroni correction applied by multiplying p-values by the number of tests performed.
    }
    \label{tab:G10-Learn-Stats-Appendix}
\end{table}
\clearpage
%---------------------------------------------------- End Guideline 10

%Begin Guideline 11----------------------------------------------------

\begin{table}[]
    \centering
    \begin{tabular}{cc|cc|cc|cc|cc}
    \multicolumn{2}{c|}{\includegraphics[width = 0.16\columnwidth]{assets/05-All-BoxPlots/10-G11/Learn/G11-Feel-In-Control-LEARN.png}} &
    \multicolumn{2}{c|}{\includegraphics[width = 0.16\columnwidth]{assets/05-All-BoxPlots/10-G11/Learn/G11-Feel-Secure-LEARN.png}} &
    \multicolumn{2}{c|}{\includegraphics[width = 0.16\columnwidth]{assets/05-All-BoxPlots/10-G11/Learn/G11-Feel-Adequate-LEARN.png}} &
    \multicolumn{2}{c|}{\includegraphics[width = 0.16\columnwidth]{assets/05-All-BoxPlots/10-G11/Learn/G11-Feel-Certain-LEARN.png}} &
    \multicolumn{2}{c}{\includegraphics[width = 0.16\columnwidth]{assets/05-All-BoxPlots/10-G11/Learn/G11-Feel-Productive-LEARN.png}}
    \\
    \hline
    \hline
    \multicolumn{2}{c|}{\includegraphics[width = 0.16\columnwidth]{assets/05-All-BoxPlots/10-G11/Learn/G11-Perceived-Useful-LEARN.png}} &
    \multicolumn{2}{c|}{\includegraphics[width = 0.16\columnwidth]{assets/05-All-BoxPlots/10-G11/Learn/G11-Not-Suspicious-LEARN.png}} &
    \multicolumn{2}{c|}{\includegraphics[width = 0.16\columnwidth]{assets/05-All-BoxPlots/10-G11/Learn/G11-Not-Harmful-LEARN.png}} &
    \multicolumn{2}{c|}{\includegraphics[width = 0.16\columnwidth]{assets/05-All-BoxPlots/10-G11/Learn/G11-Product-Reliable-LEARN.png}} &
    \multicolumn{2}{c}{\includegraphics[width = 0.16\columnwidth]{assets/05-All-BoxPlots/10-G11/Learn/G11-Trust-Product-LEARN.png}}
    \end{tabular}
    
    \caption{Guideline 11 participants' ratings for all dependent variables, disaggregated by participants' learning styles: by process vs. by tinkering.
	%For the disaggregated data, notice how large the distances between the average rating are when the guideline is applied.
	Table~\ref{tab:G11-Learn-Stats-Appendix} below provides the statistics (where applicable).
}
    \label{fig:Learn-G11-Appendix}
\end{table}

\begin{table}[h]

%\framebox[\linewidth]{For Measuring!}
\centering
\footnotesize

    \begin{tabular}{p{0.22\columnwidth}|c|c|c|c|c|c}
    
    \rowcolor{LightGray}\multicolumn{7}{c}{\textbf{Violation AI Product}}\\
    \hline
    \textbf{Dependent}  & \textbf{Distance b/w} &  &  & & \textbf{Bonferroni} &  \\
    \textbf{variable} & \textbf{Means} &  \textbf{df} &  \textbf{t-val} &   \textbf{p-value}  & \textbf{correction} & \textbf{Cohen's \textit{d}} \\
    \hline
    
    I would feel in control & - - - & - &  - - - & - - - & - - - & - - - \\
    \hline
    
    I would feel secure & - - - & - &  - - - & - - - & - - - & - - - \\
    \hline
    
    I would feel adequate & - - - & - &  - - - & - - - & - - - & - - - \\
    \hline
    
    I would feel certain & 0.5741 & 61 &  1.4804 & .1439 & - - - & .3769 \\
    \hline
    
    I would feel productive & - - - & - &  - - - & - - - & - - - & - - -  \\
    \hline
    \hline
    
    I perceived it as useful &  - - - & - &  - - - & - - - & - - - & - - -  \\
    \hline
    
    I would not be suspicious & - - - & - &  - - - & - - - & - - - & - - - \\
    \hline
    
    It would not be harmful & - - - & - &  - - - & - - - & - - - & - - -  \\
    \hline
    
    I find the product reliable & - - - & - &  - - - & - - - & - - - & - - -  \\
    \hline
    
    I would trust the product & - - - & - &  - - - & - - - & - - - & - - - \\
    \hline

    \rowcolor{LightGray}\multicolumn{7}{c}{\textbf{Application AI Product}}\\
    \hline
    \textbf{Dependent}  & \textbf{Distance b/w} &  &  & & \textbf{Bonferroni} &  \\
    \textbf{variable} & \textbf{Means} &  \textbf{df} &  \textbf{t-val} &   \textbf{p-value}  & \textbf{correction} & \textbf{Cohen's \textit{d}} \\
    \hline
    
    I would feel in control & - - - & - &  - - - & - - - & - - - & - - - \\
    \hline
    
    I would feel secure & - - - & - &  - - - & - - - & - - - & - - - \\
    \hline
    
    I would feel adequate & - - - & - &  - - - & - - - & - - - & - - - \\
    \hline
    
    I would feel certain & 0.9907 & 61 &  2.3331 & \cellcolor{AbiOrangeQuote}.0230 & - - - & .4246 \\
    \hline
    
    I would feel productive & - - - & - &  - - - & - - - & - - - & - - -   \\
    \hline
    \hline
    
    I perceived it as useful &  - - - & - &  - - - & - - - & - - - & - - -   \\
    \hline
    
    I would not be suspicious & - - - & - &  - - - & - - - & - - - & - - -   \\
    \hline
    
    It would not be harmful & - - - & - &  - - - & - - - & - - - & - - -  \\
    \hline
    
    I find the product reliable & - - - & - &  - - - & - - - & - - - & - - - \\
    \hline
    
    I would trust the product & - - - & - &  - - - & - - - & - - - & - - -

    \end{tabular}

    \caption{Guideline 11's t-test results %(\checkmark if Welch's t-test) 
    for the ``by process'' learning style vs. the ``by tinkering'' learning style participants' average ratings of the independent Violation AI product (top) and Application AI product (bottom), for all 10 dependent variables.
    If dashes (- - -) are present, no statistical test was performed.
    If the number of tests exceeded 5 for each product, Bonferroni correction applied by multiplying p-values by the number of tests performed.
    }
    \label{tab:G11-Learn-Stats-Appendix}
\end{table}
\clearpage
%---------------------------------------------------- End Guideline 11

%Begin Guideline 12----------------------------------------------------

\begin{table}[]
    \centering
    \begin{tabular}{cc|cc|cc|cc|cc}
    \multicolumn{2}{c|}{\includegraphics[width = 0.16\columnwidth]{assets/05-All-BoxPlots/11-G12/Learn/G12-Feel-In-Control-LEARN.png}} &
    \multicolumn{2}{c|}{\includegraphics[width = 0.16\columnwidth]{assets/05-All-BoxPlots/11-G12/Learn/G12-Feel-Secure-LEARN.png}} &
    \multicolumn{2}{c|}{\includegraphics[width = 0.16\columnwidth]{assets/05-All-BoxPlots/11-G12/Learn/G12-Feel-Adequate-LEARN.png}} &
    \multicolumn{2}{c|}{\includegraphics[width = 0.16\columnwidth]{assets/05-All-BoxPlots/11-G12/Learn/G12-Feel-Certain-LEARN.png}} &
    \multicolumn{2}{c}{\includegraphics[width = 0.16\columnwidth]{assets/05-All-BoxPlots/11-G12/Learn/G12-Feel-Productive-LEARN.png}}
    \\
    \hline
    \hline
    \multicolumn{2}{c|}{\includegraphics[width = 0.16\columnwidth]{assets/05-All-BoxPlots/11-G12/Learn/G12-Perceived-Useful-LEARN.png}} &
    \multicolumn{2}{c|}{\includegraphics[width = 0.16\columnwidth]{assets/05-All-BoxPlots/11-G12/Learn/G12-Not-Suspicious-LEARN.png}} &
    \multicolumn{2}{c|}{\includegraphics[width = 0.16\columnwidth]{assets/05-All-BoxPlots/11-G12/Learn/G12-Not-Harmful-LEARN.png}} &
    \multicolumn{2}{c|}{\includegraphics[width = 0.16\columnwidth]{assets/05-All-BoxPlots/11-G12/Learn/G12-Product-Reliable-LEARN.png}} &
    \multicolumn{2}{c}{\includegraphics[width = 0.16\columnwidth]{assets/05-All-BoxPlots/11-G12/Learn/G12-Trust-Product-LEARN.png}}
    \end{tabular}
    
    \caption{Guideline 12 participants' ratings for all dependent variables, disaggregated by participants' learning styles: by process vs. by tinkering.
	%For the disaggregated data, notice how large the distances between the average rating are when the guideline is applied.
	Table~\ref{tab:G12-Learn-Stats-Appendix} below provides the statistics (where applicable).
}
    \label{fig:Learn-G12-Appendix}
\end{table}

\begin{table}[h]

%\framebox[\linewidth]{For Measuring!}
\centering
\footnotesize

    \begin{tabular}{p{0.22\columnwidth}|c|c|c|c|c|c}
    
    \rowcolor{LightGray}\multicolumn{7}{c}{\textbf{Violation AI Product}}\\
    \hline
    \textbf{Dependent}  & \textbf{Distance b/w} &  &  & & \textbf{Bonferroni} &  \\
    \textbf{variable} & \textbf{Means} &  \textbf{df} &  \textbf{t-val} &   \textbf{p-value}  & \textbf{correction} & \textbf{Cohen's \textit{d}} \\
    \hline
    
    I would feel in control & - - - & - &  - - - & - - - & - - - & - - -  \\
    \hline
    
    I would feel secure & - - - & - &  - - - & - - - & - - - & - - - \\
    \hline
    
    I would feel adequate & - - -  & - &  - - - & - - - & - - - & - - - \\
    \hline
    
    I would feel certain & - - - & - &  - - - & - - - & - - - & - - - \\
    \hline
    
    I would feel productive & - - - & - &  - - - & - - - & - - - & - - -   \\
    \hline
    \hline
    
    I perceived it as useful &  - - - & - &  - - - & - - - & - - - & - - -   \\
    \hline
    
    I would not be suspicious & - - - & - &  - - - & - - - & - - - & - - -   \\
    \hline
    
    It would not be harmful & - - - & - &  - - - & - - - & - - - & - - -  \\
    \hline
    
    I find the product reliable & - - - & - &  - - - & - - - & - - - & - - - \\
    \hline
    
    I would trust the product & - - - & - &  - - - & - - - & - - - & - - - \\
    \hline

    \rowcolor{LightGray}\multicolumn{7}{c}{\textbf{Application AI Product}}\\
    \hline
    \textbf{Dependent}  & \textbf{Distance b/w} &  &  & & \textbf{Bonferroni} &  \\
    \textbf{variable} & \textbf{Means} &  \textbf{df} &  \textbf{t-val} &   \textbf{p-value}  & \textbf{correction} & \textbf{Cohen's \textit{d}} \\
    \hline
    
    I would feel in control & - - - & - &  - - - & - - - & - - - & - - -  \\
    \hline
    
    I would feel secure & - - - & - &  - - - & - - - & - - - & - - - \\
    \hline
    
    I would feel adequate & - - -  & - &  - - - & - - - & - - - & - - - \\
    \hline
    
    I would feel certain & - - - & - &  - - - & - - - & - - - & - - - \\
    \hline
    
    I would feel productive & - - - & - &  - - - & - - - & - - - & - - -   \\
    \hline
    \hline
    
    I perceived it as useful &  - - - & - &  - - - & - - - & - - - & - - -   \\
    \hline
    
    I would not be suspicious & - - - & - &  - - - & - - - & - - - & - - -   \\
    \hline
    
    It would not be harmful & - - - & - &  - - - & - - - & - - - & - - -  \\
    \hline
    
    I find the product reliable & - - - & - &  - - - & - - - & - - - & - - - \\
    \hline
    
    I would trust the product & - - - & - &  - - - & - - - & - - - & - - -

    \end{tabular}

    \caption{Guideline 12's t-test results %(\checkmark if Welch's t-test) 
    for the ``by process'' learning style vs. the ``by tinkering'' learning style participants' average ratings of the independent Violation AI product (top) and Application AI product (bottom), for all 10 dependent variables.
    If dashes (- - -) are present, no statistical test was performed.
    If the number of tests exceeded 5 for each product, Bonferroni correction applied by multiplying p-values by the number of tests performed.
    }
    \label{tab:G12-Learn-Stats-Appendix}
\end{table}
\clearpage
%---------------------------------------------------- End Guideline 12

%Begin Guideline 13----------------------------------------------------

\begin{table}[]
    \centering
    \begin{tabular}{cc|cc|cc|cc|cc}
    \multicolumn{2}{c|}{\includegraphics[width = 0.16\columnwidth]{assets/05-All-BoxPlots/12-G13/Learn/G13-Feel-In-Control-LEARN.png}} &
    \multicolumn{2}{c|}{\includegraphics[width = 0.16\columnwidth]{assets/05-All-BoxPlots/12-G13/Learn/G13-Feel-Secure-LEARN.png}} &
    \multicolumn{2}{c|}{\includegraphics[width = 0.16\columnwidth]{assets/05-All-BoxPlots/12-G13/Learn/G13-Feel-Adequate-LEARN.png}} &
    \multicolumn{2}{c|}{\includegraphics[width = 0.16\columnwidth]{assets/05-All-BoxPlots/12-G13/Learn/G13-Feel-Certain-LEARN.png}} &
    \multicolumn{2}{c}{\includegraphics[width = 0.16\columnwidth]{assets/05-All-BoxPlots/12-G13/Learn/G13-Feel-Productive-LEARN.png}}
    \\
    \hline
    \hline
    \multicolumn{2}{c|}{\includegraphics[width = 0.16\columnwidth]{assets/05-All-BoxPlots/12-G13/Learn/G13-Perceived-Useful-LEARN.png}} &
    \multicolumn{2}{c|}{\includegraphics[width = 0.16\columnwidth]{assets/05-All-BoxPlots/12-G13/Learn/G13-Not-Suspicious-LEARN.png}} &
    \multicolumn{2}{c|}{\includegraphics[width = 0.16\columnwidth]{assets/05-All-BoxPlots/12-G13/Learn/G13-Not-Harmful-LEARN.png}} &
    \multicolumn{2}{c|}{\includegraphics[width = 0.16\columnwidth]{assets/05-All-BoxPlots/12-G13/Learn/G13-Product-Reliable-LEARN.png}} &
    \multicolumn{2}{c}{\includegraphics[width = 0.16\columnwidth]{assets/05-All-BoxPlots/12-G13/Learn/G13-Trust-Product-LEARN.png}}
    \end{tabular}
    
    \caption{Guideline 13 participants' ratings for all dependent variables, disaggregated by participants' learning styles: by process vs. by tinkering.
	%For the disaggregated data, notice how large the distances between the average rating are when the guideline is applied.
	Table~\ref{tab:G13-Learn-Stats-Appendix} below provides the statistics (where applicable).
}
    \label{fig:Learn-G13-Appendix}
\end{table}

\begin{table}[h]

%\framebox[\linewidth]{For Measuring!}
\centering
\footnotesize

    \begin{tabular}{p{0.22\columnwidth}|c|c|c|c|c|c}
    
    \rowcolor{LightGray}\multicolumn{7}{c}{\textbf{Violation AI Product}}\\
    \hline
    \textbf{Dependent}  & \textbf{Distance b/w} &  &  & & \textbf{Bonferroni} &  \\
    \textbf{variable} & \textbf{Means} &  \textbf{df} &  \textbf{t-val} &   \textbf{p-value}  & \textbf{correction} & \textbf{Cohen's \textit{d}} \\
    \hline
    
    I would feel in control & 1.1268 & 55 &  3.2314 & \cellcolor{AbiOrangeQuote}.0021 & - - - & .8561  \\
    \hline
    
    I would feel secure & 0.8202 & 55 &  2.3229 & \cellcolor{AbiOrangeQuote}.0239 & - - - & .6155 \\
    \hline
    
    I would feel adequate & 0.9791  & 55 &  2.3185 & \cellcolor{AbiOrangeQuote}.0242 & - - -& .6143 \\
    \hline
    
    I would feel certain & 0.8633 & 55 &  2.0343 & \cellcolor{AbiOrangeQuote}.0468 & - - - & .5390 \\
    \hline
    
    I would feel productive & - - - & - &  - - - & - - - & - - - & - - -   \\
    \hline
    \hline
    
    I perceived it as useful &  - - - & - &  - - - & - - - & - - - & - - -   \\
    \hline
    
    I would not be suspicious & 0.9286 & 54 &  2.0758 & \cellcolor{AbiOrangeQuote}.0427 & - - - & .5548   \\
    \hline
    
    It would not be harmful & - - - & - &  - - - & - - - & - - - & - - -  \\
    \hline
    
    I find the product reliable & - - - & - &  - - - & - - - & - - - & - - - \\
    \hline
    
    I would trust the product & - - - & - &  - - - & - - - & - - - & - - - \\
    \hline

    \rowcolor{LightGray}\multicolumn{7}{c}{\textbf{Application AI Product}}\\
    \hline
    \textbf{Dependent}  & \textbf{Distance b/w} &  &  & & \textbf{Bonferroni} &  \\
    \textbf{variable} & \textbf{Means} &  \textbf{df} &  \textbf{t-val} &   \textbf{p-value}  & \textbf{correction} & \textbf{Cohen's \textit{d}} \\
    \hline
    
    I would feel in control & - - - & - &  - - - & - - - & - - - & - - -  \\
    \hline
    
    I would feel secure & - - - & - &  - - - & - - - & - - - & - - - \\
    \hline
    
    I would feel adequate & - - - & - &  - - - & - - - & - - - & - - - \\
    \hline
    
    I would feel certain & - - - & - &  - - - & - - - & - - - & - - - \\
    \hline
    
    I would feel productive & - - - & - &  - - - & - - - & - - - & - - -   \\
    \hline
    \hline
    
    I perceived it as useful &  - - - & - &  - - - & - - - & - - - & - - -   \\
    \hline
    
    I would not be suspicious & - - - & - &  - - - & - - - & - - - & - - -   \\
    \hline
    
    It would not be harmful & 0.7020 & 55 &  2.1068 & \cellcolor{AbiOrangeQuote}.0397 & - - - & .5582  \\
    \hline
    
    I find the product reliable & - - - & - &  - - - & - - - & - - - & - - - \\
    \hline
    
    I would trust the product & - - - & - &  - - - & - - - & - - - & - - -

    \end{tabular}

    \caption{Guideline 13's t-test results %(\checkmark if Welch's t-test) 
    for the ``by process'' learning style vs. the ``by tinkering'' learning style participants' average ratings of the independent Violation AI product (top) and Application AI product (bottom), for all 10 dependent variables.
    If dashes (- - -) are present, no statistical test was performed.
    If the number of tests exceeded 5 for each product, Bonferroni correction applied by multiplying p-values by the number of tests performed.
    }
    \label{tab:G13-Learn-Stats-Appendix}
\end{table}
\clearpage
%---------------------------------------------------- End Guideline 13

%Begin Guideline 14---------------------------------------------------

\begin{table}[]
    \centering
    \begin{tabular}{cc|cc|cc|cc|cc}
    \multicolumn{2}{c|}{\includegraphics[width = 0.16\columnwidth]{assets/05-All-BoxPlots/13-G14/Learn/G14-Feel-In-Control-LEARN.png}} &
    \multicolumn{2}{c|}{\includegraphics[width = 0.16\columnwidth]{assets/05-All-BoxPlots/13-G14/Learn/G14-Feel-Secure-LEARN.png}} &
    \multicolumn{2}{c|}{\includegraphics[width = 0.16\columnwidth]{assets/05-All-BoxPlots/13-G14/Learn/G14-Feel-Adequate-LEARN.png}} &
    \multicolumn{2}{c|}{\includegraphics[width = 0.16\columnwidth]{assets/05-All-BoxPlots/13-G14/Learn/G14-Feel-Certain-LEARN.png}} &
    \multicolumn{2}{c}{\includegraphics[width = 0.16\columnwidth]{assets/05-All-BoxPlots/13-G14/Learn/G14-Feel-Productive-LEARN.png}}
    \\
    \hline
    \hline
    \multicolumn{2}{c|}{\includegraphics[width = 0.16\columnwidth]{assets/05-All-BoxPlots/13-G14/Learn/G14-Perceived-Useful-LEARN.png}} &
    \multicolumn{2}{c|}{\includegraphics[width = 0.16\columnwidth]{assets/05-All-BoxPlots/13-G14/Learn/G14-Not-Suspicious-LEARN.png}} &
    \multicolumn{2}{c|}{\includegraphics[width = 0.16\columnwidth]{assets/05-All-BoxPlots/13-G14/Learn/G14-Not-Harmful-LEARN.png}} &
    \multicolumn{2}{c|}{\includegraphics[width = 0.16\columnwidth]{assets/05-All-BoxPlots/13-G14/Learn/G14-Product-Reliable-LEARN.png}} &
    \multicolumn{2}{c}{\includegraphics[width = 0.16\columnwidth]{assets/05-All-BoxPlots/13-G14/Learn/G14-Trust-Product-LEARN.png}}
    \end{tabular}
    
    \caption{Guideline 14 participants' ratings for all dependent variables, disaggregated by participants' learning styles: by process vs. by tinkering.
	%For the disaggregated data, notice how large the distances between the average rating are when the guideline is applied.
	Table~\ref{tab:G14-Learn-Stats-Appendix} below provides the statistics (where applicable).
}
    \label{fig:Learn-G14-Appendix}
\end{table}

\begin{table}[h]

%\framebox[\linewidth]{For Measuring!}
\centering
\footnotesize

    \begin{tabular}{p{0.22\columnwidth}|c|c|c|c|c|c}
    
    \rowcolor{LightGray}\multicolumn{7}{c}{\textbf{Violation AI Product}}\\
    \hline
    \textbf{Dependent}  & \textbf{Distance b/w} &  &  & & \textbf{Bonferroni} &  \\
    \textbf{variable} & \textbf{Means} &  \textbf{df} &  \textbf{t-val} &   \textbf{p-value}  & \textbf{correction} & \textbf{Cohen's \textit{d}} \\
    \hline
    
    I would feel in control & - - - & - &  - - - & - - - & - - - & - - -  \\
    \hline
    
    I would feel secure & - - - & - &  - - - & - - - & - - - & - - - \\
    \hline
    
    I would feel adequate & - - - & - &  - - - & - - - & - - - & - - - \\
    \hline
    
    I would feel certain & - - - & - &  - - - & - - - & - - - & - - - \\
    \hline
    
    I would feel productive & - - - & - &  - - - & - - - & - - - & - - -   \\
    \hline
    \hline
    
    I perceived it as useful &  - - - & - &  - - - & - - - & - - - & - - -   \\
    \hline
    
    I would not be suspicious & 1.1141 & 65 &  2.6552 & \cellcolor{AbiOrangeQuote}.0100 & - - - & .6488   \\
    \hline
    
    It would not be harmful & - - - & - &  - - - & - - - & - - - & - - -  \\
    \hline
    
    I find the product reliable & - - - & - &  - - - & - - - & - - - & - - - \\
    \hline
    
    I would trust the product & - - - & - &  - - - & - - - & - - - & - - - \\
    \hline

    \rowcolor{LightGray}\multicolumn{7}{c}{\textbf{Application AI Product}}\\
    \hline
    \textbf{Dependent}  & \textbf{Distance b/w} &  &  & & \textbf{Bonferroni} &  \\
    \textbf{variable} & \textbf{Means} &  \textbf{df} &  \textbf{t-val} &   \textbf{p-value}  & \textbf{correction} & \textbf{Cohen's \textit{d}} \\
    \hline
    
    I would feel in control & 0.7059 & 66 &  2.0756 & \cellcolor{AbiOrangeQuote}.0418 & .2508 & .5034  \\
    \hline
    
    I would feel secure & 1.0927 & 65 &  3.6028 & \cellcolor{AbiOrangeQuote}.0006 & \cellcolor{AbiOrangeQuote}.0036 & .8804 \\
    \hline
    
    I would feel adequate & 0.8824  & 65 &  2.9784 & \cellcolor{AbiOrangeQuote}.0041 & \cellcolor{AbiOrangeQuote}.0246  & .7278 \\
    \hline
    
    I would feel certain & 0.7353 & 66 &  2.2296 & \cellcolor{AbiOrangeQuote}.0292 & .1752 & .5408 \\
    \hline
    
    I would feel productive & - - - & - &  - - - & - - - & - - - & - - -   \\
    \hline
    \hline
    
    I perceived it as useful &  .5956 & 64 &  2.3127 & \cellcolor{AbiOrangeQuote}.0240 & .144 & .5696   \\
    \hline
    
    I would not be suspicious & - - - & - &  - - - & - - - & - - - & - - -   \\
    \hline
    
    It would not be harmful & - - - & - &  - - - & - - - & - - - & - - -  \\
    \hline
    
    I find the product reliable & - - - & - &  - - - & - - - & - - - & - - - \\
    \hline
    
    I would trust the product & 0.5784 & 65 &  2.1066 & \cellcolor{AbiOrangeQuote}.0390 & .234 & .5148

    \end{tabular}

    \caption{Guideline 14's t-test results %(\checkmark if Welch's t-test) 
    for the ``by process'' learning style vs. the ``by tinkering'' learning style participants' average ratings of the independent Violation AI product (top) and Application AI product (bottom), for all 10 dependent variables.
    If dashes (- - -) are present, no statistical test was performed.
    If the number of tests exceeded 5 for each product, Bonferroni correction applied by multiplying p-values by the number of tests performed.
    }
    \label{tab:G14-Learn-Stats-Appendix}
\end{table}
\clearpage
%---------------------------------------------------- End Guideline 14

%Begin Guideline 15---------------------------------------------------

\begin{table}[]
    \centering
    \begin{tabular}{cc|cc|cc|cc|cc}
    \multicolumn{2}{c|}{\includegraphics[width = 0.16\columnwidth]{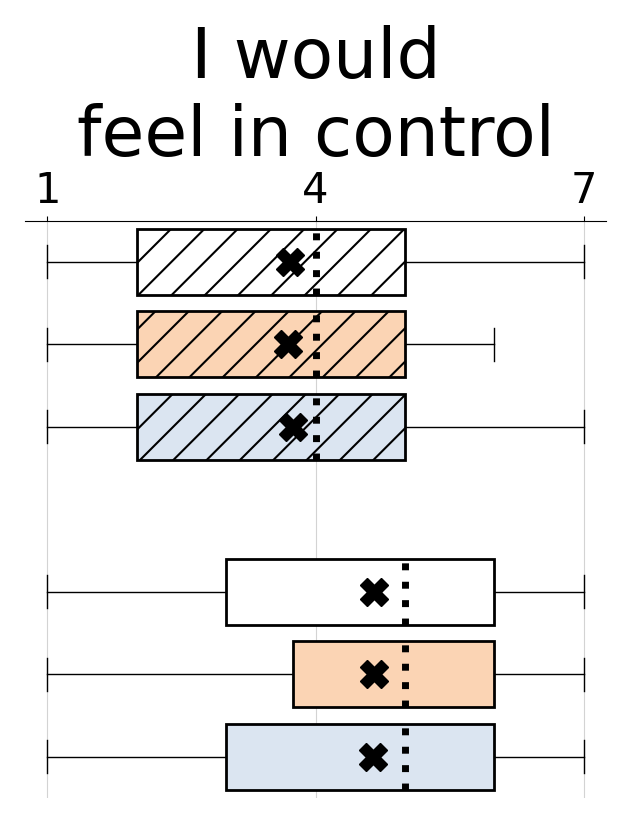}} &
    \multicolumn{2}{c|}{\includegraphics[width = 0.16\columnwidth]{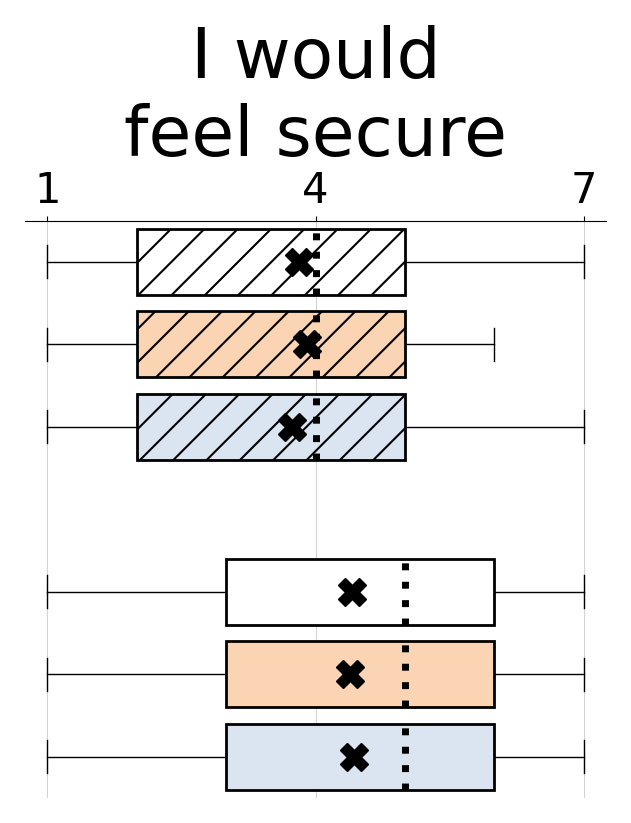}} &
    \multicolumn{2}{c|}{\includegraphics[width = 0.16\columnwidth]{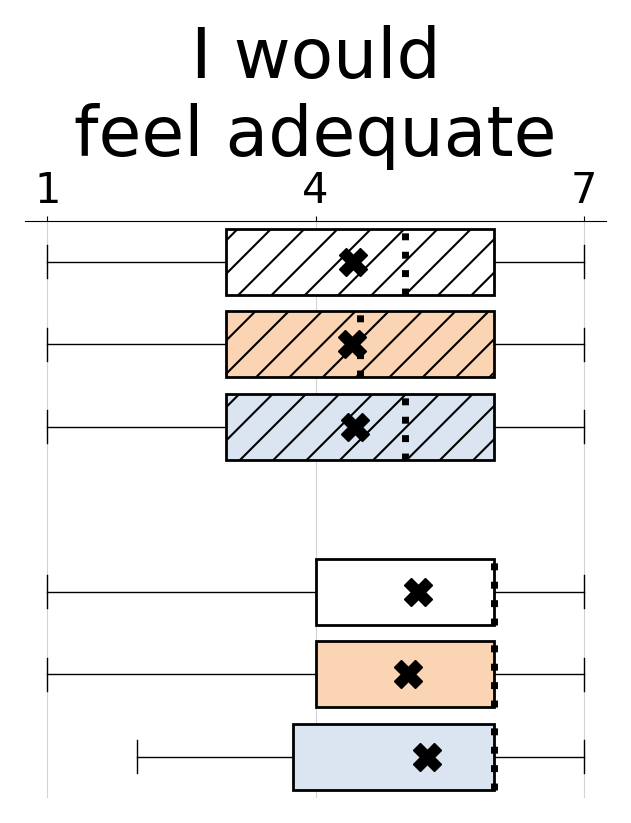}} &
    \multicolumn{2}{c|}{\includegraphics[width = 0.16\columnwidth]{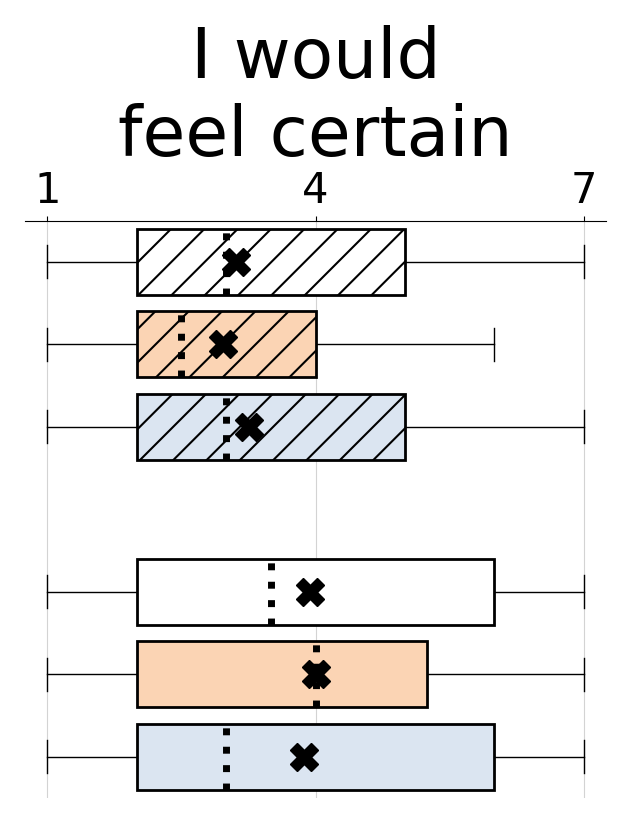}} &
    \multicolumn{2}{c}{\includegraphics[width = 0.16\columnwidth]{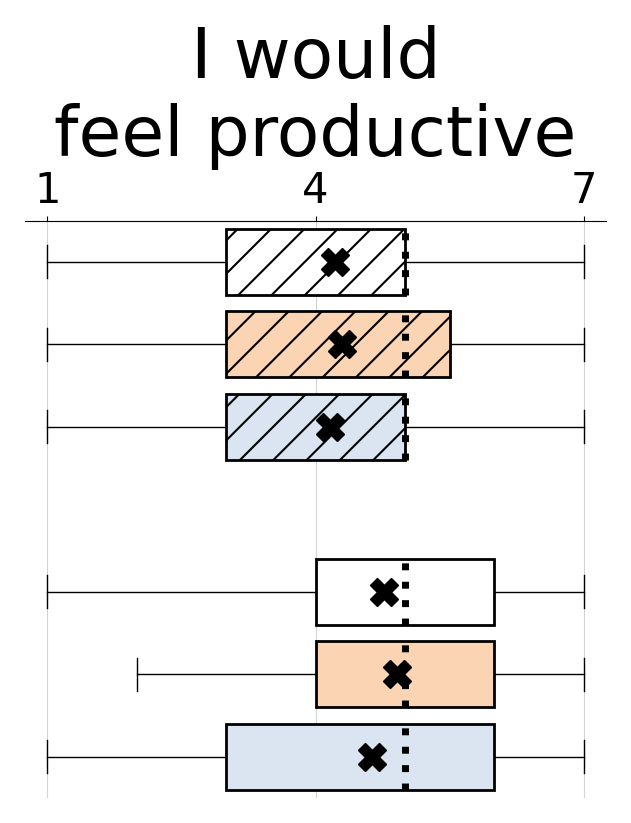}}
    \\
    \hline
    \hline
    \multicolumn{2}{c|}{\includegraphics[width = 0.16\columnwidth]{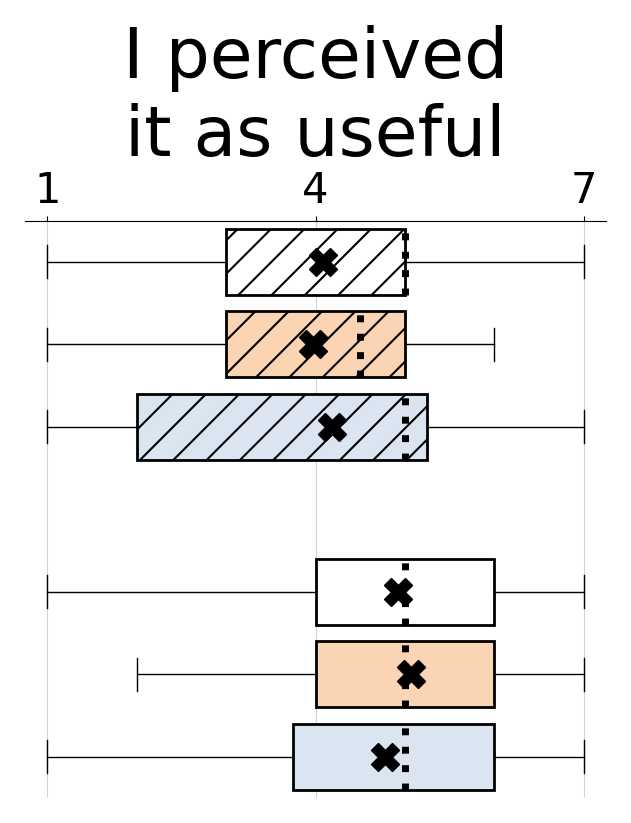}} &
    \multicolumn{2}{c|}{\includegraphics[width = 0.16\columnwidth]{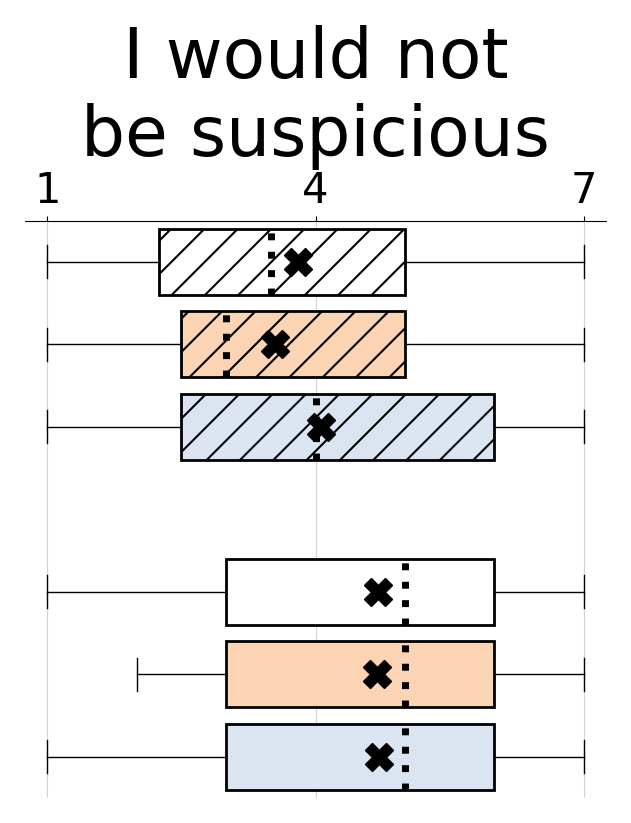}} &
    \multicolumn{2}{c|}{\includegraphics[width = 0.16\columnwidth]{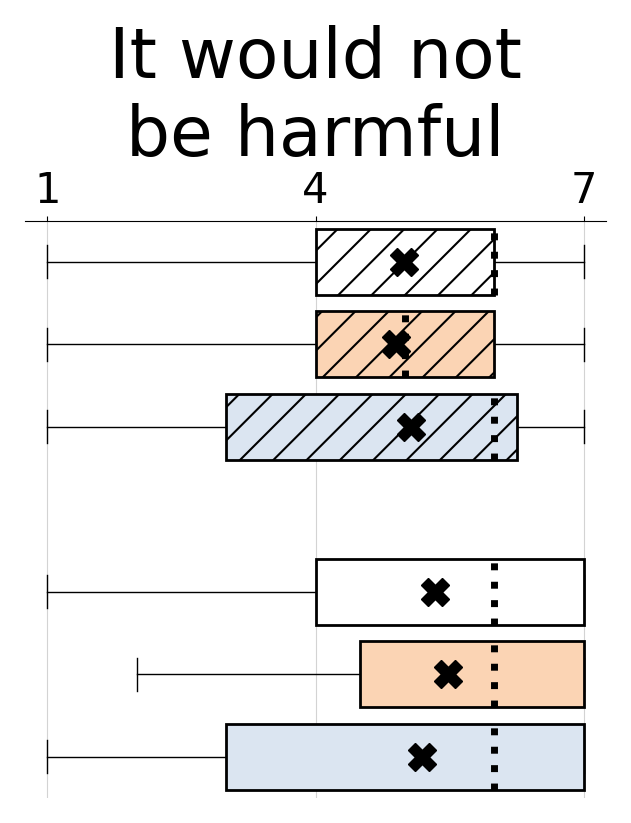}} &
    \multicolumn{2}{c|}{\includegraphics[width = 0.16\columnwidth]{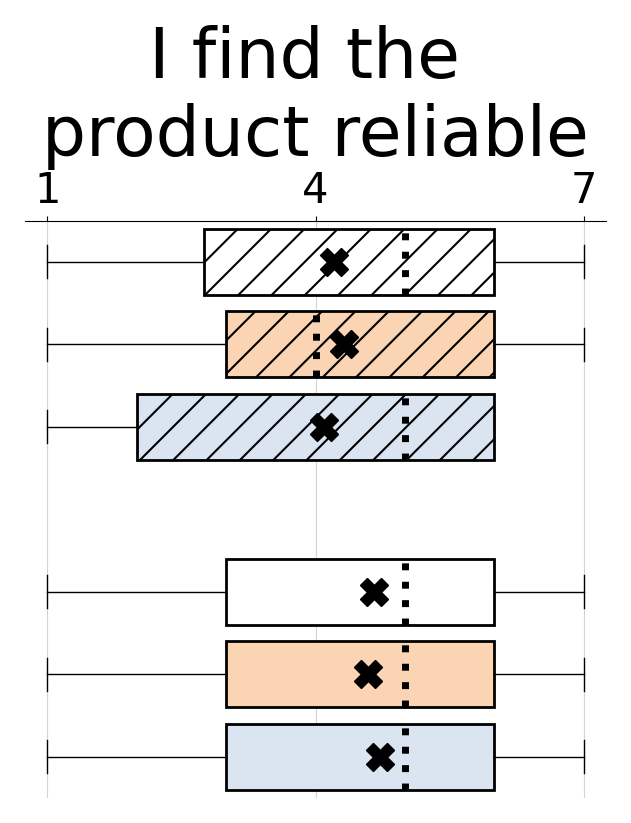}} &
    \multicolumn{2}{c}{\includegraphics[width = 0.16\columnwidth]{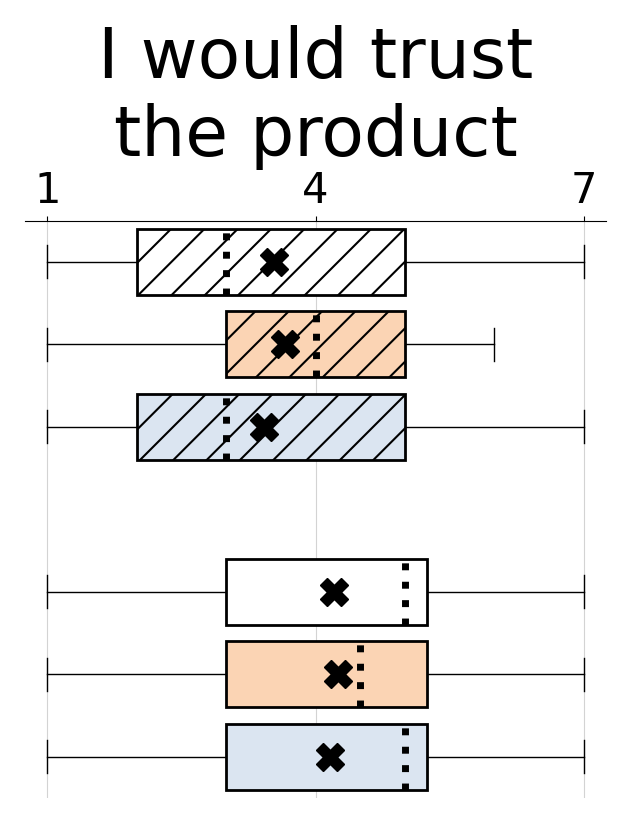}}
    \end{tabular}
    
    \caption{Guideline 15 participants' ratings for all dependent variables, disaggregated by participants' learning styles: by process vs. by tinkering.
	%For the disaggregated data, notice how large the distances between the average rating are when the guideline is applied.
	Table~\ref{tab:G15-Learn-Stats-Appendix} below provides the statistics (where applicable).
}
    \label{fig:Learn-G15-Appendix}
\end{table}

\begin{table}[h]

%\framebox[\linewidth]{For Measuring!}
\centering
\footnotesize

    \begin{tabular}{p{0.22\columnwidth}|c|c|c|c|c|c}
    
    \rowcolor{LightGray}\multicolumn{7}{c}{\textbf{Violation AI Product}}\\
    \hline
    \textbf{Dependent}  & \textbf{Distance b/w} &  &  & & \textbf{Bonferroni} &  \\
    \textbf{variable} & \textbf{Means} &  \textbf{df} &  \textbf{t-val} &   \textbf{p-value}  & \textbf{correction} & \textbf{Cohen's \textit{d}} \\
    \hline
    
    I would feel in control & - - - & - &  - - - & - - - & - - - & - - -  \\
    \hline
    
    I would feel secure & - - - & - &  - - - & - - - & - - - & - - - \\
    \hline
    
    I would feel adequate & - - - & - &  - - - & - - - & - - - & - - - \\
    \hline
    
    I would feel certain & - - - & - &  - - - & - - - & - - - & - - - \\
    \hline
    
    I would feel productive & - - - & - &  - - - & - - - & - - - & - - -   \\
    \hline
    \hline
    
    I perceived it as useful &  - - - & - &  - - - & - - - & - - - & - - -   \\
    \hline
    
    I would not be suspicious & - - - & - &  - - - & - - - & - - - & - - -   \\
    \hline
    
    It would not be harmful & - - - & - &  - - - & - - - & - - - & - - -  \\
    \hline
    
    I find the product reliable & - - - & - &  - - - & - - - & - - - & - - - \\
    \hline
    
    I would trust the product & - - - & - &  - - - & - - - & - - - & - - - \\
    \hline

    \rowcolor{LightGray}\multicolumn{7}{c}{\textbf{Application AI Product}}\\
    \hline
    \textbf{Dependent}  & \textbf{Distance b/w} &  &  & & \textbf{Bonferroni} &  \\
    \textbf{variable} & \textbf{Means} &  \textbf{df} &  \textbf{t-val} &   \textbf{p-value}  & \textbf{correction} & \textbf{Cohen's \textit{d}} \\
    \hline
    
    I would feel in control & - - - & - &  - - - & - - - & - - - & - - -  \\
    \hline
    
    I would feel secure & - - - & - &  - - - & - - - & - - - & - - - \\
    \hline
    
    I would feel adequate & - - - & - &  - - - & - - - & - - - & - - - \\
    \hline
    
    I would feel certain & - - - & - &  - - - & - - - & - - - & - - - \\
    \hline
    
    I would feel productive & - - - & - &  - - - & - - - & - - - & - - -   \\
    \hline
    \hline
    
    I perceived it as useful &  - - - & - &  - - - & - - - & - - - & - - -   \\
    \hline
    
    I would not be suspicious & - - - & - &  - - - & - - - & - - - & - - -   \\
    \hline
    
    It would not be harmful & - - - & - &  - - - & - - - & - - - & - - -  \\
    \hline
    
    I find the product reliable & - - - & - &  - - - & - - - & - - - & - - - \\
    \hline
    
    I would trust the product & - - - & - &  - - - & - - - & - - - & - - -

    \end{tabular}

    \caption{Guideline 15's t-test results %(\checkmark if Welch's t-test) 
    for the ``by process'' learning style vs. the ``by tinkering'' learning style participants' average ratings of the independent Violation AI product (top) and Application AI product (bottom), for all 10 dependent variables.
    If dashes (- - -) are present, no statistical test was performed.
    If the number of tests exceeded 5 for each product, Bonferroni correction applied by multiplying p-values by the number of tests performed.
    }
    \label{tab:G15-Learn-Stats-Appendix}
\end{table}
\clearpage
%---------------------------------------------------- End Guideline 15

%Begin Guideline 17---------------------------------------------------

\begin{table}[]
    \centering
    \begin{tabular}{cc|cc|cc|cc|cc}
    \multicolumn{2}{c|}{\includegraphics[width = 0.16\columnwidth]{assets/05-All-BoxPlots/15-G17/Learn/G17-Feel-In-Control-LEARN.png}} &
    \multicolumn{2}{c|}{\includegraphics[width = 0.16\columnwidth]{assets/05-All-BoxPlots/15-G17/Learn/G17-Feel-Secure-LEARN.png}} &
    \multicolumn{2}{c|}{\includegraphics[width = 0.16\columnwidth]{assets/05-All-BoxPlots/15-G17/Learn/G17-Feel-Adequate-LEARN.png}} &
    \multicolumn{2}{c|}{\includegraphics[width = 0.16\columnwidth]{assets/05-All-BoxPlots/15-G17/Learn/G17-Feel-Certain-LEARN.png}} &
    \multicolumn{2}{c}{\includegraphics[width = 0.16\columnwidth]{assets/05-All-BoxPlots/15-G17/Learn/G17-Feel-Productive-LEARN.png}}
    \\
    \hline
    \hline
    \multicolumn{2}{c|}{\includegraphics[width = 0.16\columnwidth]{assets/05-All-BoxPlots/15-G17/Learn/G17-Perceived-Useful-LEARN.png}} &
    \multicolumn{2}{c|}{\includegraphics[width = 0.16\columnwidth]{assets/05-All-BoxPlots/15-G17/Learn/G17-Not-Suspicious-LEARN.png}} &
    \multicolumn{2}{c|}{\includegraphics[width = 0.16\columnwidth]{assets/05-All-BoxPlots/15-G17/Learn/G17-Not-Harmful-LEARN.png}} &
    \multicolumn{2}{c|}{\includegraphics[width = 0.16\columnwidth]{assets/05-All-BoxPlots/15-G17/Learn/G17-Product-Reliable-LEARN.png}} &
    \multicolumn{2}{c}{\includegraphics[width = 0.16\columnwidth]{assets/05-All-BoxPlots/15-G17/Learn/G17-Trust-Product-LEARN.png}}
    \end{tabular}
    
    \caption{Guideline 17 participants' ratings for all dependent variables, disaggregated by participants' learning styles: by process vs. by tinkering.
	%For the disaggregated data, notice how large the distances between the average rating are when the guideline is applied.
	Table~\ref{tab:G17-Learn-Stats-Appendix} below provides the statistics (where applicable).
}
    \label{fig:Learn-G17-Appendix}
\end{table}

\begin{table}[h]

%\framebox[\linewidth]{For Measuring!}
\centering
\footnotesize

    \begin{tabular}{p{0.22\columnwidth}|c|c|c|c|c|c}
    
    \rowcolor{LightGray}\multicolumn{7}{c}{\textbf{Violation AI Product}}\\
    \hline
    \textbf{Dependent}  & \textbf{Distance b/w} &  &  & & \textbf{Bonferroni} &  \\
    \textbf{variable} & \textbf{Means} &  \textbf{df} &  \textbf{t-val} &   \textbf{p-value}  & \textbf{correction} & \textbf{Cohen's \textit{d}} \\
    \hline
    
    I would feel in control & - - - & - &  - - - & - - - & - - - & - - -  \\
    \hline
    
    I would feel secure & - - - & - &  - - - & - - - & - - - & - - - \\
    \hline
    
    I would feel adequate & - - -  & - &  - - - & - - - & - - - & - - - \\
    \hline
    
    I would feel certain & - - - & - &  - - - & - - - & - - - & - - - \\
    \hline
    
    I would feel productive & - - - & - &  - - - & - - - & - - - & - - -   \\
    \hline
    \hline
    
    I perceived it as useful &  - - - & - &  - - - & - - - & - - - & - - -   \\
    \hline
    
    I would not be suspicious & - - - & - &  - - - & - - - & - - - & - - -   \\
    \hline
    
    It would not be harmful & - - - & - &  - - - & - - - & - - - & - - -  \\
    \hline
    
    I find the product reliable & - - - & - &  - - - & - - - & - - - & - - - \\
    \hline
    
    I would trust the product & - - - & - &  - - - & - - - & - - - & - - - \\
    \hline

    \rowcolor{LightGray}\multicolumn{7}{c}{\textbf{Application AI Product}}\\
    \hline
    \textbf{Dependent}  & \textbf{Distance b/w} &  &  & & \textbf{Bonferroni} &  \\
    \textbf{variable} & \textbf{Means} &  \textbf{df} &  \textbf{t-val} &   \textbf{p-value}  & \textbf{correction} & \textbf{Cohen's \textit{d}} \\
    \hline
    
    I would feel in control & - - - & - &  - - - & - - - & - - - & - - -  \\
    \hline
    
    I would feel secure & - - - & - &  - - - & - - - & - - - & - - - \\
    \hline
    
    I would feel adequate & - - -  & - &  - - - & - - - & - - - & - - - \\
    \hline
    
    I would feel certain & - - - & - &  - - - & - - - & - - - & - - - \\
    \hline
    
    I would feel productive & - - - & - &  - - - & - - - & - - - & - - -   \\
    \hline
    \hline
    
    I perceived it as useful &  - - - & - &  - - - & - - - & - - - & - - -   \\
    \hline
    
    I would not be suspicious & - - - & - &  - - - & - - - & - - - & - - -   \\
    \hline
    
    It would not be harmful & - - - & - &  - - - & - - - & - - - & - - -  \\
    \hline
    
    I find the product reliable & - - - & - &  - - - & - - - & - - - & - - - \\
    \hline
    
    I would trust the product & - - - & - &  - - - & - - - & - - - & - - -

    \end{tabular}

    \caption{Guideline 17's t-test results %(\checkmark if Welch's t-test) 
    for the ``by process'' learning style vs. the ``by tinkering'' learning style participants' average ratings of the independent Violation AI product (top) and Application AI product (bottom), for all 10 dependent variables.
    If dashes (- - -) are present, no statistical test was performed.
    If the number of tests exceeded 5 for each product, Bonferroni correction applied by multiplying p-values by the number of tests performed.
    }
    \label{tab:G17-Learn-Stats-Appendix}
\end{table}
\clearpage
%---------------------------------------------------- End Guideline 17

%Begin Guideline 17---------------------------------------------------

\begin{table}[]
    \centering
    \begin{tabular}{cc|cc|cc|cc|cc}
    \multicolumn{2}{c|}{\includegraphics[width = 0.16\columnwidth]{assets/05-All-BoxPlots/16-G18/Learn/G18-Feel-In-Control-LEARN.png}} &
    \multicolumn{2}{c|}{\includegraphics[width = 0.16\columnwidth]{assets/05-All-BoxPlots/16-G18/Learn/G18-Feel-Secure-LEARN.png}} &
    \multicolumn{2}{c|}{\includegraphics[width = 0.16\columnwidth]{assets/05-All-BoxPlots/16-G18/Learn/G18-Feel-Adequate-LEARN.png}} &
    \multicolumn{2}{c|}{\includegraphics[width = 0.16\columnwidth]{assets/05-All-BoxPlots/16-G18/Learn/G18-Feel-Certain-LEARN.png}} &
    \multicolumn{2}{c}{\includegraphics[width = 0.16\columnwidth]{assets/05-All-BoxPlots/16-G18/Learn/G18-Feel-Productive-LEARN.png}}
    \\
    \hline
    \hline
    \multicolumn{2}{c|}{\includegraphics[width = 0.16\columnwidth]{assets/05-All-BoxPlots/16-G18/Learn/G18-Perceived-Useful-LEARN.png}} &
    \multicolumn{2}{c|}{\includegraphics[width = 0.16\columnwidth]{assets/05-All-BoxPlots/16-G18/Learn/G18-Not-Suspicious-LEARN.png}} &
    \multicolumn{2}{c|}{\includegraphics[width = 0.16\columnwidth]{assets/05-All-BoxPlots/16-G18/Learn/G18-Not-Harmful-LEARN.png}} &
    \multicolumn{2}{c|}{\includegraphics[width = 0.16\columnwidth]{assets/05-All-BoxPlots/16-G18/Learn/G18-Product-Reliable-LEARN.png}} &
    \multicolumn{2}{c}{\includegraphics[width = 0.16\columnwidth]{assets/05-All-BoxPlots/16-G18/Learn/G18-Trust-Product-LEARN.png}}
    \end{tabular}
    
    \caption{Guideline 18 participants' ratings for all dependent variables, disaggregated by participants' learning styles: by process vs. by tinkering.
	%For the disaggregated data, notice how large the distances between the average rating are when the guideline is applied.
	Table~\ref{tab:G18-Learn-Stats-Appendix} below provides the statistics (where applicable).
}
    \label{fig:Learn-G18-Appendix}
\end{table}

\begin{table}[h]

%\framebox[\linewidth]{For Measuring!}
\centering
\footnotesize

    \begin{tabular}{p{0.22\columnwidth}|c|c|c|c|c|c}
    
    \rowcolor{LightGray}\multicolumn{7}{c}{\textbf{Violation AI Product}}\\
    \hline
    \textbf{Dependent}  & \textbf{Distance b/w} &  &  & & \textbf{Bonferroni} &  \\
    \textbf{variable} & \textbf{Means} &  \textbf{df} &  \textbf{t-val} &   \textbf{p-value}  & \textbf{correction} & \textbf{Cohen's \textit{d}} \\
    \hline
    
    I would feel in control & - - -  & - &  - - - & - - - & - - - & - - -  \\
    \hline
    
    I would feel secure & - - -  & - &  - - - & - - - & - - - & - - - \\
    \hline
    
    I would feel adequate & 0.6359  & 64 &  1.5618 & .1233 & - - - & 0.3852 \\
    \hline
    
    I would feel certain & 0.9561 & 65 &  2.1776 & \cellcolor{AbiOrangeQuote}.0331 & - - - & 0.5336 \\
    \hline
    
    I would feel productive & 0.6710 & 64   &  1.7476 & .0853 & - - - & 0.4310   \\
    \hline
    \hline
    
    I perceived it as useful &  - - - & - &  - - - & - - - & - - - & - - -   \\
    \hline
    
    I would not be suspicious & 1.1167 & 64 &  2.6771 & \cellcolor{AbiOrangeQuote}.0094 & - - - & 0.6618   \\
    \hline
    
    It would not be harmful & - - - & - &  - - - & - - - & - - - & - - -  \\
    \hline
    
    I find the product reliable & - - - & - &  - - - & - - - & - - - & - - - \\
    \hline
    
    I would trust the product & - - - & - &  - - - & - - - & - - - & - - - \\
    \hline

    \rowcolor{LightGray}\multicolumn{7}{c}{\textbf{Application AI Product}}\\
    \hline
    \textbf{Dependent}  & \textbf{Distance b/w} &  &  & & \textbf{Bonferroni} &  \\
    \textbf{variable} & \textbf{Means} &  \textbf{df} &  \textbf{t-val} &   \textbf{p-value}  & \textbf{correction} & \textbf{Cohen's \textit{d}} \\
    \hline
    
    I would feel in control & - - - & - &  - - - & - - - & - - - & - - -  \\
    \hline
    
    I would feel secure & - - - & - &  - - - & - - - & - - - & - - - \\
    \hline
    
    I would feel adequate & - - -  & - &  - - - & - - - & - - - & - - - \\
    \hline
    
    I would feel certain & 0.7787 & 65 &  1.9323 & .0577 & - - - & 0.4735 \\
    \hline
    
    I would feel productive & - - -  & - &  - - - & - - - & - - - & - - -   \\
    \hline
    \hline
    
    I perceived it as useful &  - - -  & - &  - - - & - - - & - - - & - - -   \\
    \hline
    
    I would not be suspicious & 0.6722 & 64 &  1.7496 & .0850 & - - - & 0.4325   \\
    \hline
    
    It would not be harmful & - - - & - &  - - - & - - - & - - - & - - -  \\
    \hline
    
    I find the product reliable & - - - & - &  - - - & - - - & - - - & - - - \\
    \hline
    
    I would trust the product & - - - & - &  - - - & - - - & - - - & - - -

    \end{tabular}

    \caption{Guideline 18's t-test results %(\checkmark if Welch's t-test) 
    for the ``by process'' learning style vs. the ``by tinkering'' learning style participants' average ratings of the independent Violation AI product (top) and Application AI product (bottom), for all 10 dependent variables.
    If dashes (- - -) are present, no statistical test was performed.
    If the number of tests exceeded 5 for each product, Bonferroni correction applied by multiplying p-values by the number of tests performed.
    }
    \label{tab:G18-Learn-Stats-Appendix}
\end{table}
\clearpage
%---------------------------------------------------- End Guideline 18
