# Supplementary material for: Measuring User Experience Inclusivity in Human-AI Interaction via Five User Problem-Solving Styles
Source: arXiv:2108.00588 source file (2024-02-17)
Supplement: Supplementary file 4 [file Appendix-Boxplots.tex]

\section{Problem Solving Styles Boxplots}
\label{sec:Appendix-Boxplots}

\subsection{Attitudes Toward Risk \hfill pp. 26--41 }
\label{subsec:Appendix-Risk}
\subsection{Learning Style (by process vs. by tinkering) \hfill pp. 42--57}
\label{subsec:Appendix-LearningStyle}
\subsection{Computer Self-Efficacy \hfill pp. 58--73}
\label{subsec:Appendix-SelfEfficacy}
\subsection{Information Processing Style \hfill pp. 74--89}
\label{subsec:Appendix-InfoProc}
\subsection{Motivations \hfill pp. 90--105}
\label{subsec:Appendix-Motivations}
\clearpage

%\href{https://drive.google.com/drive/u/0/folders/1ilsIjpfB8GVcQmcuNgCd3ccj_hnbPvt-}{Link to Our Data Folder. Focus on the by-facet Sheets (eg, SE-Data, etc.)}

%Guideline 1 ------------------------------
\begin{table}[]
    \centering
    % [inline block 0: 2 envs, 4469 chars -> data_tex | \begin{tabular}{cc|cc|cc|cc|cc}     \multicolumn{2}{c|}{\includegraphics[width = 0.16\columnwidth]{assets/05-All-BoxPlot...]


    \caption{Guideline 4's t-test results %(\checkmark if Welch's t-test) 
    for risk-averse vs. risk-tolerant participants' average ratings of the independent Violation AI product (top) and Application AI product (bottom), for all 10 dependent variables.
    If dashes (- - -) are present, no statistical test was performed.
    If the number of tests exceeded 5 for each product, Bonferroni correction applied by multiplying p-values by the number of tests performed.
    }
    \label{tab:G1-Risk-Stats-Appendix}
    
    % \FIXME{MMB@AAA: FYI, I took the \checkmark s out and replaced them with plain text, because the \checkmark vs blank visually stood out so much, I kept mis-seeing it as saying only those 4 rows were signif. or important.\\
    % AAA@MMB: Redid it with Y/N. The Welch's t and t were cluttering up the table too much.\\
    % MMB@AAA: I actually prefer the spelled-out way.  Visually, the table layout now screams WELCHES IS GOOD, and draws attention away from all other columns.  Meta-comment: it might help if you forced yourself to look at this paper with a reader hat on.}

\end{table}

\clearpage
%---------------------------------------------------- End Guideline 1

%Guideline 3 ------------------------------
\begin{table}[]
    \centering
    % [inline block 1: 2 envs, 4469 chars -> data_tex | \begin{tabular}{cc|cc|cc|cc|cc}     \multicolumn{2}{c|}{\includegraphics[width = 0.16\columnwidth]{assets/05-All-BoxPlot...]


    \caption{Guideline 3's t-test results %(\checkmark if Welch's t-test) 
    for risk-averse vs. risk-tolerant participants' average ratings of the independent Violation AI product (top) and Application AI product (bottom), for all 10 dependent variables.
    If dashes (- - -) are present, no statistical test was performed.
    If the number of tests exceeded 5 for each product, Bonferroni correction applied by multiplying p-values by the number of tests performed.
    }
    \label{tab:G3-Risk-Stats-Appendix}
    
    % \FIXME{MMB@AAA: FYI, I took the \checkmark s out and replaced them with plain text, because the \checkmark vs blank visually stood out so much, I kept mis-seeing it as saying only those 4 rows were signif. or important.\\
    % AAA@MMB: Redid it with Y/N. The Welch's t and t were cluttering up the table too much.\\
    % MMB@AAA: I actually prefer the spelled-out way.  Visually, the table layout now screams WELCHES IS GOOD, and draws attention away from all other columns.  Meta-comment: it might help if you forced yourself to look at this paper with a reader hat on.}

\end{table}

\clearpage
%---------------------------------------------------- End Guideline 3

%Begin Guideline 4----------------------------------------------------

\begin{table}[]
    \centering
    % [inline block 2: 2 envs, 4870 chars -> data_tex | \begin{tabular}{cc|cc|cc|cc|cc}     \multicolumn{2}{c|}{\includegraphics[width = 0.16\columnwidth]{assets/05-All-BoxPlot...]


    \caption{Guideline 4's t-test results %(\checkmark if Welch's t-test) 
    for risk-averse vs. risk-tolerant participants' average ratings of the independent Violation AI product (top) and Application AI product (bottom), for all 10 dependent variables.
    If dashes (- - -) are present, no statistical test was performed.
    If the number of tests exceeded 5 for each product, Bonferroni correction applied by multiplying p-values by the number of tests performed.
    }
    \label{tab:G4-Risk-Stats-Appendix}
\end{table}

%---------------------------------------------------- End Guideline 4

\clearpage

%Begin Guideline 5----------------------------------------------------

\begin{table}[]
    \centering
    % [inline block 3: 2 envs, 4504 chars -> data_tex | \begin{tabular}{cc|cc|cc|cc|cc}     \multicolumn{2}{c|}{\includegraphics[width = 0.16\columnwidth]{assets/05-All-BoxPlot...]


    \caption{Guideline 5's t-test results %(\checkmark if Welch's t-test) 
    for risk-averse vs. risk-tolerant participants' average ratings of the independent Violation AI product (top) and Application AI product (bottom), for all 10 dependent variables.
    If dashes (- - -) are present, no statistical test was performed.
    If the number of tests exceeded 5 for each product, Bonferroni correction applied by multiplying p-values by the number of tests performed.
    }
    \label{tab:G5-Risk-Stats-Appendix}
\end{table}

%---------------------------------------------------- End Guideline 5

\clearpage

%Begin Guideline 6----------------------------------------------------

\begin{table}[]
    \centering
    % [inline block 4: 2 envs, 4480 chars -> data_tex | \begin{tabular}{cc|cc|cc|cc|cc}     \multicolumn{2}{c|}{\includegraphics[width = 0.16\columnwidth]{assets/05-All-BoxPlot...]


    \caption{Guideline 6's t-test results %(\checkmark if Welch's t-test) 
    for risk-averse vs. risk-tolerant participants' average ratings of the independent Violation AI product (top) and Application AI product (bottom), for all 10 dependent variables.
    If dashes (- - -) are present, no statistical test was performed.
    If the number of tests exceeded 5 for each product, Bonferroni correction applied by multiplying p-values by the number of tests performed.
    }
    \label{tab:G6-Risk-Stats-Appendix}
\end{table}

%---------------------------------------------------- End Guideline 6

\clearpage

%Begin Guideline 7----------------------------------------------------

\begin{table}[]
    \centering
    % [inline block 5: 2 envs, 4506 chars -> data_tex | \begin{tabular}{cc|cc|cc|cc|cc}     \multicolumn{2}{c|}{\includegraphics[width = 0.16\columnwidth]{assets/05-All-BoxPlot...]


    \caption{Guideline 7's t-test results %(\checkmark if Welch's t-test) 
    for risk-averse vs. risk-tolerant participants' average ratings of the independent Violation AI product (top) and Application AI product (bottom), for all 10 dependent variables.
    If dashes (- - -) are present, no statistical test was performed.
    If the number of tests exceeded 5 for each product, Bonferroni correction applied by multiplying p-values by the number of tests performed.
    }
    \label{tab:G7-Risk-Stats-Appendix}
\end{table}

%---------------------------------------------------- End Guideline 7

\clearpage

%Begin Guideline 8----------------------------------------------------

\begin{table}[]
    \centering
    % [inline block 6: 2 envs, 4515 chars -> data_tex | \begin{tabular}{cc|cc|cc|cc|cc}     \multicolumn{2}{c|}{\includegraphics[width = 0.16\columnwidth]{assets/05-All-BoxPlot...]


    \caption{Guideline 8's t-test results %(\checkmark if Welch's t-test) 
    for risk-averse vs. risk-tolerant participants' average ratings of the independent Violation AI product (top) and Application AI product (bottom), for all 10 dependent variables.
    If dashes (- - -) are present, no statistical test was performed.
    If the number of tests exceeded 5 for each product, Bonferroni correction applied by multiplying p-values by the number of tests performed.
    }
    \label{tab:G8-Risk-Stats-Appendix}
\end{table}
\clearpage
%---------------------------------------------------- End Guideline 8

%Begin Guideline 9----------------------------------------------------

\begin{table}[]
    \centering
    % [inline block 7: 2 envs, 4531 chars -> data_tex | \begin{tabular}{cc|cc|cc|cc|cc}     \multicolumn{2}{c|}{\includegraphics[width = 0.16\columnwidth]{assets/05-All-BoxPlot...]


    \caption{Guideline 9's t-test results %(\checkmark if Welch's t-test) 
    for risk-averse vs. risk-tolerant participants' average ratings of the independent Violation AI product (top) and Application AI product (bottom), for all 10 dependent variables.
    If dashes (- - -) are present, no statistical test was performed.
    If the number of tests exceeded 5 for each product, Bonferroni correction applied by multiplying p-values by the number of tests performed.
    }
    \label{tab:G9-Risk-Stats-Appendix}
\end{table}
\clearpage
%---------------------------------------------------- End Guideline 9

%Begin Guideline 10----------------------------------------------------

\begin{table}[]
    \centering
    % [inline block 8: 2 envs, 4549 chars -> data_tex | \begin{tabular}{cc|cc|cc|cc|cc}     \multicolumn{2}{c|}{\includegraphics[width = 0.16\columnwidth]{assets/05-All-BoxPlot...]


    \caption{Guideline 10's t-test results %(\checkmark if Welch's t-test) 
    for risk-averse vs. risk-tolerant participants' average ratings of the independent Violation AI product (top) and Application AI product (bottom), for all 10 dependent variables.
    If dashes (- - -) are present, no statistical test was performed.
    If the number of tests exceeded 5 for each product, Bonferroni correction applied by multiplying p-values by the number of tests performed.
    }
    \label{tab:G10-Risk-Stats-Appendix}
\end{table}
\clearpage
%---------------------------------------------------- End Guideline 10

%Begin Guideline 11----------------------------------------------------

\begin{table}[]
    \centering
    % [inline block 9: 2 envs, 4567 chars -> data_tex | \begin{tabular}{cc|cc|cc|cc|cc}     \multicolumn{2}{c|}{\includegraphics[width = 0.16\columnwidth]{assets/05-All-BoxPlot...]


    \caption{Guideline 11's t-test results %(\checkmark if Welch's t-test) 
    for risk-averse vs. risk-tolerant participants' average ratings of the independent Violation AI product (top) and Application AI product (bottom), for all 10 dependent variables.
    If dashes (- - -) are present, no statistical test was performed.
    If the number of tests exceeded 5 for each product, Bonferroni correction applied by multiplying p-values by the number of tests performed.
    }
    \label{tab:G11-Risk-Stats-Appendix}
\end{table}
\clearpage
%---------------------------------------------------- End Guideline 11

%Begin Guideline 12----------------------------------------------------

\begin{table}[]
    \centering
    % [inline block 10: 2 envs, 4500 chars -> data_tex | \begin{tabular}{cc|cc|cc|cc|cc}     \multicolumn{2}{c|}{\includegraphics[width = 0.16\columnwidth]{assets/05-All-BoxPlot...]


    \caption{Guideline 12's t-test results %(\checkmark if Welch's t-test) 
    for risk-averse vs. risk-tolerant participants' average ratings of the independent Violation AI product (top) and Application AI product (bottom), for all 10 dependent variables.
    If dashes (- - -) are present, no statistical test was performed.
    If the number of tests exceeded 5 for each product, Bonferroni correction applied by multiplying p-values by the number of tests performed.
    }
    \label{tab:G12-Risk-Stats-Appendix}
\end{table}
\clearpage
%---------------------------------------------------- End Guideline 12

%Begin Guideline 13----------------------------------------------------

\begin{table}[]
    \centering
    % [inline block 11: 2 envs, 4815 chars -> data_tex | \begin{tabular}{cc|cc|cc|cc|cc}     \multicolumn{2}{c|}{\includegraphics[width = 0.16\columnwidth]{assets/05-All-BoxPlot...]


    \caption{Guideline 13's t-test results %(\checkmark if Welch's t-test) 
    for risk-averse vs. risk-tolerant participants' average ratings of the independent Violation AI product (top) and Application AI product (bottom), for all 10 dependent variables.
    If dashes (- - -) are present, no statistical test was performed.
    If the number of tests exceeded 5 for each product, Bonferroni correction applied by multiplying p-values by the number of tests performed.
    }
    \label{tab:G13-Risk-Stats-Appendix}
\end{table}
\clearpage
%---------------------------------------------------- End Guideline 13

%Begin Guideline 14---------------------------------------------------

\begin{table}[]
    \centering
    % [inline block 12: 2 envs, 4626 chars -> data_tex | \begin{tabular}{cc|cc|cc|cc|cc}     \multicolumn{2}{c|}{\includegraphics[width = 0.16\columnwidth]{assets/05-All-BoxPlot...]


    \caption{Guideline 14's t-test results %(\checkmark if Welch's t-test) 
    for risk-averse vs. risk-tolerant participants' average ratings of the independent Violation AI product (top) and Application AI product (bottom), for all 10 dependent variables.
    If dashes (- - -) are present, no statistical test was performed.
    If the number of tests exceeded 5 for each product, Bonferroni correction applied by multiplying p-values by the number of tests performed.
    }
    \label{tab:G14-Risk-Stats-Appendix}
\end{table}
\clearpage
%---------------------------------------------------- End Guideline 14

%Begin Guideline 15---------------------------------------------------

\begin{table}[]
    \centering
    % [inline block 13: 2 envs, 4535 chars -> data_tex | \begin{tabular}{cc|cc|cc|cc|cc}     \multicolumn{2}{c|}{\includegraphics[width = 0.16\columnwidth]{assets/05-All-BoxPlot...]


    \caption{Guideline 15's t-test results %(\checkmark if Welch's t-test) 
    for risk-averse vs. risk-tolerant participants' average ratings of the independent Violation AI product (top) and Application AI product (bottom), for all 10 dependent variables.
    If dashes (- - -) are present, no statistical test was performed.
    If the number of tests exceeded 5 for each product, Bonferroni correction applied by multiplying p-values by the number of tests performed.
    }
    \label{tab:G15-Risk-Stats-Appendix}
\end{table}
\clearpage
%---------------------------------------------------- End Guideline 15

%Begin Guideline 17---------------------------------------------------

\begin{table}[]
    \centering
    % [inline block 14: 2 envs, 4500 chars -> data_tex | \begin{tabular}{cc|cc|cc|cc|cc}     \multicolumn{2}{c|}{\includegraphics[width = 0.16\columnwidth]{assets/05-All-BoxPlot...]


    \caption{Guideline 17's t-test results %(\checkmark if Welch's t-test) 
    for risk-averse vs. risk-tolerant participants' average ratings of the independent Violation AI product (top) and Application AI product (bottom), for all 10 dependent variables.
    If dashes (- - -) are present, no statistical test was performed.
    If the number of tests exceeded 5 for each product, Bonferroni correction applied by multiplying p-values by the number of tests performed.
    }
    \label{tab:G17-Risk-Stats-Appendix}
\end{table}
\clearpage
%---------------------------------------------------- End Guideline 17

%Begin Guideline 17---------------------------------------------------

\begin{table}[]
    \centering
    % [inline block 15: 2 envs, 4784 chars -> data_tex | \begin{tabular}{cc|cc|cc|cc|cc}     \multicolumn{2}{c|}{\includegraphics[width = 0.16\columnwidth]{assets/05-All-BoxPlot...]


    \caption{Guideline 18's t-test results %(\checkmark if Welch's t-test) 
    for risk-averse vs. risk-tolerant participants' average ratings of the independent Violation AI product (top) and Application AI product (bottom), for all 10 dependent variables.
    If dashes (- - -) are present, no statistical test was performed.
    If the number of tests exceeded 5 for each product, Bonferroni correction applied by multiplying p-values by the number of tests performed.
    }
    \label{tab:G18-Risk-Stats-Appendix}
\end{table}
\clearpage
%---------------------------------------------------- End Guideline 18
\clearpage

%Guideline 1 ------------------------------
\begin{table}[]
    \centering
    % [inline block 16: 2 envs, 4510 chars -> data_tex | \begin{tabular}{cc|cc|cc|cc|cc}     \multicolumn{2}{c|}{\includegraphics[width = 0.16\columnwidth]{assets/05-All-BoxPlot...]


    \caption{Guideline 1's t-test results %(\checkmark if Welch's t-test) 
    for task-oriented vs. tech-oriented participants' average ratings of the independent Violation AI product (top) and Application AI product (bottom), for all 10 dependent variables.
    If dashes (- - -) are present, no statistical test was performed.
    If the number of tests exceeded 5 for each product, Bonferroni correction applied by multiplying p-values by the number of tests performed.
    }
    \label{tab:G1-Motiv-Stats-Appendix}
    
    % \FIXME{MMB@AAA: FYI, I took the \checkmark s out and replaced them with plain text, because the \checkmark vs blank visually stood out so much, I kept mis-seeing it as saying only those 4 rows were signif. or important.\\
    % AAA@MMB: Redid it with Y/N. The Welch's t and t were cluttering up the table too much.\\
    % MMB@AAA: I actually prefer the spelled-out way.  Visually, the table layout now screams WELCHES IS GOOD, and draws attention away from all other columns.  Meta-comment: it might help if you forced yourself to look at this paper with a reader hat on.}

\end{table}

\clearpage
%---------------------------------------------------- End Guideline 1

%Guideline 3 ------------------------------
\begin{table}[]
    \centering
    % [inline block 17: 2 envs, 4506 chars -> data_tex | \begin{tabular}{cc|cc|cc|cc|cc}     \multicolumn{2}{c|}{\includegraphics[width = 0.16\columnwidth]{assets/05-All-BoxPlot...]


    \caption{Guideline 3's t-test results %(\checkmark if Welch's t-test) 
    for task-oriented  vs. tech-oriented participants' average ratings of the independent Violation AI product (top) and Application AI product (bottom), for all 10 dependent variables.
    If dashes (- - -) are present, no statistical test was performed.
    If the number of tests exceeded 5 for each product, Bonferroni correction applied by multiplying p-values by the number of tests performed.
    }
    \label{tab:G3-Motiv-Stats-Appendix}
    
    % \FIXME{MMB@AAA: FYI, I took the \checkmark s out and replaced them with plain text, because the \checkmark vs blank visually stood out so much, I kept mis-seeing it as saying only those 4 rows were signif. or important.\\
    % AAA@MMB: Redid it with Y/N. The Welch's t and t were cluttering up the table too much.\\
    % MMB@AAA: I actually prefer the spelled-out way.  Visually, the table layout now screams WELCHES IS GOOD, and draws attention away from all other columns.  Meta-comment: it might help if you forced yourself to look at this paper with a reader hat on.}

\end{table}

\clearpage
%---------------------------------------------------- End Guideline 3

%Begin Guideline 4----------------------------------------------------

\begin{table}[]
    \centering
    % [inline block 18: 2 envs, 4503 chars -> data_tex | \begin{tabular}{cc|cc|cc|cc|cc}     \multicolumn{2}{c|}{\includegraphics[width = 0.16\columnwidth]{assets/05-All-BoxPlot...]


    \caption{Guideline 4's t-test results %(\checkmark if Welch's t-test) 
    for task-oriented vs. tech-oriented participants' average ratings of the independent Violation AI product (top) and Application AI product (bottom), for all 10 dependent variables.
    If dashes (- - -) are present, no statistical test was performed.
    If the number of tests exceeded 5 for each product, Bonferroni correction applied by multiplying p-values by the number of tests performed.
    }
    \label{tab:G4-Motiv-Stats-Appendix}
\end{table}

%---------------------------------------------------- End Guideline 4

\clearpage

%Begin Guideline 5----------------------------------------------------

\begin{table}[]
    \centering
    % [inline block 19: 2 envs, 4509 chars -> data_tex | \begin{tabular}{cc|cc|cc|cc|cc}     \multicolumn{2}{c|}{\includegraphics[width = 0.16\columnwidth]{assets/05-All-BoxPlot...]


    \caption{Guideline 5's t-test results %(\checkmark if Welch's t-test) 
    for task-oriented vs. tech-oriented participants' average ratings of the independent Violation AI product (top) and Application AI product (bottom), for all 10 dependent variables.
    If dashes (- - -) are present, no statistical test was performed.
    If the number of tests exceeded 5 for each product, Bonferroni correction applied by multiplying p-values by the number of tests performed.
    }
    \label{tab:G5-Motiv-Stats-Appendix}
\end{table}

%---------------------------------------------------- End Guideline 5

\clearpage

%Begin Guideline 6----------------------------------------------------

\begin{table}[]
    \centering
    % [inline block 20: 2 envs, 4518 chars -> data_tex | \begin{tabular}{cc|cc|cc|cc|cc}     \multicolumn{2}{c|}{\includegraphics[width = 0.16\columnwidth]{assets/05-All-BoxPlot...]


    \caption{Guideline 6's t-test results %(\checkmark if Welch's t-test) 
    for task-oriented vs. tech-oriented participants' average ratings of the independent Violation AI product (top) and Application AI product (bottom), for all 10 dependent variables.
    If dashes (- - -) are present, no statistical test was performed.
    If the number of tests exceeded 5 for each product, Bonferroni correction applied by multiplying p-values by the number of tests performed.
    }
    \label{tab:G6-Motiv-Stats-Appendix}
\end{table}

%---------------------------------------------------- End Guideline 6

\clearpage

%Begin Guideline 7----------------------------------------------------

\begin{table}[]
    \centering
    % [inline block 21: 2 envs, 4537 chars -> data_tex | \begin{tabular}{cc|cc|cc|cc|cc}     \multicolumn{2}{c|}{\includegraphics[width = 0.16\columnwidth]{assets/05-All-BoxPlot...]


    \caption{Guideline 7's t-test results %(\checkmark if Welch's t-test) 
    for task-oriented vs. tech-oriented participants' average ratings of the independent Violation AI product (top) and Application AI product (bottom), for all 10 dependent variables.
    If dashes (- - -) are present, no statistical test was performed.
    If the number of tests exceeded 5 for each product, Bonferroni correction applied by multiplying p-values by the number of tests performed.
    }
    \label{tab:G7-Motiv-Stats-Appendix}
\end{table}

%---------------------------------------------------- End Guideline 7

\clearpage

%Begin Guideline 8----------------------------------------------------

\begin{table}[]
    \centering
    % [inline block 22: 2 envs, 4537 chars -> data_tex | \begin{tabular}{cc|cc|cc|cc|cc}     \multicolumn{2}{c|}{\includegraphics[width = 0.16\columnwidth]{assets/05-All-BoxPlot...]


    \caption{Guideline 8's t-test results %(\checkmark if Welch's t-test) 
    for task-oriented vs. tech-oriented participants' average ratings of the independent Violation AI product (top) and Application AI product (bottom), for all 10 dependent variables.
    If dashes (- - -) are present, no statistical test was performed.
    If the number of tests exceeded 5 for each product, Bonferroni correction applied by multiplying p-values by the number of tests performed.
    }
    \label{tab:G8-Motiv-Stats-Appendix}
\end{table}
\clearpage
%---------------------------------------------------- End Guideline 8

%Begin Guideline 9----------------------------------------------------

\begin{table}[]
    \centering
    % [inline block 23: 2 envs, 4552 chars -> data_tex | \begin{tabular}{cc|cc|cc|cc|cc}     \multicolumn{2}{c|}{\includegraphics[width = 0.16\columnwidth]{assets/05-All-BoxPlot...]


    \caption{Guideline 9's t-test results %(\checkmark if Welch's t-test) 
    for task-oriented vs. tech-oriented participants' average ratings of the independent Violation AI product (top) and Application AI product (bottom), for all 10 dependent variables.
    If dashes (- - -) are present, no statistical test was performed.
    If the number of tests exceeded 5 for each product, Bonferroni correction applied by multiplying p-values by the number of tests performed.
    }
    \label{tab:G9-Motiv-Stats-Appendix}
\end{table}
\clearpage
%---------------------------------------------------- End Guideline 9

%Begin Guideline 10----------------------------------------------------

\begin{table}[]
    \centering
    % [inline block 24: 2 envs, 4596 chars -> data_tex | \begin{tabular}{cc|cc|cc|cc|cc}     \multicolumn{2}{c|}{\includegraphics[width = 0.16\columnwidth]{assets/05-All-BoxPlot...]


    \caption{Guideline 10's t-test results %(\checkmark if Welch's t-test) 
    for task-oriented vs. tech-oriented participants' average ratings of the independent Violation AI product (top) and Application AI product (bottom), for all 10 dependent variables.
    If dashes (- - -) are present, no statistical test was performed.
    If the number of tests exceeded 5 for each product, Bonferroni correction applied by multiplying p-values by the number of tests performed.
    }
    \label{tab:G10-Motiv-Stats-Appendix}
\end{table}
\clearpage
%---------------------------------------------------- End Guideline 10

%Begin Guideline 11----------------------------------------------------

\begin{table}[]
    \centering
    % [inline block 25: 2 envs, 4527 chars -> data_tex | \begin{tabular}{cc|cc|cc|cc|cc}     \multicolumn{2}{c|}{\includegraphics[width = 0.16\columnwidth]{assets/05-All-BoxPlot...]


    \caption{Guideline 11's t-test results %(\checkmark if Welch's t-test) 
    for task-oriented vs. tech-oriented participants' average ratings of the independent Violation AI product (top) and Application AI product (bottom), for all 10 dependent variables.
    If dashes (- - -) are present, no statistical test was performed.
    If the number of tests exceeded 5 for each product, Bonferroni correction applied by multiplying p-values by the number of tests performed.
    }
    \label{tab:G11-Motiv-Stats-Appendix}
\end{table}
\clearpage
%---------------------------------------------------- End Guideline 11

%Begin Guideline 12----------------------------------------------------

\begin{table}[]
    \centering
    % [inline block 26: 2 envs, 4561 chars -> data_tex | \begin{tabular}{cc|cc|cc|cc|cc}     \multicolumn{2}{c|}{\includegraphics[width = 0.16\columnwidth]{assets/05-All-BoxPlot...]


    \caption{Guideline 12's t-test results %(\checkmark if Welch's t-test) 
    for task-oriented vs. tech-oriented participants' average ratings of the independent Violation AI product (top) and Application AI product (bottom), for all 10 dependent variables.
    If dashes (- - -) are present, no statistical test was performed.
    If the number of tests exceeded 5 for each product, Bonferroni correction applied by multiplying p-values by the number of tests performed.
    }
    \label{tab:G12-Motiv-Stats-Appendix}
\end{table}
\clearpage
%---------------------------------------------------- End Guideline 12

%Begin Guideline 13----------------------------------------------------

\begin{table}[]
    \centering
    % [inline block 27: 2 envs, 4541 chars -> data_tex | \begin{tabular}{cc|cc|cc|cc|cc}     \multicolumn{2}{c|}{\includegraphics[width = 0.16\columnwidth]{assets/05-All-BoxPlot...]


    \caption{Guideline 13's t-test results %(\checkmark if Welch's t-test) 
    for task-oriented vs. tech-oriented participants' average ratings of the independent Violation AI product (top) and Application AI product (bottom), for all 10 dependent variables.
    If dashes (- - -) are present, no statistical test was performed.
    If the number of tests exceeded 5 for each product, Bonferroni correction applied by multiplying p-values by the number of tests performed.
    }
    \label{tab:G13-Motiv-Stats-Appendix}
\end{table}
\clearpage
%---------------------------------------------------- End Guideline 13

%Begin Guideline 14---------------------------------------------------

\begin{table}[]
    \centering
    % [inline block 28: 2 envs, 4532 chars -> data_tex | \begin{tabular}{cc|cc|cc|cc|cc}     \multicolumn{2}{c|}{\includegraphics[width = 0.16\columnwidth]{assets/05-All-BoxPlot...]


    \caption{Guideline 14's t-test results %(\checkmark if Welch's t-test) 
    for task-oriented vs. tech-oriented participants' average ratings of the independent Violation AI product (top) and Application AI product (bottom), for all 10 dependent variables.
    If dashes (- - -) are present, no statistical test was performed.
    If the number of tests exceeded 5 for each product, Bonferroni correction applied by multiplying p-values by the number of tests performed.
    }
    \label{tab:G14-Motiv-Stats-Appendix}
\end{table}
\clearpage
%---------------------------------------------------- End Guideline 14

%Begin Guideline 15---------------------------------------------------

\begin{table}[]
    \centering
    % [inline block 29: 2 envs, 4542 chars -> data_tex | \begin{tabular}{cc|cc|cc|cc|cc}     \multicolumn{2}{c|}{\includegraphics[width = 0.16\columnwidth]{assets/05-All-BoxPlot...]


    \caption{Guideline 15's t-test results %(\checkmark if Welch's t-test) 
    for task-oriented vs. tech-oriented participants' average ratings of the independent Violation AI product (top) and Application AI product (bottom), for all 10 dependent variables.
    If dashes (- - -) are present, no statistical test was performed.
    If the number of tests exceeded 5 for each product, Bonferroni correction applied by multiplying p-values by the number of tests performed.
    }
    \label{tab:G15-Motiv-Stats-Appendix}
\end{table}
\clearpage
%---------------------------------------------------- End Guideline 15

%Begin Guideline 17---------------------------------------------------

\begin{table}[]
    \centering
    % [inline block 30: 2 envs, 4533 chars -> data_tex | \begin{tabular}{cc|cc|cc|cc|cc}     \multicolumn{2}{c|}{\includegraphics[width = 0.16\columnwidth]{assets/05-All-BoxPlot...]


    \caption{Guideline 17's t-test results %(\checkmark if Welch's t-test) 
    for task-oriented vs. tech-oriented participants' average ratings of the independent Violation AI product (top) and Application AI product (bottom), for all 10 dependent variables.
    If dashes (- - -) are present, no statistical test was performed.
    If the number of tests exceeded 5 for each product, Bonferroni correction applied by multiplying p-values by the number of tests performed.
    }
    \label{tab:G17-Motiv-Stats-Appendix}
\end{table}
\clearpage
%---------------------------------------------------- End Guideline 17

%Begin Guideline 17---------------------------------------------------

\begin{table}[]
    \centering
    % [inline block 31: 2 envs, 4605 chars -> data_tex | \begin{tabular}{cc|cc|cc|cc|cc}     \multicolumn{2}{c|}{\includegraphics[width = 0.16\columnwidth]{assets/05-All-BoxPlot...]


    \caption{Guideline 18's t-test results %(\checkmark if Welch's t-test) 
    for task-oriented vs. tech-oriented participants' average ratings of the independent Violation AI product (top) and Application AI product (bottom), for all 10 dependent variables.
    If dashes (- - -) are present, no statistical test was performed.
    If the number of tests exceeded 5 for each product, Bonferroni correction applied by multiplying p-values by the number of tests performed.
    }
    \label{tab:G18-Motiv-Stats-Appendix}
\end{table}
\clearpage
%---------------------------------------------------- End Guideline 18
\clearpage

%Guideline 1 ------------------------------
\begin{table}[]
    \centering
    % [inline block 32: 2 envs, 4514 chars -> data_tex | \begin{tabular}{cc|cc|cc|cc|cc}     \multicolumn{2}{c|}{\includegraphics[width = 0.16\columnwidth]{assets/05-All-BoxPlot...]


    \caption{Guideline 1's t-test results %(\checkmark if Welch's t-test) 
    for the ``by process'' learning style vs. the ``by tinkering'' learning style participants' average ratings of the independent Violation AI product (top) and Application AI product (bottom), for all 10 dependent variables.
    If dashes (- - -) are present, no statistical test was performed.
    If the number of tests exceeded 5 for each product, Bonferroni correction applied by multiplying p-values by the number of tests performed.
    }
    \label{tab:G1-Learn-Stats-Appendix}
    
    % \FIXME{MMB@AAA: FYI, I took the \checkmark s out and replaced them with plain text, because the \checkmark vs blank visually stood out so much, I kept mis-seeing it as saying only those 4 rows were signif. or important.\\
    % AAA@MMB: Redid it with Y/N. The Welch's t and t were cluttering up the table too much.\\
    % MMB@AAA: I actually prefer the spelled-out way.  Visually, the table layout now screams WELCHES IS GOOD, and draws attention away from all other columns.  Meta-comment: it might help if you forced yourself to look at this paper with a reader hat on.}

\end{table}

\clearpage
%---------------------------------------------------- End Guideline 1

%Guideline 3 ------------------------------
\begin{table}[]
    \centering
    % [inline block 33: 2 envs, 4540 chars -> data_tex | \begin{tabular}{cc|cc|cc|cc|cc}     \multicolumn{2}{c|}{\includegraphics[width = 0.16\columnwidth]{assets/05-All-BoxPlot...]


    \caption{Guideline 3's t-test results %(\checkmark if Welch's t-test) 
    for the ``by process'' learning style vs. the ``by tinkering'' learning style participants' average ratings of the independent Violation AI product (top) and Application AI product (bottom), for all 10 dependent variables.
    If dashes (- - -) are present, no statistical test was performed.
    If the number of tests exceeded 5 for each product, Bonferroni correction applied by multiplying p-values by the number of tests performed.
    }
    \label{tab:G3-Learn-Stats-Appendix}
    
    % \FIXME{MMB@AAA: FYI, I took the \checkmark s out and replaced them with plain text, because the \checkmark vs blank visually stood out so much, I kept mis-seeing it as saying only those 4 rows were signif. or important.\\
    % AAA@MMB: Redid it with Y/N. The Welch's t and t were cluttering up the table too much.\\
    % MMB@AAA: I actually prefer the spelled-out way.  Visually, the table layout now screams WELCHES IS GOOD, and draws attention away from all other columns.  Meta-comment: it might help if you forced yourself to look at this paper with a reader hat on.}

\end{table}

\clearpage
%---------------------------------------------------- End Guideline 3

%Begin Guideline 4----------------------------------------------------

\begin{table}[]
    \centering
    % [inline block 34: 2 envs, 4661 chars -> data_tex | \begin{tabular}{cc|cc|cc|cc|cc}     \multicolumn{2}{c|}{\includegraphics[width = 0.16\columnwidth]{assets/05-All-BoxPlot...]


    \caption{Guideline 4's t-test results %(\checkmark if Welch's t-test) 
    for the ``by process'' learning style vs. the ``by tinkering'' learning style participants' average ratings of the independent Violation AI product (top) and Application AI product (bottom), for all 10 dependent variables.
    If dashes (- - -) are present, no statistical test was performed.
    If the number of tests exceeded 5 for each product, Bonferroni correction applied by multiplying p-values by the number of tests performed.
    }
    \label{tab:G4-Learn-Stats-Appendix}
\end{table}

%---------------------------------------------------- End Guideline 4

\clearpage

%Begin Guideline 5----------------------------------------------------

\begin{table}[]
    \centering
    % [inline block 35: 2 envs, 4546 chars -> data_tex | \begin{tabular}{cc|cc|cc|cc|cc}     \multicolumn{2}{c|}{\includegraphics[width = 0.16\columnwidth]{assets/05-All-BoxPlot...]


    \caption{Guideline 5's t-test results %(\checkmark if Welch's t-test) 
    for the ``by process'' learning style vs. the ``by tinkering'' learning style participants' average ratings of the independent Violation AI product (top) and Application AI product (bottom), for all 10 dependent variables.
    If dashes (- - -) are present, no statistical test was performed.
    If the number of tests exceeded 5 for each product, Bonferroni correction applied by multiplying p-values by the number of tests performed.
    }
    \label{tab:G5-Learn-Stats-Appendix}
\end{table}

%---------------------------------------------------- End Guideline 5

\clearpage

%Begin Guideline 6----------------------------------------------------

\begin{table}[]
    \centering
    % [inline block 36: 2 envs, 4559 chars -> data_tex | \begin{tabular}{cc|cc|cc|cc|cc}     \multicolumn{2}{c|}{\includegraphics[width = 0.16\columnwidth]{assets/05-All-BoxPlot...]


    \caption{Guideline 6's t-test results %(\checkmark if Welch's t-test) 
    for the ``by process'' learning style vs. the ``by tinkering'' learning style participants' average ratings of the independent Violation AI product (top) and Application AI product (bottom), for all 10 dependent variables.
    If dashes (- - -) are present, no statistical test was performed.
    If the number of tests exceeded 5 for each product, Bonferroni correction applied by multiplying p-values by the number of tests performed.
    }
    \label{tab:G6-Learn-Stats-Appendix}
\end{table}

%---------------------------------------------------- End Guideline 6

\clearpage

%Begin Guideline 7----------------------------------------------------

\begin{table}[]
    \centering
    % [inline block 37: 2 envs, 4522 chars -> data_tex | \begin{tabular}{cc|cc|cc|cc|cc}     \multicolumn{2}{c|}{\includegraphics[width = 0.16\columnwidth]{assets/05-All-BoxPlot...]


    \caption{Guideline 7's t-test results %(\checkmark if Welch's t-test) 
    for the ``by process'' learning style vs. the ``by tinkering'' learning style participants' average ratings of the independent Violation AI product (top) and Application AI product (bottom), for all 10 dependent variables.
    If dashes (- - -) are present, no statistical test was performed.
    If the number of tests exceeded 5 for each product, Bonferroni correction applied by multiplying p-values by the number of tests performed.
    }
    \label{tab:G7-Learn-Stats-Appendix}
\end{table}

%---------------------------------------------------- End Guideline 7

\clearpage

%Begin Guideline 8----------------------------------------------------

\begin{table}[]
    \centering
    % [inline block 38: 2 envs, 4520 chars -> data_tex | \begin{tabular}{cc|cc|cc|cc|cc}     \multicolumn{2}{c|}{\includegraphics[width = 0.16\columnwidth]{assets/05-All-BoxPlot...]


    \caption{Guideline 8's t-test results %(\checkmark if Welch's t-test) 
    for the ``by process'' learning style vs. the ``by tinkering'' learning style participants' average ratings of the independent Violation AI product (top) and Application AI product (bottom), for all 10 dependent variables.
    If dashes (- - -) are present, no statistical test was performed.
    If the number of tests exceeded 5 for each product, Bonferroni correction applied by multiplying p-values by the number of tests performed.
    }
    \label{tab:G8-Learn-Stats-Appendix}
\end{table}
\clearpage
%---------------------------------------------------- End Guideline 8

%Begin Guideline 9----------------------------------------------------

\begin{table}[]
    \centering
    % [inline block 39: 2 envs, 4518 chars -> data_tex | \begin{tabular}{cc|cc|cc|cc|cc}     \multicolumn{2}{c|}{\includegraphics[width = 0.16\columnwidth]{assets/05-All-BoxPlot...]


    \caption{Guideline 9's t-test results %(\checkmark if Welch's t-test) 
    for the ``by process'' learning style vs. the ``by tinkering'' learning style participants' average ratings of the independent Violation AI product (top) and Application AI product (bottom), for all 10 dependent variables.
    If dashes (- - -) are present, no statistical test was performed.
    If the number of tests exceeded 5 for each product, Bonferroni correction applied by multiplying p-values by the number of tests performed.
    }
    \label{tab:G9-Learn-Stats-Appendix}
\end{table}
\clearpage
%---------------------------------------------------- End Guideline 9

%Begin Guideline 10----------------------------------------------------

\begin{table}[]
    \centering
    % [inline block 40: 2 envs, 4569 chars -> data_tex | \begin{tabular}{cc|cc|cc|cc|cc}     \multicolumn{2}{c|}{\includegraphics[width = 0.16\columnwidth]{assets/05-All-BoxPlot...]


    \caption{Guideline 10's t-test results %(\checkmark if Welch's t-test) 
    for the ``by process'' learning style vs. the ``by tinkering'' learning style participants' average ratings of the independent Violation AI product (top) and Application AI product (bottom), for all 10 dependent variables.
    If dashes (- - -) are present, no statistical test was performed.
    If the number of tests exceeded 5 for each product, Bonferroni correction applied by multiplying p-values by the number of tests performed.
    }
    \label{tab:G10-Learn-Stats-Appendix}
\end{table}
\clearpage
%---------------------------------------------------- End Guideline 10

%Begin Guideline 11----------------------------------------------------

\begin{table}[]
    \centering
    % [inline block 41: 2 envs, 4570 chars -> data_tex | \begin{tabular}{cc|cc|cc|cc|cc}     \multicolumn{2}{c|}{\includegraphics[width = 0.16\columnwidth]{assets/05-All-BoxPlot...]


    \caption{Guideline 11's t-test results %(\checkmark if Welch's t-test) 
    for the ``by process'' learning style vs. the ``by tinkering'' learning style participants' average ratings of the independent Violation AI product (top) and Application AI product (bottom), for all 10 dependent variables.
    If dashes (- - -) are present, no statistical test was performed.
    If the number of tests exceeded 5 for each product, Bonferroni correction applied by multiplying p-values by the number of tests performed.
    }
    \label{tab:G11-Learn-Stats-Appendix}
\end{table}
\clearpage
%---------------------------------------------------- End Guideline 11

%Begin Guideline 12----------------------------------------------------

\begin{table}[]
    \centering
    % [inline block 42: 2 envs, 4545 chars -> data_tex | \begin{tabular}{cc|cc|cc|cc|cc}     \multicolumn{2}{c|}{\includegraphics[width = 0.16\columnwidth]{assets/05-All-BoxPlot...]


    \caption{Guideline 12's t-test results %(\checkmark if Welch's t-test) 
    for the ``by process'' learning style vs. the ``by tinkering'' learning style participants' average ratings of the independent Violation AI product (top) and Application AI product (bottom), for all 10 dependent variables.
    If dashes (- - -) are present, no statistical test was performed.
    If the number of tests exceeded 5 for each product, Bonferroni correction applied by multiplying p-values by the number of tests performed.
    }
    \label{tab:G12-Learn-Stats-Appendix}
\end{table}
\clearpage
%---------------------------------------------------- End Guideline 12

%Begin Guideline 13----------------------------------------------------

\begin{table}[]
    \centering
    % [inline block 43: 2 envs, 4717 chars -> data_tex | \begin{tabular}{cc|cc|cc|cc|cc}     \multicolumn{2}{c|}{\includegraphics[width = 0.16\columnwidth]{assets/05-All-BoxPlot...]


    \caption{Guideline 13's t-test results %(\checkmark if Welch's t-test) 
    for the ``by process'' learning style vs. the ``by tinkering'' learning style participants' average ratings of the independent Violation AI product (top) and Application AI product (bottom), for all 10 dependent variables.
    If dashes (- - -) are present, no statistical test was performed.
    If the number of tests exceeded 5 for each product, Bonferroni correction applied by multiplying p-values by the number of tests performed.
    }
    \label{tab:G13-Learn-Stats-Appendix}
\end{table}
\clearpage
%---------------------------------------------------- End Guideline 13

%Begin Guideline 14---------------------------------------------------

\begin{table}[]
    \centering
    % [inline block 44: 2 envs, 4797 chars -> data_tex | \begin{tabular}{cc|cc|cc|cc|cc}     \multicolumn{2}{c|}{\includegraphics[width = 0.16\columnwidth]{assets/05-All-BoxPlot...]


    \caption{Guideline 14's t-test results %(\checkmark if Welch's t-test) 
    for the ``by process'' learning style vs. the ``by tinkering'' learning style participants' average ratings of the independent Violation AI product (top) and Application AI product (bottom), for all 10 dependent variables.
    If dashes (- - -) are present, no statistical test was performed.
    If the number of tests exceeded 5 for each product, Bonferroni correction applied by multiplying p-values by the number of tests performed.
    }
    \label{tab:G14-Learn-Stats-Appendix}
\end{table}
\clearpage
%---------------------------------------------------- End Guideline 14

%Begin Guideline 15---------------------------------------------------

\begin{table}[]
    \centering
    % [inline block 45: 2 envs, 4543 chars -> data_tex | \begin{tabular}{cc|cc|cc|cc|cc}     \multicolumn{2}{c|}{\includegraphics[width = 0.16\columnwidth]{assets/05-All-BoxPlot...]


    \caption{Guideline 15's t-test results %(\checkmark if Welch's t-test) 
    for the ``by process'' learning style vs. the ``by tinkering'' learning style participants' average ratings of the independent Violation AI product (top) and Application AI product (bottom), for all 10 dependent variables.
    If dashes (- - -) are present, no statistical test was performed.
    If the number of tests exceeded 5 for each product, Bonferroni correction applied by multiplying p-values by the number of tests performed.
    }
    \label{tab:G15-Learn-Stats-Appendix}
\end{table}
\clearpage
%---------------------------------------------------- End Guideline 15

%Begin Guideline 17---------------------------------------------------

\begin{table}[]
    \centering
    % [inline block 46: 2 envs, 4545 chars -> data_tex | \begin{tabular}{cc|cc|cc|cc|cc}     \multicolumn{2}{c|}{\includegraphics[width = 0.16\columnwidth]{assets/05-All-BoxPlot...]


    \caption{Guideline 17's t-test results %(\checkmark if Welch's t-test) 
    for the ``by process'' learning style vs. the ``by tinkering'' learning style participants' average ratings of the independent Violation AI product (top) and Application AI product (bottom), for all 10 dependent variables.
    If dashes (- - -) are present, no statistical test was performed.
    If the number of tests exceeded 5 for each product, Bonferroni correction applied by multiplying p-values by the number of tests performed.
    }
    \label{tab:G17-Learn-Stats-Appendix}
\end{table}
\clearpage
%---------------------------------------------------- End Guideline 17

%Begin Guideline 17---------------------------------------------------

\begin{table}[]
    \centering
    % [inline block 47: 2 envs, 4627 chars -> data_tex | \begin{tabular}{cc|cc|cc|cc|cc}     \multicolumn{2}{c|}{\includegraphics[width = 0.16\columnwidth]{assets/05-All-BoxPlot...]


    \caption{Guideline 18's t-test results %(\checkmark if Welch's t-test) 
    for the ``by process'' learning style vs. the ``by tinkering'' learning style participants' average ratings of the independent Violation AI product (top) and Application AI product (bottom), for all 10 dependent variables.
    If dashes (- - -) are present, no statistical test was performed.
    If the number of tests exceeded 5 for each product, Bonferroni correction applied by multiplying p-values by the number of tests performed.
    }
    \label{tab:G18-Learn-Stats-Appendix}
\end{table}
\clearpage
%---------------------------------------------------- End Guideline 18
\clearpage

%Guideline 1 ------------------------------
\begin{table}[]
    \centering
    % [inline block 48: 2 envs, 4513 chars -> data_tex | \begin{tabular}{cc|cc|cc|cc|cc}     \multicolumn{2}{c|}{\includegraphics[width = 0.16\columnwidth]{assets/05-All-BoxPlot...]


    \caption{Guideline 1's t-test results %(\checkmark if Welch's t-test) 
    for comprehensive information processors vs. selective information processors participants' average ratings of the independent Violation AI product (top) and Application AI product (bottom), for all 10 dependent variables.
    If dashes (- - -) are present, no statistical test was performed.
    If the number of tests exceeded 5 for each product, Bonferroni correction applied by multiplying p-values by the number of tests performed.
    }
    \label{tab:G1-Info-Stats-Appendix}
    
    % \FIXME{MMB@AAA: FYI, I took the \checkmark s out and replaced them with plain text, because the \checkmark vs blank visually stood out so much, I kept mis-seeing it as saying only those 4 rows were signif. or important.\\
    % AAA@MMB: Redid it with Y/N. The Welch's t and t were cluttering up the table too much.\\
    % MMB@AAA: I actually prefer the spelled-out way.  Visually, the table layout now screams WELCHES IS GOOD, and draws attention away from all other columns.  Meta-comment: it might help if you forced yourself to look at this paper with a reader hat on.}

\end{table}

\clearpage
%---------------------------------------------------- End Guideline 1

%Guideline 3 ------------------------------
\begin{table}[]
    \centering
    % [inline block 49: 2 envs, 4519 chars -> data_tex | \begin{tabular}{cc|cc|cc|cc|cc}     \multicolumn{2}{c|}{\includegraphics[width = 0.16\columnwidth]{assets/05-All-BoxPlot...]


    \caption{Guideline 3's t-test results %(\checkmark if Welch's t-test) 
    for comprehensive information processors vs. selective information processors participants' average ratings of the independent Violation AI product (top) and Application AI product (bottom), for all 10 dependent variables.
    If dashes (- - -) are present, no statistical test was performed.
    If the number of tests exceeded 5 for each product, Bonferroni correction applied by multiplying p-values by the number of tests performed.
    }
    \label{tab:G3-Info-Stats-Appendix}
    
    % \FIXME{MMB@AAA: FYI, I took the \checkmark s out and replaced them with plain text, because the \checkmark vs blank visually stood out so much, I kept mis-seeing it as saying only those 4 rows were signif. or important.\\
    % AAA@MMB: Redid it with Y/N. The Welch's t and t were cluttering up the table too much.\\
    % MMB@AAA: I actually prefer the spelled-out way.  Visually, the table layout now screams WELCHES IS GOOD, and draws attention away from all other columns.  Meta-comment: it might help if you forced yourself to look at this paper with a reader hat on.}

\end{table}

\clearpage
%---------------------------------------------------- End Guideline 3

%Begin Guideline 4----------------------------------------------------

\begin{table}[]
    \centering
    % [inline block 50: 2 envs, 4532 chars -> data_tex | \begin{tabular}{cc|cc|cc|cc|cc}     \multicolumn{2}{c|}{\includegraphics[width = 0.16\columnwidth]{assets/05-All-BoxPlot...]


    \caption{Guideline 4's t-test results %(\checkmark if Welch's t-test) 
    for comprehensive information processors vs. selective information processors participants' average ratings of the independent Violation AI product (top) and Application AI product (bottom), for all 10 dependent variables.
    If dashes (- - -) are present, no statistical test was performed.
    If the number of tests exceeded 5 for each product, Bonferroni correction applied by multiplying p-values by the number of tests performed.
    }
    \label{tab:G4-Info-Stats-Appendix}
\end{table}

%---------------------------------------------------- End Guideline 4

\clearpage

%Begin Guideline 5----------------------------------------------------

\begin{table}[]
    \centering
    % [inline block 51: 2 envs, 4481 chars -> data_tex | \begin{tabular}{cc|cc|cc|cc|cc}     \multicolumn{2}{c|}{\includegraphics[width = 0.16\columnwidth]{assets/05-All-BoxPlot...]


    \caption{Guideline 5's t-test results %(\checkmark if Welch's t-test) 
    for comprehensive information processors vs. selective information processors participants' average ratings of the independent Violation AI product (top) and Application AI product (bottom), for all 10 dependent variables.
    If dashes (- - -) are present, no statistical test was performed.
    If the number of tests exceeded 5 for each product, Bonferroni correction applied by multiplying p-values by the number of tests performed.
    }
    \label{tab:G5-Info-Stats-Appendix}
\end{table}

%---------------------------------------------------- End Guideline 5

\clearpage

%Begin Guideline 6----------------------------------------------------

\begin{table}[]
    \centering
    % [inline block 52: 2 envs, 4485 chars -> data_tex | \begin{tabular}{cc|cc|cc|cc|cc}     \multicolumn{2}{c|}{\includegraphics[width = 0.16\columnwidth]{assets/05-All-BoxPlot...]


    \caption{Guideline 6's t-test results %(\checkmark if Welch's t-test) 
    for comprehensive information processors vs. selective information processors participants' average ratings of the independent Violation AI product (top) and Application AI product (bottom), for all 10 dependent variables.
    If dashes (- - -) are present, no statistical test was performed.
    If the number of tests exceeded 5 for each product, Bonferroni correction applied by multiplying p-values by the number of tests performed.
    }
    \label{tab:G6-Info-Stats-Appendix}
\end{table}

%---------------------------------------------------- End Guideline 6

\clearpage

%Begin Guideline 7----------------------------------------------------

\begin{table}[]
    \centering
    % [inline block 53: 2 envs, 4513 chars -> data_tex | \begin{tabular}{cc|cc|cc|cc|cc}     \multicolumn{2}{c|}{\includegraphics[width = 0.16\columnwidth]{assets/05-All-BoxPlot...]


    \caption{Guideline 7's t-test results %(\checkmark if Welch's t-test) 
    for comprehensive information processors vs. selective information processors participants' average ratings of the independent Violation AI product (top) and Application AI product (bottom), for all 10 dependent variables.
    If dashes (- - -) are present, no statistical test was performed.
    If the number of tests exceeded 5 for each product, Bonferroni correction applied by multiplying p-values by the number of tests performed.
    }
    \label{tab:G7-Info-Stats-Appendix}
\end{table}

%---------------------------------------------------- End Guideline 7

\clearpage

%Begin Guideline 8----------------------------------------------------

\begin{table}[]
    \centering
    % [inline block 54: 2 envs, 4625 chars -> data_tex | \begin{tabular}{cc|cc|cc|cc|cc}     \multicolumn{2}{c|}{\includegraphics[width = 0.16\columnwidth]{assets/05-All-BoxPlot...]


    \caption{Guideline 8's t-test results %(\checkmark if Welch's t-test) 
    for comprehensive information processors vs. selective information processors participants' average ratings of the independent Violation AI product (top) and Application AI product (bottom), for all 10 dependent variables.
    If dashes (- - -) are present, no statistical test was performed.
    If the number of tests exceeded 5 for each product, Bonferroni correction applied by multiplying p-values by the number of tests performed.
    }
    \label{tab:G8-Info-Stats-Appendix}
\end{table}
\clearpage
%---------------------------------------------------- End Guideline 8

%Begin Guideline 9----------------------------------------------------

\begin{table}[]
    \centering
    % [inline block 55: 2 envs, 4478 chars -> data_tex | \begin{tabular}{cc|cc|cc|cc|cc}     \multicolumn{2}{c|}{\includegraphics[width = 0.16\columnwidth]{assets/05-All-BoxPlot...]


    \caption{Guideline 9's t-test results %(\checkmark if Welch's t-test) 
    for comprehensive information processors vs. selective information processors participants' average ratings of the independent Violation AI product (top) and Application AI product (bottom), for all 10 dependent variables.
    If dashes (- - -) are present, no statistical test was performed.
    If the number of tests exceeded 5 for each product, Bonferroni correction applied by multiplying p-values by the number of tests performed.
    }
    \label{tab:G9-Info-Stats-Appendix}
\end{table}
\clearpage
%---------------------------------------------------- End Guideline 9

%Begin Guideline 10----------------------------------------------------

\begin{table}[]
    \centering
    % [inline block 56: 2 envs, 4528 chars -> data_tex | \begin{tabular}{cc|cc|cc|cc|cc}     \multicolumn{2}{c|}{\includegraphics[width = 0.16\columnwidth]{assets/05-All-BoxPlot...]


    \caption{Guideline 10's t-test results %(\checkmark if Welch's t-test) 
    for comprehensive information processors vs. selective information processors participants' average ratings of the independent Violation AI product (top) and Application AI product (bottom), for all 10 dependent variables.
    If dashes (- - -) are present, no statistical test was performed.
    If the number of tests exceeded 5 for each product, Bonferroni correction applied by multiplying p-values by the number of tests performed.
    }
    \label{tab:G10-Info-Stats-Appendix}
\end{table}
\clearpage
%---------------------------------------------------- End Guideline 10

%Begin Guideline 11----------------------------------------------------

\begin{table}[]
    \centering
    % [inline block 57: 2 envs, 4532 chars -> data_tex | \begin{tabular}{cc|cc|cc|cc|cc}     \multicolumn{2}{c|}{\includegraphics[width = 0.16\columnwidth]{assets/05-All-BoxPlot...]


    \caption{Guideline 11's t-test results %(\checkmark if Welch's t-test) 
    for comprehensive information processors vs. selective information processors participants' average ratings of the independent Violation AI product (top) and Application AI product (bottom), for all 10 dependent variables.
    If dashes (- - -) are present, no statistical test was performed.
    If the number of tests exceeded 5 for each product, Bonferroni correction applied by multiplying p-values by the number of tests performed.
    }
    \label{tab:G11-Info-Stats-Appendix}
\end{table}
\clearpage
%---------------------------------------------------- End Guideline 11

%Begin Guideline 12----------------------------------------------------

\begin{table}[]
    \centering
    % [inline block 58: 2 envs, 4542 chars -> data_tex | \begin{tabular}{cc|cc|cc|cc|cc}     \multicolumn{2}{c|}{\includegraphics[width = 0.16\columnwidth]{assets/05-All-BoxPlot...]


    \caption{Guideline 12's t-test results %(\checkmark if Welch's t-test) 
    for comprehensive information processors vs. selective information processors participants' average ratings of the independent Violation AI product (top) and Application AI product (bottom), for all 10 dependent variables.
    If dashes (- - -) are present, no statistical test was performed.
    If the number of tests exceeded 5 for each product, Bonferroni correction applied by multiplying p-values by the number of tests performed.
    }
    \label{tab:G12-Info-Stats-Appendix}
\end{table}
\clearpage
%---------------------------------------------------- End Guideline 12

%Begin Guideline 13----------------------------------------------------

\begin{table}[]
    \centering
    % [inline block 59: 2 envs, 4540 chars -> data_tex | \begin{tabular}{cc|cc|cc|cc|cc}     \multicolumn{2}{c|}{\includegraphics[width = 0.16\columnwidth]{assets/05-All-BoxPlot...]


    \caption{Guideline 13's t-test results %(\checkmark if Welch's t-test) 
    for comprehensive information processors vs. selective information processors participants' average ratings of the independent Violation AI product (top) and Application AI product (bottom), for all 10 dependent variables.
    If dashes (- - -) are present, no statistical test was performed.
    If the number of tests exceeded 5 for each product, Bonferroni correction applied by multiplying p-values by the number of tests performed.
    }
    \label{tab:G13-Info-Stats-Appendix}
\end{table}
\clearpage
%---------------------------------------------------- End Guideline 13

%Begin Guideline 14---------------------------------------------------

\begin{table}[]
    \centering
    % [inline block 60: 2 envs, 4532 chars -> data_tex | \begin{tabular}{cc|cc|cc|cc|cc}     \multicolumn{2}{c|}{\includegraphics[width = 0.16\columnwidth]{assets/05-All-BoxPlot...]


    \caption{Guideline 14's t-test results %(\checkmark if Welch's t-test) 
    for comprehensive information processors vs. selective information processors participants' average ratings of the independent Violation AI product (top) and Application AI product (bottom), for all 10 dependent variables.
    If dashes (- - -) are present, no statistical test was performed.
    If the number of tests exceeded 5 for each product, Bonferroni correction applied by multiplying p-values by the number of tests performed.
    }
    \label{tab:G14-Info-Stats-Appendix}
\end{table}
\clearpage
%---------------------------------------------------- End Guideline 14

%Begin Guideline 15---------------------------------------------------

\begin{table}[]
    \centering
    % [inline block 61: 2 envs, 4661 chars -> data_tex | \begin{tabular}{cc|cc|cc|cc|cc}     \multicolumn{2}{c|}{\includegraphics[width = 0.16\columnwidth]{assets/05-All-BoxPlot...]


    \caption{Guideline 15's t-test results %(\checkmark if Welch's t-test) 
    for comprehensive information processors vs. selective information processors participants' average ratings of the independent Violation AI product (top) and Application AI product (bottom), for all 10 dependent variables.
    If dashes (- - -) are present, no statistical test was performed.
    If the number of tests exceeded 5 for each product, Bonferroni correction applied by multiplying p-values by the number of tests performed.
    }
    \label{tab:G15-Info-Stats-Appendix}
\end{table}
\clearpage
%---------------------------------------------------- End Guideline 15

%Begin Guideline 17---------------------------------------------------

\begin{table}[]
    \centering
    % [inline block 62: 2 envs, 4520 chars -> data_tex | \begin{tabular}{cc|cc|cc|cc|cc}     \multicolumn{2}{c|}{\includegraphics[width = 0.16\columnwidth]{assets/05-All-BoxPlot...]


    \caption{Guideline 17's t-test results %(\checkmark if Welch's t-test) 
    for comprehensive information processors vs. selective information processors participants' average ratings of the independent Violation AI product (top) and Application AI product (bottom), for all 10 dependent variables.
    If dashes (- - -) are present, no statistical test was performed.
    If the number of tests exceeded 5 for each product, Bonferroni correction applied by multiplying p-values by the number of tests performed.
    }
    \label{tab:G17-Info-Stats-Appendix}
\end{table}
\clearpage
%---------------------------------------------------- End Guideline 17

%Begin Guideline 17---------------------------------------------------

\begin{table}[]
    \centering
    % [inline block 63: 2 envs, 4507 chars -> data_tex | \begin{tabular}{cc|cc|cc|cc|cc}     \multicolumn{2}{c|}{\includegraphics[width = 0.16\columnwidth]{assets/05-All-BoxPlot...]


    \caption{Guideline 18's t-test results %(\checkmark if Welch's t-test) 
    for comprehensive information processors vs. selective information processors participants' average ratings of the independent Violation AI product (top) and Application AI product (bottom), for all 10 dependent variables.
    If dashes (- - -) are present, no statistical test was performed.
    If the number of tests exceeded 5 for each product, Bonferroni correction applied by multiplying p-values by the number of tests performed.
    }
    \label{tab:G18-Info-Stats-Appendix}
\end{table}
\clearpage
%---------------------------------------------------- End Guideline 18
\clearpage

%Guideline 1 ------------------------------
\begin{table}[]
    \centering
    % [inline block 64: 2 envs, 4518 chars -> data_tex | \begin{tabular}{cc|cc|cc|cc|cc}     \multicolumn{2}{c|}{\includegraphics[width = 0.16\columnwidth]{assets/05-All-BoxPlot...]


    \caption{Guideline 1's t-test results %(\checkmark if Welch's t-test) 
    for lower self-efficacy vs. higher self-efficacy participants' average ratings of the independent Violation AI product (top) and Application AI product (bottom), for all 10 dependent variables.
    If dashes (- - -) are present, no statistical test was performed.
    If the number of tests exceeded 5 for each product, Bonferroni correction applied by multiplying p-values by the number of tests performed.
    }
    \label{tab:G1-SE-Stats-Appendix}
    
    % \FIXME{MMB@AAA: FYI, I took the \checkmark s out and replaced them with plain text, because the \checkmark vs blank visually stood out so much, I kept mis-seeing it as saying only those 4 rows were signif. or important.\\
    % AAA@MMB: Redid it with Y/N. The Welch's t and t were cluttering up the table too much.\\
    % MMB@AAA: I actually prefer the spelled-out way.  Visually, the table layout now screams WELCHES IS GOOD, and draws attention away from all other columns.  Meta-comment: it might help if you forced yourself to look at this paper with a reader hat on.}

\end{table}

\clearpage
%---------------------------------------------------- End Guideline 1

%Guideline 3 ------------------------------
\begin{table}[]
    \centering
    % [inline block 65: 2 envs, 4488 chars -> data_tex | \begin{tabular}{cc|cc|cc|cc|cc}     \multicolumn{2}{c|}{\includegraphics[width = 0.16\columnwidth]{assets/05-All-BoxPlot...]


    \caption{Guideline 3's t-test results %(\checkmark if Welch's t-test) 
    for lower self-efficacy vs. higher self-efficacy participants' average ratings of the independent Violation AI product (top) and Application AI product (bottom), for all 10 dependent variables.
    If dashes (- - -) are present, no statistical test was performed.
    If the number of tests exceeded 5 for each product, Bonferroni correction applied by multiplying p-values by the number of tests performed.
    }
    \label{tab:G3-SE-Stats-Appendix}
    
    % \FIXME{MMB@AAA: FYI, I took the \checkmark s out and replaced them with plain text, because the \checkmark vs blank visually stood out so much, I kept mis-seeing it as saying only those 4 rows were signif. or important.\\
    % AAA@MMB: Redid it with Y/N. The Welch's t and t were cluttering up the table too much.\\
    % MMB@AAA: I actually prefer the spelled-out way.  Visually, the table layout now screams WELCHES IS GOOD, and draws attention away from all other columns.  Meta-comment: it might help if you forced yourself to look at this paper with a reader hat on.}

\end{table}

\clearpage
%---------------------------------------------------- End Guideline 3

%Begin Guideline 4----------------------------------------------------

\begin{table}[]
    \centering
    % [inline block 66: 2 envs, 4487 chars -> data_tex | \begin{tabular}{cc|cc|cc|cc|cc}     \multicolumn{2}{c|}{\includegraphics[width = 0.16\columnwidth]{assets/05-All-BoxPlot...]


    \caption{Guideline 4's t-test results %(\checkmark if Welch's t-test) 
    for lower self-efficacy vs. higher self-efficacy participants' average ratings of the independent Violation AI product (top) and Application AI product (bottom), for all 10 dependent variables.
    If dashes (- - -) are present, no statistical test was performed.
    If the number of tests exceeded 5 for each product, Bonferroni correction applied by multiplying p-values by the number of tests performed.
    }
    \label{tab:G4-SE-Stats-Appendix}
\end{table}

%---------------------------------------------------- End Guideline 4

\clearpage

%Begin Guideline 5----------------------------------------------------

\begin{table}[]
    \centering
    % [inline block 67: 2 envs, 4673 chars -> data_tex | \begin{tabular}{cc|cc|cc|cc|cc}     \multicolumn{2}{c|}{\includegraphics[width = 0.16\columnwidth]{assets/05-All-BoxPlot...]


    \caption{Guideline 5's t-test results %(\checkmark if Welch's t-test) 
    for lower self-efficacy vs. higher self-efficacy participants' average ratings of the independent Violation AI product (top) and Application AI product (bottom), for all 10 dependent variables.
    If dashes (- - -) are present, no statistical test was performed.
    If the number of tests exceeded 5 for each product, Bonferroni correction applied by multiplying p-values by the number of tests performed.
    }
    \label{tab:G5-SE-Stats-Appendix}
\end{table}

%---------------------------------------------------- End Guideline 5

\clearpage

%Begin Guideline 6----------------------------------------------------

\begin{table}[]
    \centering
    % [inline block 68: 2 envs, 4445 chars -> data_tex | \begin{tabular}{cc|cc|cc|cc|cc}     \multicolumn{2}{c|}{\includegraphics[width = 0.16\columnwidth]{assets/05-All-BoxPlot...]


    \caption{Guideline 6's t-test results %(\checkmark if Welch's t-test) 
    for lower self-efficacy vs. higher self-efficacy participants' average ratings of the independent Violation AI product (top) and Application AI product (bottom), for all 10 dependent variables.
    If dashes (- - -) are present, no statistical test was performed.
    If the number of tests exceeded 5 for each product, Bonferroni correction applied by multiplying p-values by the number of tests performed.
    }
    \label{tab:G6-SE-Stats-Appendix}
\end{table}

%---------------------------------------------------- End Guideline 6

\clearpage

%Begin Guideline 7----------------------------------------------------

\begin{table}[]
    \centering
    % [inline block 69: 2 envs, 4466 chars -> data_tex | \begin{tabular}{cc|cc|cc|cc|cc}     \multicolumn{2}{c|}{\includegraphics[width = 0.16\columnwidth]{assets/05-All-BoxPlot...]


    \caption{Guideline 7's t-test results %(\checkmark if Welch's t-test) 
    for lower self-efficacy vs. higher self-efficacy participants' average ratings of the independent Violation AI product (top) and Application AI product (bottom), for all 10 dependent variables.
    If dashes (- - -) are present, no statistical test was performed.
    If the number of tests exceeded 5 for each product, Bonferroni correction applied by multiplying p-values by the number of tests performed.
    }
    \label{tab:G7-SE-Stats-Appendix}
\end{table}

%---------------------------------------------------- End Guideline 7

\clearpage

%Begin Guideline 8----------------------------------------------------

\begin{table}[]
    \centering
    % [inline block 70: 2 envs, 4429 chars -> data_tex | \begin{tabular}{cc|cc|cc|cc|cc}     \multicolumn{2}{c|}{\includegraphics[width = 0.16\columnwidth]{assets/05-All-BoxPlot...]


    \caption{Guideline 8's t-test results %(\checkmark if Welch's t-test) 
    for lower self-efficacy vs. higher self-efficacy participants' average ratings of the independent Violation AI product (top) and Application AI product (bottom), for all 10 dependent variables.
    If dashes (- - -) are present, no statistical test was performed.
    If the number of tests exceeded 5 for each product, Bonferroni correction applied by multiplying p-values by the number of tests performed.
    }
    \label{tab:G8-SE-Stats-Appendix}
\end{table}
\clearpage
%---------------------------------------------------- End Guideline 8

%Begin Guideline 9----------------------------------------------------

\begin{table}[]
    \centering
    % [inline block 71: 2 envs, 4520 chars -> data_tex | \begin{tabular}{cc|cc|cc|cc|cc}     \multicolumn{2}{c|}{\includegraphics[width = 0.16\columnwidth]{assets/05-All-BoxPlot...]


    \caption{Guideline 9's t-test results %(\checkmark if Welch's t-test) 
    for lower self-efficacy vs. higher self-efficacy participants' average ratings of the independent Violation AI product (top) and Application AI product (bottom), for all 10 dependent variables.
    If dashes (- - -) are present, no statistical test was performed.
    If the number of tests exceeded 5 for each product, Bonferroni correction applied by multiplying p-values by the number of tests performed.
    }
    \label{tab:G9-SE-Stats-Appendix}
\end{table}
\clearpage
%---------------------------------------------------- End Guideline 9

%Begin Guideline 10----------------------------------------------------

\begin{table}[]
    \centering
    % [inline block 72: 2 envs, 4485 chars -> data_tex | \begin{tabular}{cc|cc|cc|cc|cc}     \multicolumn{2}{c|}{\includegraphics[width = 0.16\columnwidth]{assets/05-All-BoxPlot...]


    \caption{Guideline 10's t-test results %(\checkmark if Welch's t-test) 
    for lower self-efficacy vs. higher self-efficacy participants' average ratings of the independent Violation AI product (top) and Application AI product (bottom), for all 10 dependent variables.
    If dashes (- - -) are present, no statistical test was performed.
    If the number of tests exceeded 5 for each product, Bonferroni correction applied by multiplying p-values by the number of tests performed.
    }
    \label{tab:G10-SE-Stats-Appendix}
\end{table}
\clearpage
%---------------------------------------------------- End Guideline 10

%Begin Guideline 11----------------------------------------------------

\begin{table}[]
    \centering
    % [inline block 73: 2 envs, 4455 chars -> data_tex | \begin{tabular}{cc|cc|cc|cc|cc}     \multicolumn{2}{c|}{\includegraphics[width = 0.16\columnwidth]{assets/05-All-BoxPlot...]


    \caption{Guideline 11's t-test results %(\checkmark if Welch's t-test) 
    for lower self-efficacy vs. higher self-efficacy participants' average ratings of the independent Violation AI product (top) and Application AI product (bottom), for all 10 dependent variables.
    If dashes (- - -) are present, no statistical test was performed.
    If the number of tests exceeded 5 for each product, Bonferroni correction applied by multiplying p-values by the number of tests performed.
    }
    \label{tab:G11-SE-Stats-Appendix}
\end{table}
\clearpage
%---------------------------------------------------- End Guideline 11

%Begin Guideline 12----------------------------------------------------

\begin{table}[]
    \centering
    % [inline block 74: 2 envs, 4457 chars -> data_tex | \begin{tabular}{cc|cc|cc|cc|cc}     \multicolumn{2}{c|}{\includegraphics[width = 0.16\columnwidth]{assets/05-All-BoxPlot...]


    \caption{Guideline 12's t-test results %(\checkmark if Welch's t-test) 
    for lower self-efficacy vs. higher self-efficacy participants' average ratings of the independent Violation AI product (top) and Application AI product (bottom), for all 10 dependent variables.
    If dashes (- - -) are present, no statistical test was performed.
    If the number of tests exceeded 5 for each product, Bonferroni correction applied by multiplying p-values by the number of tests performed.
    }
    \label{tab:G12-SE-Stats-Appendix}
\end{table}
\clearpage
%---------------------------------------------------- End Guideline 12

%Begin Guideline 13----------------------------------------------------

\begin{table}[]
    \centering
    % [inline block 75: 2 envs, 4787 chars -> data_tex | \begin{tabular}{cc|cc|cc|cc|cc}     \multicolumn{2}{c|}{\includegraphics[width = 0.16\columnwidth]{assets/05-All-BoxPlot...]


    \caption{Guideline 13's t-test results %(\checkmark if Welch's t-test) 
    for lower self-efficacy vs. higher self-efficacy participants' average ratings of the independent Violation AI product (top) and Application AI product (bottom), for all 10 dependent variables.
    If dashes (- - -) are present, no statistical test was performed.
    If the number of tests exceeded 5 for each product, Bonferroni correction applied by multiplying p-values by the number of tests performed.
    }
    \label{tab:G13-SE-Stats-Appendix}
\end{table}
\clearpage
%---------------------------------------------------- End Guideline 13

%Begin Guideline 14---------------------------------------------------

\begin{table}[]
    \centering
    % [inline block 76: 2 envs, 4519 chars -> data_tex | \begin{tabular}{cc|cc|cc|cc|cc}     \multicolumn{2}{c|}{\includegraphics[width = 0.16\columnwidth]{assets/05-All-BoxPlot...]


    \caption{Guideline 14's t-test results %(\checkmark if Welch's t-test) 
    for lower self-efficacy vs. higher self-efficacy participants' average ratings of the independent Violation AI product (top) and Application AI product (bottom), for all 10 dependent variables.
    If dashes (- - -) are present, no statistical test was performed.
    If the number of tests exceeded 5 for each product, Bonferroni correction applied by multiplying p-values by the number of tests performed.
    }
    \label{tab:G14-SE-Stats-Appendix}
\end{table}
\clearpage
%---------------------------------------------------- End Guideline 14

%Begin Guideline 15---------------------------------------------------

\begin{table}[]
    \centering
    % [inline block 77: 2 envs, 4474 chars -> data_tex | \begin{tabular}{cc|cc|cc|cc|cc}     \multicolumn{2}{c|}{\includegraphics[width = 0.16\columnwidth]{assets/05-All-BoxPlot...]


    \caption{Guideline 15's t-test results %(\checkmark if Welch's t-test) 
    for lower self-efficacy vs. higher self-efficacy participants' average ratings of the independent Violation AI product (top) and Application AI product (bottom), for all 10 dependent variables.
    If dashes (- - -) are present, no statistical test was performed.
    If the number of tests exceeded 5 for each product, Bonferroni correction applied by multiplying p-values by the number of tests performed.
    }
    \label{tab:G15-SE-Stats-Appendix}
\end{table}
\clearpage
%---------------------------------------------------- End Guideline 15

%Begin Guideline 17---------------------------------------------------

\begin{table}[]
    \centering
    % [inline block 78: 2 envs, 4457 chars -> data_tex | \begin{tabular}{cc|cc|cc|cc|cc}     \multicolumn{2}{c|}{\includegraphics[width = 0.16\columnwidth]{assets/05-All-BoxPlot...]


    \caption{Guideline 17's t-test results %(\checkmark if Welch's t-test) 
    for lower self-efficacy vs. higher self-efficacy participants' average ratings of the independent Violation AI product (top) and Application AI product (bottom), for all 10 dependent variables.
    If dashes (- - -) are present, no statistical test was performed.
    If the number of tests exceeded 5 for each product, Bonferroni correction applied by multiplying p-values by the number of tests performed.
    }
    \label{tab:G17-SE-Stats-Appendix}
\end{table}
\clearpage
%---------------------------------------------------- End Guideline 17

%Begin Guideline 17---------------------------------------------------

\begin{table}[]
    \centering
    % [inline block 79: 2 envs, 4736 chars -> data_tex | \begin{tabular}{cc|cc|cc|cc|cc}     \multicolumn{2}{c|}{\includegraphics[width = 0.16\columnwidth]{assets/05-All-BoxPlot...]


    \caption{Guideline 18's t-test results %(\checkmark if Welch's t-test) 
    for lower self-efficacy vs. higher self-efficacy participants' average ratings of the independent Violation AI product (top) and Application AI product (bottom), for all 10 dependent variables.
    If dashes (- - -) are present, no statistical test was performed.
    If the number of tests exceeded 5 for each product, Bonferroni correction applied by multiplying p-values by the number of tests performed.
    }
    \label{tab:G18-SE-Stats-Appendix}
\end{table}
\clearpage
%---------------------------------------------------- End Guideline 18
\clearpage

%---------------------

%---------------------
