# Supplementary material for: Measuring User Experience Inclusivity in Human-AI Interaction via Five User Problem-Solving Styles
Source: arXiv:2108.00588 source file (2024-02-17)
Supplement: Supplementary file 5 [file Appendix-FacetSurvey.tex]

\section{Facet Survey}
\label{sec:appendix-facets}
\begin{figure}[b!]
    \centering
    \includegraphics[width = \columnwidth]{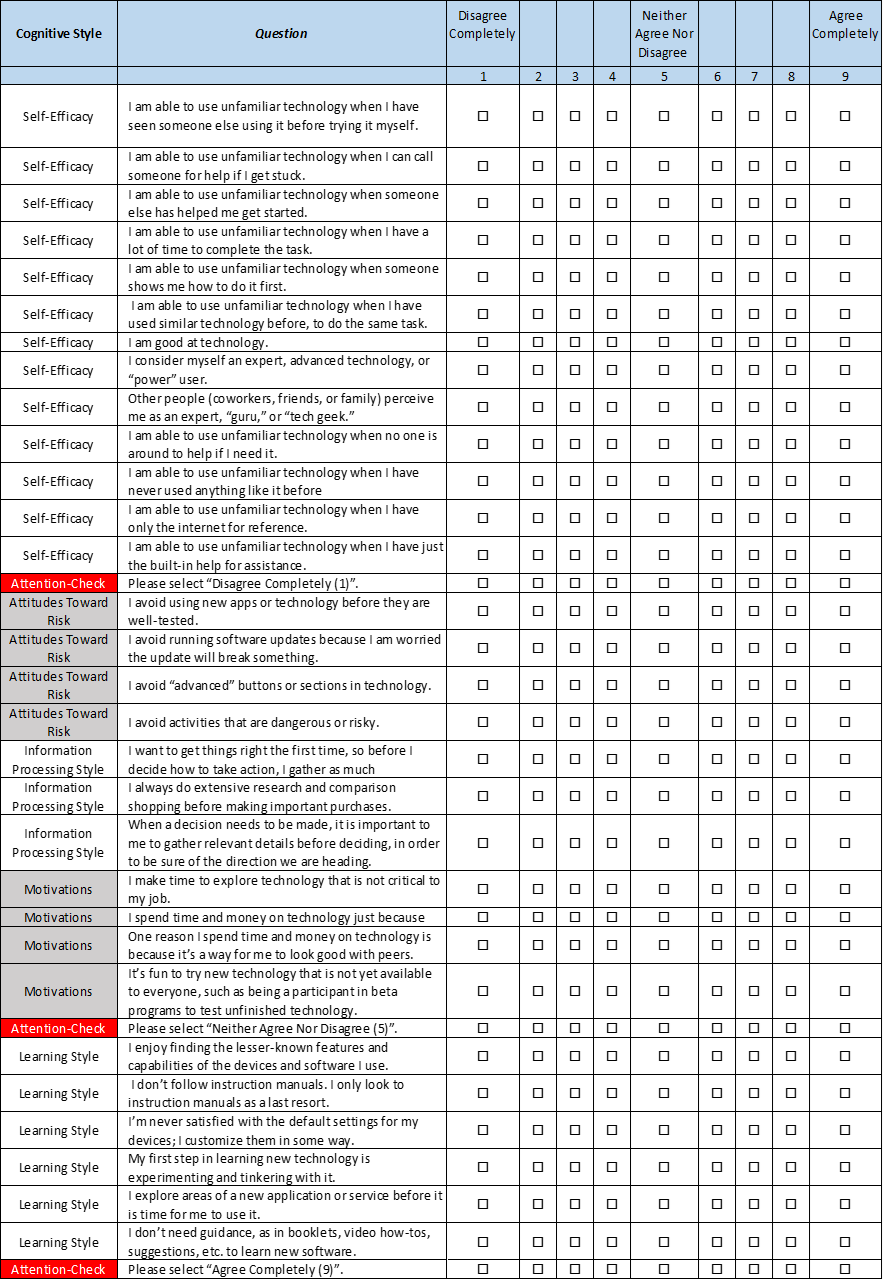}
\end{figure}
% \begin{figure}[b!]
%     \centering
%     \includegraphics[width = \columnwidth]{assets/Facet-Survey-P2.png}
% \end{figure}
% \begin{figure}[b!]
%     \centering
%     \includegraphics[width = \columnwidth]{assets/Facet-Survey-P3.pdf}
% \end{figure}
\begin{figure}[b!]
    \centering
    \includegraphics[width = \columnwidth]{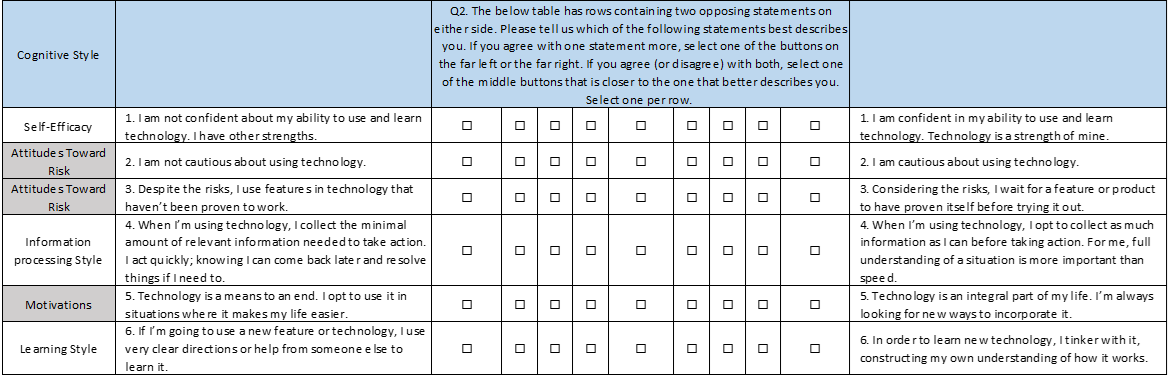}
    \label{fig:facet-survey}
    \caption{The GenderMag problem solving style survey.
            The left-most column shows which of the styles each question relates to, as well as the 3 attention check questions.
            On the first page, people respond from "strongly disagree" to "strongly agree."
            On the second page, people responses relate to which end of the question they align with more.}
\end{figure}
% \FIXME{include the 36-question survey used}

% \FIXME{MMB to anyone: \\
% PROBLEM: in the body of hte text, we say 36 questions. We say it here in the caption too.  But the numbering goes up into the 40s.  
% \\SOLUTION: (1) count them up to make sure it's really 36. (2) explain in the caption that it's really 36, and say why the numbers are so weird. (?probably has to do with numbering of internal answer key, or random attention check questions, etc?)}

\clearpage
