# Supplementary material for: Measuring User Experience Inclusivity in Human-AI Interaction via Five User Problem-Solving Styles
Source: arXiv:2108.00588 source file (2024-02-17)
Supplement: Supplementary file 6 [file Appendix-GM-Rules.tex]

\section{GenderMag Problem Solving Style Spectra Classification Rules}
\label{app:GM-Rules}

\begin{table}[h]
    \centering
    \begin{tabular}{p{0.3\linewidth}|c|c|c}
%         & \textbf{Inequality:} &  &  \\
       \textbf{problem solving style} & \textbf{Comparison} & \textbf{If True: } &\textbf{If False: }\\
       \hline
        Attitudes Toward Risk & $>$ median & \cellcolor{AbiOrangeQuote} more risk-averse & \cellcolor{TimBlueQuote} more risk-tolerant \\
        \hline
        Computer Self-Efficacy & $<$ median & \cellcolor{AbiOrangeQuote} lower & \cellcolor{TimBlueQuote} higher \\
        \hline
        Information Processing Style & $>$ median & \cellcolor{AbiOrangeQuote} more comprehensive & \cellcolor{TimBlueQuote} more selective \\
        \hline
        Motivations & $<$ median & \cellcolor{AbiOrangeQuote} more for task & \cellcolor{TimBlueQuote} more for fun \\
        \hline
        Learning Style & $<$ median & \cellcolor{AbiOrangeQuote} more by process & \cellcolor{TimBlueQuote} more by tinkering \\
    \end{tabular}
    \caption{The rules for each problem solving style spectrum, used to categorize which style participants exhibited from their survey responses, relative to other participants.}
    \label{tab:style_rules}
\end{table}
