# Supplementary material for: Measuring User Experience Inclusivity in Human-AI Interaction via Five User Problem-Solving Styles
Source: arXiv:2108.00588 source file (2024-02-17)
Supplement: Supplementary file 7 [file Facet-Survey.tex]

\begin{figure}[b!]
    \centering
    \includegraphics[width = \columnwidth]{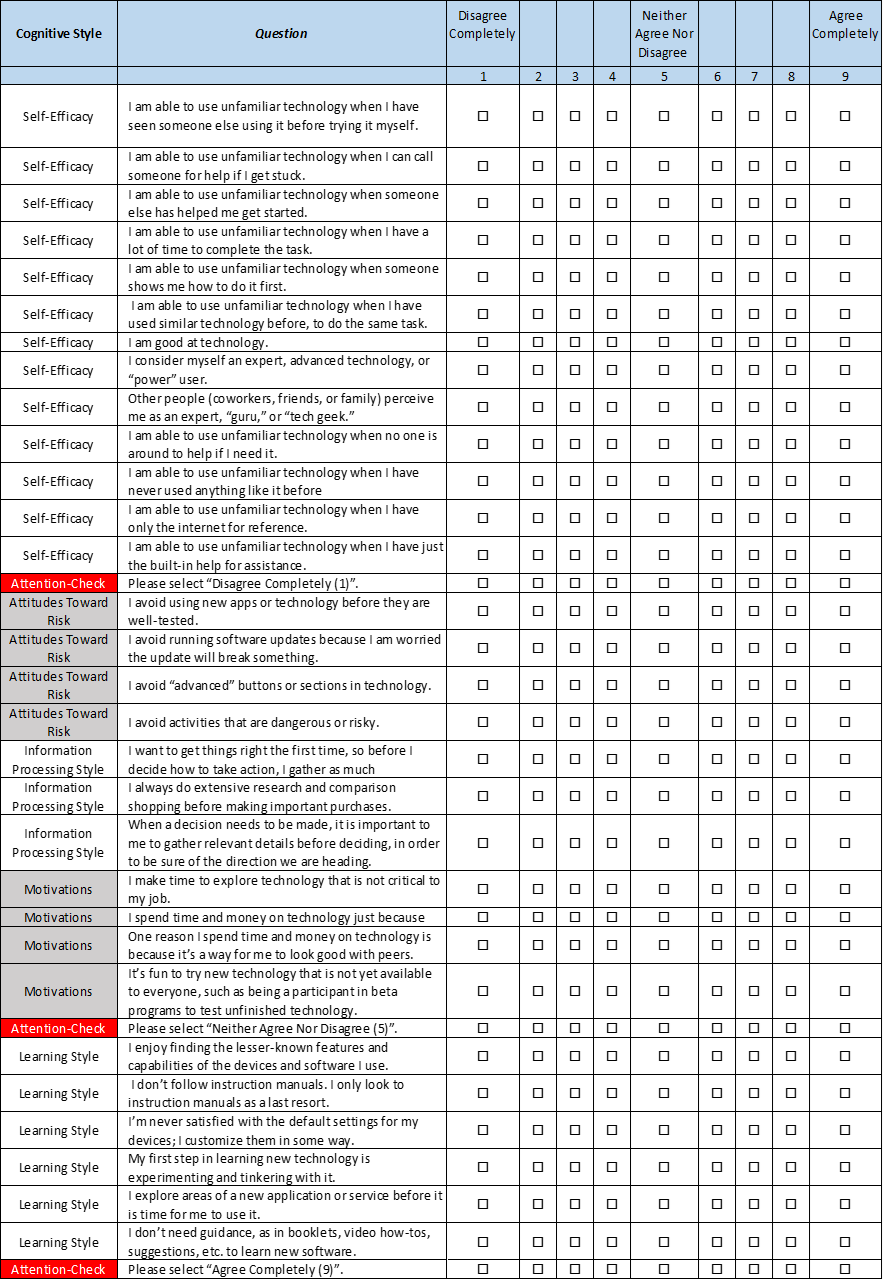}
\end{figure}
% \begin{figure}[b!]
%     \centering
%     \includegraphics[width = \columnwidth]{assets/Facet-Survey-P2.png}
% \end{figure}
% \begin{figure}[b!]
%     \centering
%     \includegraphics[width = \columnwidth]{assets/Facet-Survey-P3.pdf}
% \end{figure}
\begin{figure}[b!]
    \centering
    \includegraphics[width = \columnwidth]{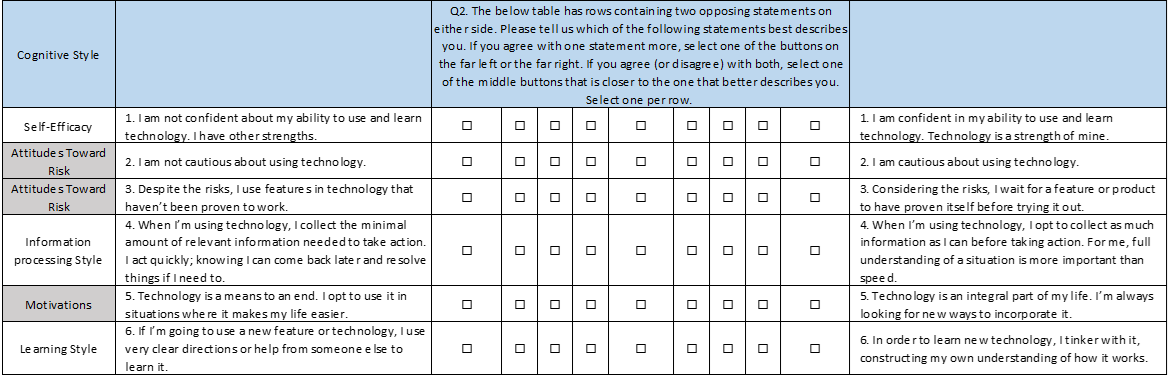}
    \label{fig:facet-survey}
    \caption{The GenderMag problem solving style survey.
            The left-most column shows which of the styles each question relates to, as well as the 3 attention check questions.
            On the first page, people respond from "strongly disagree" to "strongly agree."
            On the second page, people responses relate to which end of the question they align with more.}
\end{figure}
