# Supplementary material for: Measuring User Experience Inclusivity in Human-AI Interaction via Five User Problem-Solving Styles
Source: arXiv:2108.00588 source file (2024-02-17)
Supplement: Supplementary file 8 [file Info-Appendix.tex]

%Guideline 1 ------------------------------
\begin{table}[]
    \centering
    \begin{tabular}{cc|cc|cc|cc|cc}
    \multicolumn{2}{c|}{\includegraphics[width = 0.16\columnwidth]{assets/05-All-BoxPlots/01-G1/Info/G1-Feel-In-Control-INFO.png}} &
    \multicolumn{2}{c|}{\includegraphics[width = 0.16\columnwidth]{assets/05-All-BoxPlots/01-G1/Info/G1-Feel-Secure-INFO.png}} &
    \multicolumn{2}{c|}{\includegraphics[width = 0.16\columnwidth]{assets/05-All-BoxPlots/01-G1/Info/G1-Feel-Adequate-INFO.png}} &
    \multicolumn{2}{c|}{\includegraphics[width = 0.16\columnwidth]{assets/05-All-BoxPlots/01-G1/Info/G1-Feel-Certain-INFO.png}} &
    \multicolumn{2}{c}{\includegraphics[width = 0.16\columnwidth]{assets/05-All-BoxPlots/01-G1/Info/G1-Feel-Productive-INFO.png}}
    \\
    \hline
    \hline
    \multicolumn{2}{c|}{\includegraphics[width = 0.16\columnwidth]{assets/05-All-BoxPlots/01-G1/Info/G1-Perceived-Useful-INFO.png}} &
    \multicolumn{2}{c|}{\includegraphics[width = 0.16\columnwidth]{assets/05-All-BoxPlots/01-G1/Info/G1-Not-Suspicious-INFO.png}} &
    \multicolumn{2}{c|}{\includegraphics[width = 0.16\columnwidth]{assets/05-All-BoxPlots/01-G1/Info/G1-Not-Harmful-INFO.png}} &
    \multicolumn{2}{c|}{\includegraphics[width = 0.16\columnwidth]{assets/05-All-BoxPlots/01-G1/Info/G1-Product-Reliable-INFO.png}} &
    \multicolumn{2}{c}{\includegraphics[width = 0.16\columnwidth]{assets/05-All-BoxPlots/01-G1/Info/G1-Trust-Product-INFO.png}}
    \end{tabular}
    
    \caption{Guideline 1 participants' ratings for all dependent variables, disaggregated by participants' information processing styles.
	%For the disaggregated data, notice how large the distances between the average rating are when the guideline is applied.
	Table~\ref{tab:G1-Info-Stats-Appendix} below provides the statistics (where applicable).
}
    \label{fig:Info-G1-Appendix}
\end{table}

\begin{table}[h]

%\framebox[\linewidth]{For Measuring!}
\centering
\footnotesize

    \begin{tabular}{p{0.22\columnwidth}|c|c|c|c|c|c}
    
    \rowcolor{LightGray}\multicolumn{7}{c}{\textbf{Violation AI Product}}\\
    \hline
    \textbf{Dependent}  & \textbf{Distance b/w} &  &  & & \textbf{Bonferroni} &  \\
    \textbf{variable} & \textbf{Means} &  \textbf{df} &  \textbf{t-val} &   \textbf{p-value}  & \textbf{correction} & \textbf{Cohen's \textit{d}} \\
    \hline
    
    I would feel in control & - - - & - &  - - - & - - - & - - - & - - -\\
    \hline
    
    I would feel secure & - - - & - &  - - - & - - - & - - - & - - - \\
    \hline
    
    I would feel adequate & 0.8016 & 53 &  1.8614 & .0682 & - - - & 0.5021 \\
    \hline
    
    I would feel certain & - - - & - &  - - - & - - - & - - - & - - - \\
    \hline
    
    I would feel productive & - - - & - &  - - - & - - - & - - - & - - -  \\
    \hline
    \hline
    
    I perceived it as useful &  - - - & - &  - - - & - - - & - - - & - - -  \\
    \hline
    
    I would not be suspicious & - - - & - &  - - - & - - - & - - - & - - -  \\
    \hline
    
    It would not be harmful & - - - & - &  - - - & - - - & - - - & - - -  \\
    \hline
    
    I find the product reliable & - - - & - &  - - - & - - - & - - - & - - -  \\
    \hline
    
    I would trust the product & - - - & - &  - - - & - - - & - - - & - - - \\
    \hline

    \rowcolor{LightGray}\multicolumn{7}{c}{\textbf{Application AI Product}}\\
    \hline
    \textbf{Dependent}  & \textbf{Distance b/w} &  &  & & \textbf{Bonferroni} &  \\
    \textbf{variable} & \textbf{Means} &  \textbf{df} &  \textbf{t-val} &   \textbf{p-value}  & \textbf{correction} & \textbf{Cohen's \textit{d}} \\
    \hline
    
    I would feel in control & - - - & - &  - - - & - - - & - - - & - - -  \\
    \hline
    
    I would feel secure & - - - & - &  - - - & - - - & - - - & - - - \\
    \hline
    
    I would feel adequate & 0.8812 & 54 &  2.1457 & \cellcolor{TimBlueQuote}.0364 & - - - & 0.5738 \\
    \hline
    
    I would feel certain & 0.7217 & 55 &  1.6246 & .1100 & - - - & 0.4304 \\
    \hline
    
    I would feel productive & - - - & - &  - - - & - - - & - - - & - - -   \\
    \hline
    \hline
    
    I perceived it as useful &  - - - & - &  - - - & - - - & - - - & - - -  \\
    \hline
    
    I would not be suspicious & - - - & - &  - - - & - - - & - - - & - - -  \\
    \hline
    
    It would not be harmful & - - - & - &  - - - & - - - & - - - & - - -  \\
    \hline
    
    I find the product reliable & - - - & - &  - - - & - - - & - - - & - - - \\
    \hline
    
    I would trust the product & - - - & - &  - - - & - - - & - - - & - - -

    \end{tabular}

    \caption{Guideline 1's t-test results %(\checkmark if Welch's t-test) 
    for comprehensive information processors vs. selective information processors participants' average ratings of the independent Violation AI product (top) and Application AI product (bottom), for all 10 dependent variables.
    If dashes (- - -) are present, no statistical test was performed.
    If the number of tests exceeded 5 for each product, Bonferroni correction applied by multiplying p-values by the number of tests performed.
    }
    \label{tab:G1-Info-Stats-Appendix}
    
    % \FIXME{MMB@AAA: FYI, I took the \checkmark s out and replaced them with plain text, because the \checkmark vs blank visually stood out so much, I kept mis-seeing it as saying only those 4 rows were signif. or important.\\
    % AAA@MMB: Redid it with Y/N. The Welch's t and t were cluttering up the table too much.\\
    % MMB@AAA: I actually prefer the spelled-out way.  Visually, the table layout now screams WELCHES IS GOOD, and draws attention away from all other columns.  Meta-comment: it might help if you forced yourself to look at this paper with a reader hat on.}

\end{table}

\clearpage
%---------------------------------------------------- End Guideline 1

%Guideline 3 ------------------------------
\begin{table}[]
    \centering
    \begin{tabular}{cc|cc|cc|cc|cc}
    \multicolumn{2}{c|}{\includegraphics[width = 0.16\columnwidth]{assets/05-All-BoxPlots/02-G3/Info/G3-Feel-In-Control-INFO.png}} &
    \multicolumn{2}{c|}{\includegraphics[width = 0.16\columnwidth]{assets/05-All-BoxPlots/02-G3/Info/G3-Feel-Secure-INFO.png}} &
    \multicolumn{2}{c|}{\includegraphics[width = 0.16\columnwidth]{assets/05-All-BoxPlots/02-G3/Info/G3-Feel-Adequate-INFO.png}} &
    \multicolumn{2}{c|}{\includegraphics[width = 0.16\columnwidth]{assets/05-All-BoxPlots/02-G3/Info/G3-Feel-Certain-INFO.png}} &
    \multicolumn{2}{c}{\includegraphics[width = 0.16\columnwidth]{assets/05-All-BoxPlots/02-G3/Info/G3-Feel-Productive-INFO.png}}
    \\
    \hline
    \hline
    \multicolumn{2}{c|}{\includegraphics[width = 0.16\columnwidth]{assets/05-All-BoxPlots/02-G3/Info/G3-Perceived-Useful-INFO.png}} &
    \multicolumn{2}{c|}{\includegraphics[width = 0.16\columnwidth]{assets/05-All-BoxPlots/02-G3/Info/G3-Not-Suspicious-INFO.png}} &
    \multicolumn{2}{c|}{\includegraphics[width = 0.16\columnwidth]{assets/05-All-BoxPlots/02-G3/Info/G3-Not-Harmful-INFO.png}} &
    \multicolumn{2}{c|}{\includegraphics[width = 0.16\columnwidth]{assets/05-All-BoxPlots/02-G3/Info/G3-Product-Reliable-INFO.png}} &
    \multicolumn{2}{c}{\includegraphics[width = 0.16\columnwidth]{assets/05-All-BoxPlots/02-G3/Info/G3-Trust-Product-INFO.png}}
    \end{tabular}
    
    \caption{Guideline 3 participants' ratings for all dependent variables, disaggregated by participants' information processing styles.
	%For the disaggregated data, notice how large the distances between the average rating are when the guideline is applied.
	Table~\ref{tab:G3-Info-Stats-Appendix} below provides the statistics (where applicable).
}
    \label{fig:Info-G3-Appendix}
\end{table}

\begin{table}[h]

%\framebox[\linewidth]{For Measuring!}
\centering
\footnotesize

    \begin{tabular}{p{0.22\columnwidth}|c|c|c|c|c|c}
    
    \rowcolor{LightGray}\multicolumn{7}{c}{\textbf{Violation AI Product}}\\
    \hline
    \textbf{Dependent}  & \textbf{Distance b/w} &  &  & & \textbf{Bonferroni} &  \\
    \textbf{variable} & \textbf{Means} &  \textbf{df} &  \textbf{t-val} &   \textbf{p-value}  & \textbf{correction} & \textbf{Cohen's \textit{d}} \\
    \hline
    
    I would feel in control & - - - & - &  - - - & - - - & - - - & - - -\\
    \hline
    
    I would feel secure & - - - & - &  - - - & - - - & - - - & - - - \\
    \hline
    
    I would feel adequate & - - - & - &  - - - & - - - & - - - & - - - \\
    \hline
    
    I would feel certain & - - - & - &  - - - & - - - & - - - & - - - \\
    \hline
    
    I would feel productive & - - - & - &  - - - & - - - & - - - & - - -  \\
    \hline
    \hline
    
    I perceived it as useful &  - - - & - &  - - - & - - - & - - - & - - -  \\
    \hline
    
    I would not be suspicious & - - - & - &  - - - & - - - & - - - & - - -  \\
    \hline
    
    It would not be harmful & - - - & - &  - - - & - - - & - - - & - - -  \\  \\
    \hline
    
    I find the product reliable & - - - & - &  - - - & - - - & - - - & - - -  \\  \\
    \hline
    
    I would trust the product & - - - & - &  - - - & - - - & - - - & - - - \\
    \hline

    \rowcolor{LightGray}\multicolumn{7}{c}{\textbf{Application AI Product}}\\
    \hline
    \textbf{Dependent}  & \textbf{Distance b/w} &  &  & & \textbf{Bonferroni} &  \\
    \textbf{variable} & \textbf{Means} &  \textbf{df} &  \textbf{t-val} &   \textbf{p-value}  & \textbf{correction} & \textbf{Cohen's \textit{d}} \\
    \hline
    
    I would feel in control & - - - & - &  - - - & - - - & - - - & - - -  \\
    \hline
    
    I would feel secure & - - - & - &  - - - & - - - & - - - & - - - \\
    \hline
    
    I would feel adequate & - - - & - &  - - - & - - - & - - - & - - - \\
    \hline
    
    I would feel certain & - - - & - &  - - - & - - - & - - - & - - - \\
    \hline
    
    I would feel productive & - - - & - &  - - - & - - - & - - - & - - -   \\
    \hline
    \hline
    
    I perceived it as useful &  - - - & - &  - - - & - - - & - - - & - - -  \\
    \hline
    
    I would not be suspicious & - - - & - &  - - - & - - - & - - - & - - -  \\
    \hline
    
    It would not be harmful & 0.6973 & 65 &  2.4542 &\cellcolor{AbiOrangeQuote}.0168 & - - - & 0.6030  \\
    \hline
    
    I find the product reliable & 0.5650 & 66 &  1.7616 & .0828 & - - - & 0.4289  \\
    \hline
    
    I would trust the product & - - - & - &  - - - & - - - & - - - & - - -

    \end{tabular}

    \caption{Guideline 3's t-test results %(\checkmark if Welch's t-test) 
    for comprehensive information processors vs. selective information processors participants' average ratings of the independent Violation AI product (top) and Application AI product (bottom), for all 10 dependent variables.
    If dashes (- - -) are present, no statistical test was performed.
    If the number of tests exceeded 5 for each product, Bonferroni correction applied by multiplying p-values by the number of tests performed.
    }
    \label{tab:G3-Info-Stats-Appendix}
    
    % \FIXME{MMB@AAA: FYI, I took the \checkmark s out and replaced them with plain text, because the \checkmark vs blank visually stood out so much, I kept mis-seeing it as saying only those 4 rows were signif. or important.\\
    % AAA@MMB: Redid it with Y/N. The Welch's t and t were cluttering up the table too much.\\
    % MMB@AAA: I actually prefer the spelled-out way.  Visually, the table layout now screams WELCHES IS GOOD, and draws attention away from all other columns.  Meta-comment: it might help if you forced yourself to look at this paper with a reader hat on.}

\end{table}

\clearpage
%---------------------------------------------------- End Guideline 3

%Begin Guideline 4----------------------------------------------------

\begin{table}[]
    \centering
    \begin{tabular}{cc|cc|cc|cc|cc}
    \multicolumn{2}{c|}{\includegraphics[width = 0.16\columnwidth]{assets/05-All-BoxPlots/03-G4/Info/G4-Feel-In-Control-INFO.png}} &
    \multicolumn{2}{c|}{\includegraphics[width = 0.16\columnwidth]{assets/05-All-BoxPlots/03-G4/Info/G4-Feel-Secure-INFO.png}} &
    \multicolumn{2}{c|}{\includegraphics[width = 0.16\columnwidth]{assets/05-All-BoxPlots/03-G4/Info/G4-Feel-Adequate-INFO.png}} &
    \multicolumn{2}{c|}{\includegraphics[width = 0.16\columnwidth]{assets/05-All-BoxPlots/03-G4/Info/G4-Feel-Certain-INFO.png}} &
    \multicolumn{2}{c}{\includegraphics[width = 0.16\columnwidth]{assets/05-All-BoxPlots/03-G4/Info/G4-Feel-Productive-INFO.png}}
    \\
    \hline
    \hline
    \multicolumn{2}{c|}{\includegraphics[width = 0.16\columnwidth]{assets/05-All-BoxPlots/03-G4/Info/G4-Perceived-Useful-INFO.png}} &
    \multicolumn{2}{c|}{\includegraphics[width = 0.16\columnwidth]{assets/05-All-BoxPlots/03-G4/Info/G4-Not-Suspicious-INFO.png}} &
    \multicolumn{2}{c|}{\includegraphics[width = 0.16\columnwidth]{assets/05-All-BoxPlots/03-G4/Info/G4-Not-Harmful-INFO.png}} &
    \multicolumn{2}{c|}{\includegraphics[width = 0.16\columnwidth]{assets/05-All-BoxPlots/03-G4/Info/G4-Product-Reliable-INFO.png}} &
    \multicolumn{2}{c}{\includegraphics[width = 0.16\columnwidth]{assets/05-All-BoxPlots/03-G4/Info/G4-Trust-Product-INFO.png}}
    \end{tabular}
    
    \caption{Guideline 4 participants' ratings for all dependent variables, disaggregated by participants' information processing styles.
	%For the disaggregated data, notice how large the distances between the average rating are when the guideline is applied.
	Table~\ref{tab:G4-Info-Stats-Appendix} below provides the statistics (where applicable).
}
    \label{fig:Info-G4-Appendix}
\end{table}

\begin{table}[h]

%\framebox[\linewidth]{For Measuring!}
\centering
\footnotesize

    \begin{tabular}{p{0.22\columnwidth}|c|c|c|c|c|c}
    
    \rowcolor{LightGray}\multicolumn{7}{c}{\textbf{Violation AI Product}}\\
    \hline
    \textbf{Dependent}  & \textbf{Distance b/w} &  &  & & \textbf{Bonferroni} &  \\
    \textbf{variable} & \textbf{Means} &  \textbf{df} &  \textbf{t-val} &   \textbf{p-value}  & \textbf{correction} & \textbf{Cohen's \textit{d}} \\
    \hline
    
    I would feel in control & - - - & - &  - - - & - - - & - - - & - - - \\
    \hline
    
    I would feel secure & 0.6334 & 62 &  2.1943 & \cellcolor{AbiOrangeQuote}.0320 & - - - & 0.5488 \\
    \hline
    
    I would feel adequate & - - - & - &  - - - & - - - & - - - & - - - \\
    \hline
    
    I would feel certain & 0.9062 & 62 &  2.4535 & \cellcolor{AbiOrangeQuote}.0170 & - - - & 0.6134 \\
    \hline
    
    I would feel productive & - - - & - &  - - - & - - - & - - - & - - -  \\
    \hline
    \hline
    
    I perceived it as useful &  - - - & - &  - - - & - - - & - - - & - - - \\
    \hline
    
    I would not be suspicious & - - - & - &  - - - & - - - & - - - & - - -  \\
    \hline
    
    It would not be harmful & - - - & - &  - - - & - - - & - - - & - - -  \\
    \hline
    
    I find the product reliable & - - - & - &  - - - & - - - & - - - & - - -  \\
    \hline
    
    I would trust the product & - - - & - &  - - - & - - - & - - - & - - -\\
    \hline

    \rowcolor{LightGray}\multicolumn{7}{c}{\textbf{Application AI Product}}\\
    \hline
    \textbf{Dependent}  & \textbf{Distance b/w} &  &  & & \textbf{Bonferroni} &  \\
    \textbf{variable} & \textbf{Means} &  \textbf{df} &  \textbf{t-val} &   \textbf{p-value}  & \textbf{correction} & \textbf{Cohen's \textit{d}} \\
    \hline
    
    I would feel in control & - - - & - &  - - - & - - - & - - - & - - - \\
    \hline
    
    I would feel secure & - - - & - &  - - - & - - - & - - - & - - - \\
    \hline
    
    I would feel adequate & - - - & - &  - - - & - - - & - - - & - - - \\
    \hline
    
    I would feel certain & - - - & - &  - - - & - - - & - - - & - - - \\
    \hline
    
    I would feel productive & - - - & - &  - - - & - - - & - - - & - - -  \\
    \hline
    \hline
    
    I perceived it as useful &  - - - & - &  - - - & - - - & - - - & - - -\\
    \hline
    
    I would not be suspicious & - - - & - &  - - - & - - - & - - - & - - -  \\
    \hline
    
    It would not be harmful & - - - & - &  - - - & - - - & - - - & - - -  \\
    \hline
    
    I find the product reliable & - - - & - &  - - - & - - - & - - - & - - - \\
    \hline
    
    I would trust the product & - - - & - &  - - - & - - - & - - - & - - -

    \end{tabular}

    \caption{Guideline 4's t-test results %(\checkmark if Welch's t-test) 
    for comprehensive information processors vs. selective information processors participants' average ratings of the independent Violation AI product (top) and Application AI product (bottom), for all 10 dependent variables.
    If dashes (- - -) are present, no statistical test was performed.
    If the number of tests exceeded 5 for each product, Bonferroni correction applied by multiplying p-values by the number of tests performed.
    }
    \label{tab:G4-Info-Stats-Appendix}
\end{table}

%---------------------------------------------------- End Guideline 4

\clearpage

%Begin Guideline 5----------------------------------------------------

\begin{table}[]
    \centering
    \begin{tabular}{cc|cc|cc|cc|cc}
    \multicolumn{2}{c|}{\includegraphics[width = 0.16\columnwidth]{assets/05-All-BoxPlots/04-G5/Info/G5-Feel-In-Control-INFO.png}} &
    \multicolumn{2}{c|}{\includegraphics[width = 0.16\columnwidth]{assets/05-All-BoxPlots/04-G5/Info/G5-Feel-Secure-INFO.png}} &
    \multicolumn{2}{c|}{\includegraphics[width = 0.16\columnwidth]{assets/05-All-BoxPlots/04-G5/Info/G5-Feel-Adequate-INFO.png}} &
    \multicolumn{2}{c|}{\includegraphics[width = 0.16\columnwidth]{assets/05-All-BoxPlots/04-G5/Info/G5-Feel-Certain-INFO.png}} &
    \multicolumn{2}{c}{\includegraphics[width = 0.16\columnwidth]{assets/05-All-BoxPlots/04-G5/Info/G5-Feel-Productive-INFO.png}}
    \\
    \hline
    \hline
    \multicolumn{2}{c|}{\includegraphics[width = 0.16\columnwidth]{assets/05-All-BoxPlots/04-G5/Info/G5-Perceived-Useful-INFO.png}} &
    \multicolumn{2}{c|}{\includegraphics[width = 0.16\columnwidth]{assets/05-All-BoxPlots/04-G5/Info/G5-Not-Suspicious-INFO.png}} &
    \multicolumn{2}{c|}{\includegraphics[width = 0.16\columnwidth]{assets/05-All-BoxPlots/04-G5/Info/G5-Not-Harmful-INFO.png}} &
    \multicolumn{2}{c|}{\includegraphics[width = 0.16\columnwidth]{assets/05-All-BoxPlots/04-G5/Info/G5-Product-Reliable-INFO.png}} &
    \multicolumn{2}{c}{\includegraphics[width = 0.16\columnwidth]{assets/05-All-BoxPlots/04-G5/Info/G5-Trust-Product-INFO.png}}
    \end{tabular}
    
    \caption{Guideline 5 participants' ratings for all dependent variables, disaggregated by participants' information processing styles.
	%For the disaggregated data, notice how large the distances between the average rating are when the guideline is applied.
	Table~\ref{tab:G5-Info-Stats-Appendix} below provides the statistics (where applicable).
}
    \label{fig:Info-G5-Appendix}
\end{table}

\begin{table}[h]

%\framebox[\linewidth]{For Measuring!}
\centering
\footnotesize

    \begin{tabular}{p{0.22\columnwidth}|c|c|c|c|c|c}
    
    \rowcolor{LightGray}\multicolumn{7}{c}{\textbf{Violation AI Product}}\\
    \hline
    \textbf{Dependent}  & \textbf{Distance b/w} &  &  & & \textbf{Bonferroni} &  \\
    \textbf{variable} & \textbf{Means} &  \textbf{df} &  \textbf{t-val} &   \textbf{p-value}  & \textbf{correction} & \textbf{Cohen's \textit{d}} \\
    \hline
    
    I would feel in control & - - - & - &  - - - & - - - & - - - & - - - \\
    \hline
    
    I would feel secure & - - - & - &  - - - & - - - & - - - & - - - \\
    \hline
    
    I would feel adequate & - - - & - &  - - - & - - - & - - - & - - - \\
    \hline
    
    I would feel certain & - - - & - &  - - - & - - - & - - - & - - - \\
    \hline
    
    I would feel productive & - - - & - &  - - - & - - - & - - - & - - -  \\
    \hline
    \hline
    
    I perceived it as useful &  - - - & - &  - - - & - - - & - - - & - - -  \\
    \hline
    
    I would not be suspicious & - - - & - &  - - - & - - - & - - - & - - -  \\
    \hline
    
    It would not be harmful & - - - & - &  - - - & - - - & - - - & - - -  \\
    \hline
    
    I find the product reliable & - - - & - &  - - - & - - - & - - - & - - -  \\
    \hline
    
    I would trust the product & - - - & - &  - - - & - - - & - - - & - - - \\
    \hline

    \rowcolor{LightGray}\multicolumn{7}{c}{\textbf{Application AI Product}}\\
    \hline
    \textbf{Dependent}  & \textbf{Distance b/w} &  &  & & \textbf{Bonferroni} &  \\
    \textbf{variable} & \textbf{Means} &  \textbf{df} &  \textbf{t-val} &   \textbf{p-value}  & \textbf{correction} & \textbf{Cohen's \textit{d}} \\
    \hline
    
    I would feel in control & - - - & - &  - - - & - - - & - - - & - - -  \\
    \hline
    
    I would feel secure & - - - & - &  - - - & - - - & - - - & - - - \\
    \hline
    
    I would feel adequate & - - - & - &  - - - & - - - & - - - & - - - \\
    \hline
    
    I would feel certain & - - - & - &  - - - & - - - & - - - & - - - \\
    \hline
    
    I would feel productive & - - - & - &  - - - & - - - & - - - & - - -    \\
    \hline
    \hline
    
    I perceived it as useful &  - - - & - &  - - - & - - - & - - - & - - -   \\
    \hline
    
    I would not be suspicious & - - - & - &  - - - & - - - & - - - & - - -   \\
    \hline
    
    It would not be harmful & - - - & - &  - - - & - - - & - - - & - - -  \\
    \hline
    
    I find the product reliable & - - - & - &  - - - & - - - & - - - & - - - \\
    \hline
    
    I would trust the product & - - - & - &  - - - & - - - & - - - & - - -

    \end{tabular}

    \caption{Guideline 5's t-test results %(\checkmark if Welch's t-test) 
    for comprehensive information processors vs. selective information processors participants' average ratings of the independent Violation AI product (top) and Application AI product (bottom), for all 10 dependent variables.
    If dashes (- - -) are present, no statistical test was performed.
    If the number of tests exceeded 5 for each product, Bonferroni correction applied by multiplying p-values by the number of tests performed.
    }
    \label{tab:G5-Info-Stats-Appendix}
\end{table}

%---------------------------------------------------- End Guideline 5

\clearpage

%Begin Guideline 6----------------------------------------------------

\begin{table}[]
    \centering
    \begin{tabular}{cc|cc|cc|cc|cc}
    \multicolumn{2}{c|}{\includegraphics[width = 0.16\columnwidth]{assets/05-All-BoxPlots/05-G6/Info/G6-Feel-In-Control-INFO.png}} &
    \multicolumn{2}{c|}{\includegraphics[width = 0.16\columnwidth]{assets/05-All-BoxPlots/05-G6/Info/G6-Feel-Secure-INFO.png}} &
    \multicolumn{2}{c|}{\includegraphics[width = 0.16\columnwidth]{assets/05-All-BoxPlots/05-G6/Info/G6-Feel-Adequate-INFO.png}} &
    \multicolumn{2}{c|}{\includegraphics[width = 0.16\columnwidth]{assets/05-All-BoxPlots/05-G6/Info/G6-Feel-Certain-INFO.png}} &
    \multicolumn{2}{c}{\includegraphics[width = 0.16\columnwidth]{assets/05-All-BoxPlots/05-G6/Info/G6-Feel-Productive-INFO.png}}
    \\
    \hline
    \hline
    \multicolumn{2}{c|}{\includegraphics[width = 0.16\columnwidth]{assets/05-All-BoxPlots/05-G6/Info/G6-Perceived-Useful-INFO.png}} &
    \multicolumn{2}{c|}{\includegraphics[width = 0.16\columnwidth]{assets/05-All-BoxPlots/05-G6/Info/G6-Not-Suspicious-INFO.png}} &
    \multicolumn{2}{c|}{\includegraphics[width = 0.16\columnwidth]{assets/05-All-BoxPlots/05-G6/Info/G6-Not-Harmful-INFO.png}} &
    \multicolumn{2}{c|}{\includegraphics[width = 0.16\columnwidth]{assets/05-All-BoxPlots/05-G6/Info/G6-Product-Reliable-INFO.png}} &
    \multicolumn{2}{c}{\includegraphics[width = 0.16\columnwidth]{assets/05-All-BoxPlots/05-G6/Info/G6-Trust-Product-INFO.png}}
    \end{tabular}
    
    \caption{Guideline 6 participants' ratings for all dependent variables, disaggregated by participants' information processing styles.
	%For the disaggregated data, notice how large the distances between the average rating are when the guideline is applied.
	Table~\ref{tab:G6-Info-Stats-Appendix} below provides the statistics (where applicable).
}
    \label{fig:Info-G6-Appendix}
\end{table}

\begin{table}[h]

%\framebox[\linewidth]{For Measuring!}
\centering
\footnotesize

    \begin{tabular}{p{0.22\columnwidth}|c|c|c|c|c|c}
    
    \rowcolor{LightGray}\multicolumn{7}{c}{\textbf{Violation AI Product}}\\
    \hline
    \textbf{Dependent}  & \textbf{Distance b/w} &  &  & & \textbf{Bonferroni} &  \\
    \textbf{variable} & \textbf{Means} &  \textbf{df} &  \textbf{t-val} &   \textbf{p-value}  & \textbf{correction} & \textbf{Cohen's \textit{d}} \\
    \hline
    
    I would feel in control & - - - & - &  - - - & - - - & - - - & - - -  \\
    \hline
    
    I would feel secure & - - - & - &  - - - & - - - & - - - & - - - \\
    \hline
    
    I would feel adequate & - - - & - &  - - - & - - - & - - - & - - - \\
    \hline
    
    I would feel certain & - - - & - &  - - - & - - - & - - - & - - - \\
    \hline
    
    I would feel productive & - - - & - &  - - - & - - - & - - - & - - -    \\
    \hline
    \hline
    
    I perceived it as useful &  - - - & - &  - - - & - - - & - - - & - - -   \\
    \hline
    
    I would not be suspicious & - - - & - &  - - - & - - - & - - - & - - -   \\
    \hline
    
    It would not be harmful & - - - & - &  - - - & - - - & - - - & - - -  \\
    \hline
    
    I find the product reliable & - - - & - &  - - - & - - - & - - - & - - - \\
    \hline
    
    I would trust the product & - - - & - &  - - - & - - - & - - - & - - - \\
    \hline

    \rowcolor{LightGray}\multicolumn{7}{c}{\textbf{Application AI Product}}\\
    \hline
    \textbf{Dependent}  & \textbf{Distance b/w} &  &  & & \textbf{Bonferroni} &  \\
    \textbf{variable} & \textbf{Means} &  \textbf{df} &  \textbf{t-val} &   \textbf{p-value}  & \textbf{correction} & \textbf{Cohen's \textit{d}} \\
    \hline
    
    I would feel in control & - - - & - &  - - - & - - - & - - - & - - -  \\
    \hline
    
    I would feel secure & - - - & - &  - - - & - - - & - - - & - - - \\
    \hline
    
    I would feel adequate & - - - & - &  - - - & - - - & - - - & - - - \\
    \hline
    
    I would feel certain & - - - & - &  - - - & - - - & - - - & - - - \\
    \hline
    
    I would feel productive & - - - & - &  - - - & - - - & - - - & - - -    \\
    \hline
    \hline
    
    I perceived it as useful &  - - - & - &  - - - & - - - & - - - & - - -   \\
    \hline
    
    I would not be suspicious & - - - & - &  - - - & - - - & - - - & - - -   \\
    \hline
    
    It would not be harmful & - - - & - &  - - - & - - - & - - - & - - -  \\
    \hline
    
    I find the product reliable & - - - & - &  - - - & - - - & - - - & - - - \\
    \hline
    
    I would trust the product & - - - & - &  - - - & - - - & - - - & - - -

    \end{tabular}

    \caption{Guideline 6's t-test results %(\checkmark if Welch's t-test) 
    for comprehensive information processors vs. selective information processors participants' average ratings of the independent Violation AI product (top) and Application AI product (bottom), for all 10 dependent variables.
    If dashes (- - -) are present, no statistical test was performed.
    If the number of tests exceeded 5 for each product, Bonferroni correction applied by multiplying p-values by the number of tests performed.
    }
    \label{tab:G6-Info-Stats-Appendix}
\end{table}

%---------------------------------------------------- End Guideline 6

\clearpage

%Begin Guideline 7----------------------------------------------------

\begin{table}[]
    \centering
    \begin{tabular}{cc|cc|cc|cc|cc}
    \multicolumn{2}{c|}{\includegraphics[width = 0.16\columnwidth]{assets/05-All-BoxPlots/06-G7/Info/G7-Feel-In-Control-INFO.png}} &
    \multicolumn{2}{c|}{\includegraphics[width = 0.16\columnwidth]{assets/05-All-BoxPlots/06-G7/Info/G7-Feel-Secure-INFO.png}} &
    \multicolumn{2}{c|}{\includegraphics[width = 0.16\columnwidth]{assets/05-All-BoxPlots/06-G7/Info/G7-Feel-Adequate-INFO.png}} &
    \multicolumn{2}{c|}{\includegraphics[width = 0.16\columnwidth]{assets/05-All-BoxPlots/06-G7/Info/G7-Feel-Certain-INFO.png}} &
    \multicolumn{2}{c}{\includegraphics[width = 0.16\columnwidth]{assets/05-All-BoxPlots/06-G7/Info/G7-Feel-Productive-INFO.png}}
    \\
    \hline
    \hline
    \multicolumn{2}{c|}{\includegraphics[width = 0.16\columnwidth]{assets/05-All-BoxPlots/06-G7/Info/G7-Perceived-Useful-INFO.png}} &
    \multicolumn{2}{c|}{\includegraphics[width = 0.16\columnwidth]{assets/05-All-BoxPlots/06-G7/Info/G7-Not-Suspicious-INFO.png}} &
    \multicolumn{2}{c|}{\includegraphics[width = 0.16\columnwidth]{assets/05-All-BoxPlots/06-G7/Info/G7-Not-Harmful-INFO.png}} &
    \multicolumn{2}{c|}{\includegraphics[width = 0.16\columnwidth]{assets/05-All-BoxPlots/06-G7/Info/G7-Product-Reliable-INFO.png}} &
    \multicolumn{2}{c}{\includegraphics[width = 0.16\columnwidth]{assets/05-All-BoxPlots/06-G7/Info/G7-Trust-Product-INFO.png}}
    \end{tabular}
    
    \caption{Guideline 7 participants' ratings for all dependent variables, disaggregated by participants' information processing styles.
	%For the disaggregated data, notice how large the distances between the average rating are when the guideline is applied.
	Table~\ref{tab:G7-Info-Stats-Appendix} below provides the statistics (where applicable).
}
    \label{fig:Info-G7-Appendix}
\end{table}

\begin{table}[h]

%\framebox[\linewidth]{For Measuring!}
\centering
\footnotesize

    \begin{tabular}{p{0.22\columnwidth}|c|c|c|c|c|c}
    
    \rowcolor{LightGray}\multicolumn{7}{c}{\textbf{Violation AI Product}}\\
    \hline
    \textbf{Dependent}  & \textbf{Distance b/w} &  &  & & \textbf{Bonferroni} &  \\
    \textbf{variable} & \textbf{Means} &  \textbf{df} &  \textbf{t-val} &   \textbf{p-value}  & \textbf{correction} & \textbf{Cohen's \textit{d}} \\
    \hline
    
    I would feel in control & 0.227 & 56 &  0.6149 & .5411 & - - - & 0.1619 \\
    \hline
    
    I would feel secure & - - - & - &  - - - & - - - & - - - & - - - \\
    \hline
    
    I would feel adequate & - - - & - &  - - - & - - - & - - - & - - - \\
    \hline
    
    I would feel certain & - - - & - &  - - - & - - - & - - - & - - - \\
    \hline
    
    I would feel productive & - - - & - &  - - - & - - - & - - - & - - -  \\
    \hline
    \hline
    
    I perceived it as useful &  - - - & - &  - - - & - - - & - - - & - - -  \\
    \hline
    
    I would not be suspicious & - - - & - &  - - - & - - - & - - - & - - -  \\
    \hline
    
    It would not be harmful & - - - & - &  - - - & - - - & - - - & - - -  \\
    \hline
    
    I find the product reliable & - - - & - &  - - - & - - - & - - - & - - -  \\
    \hline
    
    I would trust the product & - - - & - &  - - - & - - - & - - - & - - - \\
    \hline

    \rowcolor{LightGray}\multicolumn{7}{c}{\textbf{Application AI Product}}\\
    \hline
    \textbf{Dependent}  & \textbf{Distance b/w} &  &  & & \textbf{Bonferroni} &  \\
    \textbf{variable} & \textbf{Means} &  \textbf{df} &  \textbf{t-val} &   \textbf{p-value}  & \textbf{correction} & \textbf{Cohen's \textit{d}} \\
    \hline
    
    I would feel in control & 0.7168 & 56 &  2.2662 & \cellcolor{TimBlueQuote}.0273 & - - - & 0.5966  \\
    \hline
    
    I would feel secure & - - - & - &  - - - & - - - & - - - & - - - \\
    \hline
    
    I would feel adequate & - - -  & - &  - - - & - - - & - - - & - - - \\
    \hline
    
    I would feel certain & - - - & - &  - - - & - - - & - - - & - - - \\
    \hline
    
    I would feel productive & - - - & - &  - - - & - - - & - - - & - - -    \\
    \hline
    \hline
    
    I perceived it as useful &  - - - & - &  - - - & - - - & - - - & - - -   \\
    \hline
    
    I would not be suspicious & - - - & - &  - - - & - - - & - - - & - - -   \\
    \hline
    
    It would not be harmful & - - - & - &  - - - & - - - & - - - & - - -  \\
    \hline
    
    I find the product reliable & - - - & - &  - - - & - - - & - - - & - - - \\
    \hline
    
    I would trust the product & - - - & - &  - - - & - - - & - - - & - - -

    \end{tabular}

    \caption{Guideline 7's t-test results %(\checkmark if Welch's t-test) 
    for comprehensive information processors vs. selective information processors participants' average ratings of the independent Violation AI product (top) and Application AI product (bottom), for all 10 dependent variables.
    If dashes (- - -) are present, no statistical test was performed.
    If the number of tests exceeded 5 for each product, Bonferroni correction applied by multiplying p-values by the number of tests performed.
    }
    \label{tab:G7-Info-Stats-Appendix}
\end{table}

%---------------------------------------------------- End Guideline 7

\clearpage

%Begin Guideline 8----------------------------------------------------

\begin{table}[]
    \centering
    \begin{tabular}{cc|cc|cc|cc|cc}
    \multicolumn{2}{c|}{\includegraphics[width = 0.16\columnwidth]{assets/05-All-BoxPlots/07-G8/Info/G8-Feel-In-Control-INFO.png}} &
    \multicolumn{2}{c|}{\includegraphics[width = 0.16\columnwidth]{assets/05-All-BoxPlots/07-G8/Info/G8-Feel-Secure-INFO.png}} &
    \multicolumn{2}{c|}{\includegraphics[width = 0.16\columnwidth]{assets/05-All-BoxPlots/07-G8/Info/G8-Feel-Adequate-INFO.png}} &
    \multicolumn{2}{c|}{\includegraphics[width = 0.16\columnwidth]{assets/05-All-BoxPlots/07-G8/Info/G8-Feel-Certain-INFO.png}} &
    \multicolumn{2}{c}{\includegraphics[width = 0.16\columnwidth]{assets/05-All-BoxPlots/07-G8/Info/G8-Feel-Productive-INFO.png}}
    \\
    \hline
    \hline
    \multicolumn{2}{c|}{\includegraphics[width = 0.16\columnwidth]{assets/05-All-BoxPlots/07-G8/Info/G8-Perceived-Useful-INFO.png}} &
    \multicolumn{2}{c|}{\includegraphics[width = 0.16\columnwidth]{assets/05-All-BoxPlots/07-G8/Info/G8-Not-Suspicious-INFO.png}} &
    \multicolumn{2}{c|}{\includegraphics[width = 0.16\columnwidth]{assets/05-All-BoxPlots/07-G8/Info/G8-Not-Harmful-INFO.png}} &
    \multicolumn{2}{c|}{\includegraphics[width = 0.16\columnwidth]{assets/05-All-BoxPlots/07-G8/Info/G8-Product-Reliable-INFO.png}} &
    \multicolumn{2}{c}{\includegraphics[width = 0.16\columnwidth]{assets/05-All-BoxPlots/07-G8/Info/G8-Trust-Product-INFO.png}}
    \end{tabular}
    
    \caption{Guideline 8 participants' ratings for all dependent variables, disaggregated by participants' information processing styles.
	%For the disaggregated data, notice how large the distances between the average rating are when the guideline is applied.
	Table~\ref{tab:G8-Info-Stats-Appendix} below provides the statistics (where applicable).
}
    \label{fig:Info-G8-Appendix}
\end{table}

\begin{table}[h]

%\framebox[\linewidth]{For Measuring!}
\centering
\footnotesize

    \begin{tabular}{p{0.22\columnwidth}|c|c|c|c|c|c}
    
    \rowcolor{LightGray}\multicolumn{7}{c}{\textbf{Violation AI Product}}\\
    \hline
    \textbf{Dependent}  & \textbf{Distance b/w} &  &  & & \textbf{Bonferroni} &  \\
    \textbf{variable} & \textbf{Means} &  \textbf{df} &  \textbf{t-val} &   \textbf{p-value}  & \textbf{correction} & \textbf{Cohen's \textit{d}} \\
    \hline
    
    I would feel in control & 0.8145 & 58 &  1.8357 & .0715 & - - - & 0.4782 \\
    \hline
    
    I would feel secure & - - - & - &  - - - & - - - & - - - & - - - \\
    \hline
    
    I would feel adequate & - - - & - &  - - - & - - - & - - - & - - - \\
    \hline
    
    I would feel certain & - - - & - &  - - - & - - - & - - - & - - - \\
    \hline
    
    I would feel productive & - - - & - &  - - - & - - - & - - - & - - -  \\
    \hline
    \hline
    
    I perceived it as useful &  - - - & - &  - - - & - - - & - - - & - - -  \\
    \hline
    
    I would not be suspicious & - - - & - &  - - - & - - - & - - - & - - - \\
    \hline
    
    It would not be harmful & - - - & - &  - - - & - - - & - - - & - - -  \\
    \hline
    
    I find the product reliable & - - - & - &  - - - & - - - & - - - & - - -  \\
    \hline
    
    I would trust the product & 0.8824 & 58 &  2.1308 & \cellcolor{TimBlueQuote}.0374 & - - - & 0.5551 \\
    \hline

    \rowcolor{LightGray}\multicolumn{7}{c}{\textbf{Application AI Product}}\\
    \hline
    \textbf{Dependent}  & \textbf{Distance b/w} &  &  & & \textbf{Bonferroni} &  \\
    \textbf{variable} & \textbf{Means} &  \textbf{df} &  \textbf{t-val} &   \textbf{p-value}  & \textbf{correction} & \textbf{Cohen's \textit{d}} \\
    \hline
    
    I would feel in control & 0.8377 & 59 &  3.3182 & \cellcolor{TimBlueQuote}.0016 & - - - & 0.8554  \\
    \hline
    
    I would feel secure & - - - & - &  - - - & - - - & - - - & - - - \\
    \hline
    
    I would feel adequate & 0.8813  & 59 &  2.6210 & \cellcolor{TimBlueQuote}.0114 & - - - & 0.6756 \\
    \hline
    
    I would feel certain & - - - & - &  - - - & - - - & - - - & - - - \\
    \hline
    
    I would feel productive & - - - & - &  - - - & - - - & - - - & - - -    \\
    \hline
    \hline
    
    I perceived it as useful &  0.8083 & 59 &  3.5752 & \cellcolor{TimBlueQuote}.0007 & - - - & 0.9216   \\
    \hline
    
    I would not be suspicious & - - - & - &  - - - & - - - & - - - & - - -   \\
    \hline
    
    It would not be harmful & - - - & - &  - - - & - - - & - - - & - - -  \\
    \hline
    
    I find the product reliable & 0.7127 & 58 &  2.2238 & \cellcolor{TimBlueQuote}.0301 & - - - & 0.5793 \\
    \hline
    
    I would trust the product & - - - & - &  - - - & - - - & - - - & - - -

    \end{tabular}

    \caption{Guideline 8's t-test results %(\checkmark if Welch's t-test) 
    for comprehensive information processors vs. selective information processors participants' average ratings of the independent Violation AI product (top) and Application AI product (bottom), for all 10 dependent variables.
    If dashes (- - -) are present, no statistical test was performed.
    If the number of tests exceeded 5 for each product, Bonferroni correction applied by multiplying p-values by the number of tests performed.
    }
    \label{tab:G8-Info-Stats-Appendix}
\end{table}
\clearpage
%---------------------------------------------------- End Guideline 8

%Begin Guideline 9----------------------------------------------------

\begin{table}[]
    \centering
    \begin{tabular}{cc|cc|cc|cc|cc}
    \multicolumn{2}{c|}{\includegraphics[width = 0.16\columnwidth]{assets/05-All-BoxPlots/08-G9/Info/G9-Feel-In-Control-INFO.png}} &
    \multicolumn{2}{c|}{\includegraphics[width = 0.16\columnwidth]{assets/05-All-BoxPlots/08-G9/Info/G9-Feel-Secure-INFO.png}} &
    \multicolumn{2}{c|}{\includegraphics[width = 0.16\columnwidth]{assets/05-All-BoxPlots/08-G9/Info/G9-Feel-Adequate-INFO.png}} &
    \multicolumn{2}{c|}{\includegraphics[width = 0.16\columnwidth]{assets/05-All-BoxPlots/08-G9/Info/G9-Feel-Certain-INFO.png}} &
    \multicolumn{2}{c}{\includegraphics[width = 0.16\columnwidth]{assets/05-All-BoxPlots/08-G9/Info/G9-Feel-Productive-INFO.png}}
    \\
    \hline
    \hline
    \multicolumn{2}{c|}{\includegraphics[width = 0.16\columnwidth]{assets/05-All-BoxPlots/08-G9/Info/G9-Perceived-Useful-INFO.png}} &
    \multicolumn{2}{c|}{\includegraphics[width = 0.16\columnwidth]{assets/05-All-BoxPlots/08-G9/Info/G9-Not-Suspicious-INFO.png}} &
    \multicolumn{2}{c|}{\includegraphics[width = 0.16\columnwidth]{assets/05-All-BoxPlots/08-G9/Info/G9-Not-Harmful-INFO.png}} &
    \multicolumn{2}{c|}{\includegraphics[width = 0.16\columnwidth]{assets/05-All-BoxPlots/08-G9/Info/G9-Product-Reliable-INFO.png}} &
    \multicolumn{2}{c}{\includegraphics[width = 0.16\columnwidth]{assets/05-All-BoxPlots/08-G9/Info/G9-Trust-Product-INFO.png}}
    \end{tabular}
    
    \caption{Guideline 9 participants' ratings for all dependent variables, disaggregated by participants' information processing styles.
	%For the disaggregated data, notice how large the distances between the average rating are when the guideline is applied.
	Table~\ref{tab:G9-Info-Stats-Appendix} below provides the statistics (where applicable).
}
    \label{fig:Info-G9-Appendix}
\end{table}

\begin{table}[h]

%\framebox[\linewidth]{For Measuring!}
\centering
\footnotesize

    \begin{tabular}{p{0.22\columnwidth}|c|c|c|c|c|c}
    
    \rowcolor{LightGray}\multicolumn{7}{c}{\textbf{Violation AI Product}}\\
    \hline
    \textbf{Dependent}  & \textbf{Distance b/w} &  &  & & \textbf{Bonferroni} &  \\
    \textbf{variable} & \textbf{Means} &  \textbf{df} &  \textbf{t-val} &   \textbf{p-value}  & \textbf{correction} & \textbf{Cohen's \textit{d}} \\
    \hline
    
    I would feel in control & - - - & - &  - - - & - - - & - - - & - - - \\
    \hline
    
    I would feel secure & - - - & - &  - - - & - - - & - - - & - - - \\
    \hline
    
    I would feel adequate & - - - & - &  - - - & - - - & - - - & - - - \\
    \hline
    
    I would feel certain & - - - & - &  - - - & - - - & - - - & - - - \\
    \hline
    
    I would feel productive & - - - & - &  - - - & - - - & - - - & - - -  \\
    \hline
    \hline
    
    I perceived it as useful &  - - - & - &  - - - & - - - & - - - & - - -  \\
    \hline
    
    I would not be suspicious & - - - & - &  - - - & - - - & - - - & - - - \\
    \hline
    
    It would not be harmful & - - - & - &  - - - & - - - & - - - & - - -  \\
    \hline
    
    I find the product reliable & - - - & - &  - - - & - - - & - - - & - - -  \\
    \hline
    
    I would trust the product & - - - & - &  - - - & - - - & - - - & - - - \\
    \hline

    \rowcolor{LightGray}\multicolumn{7}{c}{\textbf{Application AI Product}}\\
    \hline
    \textbf{Dependent}  & \textbf{Distance b/w} &  &  & & \textbf{Bonferroni} &  \\
    \textbf{variable} & \textbf{Means} &  \textbf{df} &  \textbf{t-val} &   \textbf{p-value}  & \textbf{correction} & \textbf{Cohen's \textit{d}} \\
    \hline
    
    I would feel in control & - - - & - &  - - - & - - - & - - - & - - -  \\
    \hline
    
    I would feel secure & - - - & - &  - - - & - - - & - - - & - - - \\
    \hline
    
    I would feel adequate & - - -  & - &  - - - & - - - & - - - & - - - \\
    \hline
    
    I would feel certain & - - - & - &  - - - & - - - & - - - & - - - \\
    \hline
    
    I would feel productive & - - - & - &  - - - & - - - & - - - & - - -  \\
    \hline
    \hline
    
    I perceived it as useful &  - - - & - &  - - - & - - - & - - - & - - -  \\
    \hline
    
    I would not be suspicious & - - - & - &  - - - & - - - & - - - & - - -   \\
    \hline
    
    It would not be harmful & - - - & - &  - - - & - - - & - - - & - - -  \\
    \hline
    
    I find the product reliable & - - - & - &  - - - & - - - & - - - & - - - \\
    \hline
    
    I would trust the product & - - - & - &  - - - & - - - & - - - & - - -

    \end{tabular}

    \caption{Guideline 9's t-test results %(\checkmark if Welch's t-test) 
    for comprehensive information processors vs. selective information processors participants' average ratings of the independent Violation AI product (top) and Application AI product (bottom), for all 10 dependent variables.
    If dashes (- - -) are present, no statistical test was performed.
    If the number of tests exceeded 5 for each product, Bonferroni correction applied by multiplying p-values by the number of tests performed.
    }
    \label{tab:G9-Info-Stats-Appendix}
\end{table}
\clearpage
%---------------------------------------------------- End Guideline 9

%Begin Guideline 10----------------------------------------------------

\begin{table}[]
    \centering
    \begin{tabular}{cc|cc|cc|cc|cc}
    \multicolumn{2}{c|}{\includegraphics[width = 0.16\columnwidth]{assets/05-All-BoxPlots/09-G10/Info/G10-Feel-In-Control-INFO.png}} &
    \multicolumn{2}{c|}{\includegraphics[width = 0.16\columnwidth]{assets/05-All-BoxPlots/09-G10/Info/G10-Feel-Secure-INFO.png}} &
    \multicolumn{2}{c|}{\includegraphics[width = 0.16\columnwidth]{assets/05-All-BoxPlots/09-G10/Info/G10-Feel-Adequate-INFO.png}} &
    \multicolumn{2}{c|}{\includegraphics[width = 0.16\columnwidth]{assets/05-All-BoxPlots/09-G10/Info/G10-Feel-Certain-INFO.png}} &
    \multicolumn{2}{c}{\includegraphics[width = 0.16\columnwidth]{assets/05-All-BoxPlots/09-G10/Info/G10-Feel-Productive-INFO.png}}
    \\
    \hline
    \hline
    \multicolumn{2}{c|}{\includegraphics[width = 0.16\columnwidth]{assets/05-All-BoxPlots/09-G10/Info/G10-Perceived-Useful-INFO.png}} &
    \multicolumn{2}{c|}{\includegraphics[width = 0.16\columnwidth]{assets/05-All-BoxPlots/09-G10/Info/G10-Not-Suspicious-INFO.png}} &
    \multicolumn{2}{c|}{\includegraphics[width = 0.16\columnwidth]{assets/05-All-BoxPlots/09-G10/Info/G10-Not-Harmful-INFO.png}} &
    \multicolumn{2}{c|}{\includegraphics[width = 0.16\columnwidth]{assets/05-All-BoxPlots/09-G10/Info/G10-Product-Reliable-INFO.png}} &
    \multicolumn{2}{c}{\includegraphics[width = 0.16\columnwidth]{assets/05-All-BoxPlots/09-G10/Info/G10-Trust-Product-INFO.png}}
    \end{tabular}
    
    \caption{Guideline 10 participants' ratings for all dependent variables, disaggregated by participants' information processing styles.
	%For the disaggregated data, notice how large the distances between the average rating are when the guideline is applied.
	Table~\ref{tab:G10-Info-Stats-Appendix} below provides the statistics (where applicable).
}
    \label{fig:Info-G10-Appendix}
\end{table}

\begin{table}[h]

%\framebox[\linewidth]{For Measuring!}
\centering
\footnotesize

    \begin{tabular}{p{0.22\columnwidth}|c|c|c|c|c|c}
    
    \rowcolor{LightGray}\multicolumn{7}{c}{\textbf{Violation AI Product}}\\
    \hline
    \textbf{Dependent}  & \textbf{Distance b/w} &  &  & & \textbf{Bonferroni} &  \\
    \textbf{variable} & \textbf{Means} &  \textbf{df} &  \textbf{t-val} &   \textbf{p-value}  & \textbf{correction} & \textbf{Cohen's \textit{d}} \\
    \hline
    
    I would feel in control & - - - & - &  - - - & - - - & - - - & - - - \\
    \hline
    
    I would feel secure & - - - & - &  - - - & - - - & - - - & - - - \\
    \hline
    
    I would feel adequate & - - - & - &  - - - & - - - & - - - & - - - \\
    \hline
    
    I would feel certain & - - - & - &  - - - & - - - & - - - & - - - \\
    \hline
    
    I would feel productive & - - - & - &  - - - & - - - & - - - & - - -  \\
    \hline
    \hline
    
    I perceived it as useful &  - - - & - &  - - - & - - - & - - - & - - -  \\
    \hline
    
    I would not be suspicious & - - - & - &  - - - & - - - & - - - & - - - \\
    \hline
    
    It would not be harmful & - - - & - &  - - - & - - - & - - - & - - -  \\
    \hline
    
    I find the product reliable & - - - & - &  - - - & - - - & - - - & - - -  \\
    \hline
    
    I would trust the product & - - - & - &  - - - & - - - & - - - & - - - \\
    \hline

    \rowcolor{LightGray}\multicolumn{7}{c}{\textbf{Application AI Product}}\\
    \hline
    \textbf{Dependent}  & \textbf{Distance b/w} &  &  & & \textbf{Bonferroni} &  \\
    \textbf{variable} & \textbf{Means} &  \textbf{df} &  \textbf{t-val} &   \textbf{p-value}  & \textbf{correction} & \textbf{Cohen's \textit{d}} \\
    \hline
    
   I would feel in control & - - - & - &  - - - & - - - & - - - & - - -  \\
    \hline
    
    I would feel secure & - - - & - &  - - - & - - - & - - - & - - - \\
    \hline
    
    I would feel adequate & - - -  & - &  - - - & - - - & - - - & - - - \\
    \hline
    
    I would feel certain & - - - & - &  - - - & - - - & - - - & - - - \\
    \hline
    
    I would feel productive & - - - & - &  - - - & - - - & - - - & - - -  \\
    \hline
    \hline
    
    I perceived it as useful &  - - - & - &  - - - & - - - & - - - & - - -  \\
    \hline
    
    I would not be suspicious & - - - & - &  - - - & - - - & - - - & - - -   \\
    \hline
    
    It would not be harmful & 0.6752 & 63 &  2.2725 & \cellcolor{TimBlueQuote}.0265 & - - - & 0.5638  \\
    \hline
    
    I find the product reliable & - - - & - &  - - - & - - - & - - - & - - - \\
    \hline
    
    I would trust the product & - - - & - &  - - - & - - - & - - - & - - -

    \end{tabular}

    \caption{Guideline 10's t-test results %(\checkmark if Welch's t-test) 
    for comprehensive information processors vs. selective information processors participants' average ratings of the independent Violation AI product (top) and Application AI product (bottom), for all 10 dependent variables.
    If dashes (- - -) are present, no statistical test was performed.
    If the number of tests exceeded 5 for each product, Bonferroni correction applied by multiplying p-values by the number of tests performed.
    }
    \label{tab:G10-Info-Stats-Appendix}
\end{table}
\clearpage
%---------------------------------------------------- End Guideline 10

%Begin Guideline 11----------------------------------------------------

\begin{table}[]
    \centering
    \begin{tabular}{cc|cc|cc|cc|cc}
    \multicolumn{2}{c|}{\includegraphics[width = 0.16\columnwidth]{assets/05-All-BoxPlots/10-G11/Info/G11-Feel-In-Control-INFO.png}} &
    \multicolumn{2}{c|}{\includegraphics[width = 0.16\columnwidth]{assets/05-All-BoxPlots/10-G11/Info/G11-Feel-Secure-INFO.png}} &
    \multicolumn{2}{c|}{\includegraphics[width = 0.16\columnwidth]{assets/05-All-BoxPlots/10-G11/Info/G11-Feel-Adequate-INFO.png}} &
    \multicolumn{2}{c|}{\includegraphics[width = 0.16\columnwidth]{assets/05-All-BoxPlots/10-G11/Info/G11-Feel-Certain-INFO.png}} &
    \multicolumn{2}{c}{\includegraphics[width = 0.16\columnwidth]{assets/05-All-BoxPlots/10-G11/Info/G11-Feel-Productive-INFO.png}}
    \\
    \hline
    \hline
    \multicolumn{2}{c|}{\includegraphics[width = 0.16\columnwidth]{assets/05-All-BoxPlots/10-G11/Info/G11-Perceived-Useful-INFO.png}} &
    \multicolumn{2}{c|}{\includegraphics[width = 0.16\columnwidth]{assets/05-All-BoxPlots/10-G11/Info/G11-Not-Suspicious-INFO.png}} &
    \multicolumn{2}{c|}{\includegraphics[width = 0.16\columnwidth]{assets/05-All-BoxPlots/10-G11/Info/G11-Not-Harmful-INFO.png}} &
    \multicolumn{2}{c|}{\includegraphics[width = 0.16\columnwidth]{assets/05-All-BoxPlots/10-G11/Info/G11-Product-Reliable-INFO.png}} &
    \multicolumn{2}{c}{\includegraphics[width = 0.16\columnwidth]{assets/05-All-BoxPlots/10-G11/Info/G11-Trust-Product-INFO.png}}
    \end{tabular}
    
    \caption{Guideline 11 participants' ratings for all dependent variables, disaggregated by participants' information processing styles.
	%For the disaggregated data, notice how large the distances between the average rating are when the guideline is applied.
	Table~\ref{tab:G11-Info-Stats-Appendix} below provides the statistics (where applicable).
}
    \label{fig:Info-G11-Appendix}
\end{table}

\begin{table}[h]

%\framebox[\linewidth]{For Measuring!}
\centering
\footnotesize

    \begin{tabular}{p{0.22\columnwidth}|c|c|c|c|c|c}
    
    \rowcolor{LightGray}\multicolumn{7}{c}{\textbf{Violation AI Product}}\\
    \hline
    \textbf{Dependent}  & \textbf{Distance b/w} &  &  & & \textbf{Bonferroni} &  \\
    \textbf{variable} & \textbf{Means} &  \textbf{df} &  \textbf{t-val} &   \textbf{p-value}  & \textbf{correction} & \textbf{Cohen's \textit{d}} \\
    \hline
    
    I would feel in control & - - - & - &  - - - & - - - & - - - & - - - \\
    \hline
    
    I would feel secure & - - - & - &  - - - & - - - & - - - & - - - \\
    \hline
    
    I would feel adequate & 0.9607 & 61 &  2.3436 & \cellcolor{TimBlueQuote}.0224 & - - - & 0.5906 \\
    \hline
    
    I would feel certain & - - - & - &  - - - & - - - & - - - & - - - \\
    \hline
    
    I would feel productive & - - - & - &  - - - & - - - & - - - & - - -  \\
    \hline
    \hline
    
    I perceived it as useful &  - - - & - &  - - - & - - - & - - - & - - -  \\
    \hline
    
    I would not be suspicious & - - - & - &  - - - & - - - & - - - & - - - \\
    \hline
    
    It would not be harmful & - - - & - &  - - - & - - - & - - - & - - -  \\
    \hline
    
    I find the product reliable & - - - & - &  - - - & - - - & - - - & - - -  \\
    \hline
    
    I would trust the product & - - - & - &  - - - & - - - & - - - & - - - \\
    \hline

    \rowcolor{LightGray}\multicolumn{7}{c}{\textbf{Application AI Product}}\\
    \hline
    \textbf{Dependent}  & \textbf{Distance b/w} &  &  & & \textbf{Bonferroni} &  \\
    \textbf{variable} & \textbf{Means} &  \textbf{df} &  \textbf{t-val} &   \textbf{p-value}  & \textbf{correction} & \textbf{Cohen's \textit{d}} \\
    \hline
    
    I would feel in control &- - - & - &  - - - & - - - & - - - & - - -  \\
    \hline
    
    I would feel secure & - - - & - &  - - - & - - - & - - - & - - - \\
    \hline
    
    I would feel adequate & - - - & - &  - - - & - - - & - - - & - - - \\
    \hline
    
    I would feel certain & - - - & - &  - - - & - - - & - - - & - - - \\
    \hline
    
    I would feel productive & - - - & - &  - - - & - - - & - - - & - - -   \\
    \hline
    \hline
    
    I perceived it as useful & 0.6935 & 61 &  1.8937 & .0630 & - - - & 0.4772   \\
    \hline
    
    I would not be suspicious & - - - & - &  - - - & - - - & - - - & - - -   \\
    \hline
    
    It would not be harmful & - - - & - &  - - - & - - - & - - - & - - -  \\
    \hline
    
    I find the product reliable & - - - & - &  - - - & - - - & - - - & - - - \\
    \hline
    
    I would trust the product & - - - & - &  - - - & - - - & - - - & - - -

    \end{tabular}

    \caption{Guideline 11's t-test results %(\checkmark if Welch's t-test) 
    for comprehensive information processors vs. selective information processors participants' average ratings of the independent Violation AI product (top) and Application AI product (bottom), for all 10 dependent variables.
    If dashes (- - -) are present, no statistical test was performed.
    If the number of tests exceeded 5 for each product, Bonferroni correction applied by multiplying p-values by the number of tests performed.
    }
    \label{tab:G11-Info-Stats-Appendix}
\end{table}
\clearpage
%---------------------------------------------------- End Guideline 11

%Begin Guideline 12----------------------------------------------------

\begin{table}[]
    \centering
    \begin{tabular}{cc|cc|cc|cc|cc}
    \multicolumn{2}{c|}{\includegraphics[width = 0.16\columnwidth]{assets/05-All-BoxPlots/11-G12/Info/G12-Feel-In-Control-INFO.png}} &
    \multicolumn{2}{c|}{\includegraphics[width = 0.16\columnwidth]{assets/05-All-BoxPlots/11-G12/Info/G12-Feel-Secure-INFO.png}} &
    \multicolumn{2}{c|}{\includegraphics[width = 0.16\columnwidth]{assets/05-All-BoxPlots/11-G12/Info/G12-Feel-Adequate-INFO.png}} &
    \multicolumn{2}{c|}{\includegraphics[width = 0.16\columnwidth]{assets/05-All-BoxPlots/11-G12/Info/G12-Feel-Certain-INFO.png}} &
    \multicolumn{2}{c}{\includegraphics[width = 0.16\columnwidth]{assets/05-All-BoxPlots/11-G12/Info/G12-Feel-Productive-INFO.png}}
    \\
    \hline
    \hline
    \multicolumn{2}{c|}{\includegraphics[width = 0.16\columnwidth]{assets/05-All-BoxPlots/11-G12/Info/G12-Perceived-Useful-INFO.png}} &
    \multicolumn{2}{c|}{\includegraphics[width = 0.16\columnwidth]{assets/05-All-BoxPlots/11-G12/Info/G12-Not-Suspicious-INFO.png}} &
    \multicolumn{2}{c|}{\includegraphics[width = 0.16\columnwidth]{assets/05-All-BoxPlots/11-G12/Info/G12-Not-Harmful-INFO.png}} &
    \multicolumn{2}{c|}{\includegraphics[width = 0.16\columnwidth]{assets/05-All-BoxPlots/11-G12/Info/G12-Product-Reliable-INFO.png}} &
    \multicolumn{2}{c}{\includegraphics[width = 0.16\columnwidth]{assets/05-All-BoxPlots/11-G12/Info/G12-Trust-Product-INFO.png}}
    \end{tabular}
    
    \caption{Guideline 12 participants' ratings for all dependent variables, disaggregated by participants' information processing styles.
	%For the disaggregated data, notice how large the distances between the average rating are when the guideline is applied.
	Table~\ref{tab:G12-Info-Stats-Appendix} below provides the statistics (where applicable).
}
    \label{fig:Info-G12-Appendix}
\end{table}

\begin{table}[h]

%\framebox[\linewidth]{For Measuring!}
\centering
\footnotesize

    \begin{tabular}{p{0.22\columnwidth}|c|c|c|c|c|c}
    
    \rowcolor{LightGray}\multicolumn{7}{c}{\textbf{Violation AI Product}}\\
    \hline
    \textbf{Dependent}  & \textbf{Distance b/w} &  &  & & \textbf{Bonferroni} &  \\
    \textbf{variable} & \textbf{Means} &  \textbf{df} &  \textbf{t-val} &   \textbf{p-value}  & \textbf{correction} & \textbf{Cohen's \textit{d}} \\
    \hline
    
    I would feel in control & - - - & - &  - - - & - - - & - - - & - - -  \\
    \hline
    
    I would feel secure & - - - & - &  - - - & - - - & - - - & - - - \\
    \hline
    
    I would feel adequate & - - -  & - &  - - - & - - - & - - - & - - - \\
    \hline
    
    I would feel certain & - - - & - &  - - - & - - - & - - - & - - - \\
    \hline
    
    I would feel productive & - - - & - &  - - - & - - - & - - - & - - -   \\
    \hline
    \hline
    
    I perceived it as useful &  - - - & - &  - - - & - - - & - - - & - - -   \\
    \hline
    
    I would not be suspicious & 0.8125 & 66 &  2.2418 & \cellcolor{AbiOrangeQuote}.0283 & - - - & 0.5447   \\
    \hline
    
    It would not be harmful & - - - & - &  - - - & - - - & - - - & - - -  \\
    \hline
    
    I find the product reliable & - - - & - &  - - - & - - - & - - - & - - - \\
    \hline
    
    I would trust the product & - - - & - &  - - - & - - - & - - - & - - - \\
    \hline

    \rowcolor{LightGray}\multicolumn{7}{c}{\textbf{Application AI Product}}\\
    \hline
    \textbf{Dependent}  & \textbf{Distance b/w} &  &  & & \textbf{Bonferroni} &  \\
    \textbf{variable} & \textbf{Means} &  \textbf{df} &  \textbf{t-val} &   \textbf{p-value}  & \textbf{correction} & \textbf{Cohen's \textit{d}} \\
    \hline
    
    I would feel in control & - - - & - &  - - - & - - - & - - - & - - -  \\
    \hline
    
    I would feel secure & - - - & - &  - - - & - - - & - - - & - - - \\
    \hline
    
    I would feel adequate & - - -  & - &  - - - & - - - & - - - & - - - \\
    \hline
    
    I would feel certain & - - - & - &  - - - & - - - & - - - & - - - \\
    \hline
    
    I would feel productive & - - - & - &  - - - & - - - & - - - & - - -   \\
    \hline
    \hline
    
    I perceived it as useful &  - - - & - &  - - - & - - - & - - - & - - -   \\
    \hline
    
    I would not be suspicious & 0.7172 & 67 &  1.8252 & .0724 & - - - & 0.4399   \\
    \hline
    
    It would not be harmful & - - - & - &  - - - & - - - & - - - & - - -  \\
    \hline
    
    I find the product reliable & - - - & - &  - - - & - - - & - - - & - - - \\
    \hline
    
    I would trust the product & - - - & - &  - - - & - - - & - - - & - - -

    \end{tabular}

    \caption{Guideline 12's t-test results %(\checkmark if Welch's t-test) 
    for comprehensive information processors vs. selective information processors participants' average ratings of the independent Violation AI product (top) and Application AI product (bottom), for all 10 dependent variables.
    If dashes (- - -) are present, no statistical test was performed.
    If the number of tests exceeded 5 for each product, Bonferroni correction applied by multiplying p-values by the number of tests performed.
    }
    \label{tab:G12-Info-Stats-Appendix}
\end{table}
\clearpage
%---------------------------------------------------- End Guideline 12

%Begin Guideline 13----------------------------------------------------

\begin{table}[]
    \centering
    \begin{tabular}{cc|cc|cc|cc|cc}
    \multicolumn{2}{c|}{\includegraphics[width = 0.16\columnwidth]{assets/05-All-BoxPlots/12-G13/Info/G13-Feel-In-Control-INFO.png}} &
    \multicolumn{2}{c|}{\includegraphics[width = 0.16\columnwidth]{assets/05-All-BoxPlots/12-G13/Info/G13-Feel-Secure-INFO.png}} &
    \multicolumn{2}{c|}{\includegraphics[width = 0.16\columnwidth]{assets/05-All-BoxPlots/12-G13/Info/G13-Feel-Adequate-INFO.png}} &
    \multicolumn{2}{c|}{\includegraphics[width = 0.16\columnwidth]{assets/05-All-BoxPlots/12-G13/Info/G13-Feel-Certain-INFO.png}} &
    \multicolumn{2}{c}{\includegraphics[width = 0.16\columnwidth]{assets/05-All-BoxPlots/12-G13/Info/G13-Feel-Productive-INFO.png}}
    \\
    \hline
    \hline
    \multicolumn{2}{c|}{\includegraphics[width = 0.16\columnwidth]{assets/05-All-BoxPlots/12-G13/Info/G13-Perceived-Useful-INFO.png}} &
    \multicolumn{2}{c|}{\includegraphics[width = 0.16\columnwidth]{assets/05-All-BoxPlots/12-G13/Info/G13-Not-Suspicious-INFO.png}} &
    \multicolumn{2}{c|}{\includegraphics[width = 0.16\columnwidth]{assets/05-All-BoxPlots/12-G13/Info/G13-Not-Harmful-INFO.png}} &
    \multicolumn{2}{c|}{\includegraphics[width = 0.16\columnwidth]{assets/05-All-BoxPlots/12-G13/Info/G13-Product-Reliable-INFO.png}} &
    \multicolumn{2}{c}{\includegraphics[width = 0.16\columnwidth]{assets/05-All-BoxPlots/12-G13/Info/G13-Trust-Product-INFO.png}}
    \end{tabular}
    
    \caption{Guideline 13 participants' ratings for all dependent variables, disaggregated by participants' information processing styles.
	%For the disaggregated data, notice how large the distances between the average rating are when the guideline is applied.
	Table~\ref{tab:G13-Info-Stats-Appendix} below provides the statistics (where applicable).
}
    \label{fig:Info-G13-Appendix}
\end{table}

\begin{table}[h]

%\framebox[\linewidth]{For Measuring!}
\centering
\footnotesize

    \begin{tabular}{p{0.22\columnwidth}|c|c|c|c|c|c}
    
    \rowcolor{LightGray}\multicolumn{7}{c}{\textbf{Violation AI Product}}\\
    \hline
    \textbf{Dependent}  & \textbf{Distance b/w} &  &  & & \textbf{Bonferroni} &  \\
    \textbf{variable} & \textbf{Means} &  \textbf{df} &  \textbf{t-val} &   \textbf{p-value}  & \textbf{correction} & \textbf{Cohen's \textit{d}} \\
    \hline
    
    I would feel in control & - - - & - &  - - - & - - - & - - - & - - -  \\
    \hline
    
    I would feel secure & - - - & - &  - - - & - - - & - - - & - - - \\
    \hline
    
    I would feel adequate & 0.8300  & 55 &  1.9315 & .0586 & - - - & 0.5136 \\
    \hline
    
    I would feel certain & - - - & - &  - - - & - - - & - - - & - - - \\
    \hline
    
    I would feel productive & - - - & - &  - - - & - - - & - - - & - - -   \\
    \hline
    \hline
    
    I perceived it as useful &  - - - & - &  - - - & - - - & - - - & - - -   \\
    \hline
    
    I would not be suspicious & - - - & - &  - - - & - - - & - - - & - - - \\
    \hline
    
    It would not be harmful & - - - & - &  - - - & - - - & - - - & - - - \\
    \hline
    
    I find the product reliable & - - - & - &  - - - & - - - & - - - & - - - \\
    \hline
    
    I would trust the product & - - - & - &  - - - & - - - & - - - & - - - \\
    \hline

    \rowcolor{LightGray}\multicolumn{7}{c}{\textbf{Application AI Product}}\\
    \hline
    \textbf{Dependent}  & \textbf{Distance b/w} &  &  & & \textbf{Bonferroni} &  \\
    \textbf{variable} & \textbf{Means} &  \textbf{df} &  \textbf{t-val} &   \textbf{p-value}  & \textbf{correction} & \textbf{Cohen's \textit{d}} \\
    \hline
    
    I would feel in control & - - - & - &  - - - & - - - & - - - & - - -  \\
    \hline
    
    I would feel secure & - - - & - &  - - - & - - - & - - - & - - - \\
    \hline
    
    I would feel adequate & 0.6985 & 55 &  1.9472 & .0566 & - - - & 0.5178 \\
    \hline
    
    I would feel certain & 0.7841 & 55 &  1.9698 & .0539 & - - - & 0.5238 \\
    \hline
    
    I would feel productive & - - - & - &  - - - & - - - & - - - & - - -   \\
    \hline
    \hline
    
    I perceived it as useful &  0.5385 & 54 &  2.0789 & \cellcolor{TimBlueQuote}.0424 & - - - & 0.5570 \\
    \hline
    
    I would not be suspicious & - - - & - &  - - - & - - - & - - - & - - - \\
    \hline
    
    It would not be harmful & - - - & - &  - - - & - - - & - - - & - - -  \\
    \hline
    
    I find the product reliable & - - - & - &  - - - & - - - & - - - & - - - \\
    \hline
    
    I would trust the product & - - - & - &  - - - & - - - & - - - & - - -

    \end{tabular}

    \caption{Guideline 13's t-test results %(\checkmark if Welch's t-test) 
    for comprehensive information processors vs. selective information processors participants' average ratings of the independent Violation AI product (top) and Application AI product (bottom), for all 10 dependent variables.
    If dashes (- - -) are present, no statistical test was performed.
    If the number of tests exceeded 5 for each product, Bonferroni correction applied by multiplying p-values by the number of tests performed.
    }
    \label{tab:G13-Info-Stats-Appendix}
\end{table}
\clearpage
%---------------------------------------------------- End Guideline 13

%Begin Guideline 14---------------------------------------------------

\begin{table}[]
    \centering
    \begin{tabular}{cc|cc|cc|cc|cc}
    \multicolumn{2}{c|}{\includegraphics[width = 0.16\columnwidth]{assets/05-All-BoxPlots/13-G14/Info/G14-Feel-In-Control-INFO.png}} &
    \multicolumn{2}{c|}{\includegraphics[width = 0.16\columnwidth]{assets/05-All-BoxPlots/13-G14/Info/G14-Feel-Secure-INFO.png}} &
    \multicolumn{2}{c|}{\includegraphics[width = 0.16\columnwidth]{assets/05-All-BoxPlots/13-G14/Info/G14-Feel-Adequate-INFO.png}} &
    \multicolumn{2}{c|}{\includegraphics[width = 0.16\columnwidth]{assets/05-All-BoxPlots/13-G14/Info/G14-Feel-Certain-INFO.png}} &
    \multicolumn{2}{c}{\includegraphics[width = 0.16\columnwidth]{assets/05-All-BoxPlots/13-G14/Info/G14-Feel-Productive-INFO.png}}
    \\
    \hline
    \hline
    \multicolumn{2}{c|}{\includegraphics[width = 0.16\columnwidth]{assets/05-All-BoxPlots/13-G14/Info/G14-Perceived-Useful-INFO.png}} &
    \multicolumn{2}{c|}{\includegraphics[width = 0.16\columnwidth]{assets/05-All-BoxPlots/13-G14/Info/G14-Not-Suspicious-INFO.png}} &
    \multicolumn{2}{c|}{\includegraphics[width = 0.16\columnwidth]{assets/05-All-BoxPlots/13-G14/Info/G14-Not-Harmful-INFO.png}} &
    \multicolumn{2}{c|}{\includegraphics[width = 0.16\columnwidth]{assets/05-All-BoxPlots/13-G14/Info/G14-Product-Reliable-INFO.png}} &
    \multicolumn{2}{c}{\includegraphics[width = 0.16\columnwidth]{assets/05-All-BoxPlots/13-G14/Info/G14-Trust-Product-INFO.png}}
    \end{tabular}
    
    \caption{Guideline 14 participants' ratings for all dependent variables, disaggregated by participants' information processing styles.
	%For the disaggregated data, notice how large the distances between the average rating are when the guideline is applied.
	Table~\ref{tab:G14-Info-Stats-Appendix} below provides the statistics (where applicable).
}
    \label{fig:Info-G14-Appendix}
\end{table}

\begin{table}[h]

%\framebox[\linewidth]{For Measuring!}
\centering
\footnotesize

    \begin{tabular}{p{0.22\columnwidth}|c|c|c|c|c|c}
    
    \rowcolor{LightGray}\multicolumn{7}{c}{\textbf{Violation AI Product}}\\
    \hline
    \textbf{Dependent}  & \textbf{Distance b/w} &  &  & & \textbf{Bonferroni} &  \\
    \textbf{variable} & \textbf{Means} &  \textbf{df} &  \textbf{t-val} &   \textbf{p-value}  & \textbf{correction} & \textbf{Cohen's \textit{d}} \\
    \hline
    
    I would feel in control & - - - & - &  - - - & - - - & - - - & - - -  \\
    \hline
    
    I would feel secure & - - - & - &  - - - & - - - & - - - & - - -\\
    \hline
    
    I would feel adequate & - - - & - &  - - - & - - - & - - - & - - - \\
    \hline
    
    I would feel certain &- - - & - &  - - - & - - - & - - - & - - - \\
    \hline
    
    I would feel productive & - - - & - &  - - - & - - - & - - - & - - -  \\
    \hline
    \hline
    
    I perceived it as useful &  - - - & - &  - - - & - - - & - - - & - - -   \\
    \hline
    
    I would not be suspicious & - - - & - &  - - - & - - - & - - - & - - -  \\
    \hline
    
    It would not be harmful & - - - & - &  - - - & - - - & - - - & - - -  \\
    \hline
    
    I find the product reliable & - - - & - &  - - - & - - - & - - - & - - - \\
    \hline
    
    I would trust the product & - - - & - &  - - - & - - - & - - - & - - - \\
    \hline

    \rowcolor{LightGray}\multicolumn{7}{c}{\textbf{Application AI Product}}\\
    \hline
    \textbf{Dependent}  & \textbf{Distance b/w} &  &  & & \textbf{Bonferroni} &  \\
    \textbf{variable} & \textbf{Means} &  \textbf{df} &  \textbf{t-val} &   \textbf{p-value}  & \textbf{correction} & \textbf{Cohen's \textit{d}} \\
    \hline
    
    I would feel in control & - - - & - &  - - - & - - - & - - - & - - -  \\
    \hline
    
    I would feel secure & - - - & - &  - - - & - - - & - - - & - - - \\
    \hline
    
    I would feel adequate & 0.6378 & 65 &  2.0742 & \cellcolor{AbiOrangeQuote}.0420 & - - - & 0.5096 \\
    \hline
    
    I would feel certain & - - - & - &  - - - & - - - & - - - & - - - \\
    \hline
    
    I would feel productive & - - - & - &  - - - & - - - & - - - & - - -   \\
    \hline
    \hline
    
    I perceived it as useful &  - - - & - &  - - - & - - - & - - - & - - -   \\
    \hline
    
    I would not be suspicious & - - - & - &  - - - & - - - & - - - & - - -   \\
    \hline
    
    It would not be harmful & - - - & - &  - - - & - - - & - - - & - - -  \\
    \hline
    
    I find the product reliable & - - - & - &  - - - & - - - & - - - & - - - \\
    \hline
    
    I would trust the product & - - - & - &  - - - & - - - & - - - & - - -

    \end{tabular}

    \caption{Guideline 14's t-test results %(\checkmark if Welch's t-test) 
    for comprehensive information processors vs. selective information processors participants' average ratings of the independent Violation AI product (top) and Application AI product (bottom), for all 10 dependent variables.
    If dashes (- - -) are present, no statistical test was performed.
    If the number of tests exceeded 5 for each product, Bonferroni correction applied by multiplying p-values by the number of tests performed.
    }
    \label{tab:G14-Info-Stats-Appendix}
\end{table}
\clearpage
%---------------------------------------------------- End Guideline 14

%Begin Guideline 15---------------------------------------------------

\begin{table}[]
    \centering
    \begin{tabular}{cc|cc|cc|cc|cc}
    \multicolumn{2}{c|}{\includegraphics[width = 0.16\columnwidth]{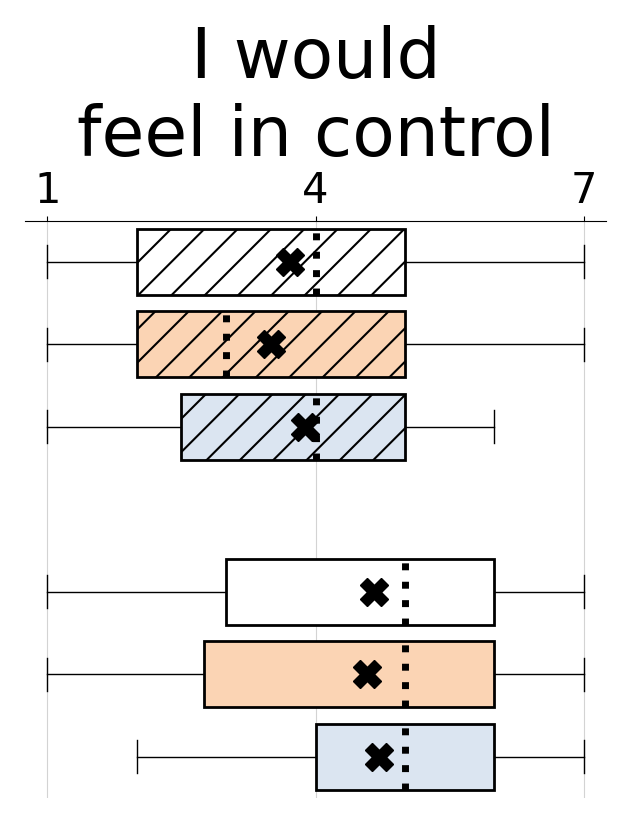}} &
    \multicolumn{2}{c|}{\includegraphics[width = 0.16\columnwidth]{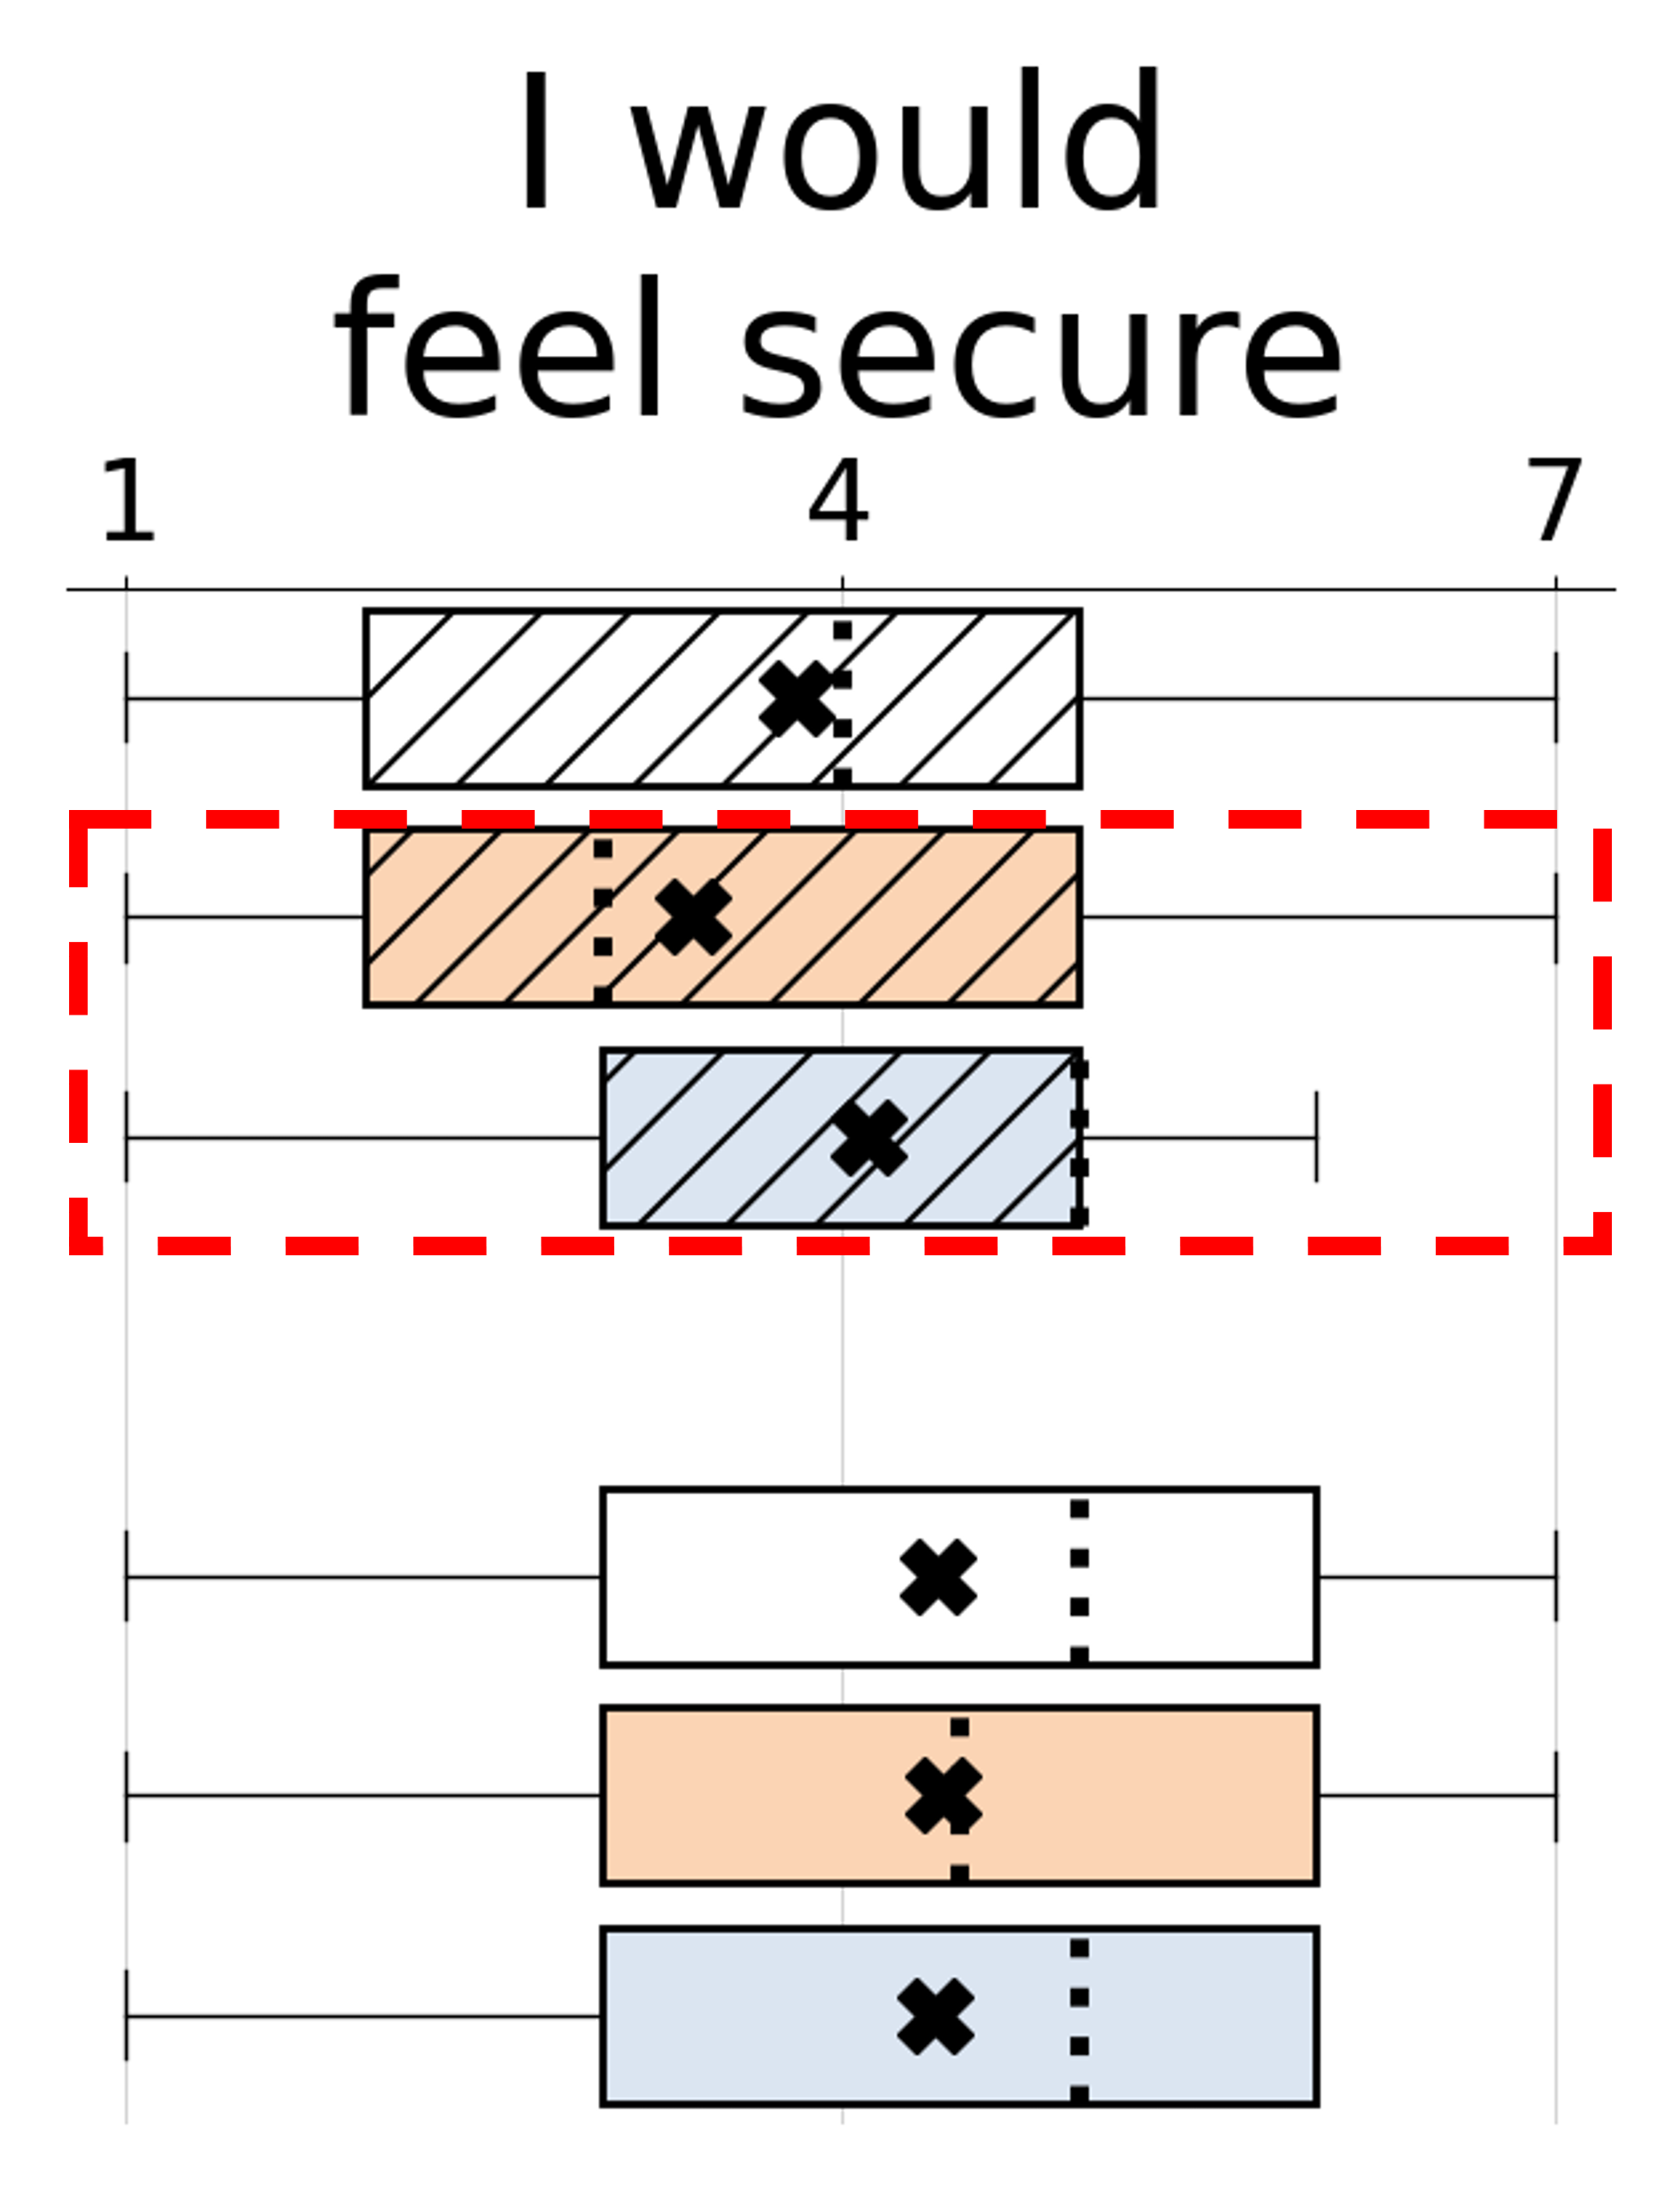}} &
    \multicolumn{2}{c|}{\includegraphics[width = 0.16\columnwidth]{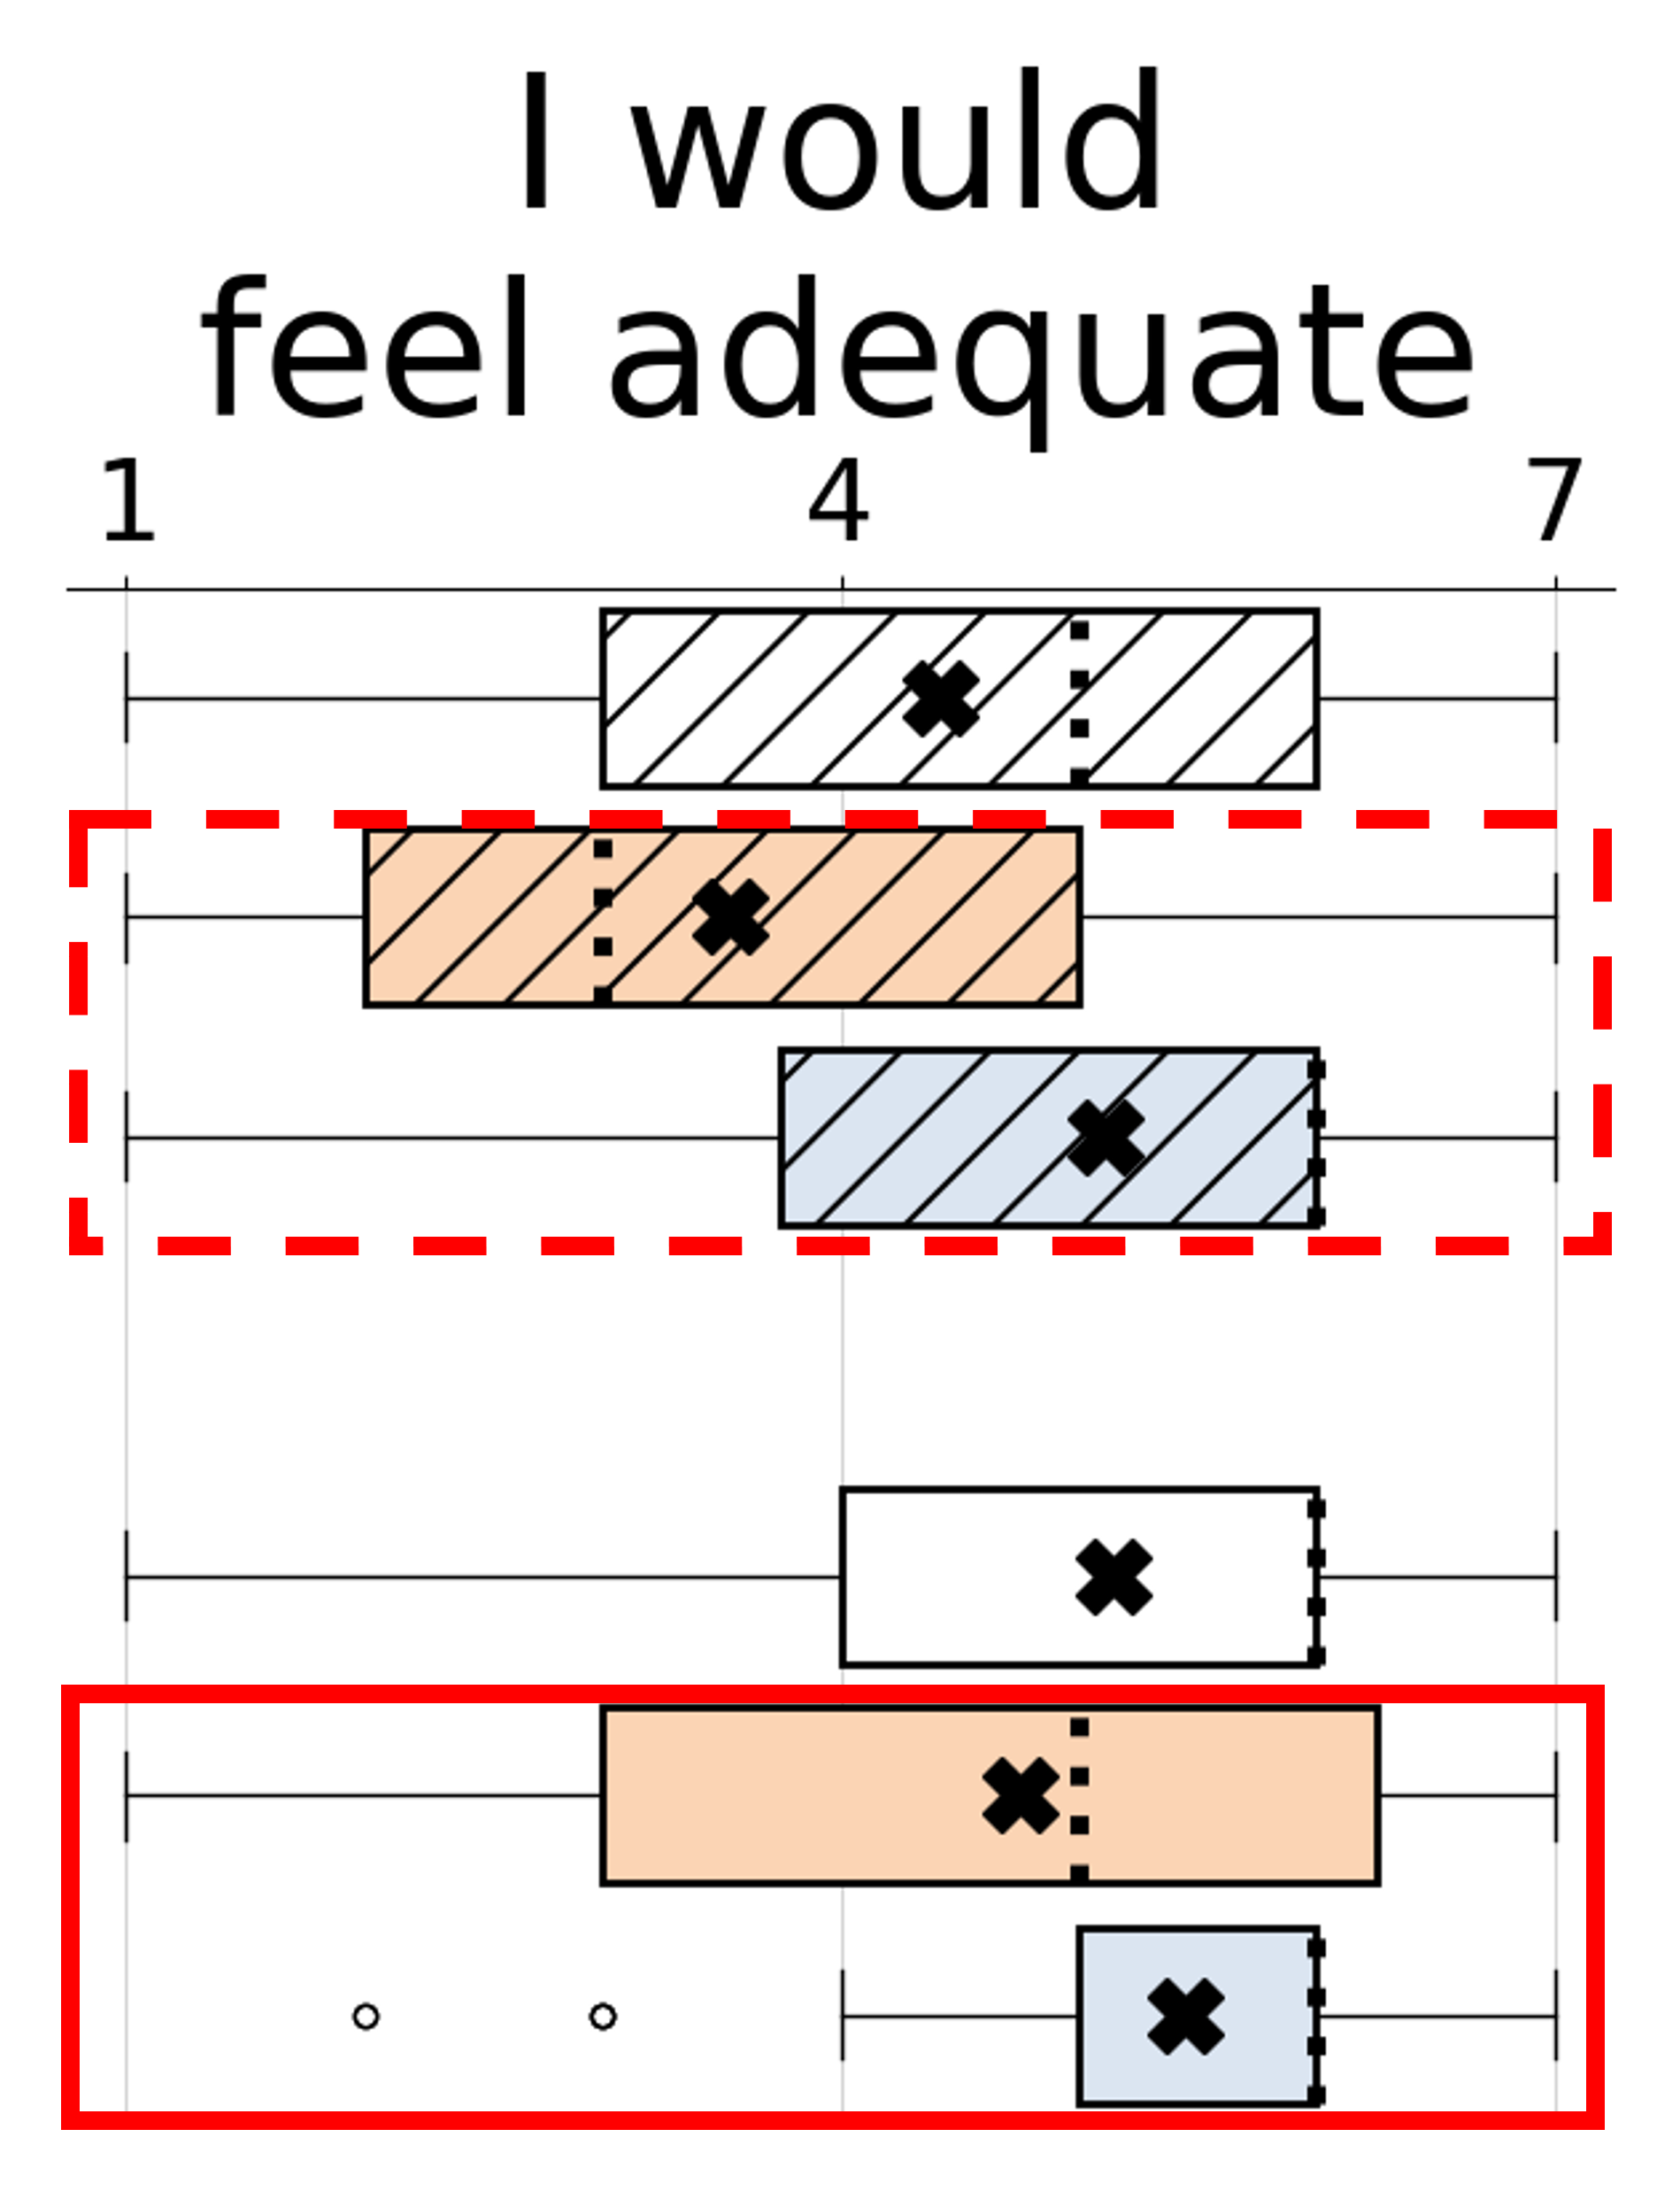}} &
    \multicolumn{2}{c|}{\includegraphics[width = 0.16\columnwidth]{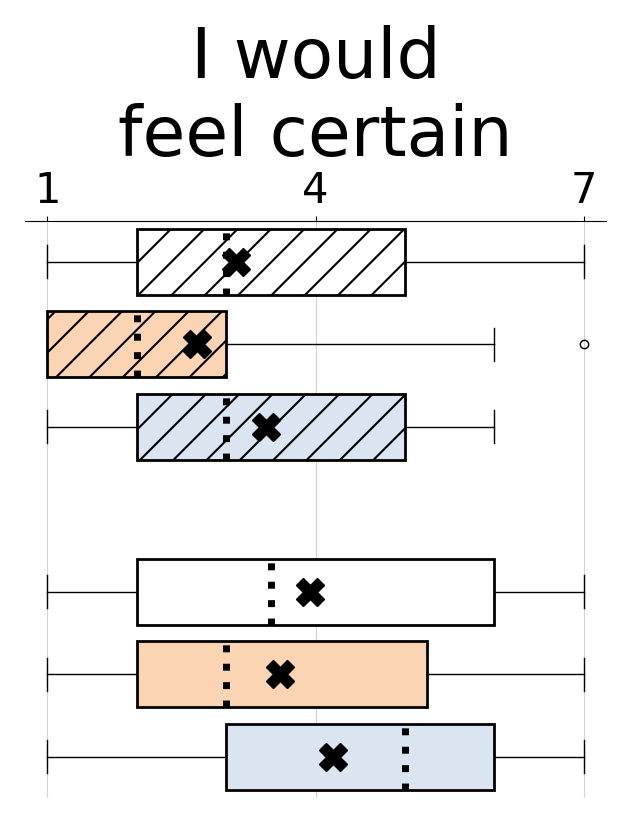}} &
    \multicolumn{2}{c}{\includegraphics[width = 0.16\columnwidth]{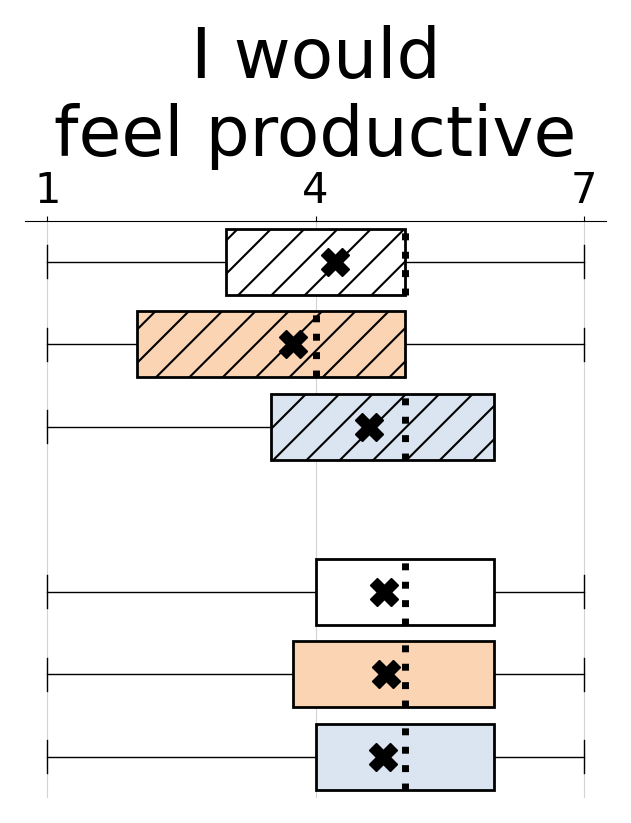}}
    \\
    \hline
    \hline
    \multicolumn{2}{c|}{\includegraphics[width = 0.16\columnwidth]{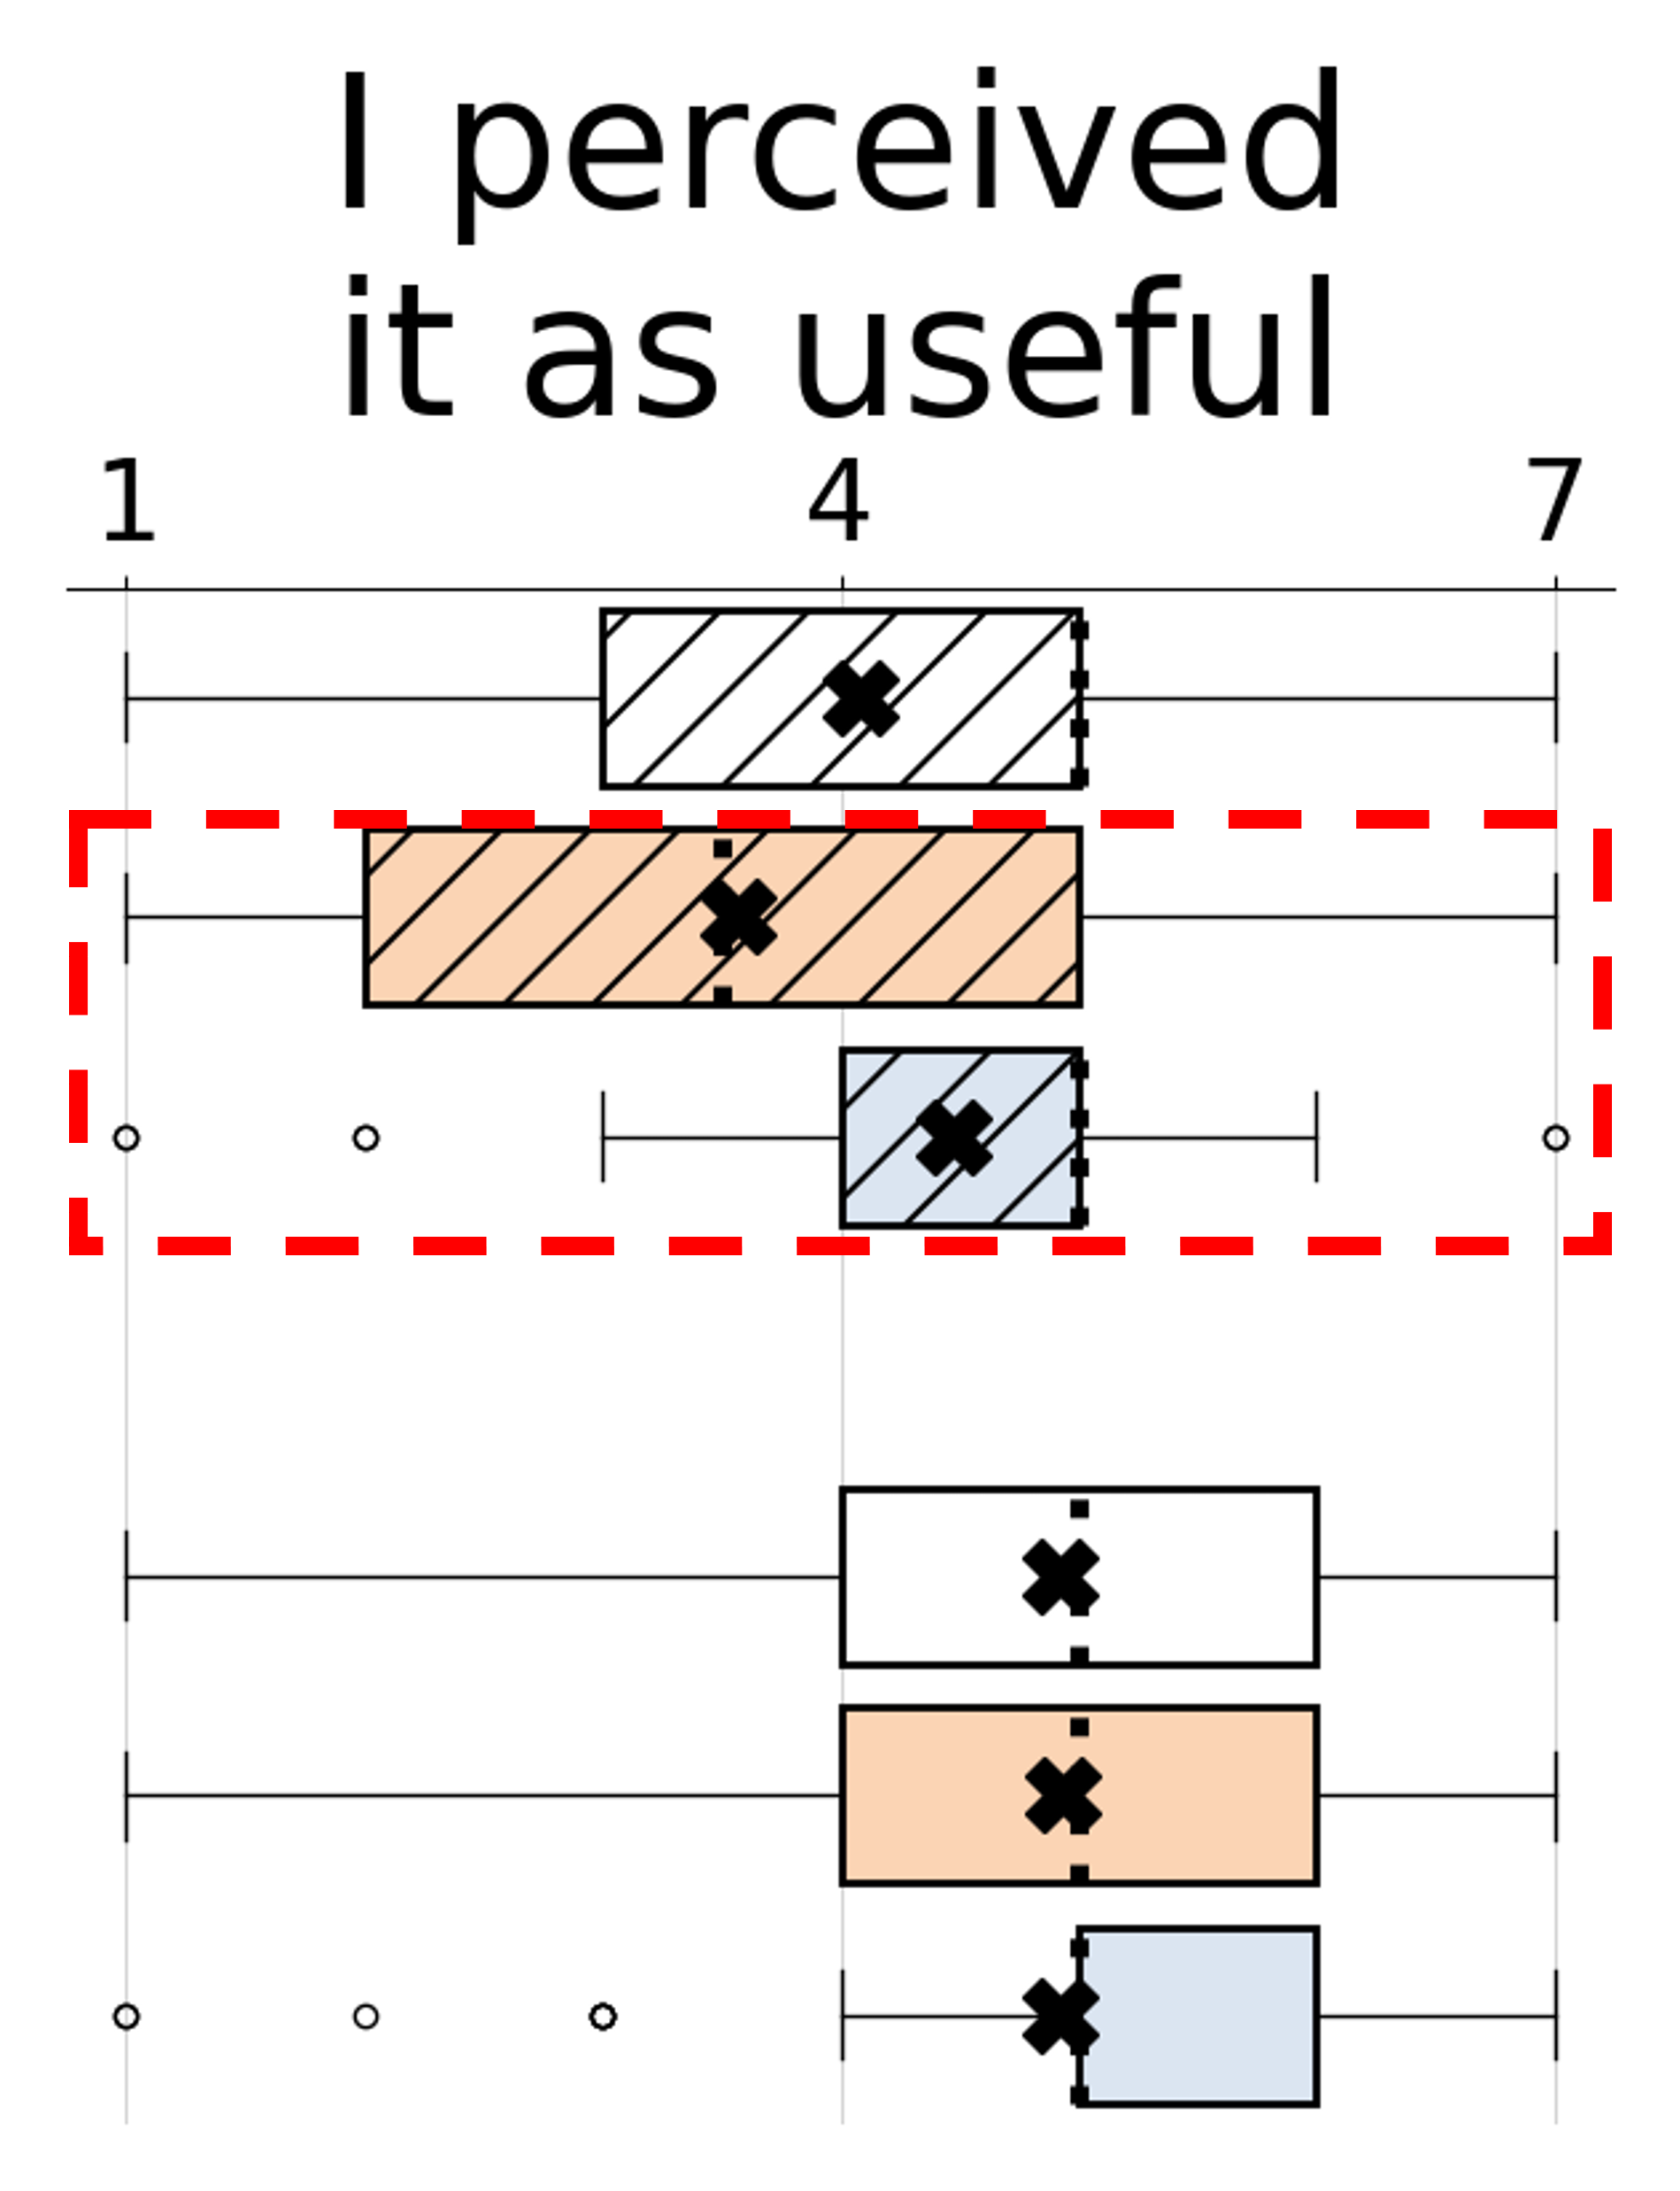}} &
    \multicolumn{2}{c|}{\includegraphics[width = 0.16\columnwidth]{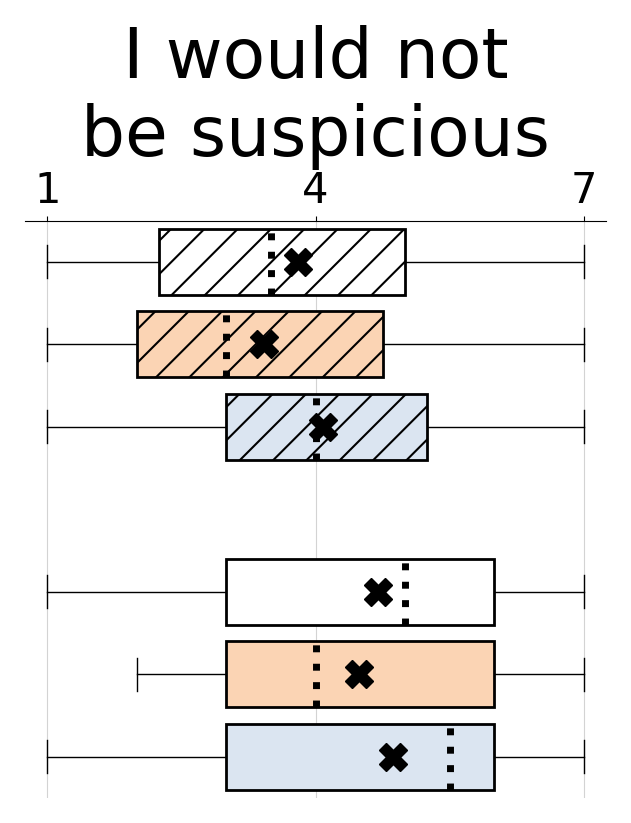}} &
    \multicolumn{2}{c|}{\includegraphics[width = 0.16\columnwidth]{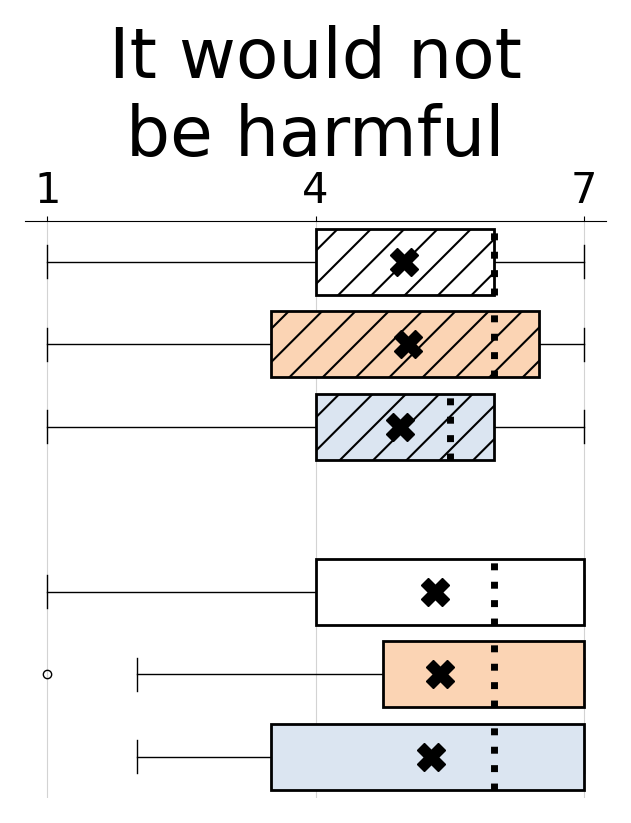}} &
    \multicolumn{2}{c|}{\includegraphics[width = 0.16\columnwidth]{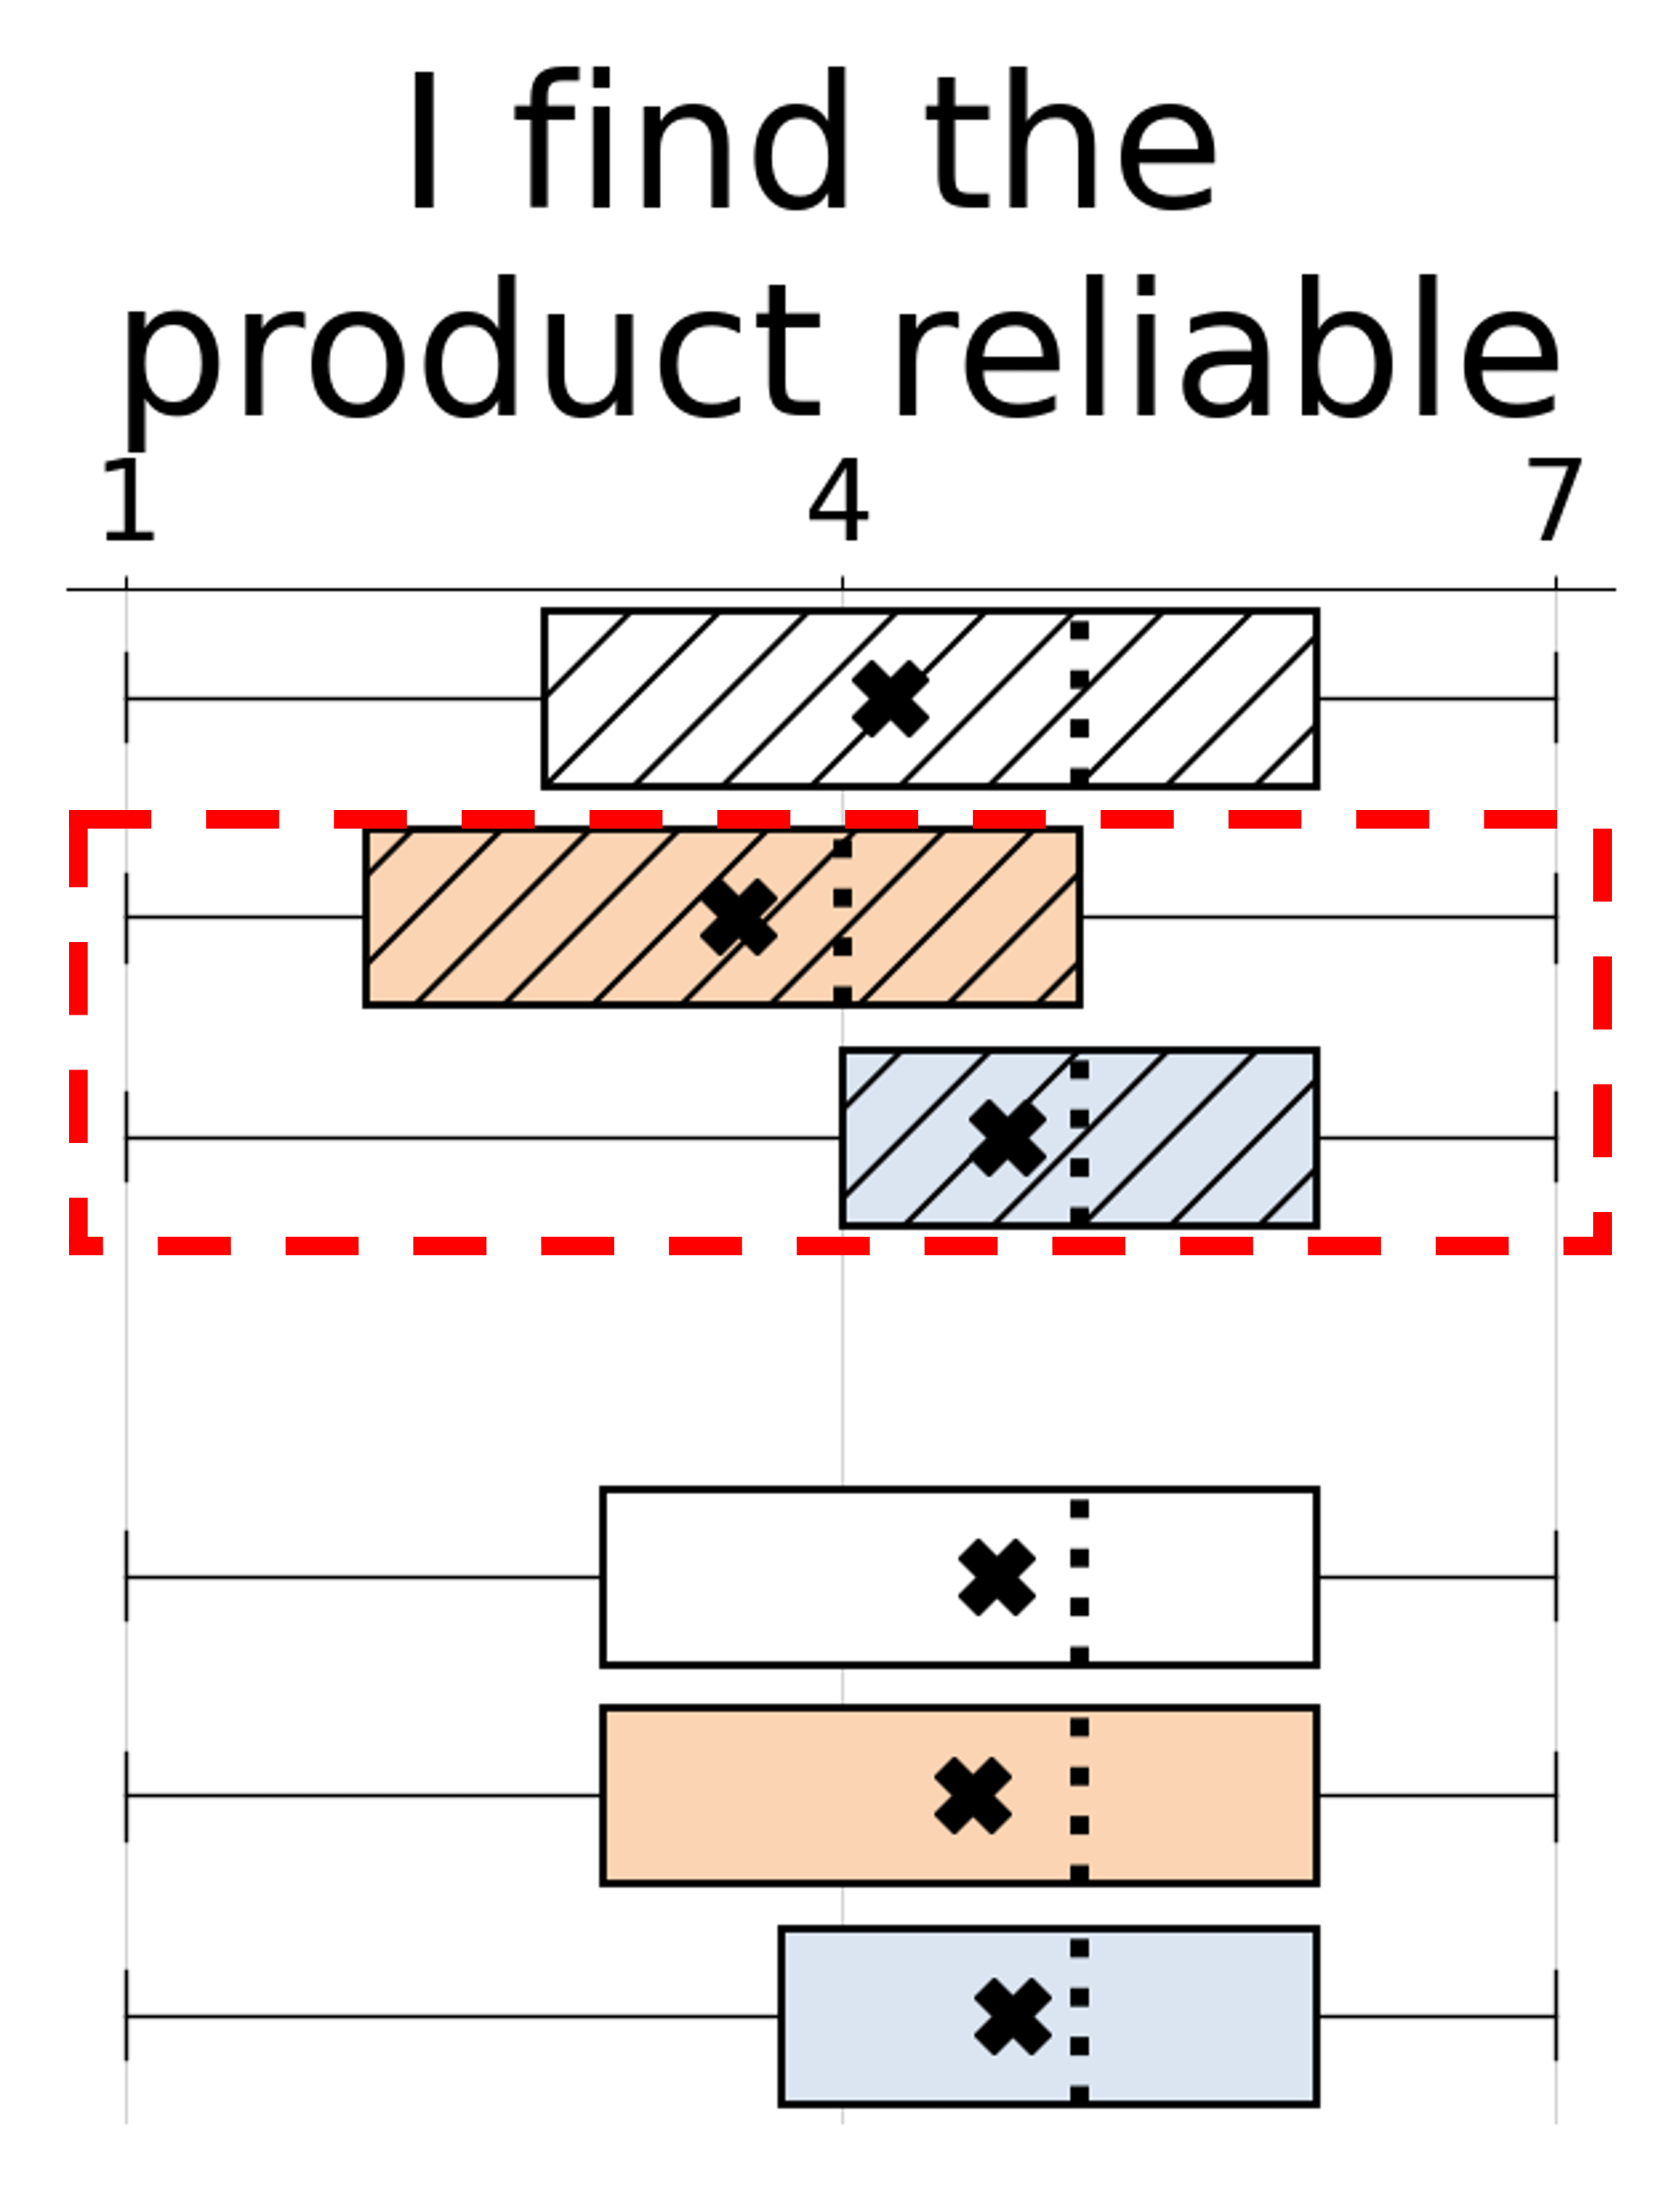}} &
    \multicolumn{2}{c}{\includegraphics[width = 0.16\columnwidth]{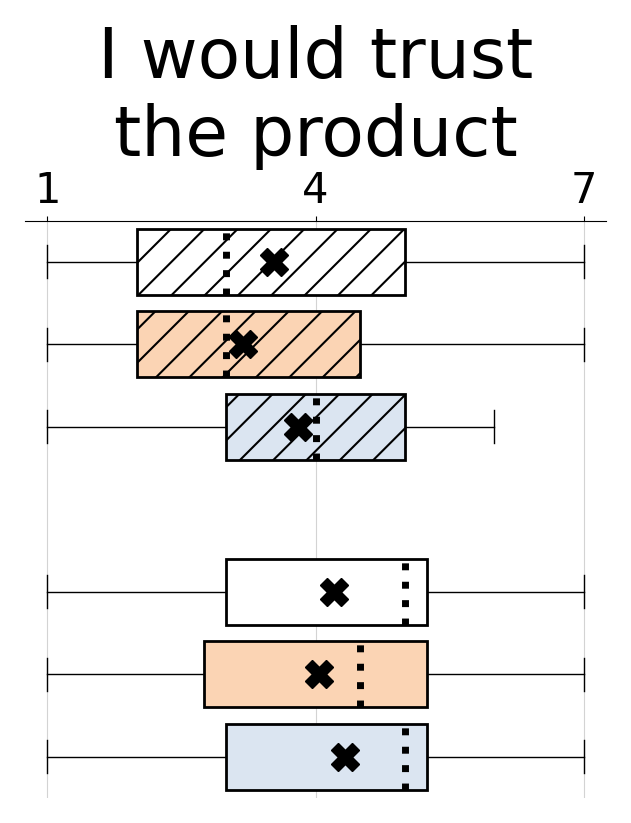}}
    \end{tabular}
    
    \caption{Guideline 15 participants' ratings for all dependent variables, disaggregated by participants' information processing styles.
	%For the disaggregated data, notice how large the distances between the average rating are when the guideline is applied.
	Table~\ref{tab:G15-Info-Stats-Appendix} below provides the statistics (where applicable).
}
    \label{fig:Info-G15-Appendix}
\end{table}

\begin{table}[h]

%\framebox[\linewidth]{For Measuring!}
\centering
\footnotesize

    \begin{tabular}{p{0.22\columnwidth}|c|c|c|c|c|c}
    
    \rowcolor{LightGray}\multicolumn{7}{c}{\textbf{Violation AI Product}}\\
    \hline
    \textbf{Dependent}  & \textbf{Distance b/w} &  &  & & \textbf{Bonferroni} &  \\
    \textbf{variable} & \textbf{Means} &  \textbf{df} &  \textbf{t-val} &   \textbf{p-value}  & \textbf{correction} & \textbf{Cohen's \textit{d}} \\
    \hline
    
    I would feel in control & - - - & - &  - - - & - - - & - - - & - - -  \\
    \hline
    
    I would feel secure & 1.0467 & 58 &  2.3627 & \cellcolor{AbiOrangeQuote}.0215 & - - - & 0.6104 \\
    \hline
    
    I would feel adequate & 1.9345 & 62 &  4.6196 & \cellcolor{AbiOrangeQuote}$<.0001$ & - - - & 1.1555 \\
    \hline
    
    I would feel certain & 0.8514 & 62 &  1.9515 & .0556 & - - - & 0.4881 \\
    \hline
    
    I would feel productive & - - - & - &  - - - & - - - & - - - & - - -   \\
    \hline
    \hline
    
    I perceived it as useful &  1.0371 & 62 &  2.4938 & \cellcolor{AbiOrangeQuote}.0153 & - - - & 0.6238   \\
    \hline
    
    I would not be suspicious & - - - & - &  - - - & - - - & - - - & - - -   \\
    \hline
    
    It would not be harmful & - - - & - &  - - - & - - - & - - - & - - -  \\
    \hline
    
    I find the product reliable & 1.4203 & 62 &  3.2775 & \cellcolor{AbiOrangeQuote}.0017 & - - - & 0.8198 \\
    \hline
    
    I would trust the product & - - - & - &  - - - & - - - & - - - & - - - \\
    \hline

    \rowcolor{LightGray}\multicolumn{7}{c}{\textbf{Application AI Product}}\\
    \hline
    \textbf{Dependent}  & \textbf{Distance b/w} &  &  & & \textbf{Bonferroni} &  \\
    \textbf{variable} & \textbf{Means} &  \textbf{df} &  \textbf{t-val} &   \textbf{p-value}  & \textbf{correction} & \textbf{Cohen's \textit{d}} \\
    \hline
    
    I would feel in control & - - - & - &  - - - & - - - & - - - & - - - \\
    \hline
    
    I would feel secure & - - - & - &  - - - & - - - & - - - & - - -\\
    \hline
    
    I would feel adequate & 0.9785 & 62 &  2.4170 & \cellcolor{AbiOrangeQuote}.0186 & - - - & 0.6045 \\
    \hline
    
    I would feel certain & - - - & - &  - - - & - - - & - - - & - - - \\
    \hline
    
    I would feel productive & - - - & - &  - - - & - - - & - - - & - - -   \\
    \hline
    \hline
    
    I perceived it as useful &  - - - & - &  - - - & - - - & - - - & - - -   \\
    \hline
    
    I would not be suspicious & - - - & - &  - - - & - - - & - - - & - - -   \\
    \hline
    
    It would not be harmful & - - - & - &  - - - & - - - & - - - & - - -  \\
    \hline
    
    I find the product reliable & - - - & - &  - - - & - - - & - - - & - - - \\
    \hline
    
    I would trust the product & - - - & - &  - - - & - - - & - - - & - - -

    \end{tabular}

    \caption{Guideline 15's t-test results %(\checkmark if Welch's t-test) 
    for comprehensive information processors vs. selective information processors participants' average ratings of the independent Violation AI product (top) and Application AI product (bottom), for all 10 dependent variables.
    If dashes (- - -) are present, no statistical test was performed.
    If the number of tests exceeded 5 for each product, Bonferroni correction applied by multiplying p-values by the number of tests performed.
    }
    \label{tab:G15-Info-Stats-Appendix}
\end{table}
\clearpage
%---------------------------------------------------- End Guideline 15

%Begin Guideline 17---------------------------------------------------

\begin{table}[]
    \centering
    \begin{tabular}{cc|cc|cc|cc|cc}
    \multicolumn{2}{c|}{\includegraphics[width = 0.16\columnwidth]{assets/05-All-BoxPlots/15-G17/Info/G17-Feel-In-Control-INFO.png}} &
    \multicolumn{2}{c|}{\includegraphics[width = 0.16\columnwidth]{assets/05-All-BoxPlots/15-G17/Info/G17-Feel-Secure-INFO.png}} &
    \multicolumn{2}{c|}{\includegraphics[width = 0.16\columnwidth]{assets/05-All-BoxPlots/15-G17/Info/G17-Feel-Adequate-INFO.png}} &
    \multicolumn{2}{c|}{\includegraphics[width = 0.16\columnwidth]{assets/05-All-BoxPlots/15-G17/Info/G17-Feel-Certain-INFO.png}} &
    \multicolumn{2}{c}{\includegraphics[width = 0.16\columnwidth]{assets/05-All-BoxPlots/15-G17/Info/G17-Feel-Productive-INFO.png}}
    \\
    \hline
    \hline
    \multicolumn{2}{c|}{\includegraphics[width = 0.16\columnwidth]{assets/05-All-BoxPlots/15-G17/Info/G17-Perceived-Useful-INFO.png}} &
    \multicolumn{2}{c|}{\includegraphics[width = 0.16\columnwidth]{assets/05-All-BoxPlots/15-G17/Info/G17-Not-Suspicious-INFO.png}} &
    \multicolumn{2}{c|}{\includegraphics[width = 0.16\columnwidth]{assets/05-All-BoxPlots/15-G17/Info/G17-Not-Harmful-INFO.png}} &
    \multicolumn{2}{c|}{\includegraphics[width = 0.16\columnwidth]{assets/05-All-BoxPlots/15-G17/Info/G17-Product-Reliable-INFO.png}} &
    \multicolumn{2}{c}{\includegraphics[width = 0.16\columnwidth]{assets/05-All-BoxPlots/15-G17/Info/G17-Trust-Product-INFO.png}}
    \end{tabular}
    
    \caption{Guideline 17 participants' ratings for all dependent variables, disaggregated by participants' information processing styles.
	%For the disaggregated data, notice how large the distances between the average rating are when the guideline is applied.
	Table~\ref{tab:G17-Info-Stats-Appendix} below provides the statistics (where applicable).
}
    \label{fig:Info-G17-Appendix}
\end{table}

\begin{table}[h]

%\framebox[\linewidth]{For Measuring!}
\centering
\footnotesize

    \begin{tabular}{p{0.22\columnwidth}|c|c|c|c|c|c}
    
    \rowcolor{LightGray}\multicolumn{7}{c}{\textbf{Violation AI Product}}\\
    \hline
    \textbf{Dependent}  & \textbf{Distance b/w} &  &  & & \textbf{Bonferroni} &  \\
    \textbf{variable} & \textbf{Means} &  \textbf{df} &  \textbf{t-val} &   \textbf{p-value}  & \textbf{correction} & \textbf{Cohen's \textit{d}} \\
    \hline
    
    I would feel in control & 0.7962 & 60 &  1.7738 & .0812 & - - - & 0.4527  \\
    \hline
    
    I would feel secure & - - - & - &  - - - & - - - & - - - & - - - \\
    \hline
    
    I would feel adequate & - - -  & - &  - - - & - - - & - - - & - - - \\
    \hline
    
    I would feel certain & - - - & - &  - - - & - - - & - - - & - - - \\
    \hline
    
    I would feel productive & - - - & - &  - - - & - - - & - - - & - - -   \\
    \hline
    \hline
    
    I perceived it as useful &  - - - & - &  - - - & - - - & - - - & - - -   \\
    \hline
    
    I would not be suspicious & 0.7511 & 58 &  1.7670 & .0825 & - - - & 0.4603   \\
    \hline
    
    It would not be harmful & - - - & - &  - - - & - - - & - - - & - - -  \\
    \hline
    
    I find the product reliable & - - - & - &  - - - & - - - & - - - & - - - \\
    \hline
    
    I would trust the product & 0.7089 & 61 &  1.9867 & .0515 & - - - & 0.5022 \\
    \hline

    \rowcolor{LightGray}\multicolumn{7}{c}{\textbf{Application AI Product}}\\
    \hline
    \textbf{Dependent}  & \textbf{Distance b/w} &  &  & & \textbf{Bonferroni} &  \\
    \textbf{variable} & \textbf{Means} &  \textbf{df} &  \textbf{t-val} &   \textbf{p-value}  & \textbf{correction} & \textbf{Cohen's \textit{d}} \\
    \hline
    
    I would feel in control & - - - & - &  - - - & - - - & - - - & - - -  \\
    \hline
    
    I would feel secure & - - - & - &  - - - & - - - & - - - & - - - \\
    \hline
    
    I would feel adequate & - - -  & - &  - - - & - - - & - - - & - - - \\
    \hline
    
    I would feel certain & - - - & - &  - - - & - - - & - - - & - - - \\
    \hline
    
    I would feel productive & - - - & - &  - - - & - - - & - - - & - - -   \\
    \hline
    \hline
    
    I perceived it as useful &  - - - & - &  - - - & - - - & - - - & - - -   \\
    \hline
    
    I would not be suspicious & - - - & - &  - - - & - - - & - - - & - - -   \\
    \hline
    
    It would not be harmful & - - - & - &  - - - & - - - & - - - & - - -  \\
    \hline
    
    I find the product reliable & - - - & - &  - - - & - - - & - - - & - - - \\
    \hline
    
    I would trust the product & - - - & - &  - - - & - - - & - - - & - - -

    \end{tabular}

    \caption{Guideline 17's t-test results %(\checkmark if Welch's t-test) 
    for comprehensive information processors vs. selective information processors participants' average ratings of the independent Violation AI product (top) and Application AI product (bottom), for all 10 dependent variables.
    If dashes (- - -) are present, no statistical test was performed.
    If the number of tests exceeded 5 for each product, Bonferroni correction applied by multiplying p-values by the number of tests performed.
    }
    \label{tab:G17-Info-Stats-Appendix}
\end{table}
\clearpage
%---------------------------------------------------- End Guideline 17

%Begin Guideline 17---------------------------------------------------

\begin{table}[]
    \centering
    \begin{tabular}{cc|cc|cc|cc|cc}
    \multicolumn{2}{c|}{\includegraphics[width = 0.16\columnwidth]{assets/05-All-BoxPlots/16-G18/Info/G18-Feel-In-Control-INFO.png}} &
    \multicolumn{2}{c|}{\includegraphics[width = 0.16\columnwidth]{assets/05-All-BoxPlots/16-G18/Info/G18-Feel-Secure-INFO.png}} &
    \multicolumn{2}{c|}{\includegraphics[width = 0.16\columnwidth]{assets/05-All-BoxPlots/16-G18/Info/G18-Feel-Adequate-INFO.png}} &
    \multicolumn{2}{c|}{\includegraphics[width = 0.16\columnwidth]{assets/05-All-BoxPlots/16-G18/Info/G18-Feel-Certain-INFO.png}} &
    \multicolumn{2}{c}{\includegraphics[width = 0.16\columnwidth]{assets/05-All-BoxPlots/16-G18/Info/G18-Feel-Productive-INFO.png}}
    \\
    \hline
    \hline
    \multicolumn{2}{c|}{\includegraphics[width = 0.16\columnwidth]{assets/05-All-BoxPlots/16-G18/Info/G18-Perceived-Useful-INFO.png}} &
    \multicolumn{2}{c|}{\includegraphics[width = 0.16\columnwidth]{assets/05-All-BoxPlots/16-G18/Info/G18-Not-Suspicious-INFO.png}} &
    \multicolumn{2}{c|}{\includegraphics[width = 0.16\columnwidth]{assets/05-All-BoxPlots/16-G18/Info/G18-Not-Harmful-INFO.png}} &
    \multicolumn{2}{c|}{\includegraphics[width = 0.16\columnwidth]{assets/05-All-BoxPlots/16-G18/Info/G18-Product-Reliable-INFO.png}} &
    \multicolumn{2}{c}{\includegraphics[width = 0.16\columnwidth]{assets/05-All-BoxPlots/16-G18/Info/G18-Trust-Product-INFO.png}}
    \end{tabular}
    
    \caption{Guideline 18 participants' ratings for all dependent variables, disaggregated by participants' information processing styles.
	%For the disaggregated data, notice how large the distances between the average rating are when the guideline is applied.
	Table~\ref{tab:G18-Info-Stats-Appendix} below provides the statistics (where applicable).
}
    \label{fig:Info-G18-Appendix}
\end{table}

\begin{table}[h]

%\framebox[\linewidth]{For Measuring!}
\centering
\footnotesize

    \begin{tabular}{p{0.22\columnwidth}|c|c|c|c|c|c}
    
    \rowcolor{LightGray}\multicolumn{7}{c}{\textbf{Violation AI Product}}\\
    \hline
    \textbf{Dependent}  & \textbf{Distance b/w} &  &  & & \textbf{Bonferroni} &  \\
    \textbf{variable} & \textbf{Means} &  \textbf{df} &  \textbf{t-val} &   \textbf{p-value}  & \textbf{correction} & \textbf{Cohen's \textit{d}} \\
    \hline
    
    I would feel in control & - - - & - &  - - - & - - - & - - - & - - -  \\
    \hline
    
    I would feel secure & - - - & - &  - - - & - - - & - - - & - - - \\
    \hline
    
    I would feel adequate & - - -  & - &  - - - & - - - & - - - & - - - \\
    \hline
    
    I would feel certain & - - - & - &  - - - & - - - & - - - & - - - \\
    \hline
    
    I would feel productive & - - - & - &  - - - & - - - & - - - & - - -   \\
    \hline
    \hline
    
    I perceived it as useful &  - - - & - &  - - - & - - - & - - - & - - -   \\
    \hline
    
    I would not be suspicious & - - - & - &  - - - & - - - & - - - & - - -   \\
    \hline
    
    It would not be harmful & - - - & - &  - - - & - - - & - - - & - - -  \\
    \hline
    
    I find the product reliable & - - - & - &  - - - & - - - & - - - & - - - \\
    \hline
    
    I would trust the product & - - - & - &  - - - & - - - & - - - & - - - \\
    \hline

    \rowcolor{LightGray}\multicolumn{7}{c}{\textbf{Application AI Product}}\\
    \hline
    \textbf{Dependent}  & \textbf{Distance b/w} &  &  & & \textbf{Bonferroni} &  \\
    \textbf{variable} & \textbf{Means} &  \textbf{df} &  \textbf{t-val} &   \textbf{p-value}  & \textbf{correction} & \textbf{Cohen's \textit{d}} \\
    \hline
    
    I would feel in control & - - - & - &  - - - & - - - & - - - & - - -  \\
    \hline
    
    I would feel secure & - - - & - &  - - - & - - - & - - - & - - - \\
    \hline
    
    I would feel adequate & - - -  & - &  - - - & - - - & - - - & - - - \\
    \hline
    
    I would feel certain & - - - & - &  - - - & - - - & - - - & - - - \\
    \hline
    
    I would feel productive & - - - & - &  - - - & - - - & - - - & - - -   \\
    \hline
    \hline
    
    I perceived it as useful &  - - - & - &  - - - & - - - & - - - & - - -   \\
    \hline
    
    I would not be suspicious & - - - & - &  - - - & - - - & - - - & - - -  \\
    \hline
    
    It would not be harmful & - - - & - &  - - - & - - - & - - - & - - -  \\
    \hline
    
    I find the product reliable & - - - & - &  - - - & - - - & - - - & - - - \\
    \hline
    
    I would trust the product & - - - & - &  - - - & - - - & - - - & - - -

    \end{tabular}

    \caption{Guideline 18's t-test results %(\checkmark if Welch's t-test) 
    for comprehensive information processors vs. selective information processors participants' average ratings of the independent Violation AI product (top) and Application AI product (bottom), for all 10 dependent variables.
    If dashes (- - -) are present, no statistical test was performed.
    If the number of tests exceeded 5 for each product, Bonferroni correction applied by multiplying p-values by the number of tests performed.
    }
    \label{tab:G18-Info-Stats-Appendix}
\end{table}
\clearpage
%---------------------------------------------------- End Guideline 18
