# Supplementary material for: Measuring User Experience Inclusivity in Human-AI Interaction via Five User Problem-Solving Styles
Source: arXiv:2108.00588 source file (2024-02-17)
Supplement: Supplementary file 9 [file Motiv-Appendix.tex]

%Guideline 1 ------------------------------
\begin{table}[]
    \centering
    \begin{tabular}{cc|cc|cc|cc|cc}
    \multicolumn{2}{c|}{\includegraphics[width = 0.16\columnwidth]{assets/05-All-BoxPlots/01-G1/Motiv/G1-Feel-In-Control-MOTIV.png}} &
    \multicolumn{2}{c|}{\includegraphics[width = 0.16\columnwidth]{assets/05-All-BoxPlots/01-G1/Motiv/G1-Feel-Secure-MOTIV.png}} &
    \multicolumn{2}{c|}{\includegraphics[width = 0.16\columnwidth]{assets/05-All-BoxPlots/01-G1/Motiv/G1-Feel-Adequate-MOTIV.png}} &
    \multicolumn{2}{c|}{\includegraphics[width = 0.16\columnwidth]{assets/05-All-BoxPlots/01-G1/Motiv/G1-Feel-Certain-MOTIV.png}} &
    \multicolumn{2}{c}{\includegraphics[width = 0.16\columnwidth]{assets/05-All-BoxPlots/01-G1/Motiv/G1-Feel-Productive-MOTIV.png}}
    \\
    \hline
    \hline
    \multicolumn{2}{c|}{\includegraphics[width = 0.16\columnwidth]{assets/05-All-BoxPlots/01-G1/Motiv/G1-Perceived-Useful-MOTIV.png}} &
    \multicolumn{2}{c|}{\includegraphics[width = 0.16\columnwidth]{assets/05-All-BoxPlots/01-G1/Motiv/G1-Not-Suspicious-MOTIV.png}} &
    \multicolumn{2}{c|}{\includegraphics[width = 0.16\columnwidth]{assets/05-All-BoxPlots/01-G1/Motiv/G1-Not-Harmful-MOTIV.png}} &
    \multicolumn{2}{c|}{\includegraphics[width = 0.16\columnwidth]{assets/05-All-BoxPlots/01-G1/Motiv/G1-Product-Reliable-MOTIV.png}} &
    \multicolumn{2}{c}{\includegraphics[width = 0.16\columnwidth]{assets/05-All-BoxPlots/01-G1/Motiv/G1-Trust-Product-MOTIV.png}}
    \end{tabular}
    
    \caption{Guideline 1 participants' ratings for all dependent variables, disaggregated by participants' motivations for using technology.
	%For the disaggregated data, notice how large the distances between the average rating are when the guideline is applied.
	Table~\ref{tab:G1-Motiv-Stats-Appendix} below provides the statistics (where applicable).
}
    \label{fig:Motiv-G1-Appendix}
\end{table}

\begin{table}[h]

%\framebox[\linewidth]{For Measuring!}
\centering
\footnotesize

    \begin{tabular}{p{0.22\columnwidth}|c|c|c|c|c|c}
    
    \rowcolor{LightGray}\multicolumn{7}{c}{\textbf{Violation AI Product}}\\
    \hline
    \textbf{Dependent}  & \textbf{Distance b/w} &  &  & & \textbf{Bonferroni} &  \\
    \textbf{variable} & \textbf{Means} &  \textbf{df} &  \textbf{t-val} &   \textbf{p-value}  & \textbf{correction} & \textbf{Cohen's \textit{d}} \\
    \hline
    
    I would feel in control & 0.5897 & 54 &  1.6816 & .0984 & - - - & 0.4506\\
    \hline
    
    I would feel secure & - - - & - &  - - - & - - - & - - - & - - - \\
    \hline
    
    I would feel adequate & - - - & - &  - - - & - - - & - - - & - - - \\
    \hline
    
    I would feel certain & - - - & - &  - - - & - - - & - - - & - - - \\
    \hline
    
    I would feel productive & - - - & - &  - - - & - - - & - - - & - - -  \\
    \hline
    \hline
    
    I perceived it as useful &  - - - & - &  - - - & - - - & - - - & - - -  \\
    \hline
    
    I would not be suspicious & - - - & - &  - - - & - - - & - - - & - - -  \\
    \hline
    
    It would not be harmful & - - - & - &  - - - & - - - & - - - & - - -  \\
    \hline
    
    I find the product reliable & - - - & - &  - - - & - - - & - - - & - - -  \\
    \hline
    
    I would trust the product & - - - & - &  - - - & - - - & - - - & - - - \\
    \hline

    \rowcolor{LightGray}\multicolumn{7}{c}{\textbf{Application AI Product}}\\
    \hline
    \textbf{Dependent}  & \textbf{Distance b/w} &  &  & & \textbf{Bonferroni} &  \\
    \textbf{variable} & \textbf{Means} &  \textbf{df} &  \textbf{t-val} &   \textbf{p-value}  & \textbf{correction} & \textbf{Cohen's \textit{d}} \\
    \hline
    
    I would feel in control & 0.6508 & 53 &  1.8361 & .0720 & - - - & 0.4952  \\
    \hline
    
    I would feel secure & - - - & - &  - - - & - - - & - - - & - - - \\
    \hline
    
    I would feel adequate & - - - & - &  - - - & - - - & - - - & - - - \\
    \hline
    
    I would feel certain & - - - & - &  - - - & - - - & - - - & - - - \\
    \hline
    
    I would feel productive & - - - & - &  - - - & - - - & - - - & - - -   \\
    \hline
    \hline
    
    I perceived it as useful &  - - - & - &  - - - & - - - & - - - & - - -  \\
    \hline
    
    I would not be suspicious & - - - & - &  - - - & - - - & - - - & - - -  \\
    \hline
    
    It would not be harmful & - - - & - &  - - - & - - - & - - - & - - -  \\
    \hline
    
    I find the product reliable & - - - & - &  - - - & - - - & - - - & - - - \\
    \hline
    
    I would trust the product & - - - & - &  - - - & - - - & - - - & - - -

    \end{tabular}

    \caption{Guideline 1's t-test results %(\checkmark if Welch's t-test) 
    for task-oriented vs. tech-oriented participants' average ratings of the independent Violation AI product (top) and Application AI product (bottom), for all 10 dependent variables.
    If dashes (- - -) are present, no statistical test was performed.
    If the number of tests exceeded 5 for each product, Bonferroni correction applied by multiplying p-values by the number of tests performed.
    }
    \label{tab:G1-Motiv-Stats-Appendix}
    
    % \FIXME{MMB@AAA: FYI, I took the \checkmark s out and replaced them with plain text, because the \checkmark vs blank visually stood out so much, I kept mis-seeing it as saying only those 4 rows were signif. or important.\\
    % AAA@MMB: Redid it with Y/N. The Welch's t and t were cluttering up the table too much.\\
    % MMB@AAA: I actually prefer the spelled-out way.  Visually, the table layout now screams WELCHES IS GOOD, and draws attention away from all other columns.  Meta-comment: it might help if you forced yourself to look at this paper with a reader hat on.}

\end{table}

\clearpage
%---------------------------------------------------- End Guideline 1

%Guideline 3 ------------------------------
\begin{table}[]
    \centering
    \begin{tabular}{cc|cc|cc|cc|cc}
    \multicolumn{2}{c|}{\includegraphics[width = 0.16\columnwidth]{assets/05-All-BoxPlots/02-G3/Motiv/G3-Feel-In-Control-MOTIV.png}} &
    \multicolumn{2}{c|}{\includegraphics[width = 0.16\columnwidth]{assets/05-All-BoxPlots/02-G3/Motiv/G3-Feel-Secure-MOTIV.png}} &
    \multicolumn{2}{c|}{\includegraphics[width = 0.16\columnwidth]{assets/05-All-BoxPlots/02-G3/Motiv/G3-Feel-Adequate-MOTIV.png}} &
    \multicolumn{2}{c|}{\includegraphics[width = 0.16\columnwidth]{assets/05-All-BoxPlots/02-G3/Motiv/G3-Feel-Certain-MOTIV.png}} &
    \multicolumn{2}{c}{\includegraphics[width = 0.16\columnwidth]{assets/05-All-BoxPlots/02-G3/Motiv/G3-Feel-Productive-MOTIV.png}}
    \\
    \hline
    \hline
    \multicolumn{2}{c|}{\includegraphics[width = 0.16\columnwidth]{assets/05-All-BoxPlots/02-G3/Motiv/G3-Perceived-Useful-MOTIV.png}} &
    \multicolumn{2}{c|}{\includegraphics[width = 0.16\columnwidth]{assets/05-All-BoxPlots/02-G3/Motiv/G3-Not-Suspicious-MOTIV.png}} &
    \multicolumn{2}{c|}{\includegraphics[width = 0.16\columnwidth]{assets/05-All-BoxPlots/02-G3/Motiv/G3-Not-Harmful-MOTIV.png}} &
    \multicolumn{2}{c|}{\includegraphics[width = 0.16\columnwidth]{assets/05-All-BoxPlots/02-G3/Motiv/G3-Product-Reliable-MOTIV.png}} &
    \multicolumn{2}{c}{\includegraphics[width = 0.16\columnwidth]{assets/05-All-BoxPlots/02-G3/Motiv/G3-Trust-Product-MOTIV.png}}
    \end{tabular}
    
    \caption{Guideline 3 participants' ratings for all dependent variables, disaggregated by participants' motivations for using technology.
	%For the disaggregated data, notice how large the distances between the average rating are when the guideline is applied.
	Table~\ref{tab:G3-Motiv-Stats-Appendix} below provides the statistics (where applicable).
}
    \label{fig:Motiv-G3-Appendix}
\end{table}

\begin{table}[h]

%\framebox[\linewidth]{For Measuring!}
\centering
\footnotesize

    \begin{tabular}{p{0.22\columnwidth}|c|c|c|c|c|c}
    
    \rowcolor{LightGray}\multicolumn{7}{c}{\textbf{Violation AI Product}}\\
    \hline
    \textbf{Dependent}  & \textbf{Distance b/w} &  &  & & \textbf{Bonferroni} &  \\
    \textbf{variable} & \textbf{Means} &  \textbf{df} &  \textbf{t-val} &   \textbf{p-value}  & \textbf{correction} & \textbf{Cohen's \textit{d}} \\
    \hline
    
    I would feel in control & - - - & - &  - - - & - - - & - - - & - - -\\
    \hline
    
    I would feel secure & - - - & - &  - - - & - - - & - - - & - - - \\
    \hline
    
    I would feel adequate & - - - & - &  - - - & - - - & - - - & - - - \\
    \hline
    
    I would feel certain & - - - & - &  - - - & - - - & - - - & - - - \\
    \hline
    
    I would feel productive & - - - & - &  - - - & - - - & - - - & - - -  \\
    \hline
    \hline
    
    I perceived it as useful &  - - - & - &  - - - & - - - & - - - & - - -  \\
    \hline
    
    I would not be suspicious & - - - & - &  - - - & - - - & - - - & - - -  \\
    \hline
    
    It would not be harmful & - - - & - &  - - - & - - - & - - - & - - -  \\
    \hline
    
    I find the product reliable & - - - & - &  - - - & - - - & - - - & - - -  \\
    \hline
    
    I would trust the product & - - - & - &  - - - & - - - & - - - & - - - \\
    \hline

    \rowcolor{LightGray}\multicolumn{7}{c}{\textbf{Application AI Product}}\\
    \hline
    \textbf{Dependent}  & \textbf{Distance b/w} &  &  & & \textbf{Bonferroni} &  \\
    \textbf{variable} & \textbf{Means} &  \textbf{df} &  \textbf{t-val} &   \textbf{p-value}  & \textbf{correction} & \textbf{Cohen's \textit{d}} \\
    \hline
    
    I would feel in control & - - - & - &  - - - & - - - & - - - & - - -  \\
    \hline
    
    I would feel secure & - - - & - &  - - - & - - - & - - - & - - - \\
    \hline
    
    I would feel adequate & - - - & - &  - - - & - - - & - - - & - - - \\
    \hline
    
    I would feel certain & - - - & - &  - - - & - - - & - - - & - - - \\
    \hline
    
    I would feel productive & - - - & - &  - - - & - - - & - - - & - - -   \\
    \hline
    \hline
    
    I perceived it as useful &  - - - & - &  - - - & - - - & - - - & - - -  \\
    \hline
    
    I would not be suspicious & - - - & - &  - - - & - - - & - - - & - - -  \\
    \hline
    
    It would not be harmful & - - - & - &  - - - & - - - & - - - & - - -  \\
    \hline
    
    I find the product reliable & - - - & - &  - - - & - - - & - - - & - - - \\
    \hline
    
    I would trust the product & 0.6364 & 66 &  1.8295 & .0718 & - - - & 0.4439

    \end{tabular}

    \caption{Guideline 3's t-test results %(\checkmark if Welch's t-test) 
    for task-oriented  vs. tech-oriented participants' average ratings of the independent Violation AI product (top) and Application AI product (bottom), for all 10 dependent variables.
    If dashes (- - -) are present, no statistical test was performed.
    If the number of tests exceeded 5 for each product, Bonferroni correction applied by multiplying p-values by the number of tests performed.
    }
    \label{tab:G3-Motiv-Stats-Appendix}
    
    % \FIXME{MMB@AAA: FYI, I took the \checkmark s out and replaced them with plain text, because the \checkmark vs blank visually stood out so much, I kept mis-seeing it as saying only those 4 rows were signif. or important.\\
    % AAA@MMB: Redid it with Y/N. The Welch's t and t were cluttering up the table too much.\\
    % MMB@AAA: I actually prefer the spelled-out way.  Visually, the table layout now screams WELCHES IS GOOD, and draws attention away from all other columns.  Meta-comment: it might help if you forced yourself to look at this paper with a reader hat on.}

\end{table}

\clearpage
%---------------------------------------------------- End Guideline 3

%Begin Guideline 4----------------------------------------------------

\begin{table}[]
    \centering
    \begin{tabular}{cc|cc|cc|cc|cc}
    \multicolumn{2}{c|}{\includegraphics[width = 0.16\columnwidth]{assets/05-All-BoxPlots/03-G4/Motiv/G4-Feel-In-Control-MOTIV.png}} &
    \multicolumn{2}{c|}{\includegraphics[width = 0.16\columnwidth]{assets/05-All-BoxPlots/03-G4/Motiv/G4-Feel-Secure-MOTIV.png}} &
    \multicolumn{2}{c|}{\includegraphics[width = 0.16\columnwidth]{assets/05-All-BoxPlots/03-G4/Motiv/G4-Feel-Adequate-MOTIV.png}} &
    \multicolumn{2}{c|}{\includegraphics[width = 0.16\columnwidth]{assets/05-All-BoxPlots/03-G4/Motiv/G4-Feel-Certain-MOTIV.png}} &
    \multicolumn{2}{c}{\includegraphics[width = 0.16\columnwidth]{assets/05-All-BoxPlots/03-G4/Motiv/G4-Feel-Productive-MOTIV.png}}
    \\
    \hline
    \hline
    \multicolumn{2}{c|}{\includegraphics[width = 0.16\columnwidth]{assets/05-All-BoxPlots/03-G4/Motiv/G4-Perceived-Useful-MOTIV.png}} &
    \multicolumn{2}{c|}{\includegraphics[width = 0.16\columnwidth]{assets/05-All-BoxPlots/03-G4/Motiv/G4-Not-Suspicious-MOTIV.png}} &
    \multicolumn{2}{c|}{\includegraphics[width = 0.16\columnwidth]{assets/05-All-BoxPlots/03-G4/Motiv/G4-Not-Harmful-MOTIV.png}} &
    \multicolumn{2}{c|}{\includegraphics[width = 0.16\columnwidth]{assets/05-All-BoxPlots/03-G4/Motiv/G4-Product-Reliable-MOTIV.png}} &
    \multicolumn{2}{c}{\includegraphics[width = 0.16\columnwidth]{assets/05-All-BoxPlots/03-G4/Motiv/G4-Trust-Product-MOTIV.png}}
    \end{tabular}
    
    \caption{Guideline 4 participants' ratings for all dependent variables, disaggregated by participants' motivations for using technology.
	%For the disaggregated data, notice how large the distances between the average rating are when the guideline is applied.
	Table~\ref{tab:G4-Motiv-Stats-Appendix} below provides the statistics (where applicable).
}
    \label{fig:Motiv-G4-Appendix}
\end{table}

\begin{table}[h]

%\framebox[\linewidth]{For Measuring!}
\centering
\footnotesize

    \begin{tabular}{p{0.22\columnwidth}|c|c|c|c|c|c}
    
    \rowcolor{LightGray}\multicolumn{7}{c}{\textbf{Violation AI Product}}\\
    \hline
    \textbf{Dependent}  & \textbf{Distance b/w} &  &  & & \textbf{Bonferroni} &  \\
    \textbf{variable} & \textbf{Means} &  \textbf{df} &  \textbf{t-val} &   \textbf{p-value}  & \textbf{correction} & \textbf{Cohen's \textit{d}} \\
    \hline
    
    I would feel in control & - - - & - &  - - - & - - - & - - - & - - - \\
    \hline
    
    I would feel secure & - - - & - &  - - - & - - - & - - - & - - - \\
    \hline
    
    I would feel adequate & - - - & - &  - - - & - - - & - - - & - - - \\
    \hline
    
    I would feel certain & - - - & - &  - - - & - - - & - - - & - - - \\
    \hline
    
    I would feel productive & - - - & - &  - - - & - - - & - - - & - - -  \\
    \hline
    \hline
    
    I perceived it as useful &  - - - & - &  - - - & - - - & - - - & - - -  \\
    \hline
    
    I would not be suspicious & - - - & - &  - - - & - - - & - - - & - - -  \\
    \hline
    
    It would not be harmful & - - - & - &  - - - & - - - & - - - & - - -  \\
    \hline
    
    I find the product reliable &- - - & - &  - - - & - - - & - - - & - - -  \\
    \hline
    
    I would trust the product & - - - & - &  - - - & - - - & - - - & - - - \\
    \hline

    \rowcolor{LightGray}\multicolumn{7}{c}{\textbf{Application AI Product}}\\
    \hline
    \textbf{Dependent}  & \textbf{Distance b/w} &  &  & & \textbf{Bonferroni} &  \\
    \textbf{variable} & \textbf{Means} &  \textbf{df} &  \textbf{t-val} &   \textbf{p-value}  & \textbf{correction} & \textbf{Cohen's \textit{d}} \\
    \hline
    
    I would feel in control & - - - & - &  - - - & - - - & - - - & - - -  \\
    \hline
    
    I would feel secure & - - - & - &  - - - & - - - & - - - & - - - \\
    \hline
    
    I would feel adequate & - - - & - &  - - - & - - - & - - - & - - - \\
    \hline
    
    I would feel certain & - - - & - &  - - - & - - - & - - - & - - - \\
    \hline
    
    I would feel productive & - - - & - &  - - - & - - - & - - - & - - -   \\
    \hline
    \hline
    
    I perceived it as useful &  - - - & - &  - - - & - - - & - - - & - - -   \\
    \hline
    
    I would not be suspicious & - - - & - &  - - - & - - - & - - - & - - -   \\
    \hline
    
    It would not be harmful & - - - & - &  - - - & - - - & - - - & - - - \\
    \hline
    
    I find the product reliable & - - - & - &  - - - & - - - & - - - & - - - \\
    \hline
    
    I would trust the product & - - - & - &  - - - & - - - & - - - & - - -

    \end{tabular}

    \caption{Guideline 4's t-test results %(\checkmark if Welch's t-test) 
    for task-oriented vs. tech-oriented participants' average ratings of the independent Violation AI product (top) and Application AI product (bottom), for all 10 dependent variables.
    If dashes (- - -) are present, no statistical test was performed.
    If the number of tests exceeded 5 for each product, Bonferroni correction applied by multiplying p-values by the number of tests performed.
    }
    \label{tab:G4-Motiv-Stats-Appendix}
\end{table}

%---------------------------------------------------- End Guideline 4

\clearpage

%Begin Guideline 5----------------------------------------------------

\begin{table}[]
    \centering
    \begin{tabular}{cc|cc|cc|cc|cc}
    \multicolumn{2}{c|}{\includegraphics[width = 0.16\columnwidth]{assets/05-All-BoxPlots/04-G5/Motiv/G5-Feel-In-Control-MOTIV.png}} &
    \multicolumn{2}{c|}{\includegraphics[width = 0.16\columnwidth]{assets/05-All-BoxPlots/04-G5/Motiv/G5-Feel-Secure-MOTIV.png}} &
    \multicolumn{2}{c|}{\includegraphics[width = 0.16\columnwidth]{assets/05-All-BoxPlots/04-G5/Motiv/G5-Feel-Adequate-MOTIV.png}} &
    \multicolumn{2}{c|}{\includegraphics[width = 0.16\columnwidth]{assets/05-All-BoxPlots/04-G5/Motiv/G5-Feel-Certain-MOTIV.png}} &
    \multicolumn{2}{c}{\includegraphics[width = 0.16\columnwidth]{assets/05-All-BoxPlots/04-G5/Motiv/G5-Feel-Productive-MOTIV.png}}
    \\
    \hline
    \hline
    \multicolumn{2}{c|}{\includegraphics[width = 0.16\columnwidth]{assets/05-All-BoxPlots/04-G5/Motiv/G5-Perceived-Useful-MOTIV.png}} &
    \multicolumn{2}{c|}{\includegraphics[width = 0.16\columnwidth]{assets/05-All-BoxPlots/04-G5/Motiv/G5-Not-Suspicious-MOTIV.png}} &
    \multicolumn{2}{c|}{\includegraphics[width = 0.16\columnwidth]{assets/05-All-BoxPlots/04-G5/Motiv/G5-Not-Harmful-MOTIV.png}} &
    \multicolumn{2}{c|}{\includegraphics[width = 0.16\columnwidth]{assets/05-All-BoxPlots/04-G5/Motiv/G5-Product-Reliable-MOTIV.png}} &
    \multicolumn{2}{c}{\includegraphics[width = 0.16\columnwidth]{assets/05-All-BoxPlots/04-G5/Motiv/G5-Trust-Product-MOTIV.png}}
    \end{tabular}
    
    \caption{Guideline 5 participants' ratings for all dependent variables, disaggregated by participants' motivations for using technology.
	%For the disaggregated data, notice how large the distances between the average rating are when the guideline is applied.
	Table~\ref{tab:G5-Motiv-Stats-Appendix} below provides the statistics (where applicable).
}
    \label{fig:Motiv-G5-Appendix}
\end{table}

\begin{table}[h]

%\framebox[\linewidth]{For Measuring!}
\centering
\footnotesize

    \begin{tabular}{p{0.22\columnwidth}|c|c|c|c|c|c}
    
    \rowcolor{LightGray}\multicolumn{7}{c}{\textbf{Violation AI Product}}\\
    \hline
    \textbf{Dependent}  & \textbf{Distance b/w} &  &  & & \textbf{Bonferroni} &  \\
    \textbf{variable} & \textbf{Means} &  \textbf{df} &  \textbf{t-val} &   \textbf{p-value}  & \textbf{correction} & \textbf{Cohen's \textit{d}} \\
    \hline
    
    I would feel in control & - - - & - &  - - - & - - - & - - - & - - - \\
    \hline
    
    I would feel secure & - - - & - &  - - - & - - - & - - - & - - - \\
    \hline
    
    I would feel adequate & - - - & - &  - - - & - - - & - - - & - - - \\
    \hline
    
    I would feel certain & - - - & - &  - - - & - - - & - - - & - - - \\
    \hline
    
    I would feel productive & - - - & - &  - - - & - - - & - - - & - - -  \\
    \hline
    \hline
    
    I perceived it as useful &  - - - & - &  - - - & - - - & - - - & - - -  \\
    \hline
    
    I would not be suspicious & - - - & - &  - - - & - - - & - - - & - - -  \\
    \hline
    
    It would not be harmful & - - - & - &  - - - & - - - & - - - & - - -  \\
    \hline
    
    I find the product reliable & - - - & - &  - - - & - - - & - - - & - - -  \\
    \hline
    
    I would trust the product & 0.7227 & 67 &  1.9950 & .0501 & - - - & 0.4804 \\
    \hline

    \rowcolor{LightGray}\multicolumn{7}{c}{\textbf{Application AI Product}}\\
    \hline
    \textbf{Dependent}  & \textbf{Distance b/w} &  &  & & \textbf{Bonferroni} &  \\
    \textbf{variable} & \textbf{Means} &  \textbf{df} &  \textbf{t-val} &   \textbf{p-value}  & \textbf{correction} & \textbf{Cohen's \textit{d}} \\
    \hline
    
    I would feel in control & - - - & - &  - - - & - - - & - - - & - - - \\
    \hline
    
    I would feel secure & - - - & - &  - - - & - - - & - - - & - - - \\
    \hline
    
    I would feel adequate & - - - & - &  - - - & - - - & - - - & - - - \\
    \hline
    
    I would feel certain & - - - & - &  - - - & - - - & - - - & - - - \\
    \hline
    
    I would feel productive & - - - & - &  - - - & - - - & - - - & - - -    \\
    \hline
    \hline
    
    I perceived it as useful &  - - - & - &  - - - & - - - & - - - & - - -   \\
    \hline
    
    I would not be suspicious & - - - & - &  - - - & - - - & - - - & - - -   \\
    \hline
    
    It would not be harmful & - - - & - &  - - - & - - - & - - - & - - -  \\
    \hline
    
    I find the product reliable & - - - & - &  - - - & - - - & - - - & - - - \\
    \hline
    
    I would trust the product & - - - & - &  - - - & - - - & - - - & - - -

    \end{tabular}

    \caption{Guideline 5's t-test results %(\checkmark if Welch's t-test) 
    for task-oriented vs. tech-oriented participants' average ratings of the independent Violation AI product (top) and Application AI product (bottom), for all 10 dependent variables.
    If dashes (- - -) are present, no statistical test was performed.
    If the number of tests exceeded 5 for each product, Bonferroni correction applied by multiplying p-values by the number of tests performed.
    }
    \label{tab:G5-Motiv-Stats-Appendix}
\end{table}

%---------------------------------------------------- End Guideline 5

\clearpage

%Begin Guideline 6----------------------------------------------------

\begin{table}[]
    \centering
    \begin{tabular}{cc|cc|cc|cc|cc}
    \multicolumn{2}{c|}{\includegraphics[width = 0.16\columnwidth]{assets/05-All-BoxPlots/05-G6/Motiv/G6-Feel-In-Control-MOTIV.png}} &
    \multicolumn{2}{c|}{\includegraphics[width = 0.16\columnwidth]{assets/05-All-BoxPlots/05-G6/Motiv/G6-Feel-Secure-MOTIV.png}} &
    \multicolumn{2}{c|}{\includegraphics[width = 0.16\columnwidth]{assets/05-All-BoxPlots/05-G6/Motiv/G6-Feel-Adequate-MOTIV.png}} &
    \multicolumn{2}{c|}{\includegraphics[width = 0.16\columnwidth]{assets/05-All-BoxPlots/05-G6/Motiv/G6-Feel-Certain-MOTIV.png}} &
    \multicolumn{2}{c}{\includegraphics[width = 0.16\columnwidth]{assets/05-All-BoxPlots/05-G6/Motiv/G6-Feel-Productive-MOTIV.png}}
    \\
    \hline
    \hline
    \multicolumn{2}{c|}{\includegraphics[width = 0.16\columnwidth]{assets/05-All-BoxPlots/05-G6/Motiv/G6-Perceived-Useful-MOTIV.png}} &
    \multicolumn{2}{c|}{\includegraphics[width = 0.16\columnwidth]{assets/05-All-BoxPlots/05-G6/Motiv/G6-Not-Suspicious-MOTIV.png}} &
    \multicolumn{2}{c|}{\includegraphics[width = 0.16\columnwidth]{assets/05-All-BoxPlots/05-G6/Motiv/G6-Not-Harmful-MOTIV.png}} &
    \multicolumn{2}{c|}{\includegraphics[width = 0.16\columnwidth]{assets/05-All-BoxPlots/05-G6/Motiv/G6-Product-Reliable-MOTIV.png}} &
    \multicolumn{2}{c}{\includegraphics[width = 0.16\columnwidth]{assets/05-All-BoxPlots/05-G6/Motiv/G6-Trust-Product-MOTIV.png}}
    \end{tabular}
    
    \caption{Guideline 6 participants' ratings for all dependent variables, disaggregated by participants' motivations for using technology.
	%For the disaggregated data, notice how large the distances between the average rating are when the guideline is applied.
	Table~\ref{tab:G6-Motiv-Stats-Appendix} below provides the statistics (where applicable).
}
    \label{fig:Motiv-G6-Appendix}
\end{table}

\begin{table}[h]

%\framebox[\linewidth]{For Measuring!}
\centering
\footnotesize

    \begin{tabular}{p{0.22\columnwidth}|c|c|c|c|c|c}
    
    \rowcolor{LightGray}\multicolumn{7}{c}{\textbf{Violation AI Product}}\\
    \hline
    \textbf{Dependent}  & \textbf{Distance b/w} &  &  & & \textbf{Bonferroni} &  \\
    \textbf{variable} & \textbf{Means} &  \textbf{df} &  \textbf{t-val} &   \textbf{p-value}  & \textbf{correction} & \textbf{Cohen's \textit{d}} \\
    \hline
    
    I would feel in control & - - - & - &  - - - & - - - & - - - & - - -  \\
    \hline
    
    I would feel secure & - - - & - &  - - - & - - - & - - - & - - - \\
    \hline
    
    I would feel adequate & - - - & - &  - - - & - - - & - - - & - - - \\
    \hline
    
    I would feel certain & - - - & - &  - - - & - - - & - - - & - - - \\
    \hline
    
    I would feel productive & - - - & - &  - - - & - - - & - - - & - - -    \\
    \hline
    \hline
    
    I perceived it as useful &  - - - & - &  - - - & - - - & - - - & - - -   \\
    \hline
    
    I would not be suspicious & - - - & - &  - - - & - - - & - - - & - - -   \\
    \hline
    
    It would not be harmful & - - - & - &  - - - & - - - & - - - & - - -  \\
    \hline
    
    I find the product reliable & - - - & - &  - - - & - - - & - - - & - - - \\
    \hline
    
    I would trust the product & - - - & - &  - - - & - - - & - - - & - - - \\
    \hline

    \rowcolor{LightGray}\multicolumn{7}{c}{\textbf{Application AI Product}}\\
    \hline
    \textbf{Dependent}  & \textbf{Distance b/w} &  &  & & \textbf{Bonferroni} &  \\
    \textbf{variable} & \textbf{Means} &  \textbf{df} &  \textbf{t-val} &   \textbf{p-value}  & \textbf{correction} & \textbf{Cohen's \textit{d}} \\
    \hline
    
    I would feel in control & - - - & - &  - - - & - - - & - - - & - - -  \\
    \hline
    
    I would feel secure & - - - & - &  - - - & - - - & - - - & - - - \\
    \hline
    
    I would feel adequate & 0.6389 & 62 &  1.6736 & .0992 & - - - & 0.4217 \\
    \hline
    
    I would feel certain & - - - & - &  - - - & - - - & - - - & - - - \\
    \hline
    
    I would feel productive & - - - & - &  - - - & - - - & - - - & - - -    \\
    \hline
    \hline
    
    I perceived it as useful &  - - - & - &  - - - & - - - & - - - & - - -   \\
    \hline
    
    I would not be suspicious & - - - & - &  - - - & - - - & - - - & - - -   \\
    \hline
    
    It would not be harmful & - - - & - &  - - - & - - - & - - - & - - -  \\
    \hline
    
    I find the product reliable & 0.6389 & 61 &  1.7643 & .0827 & - - - & 0.4492 \\
    \hline
    
    I would trust the product & - - - & - &  - - - & - - - & - - - & - - -

    \end{tabular}

    \caption{Guideline 6's t-test results %(\checkmark if Welch's t-test) 
    for task-oriented vs. tech-oriented participants' average ratings of the independent Violation AI product (top) and Application AI product (bottom), for all 10 dependent variables.
    If dashes (- - -) are present, no statistical test was performed.
    If the number of tests exceeded 5 for each product, Bonferroni correction applied by multiplying p-values by the number of tests performed.
    }
    \label{tab:G6-Motiv-Stats-Appendix}
\end{table}

%---------------------------------------------------- End Guideline 6

\clearpage

%Begin Guideline 7----------------------------------------------------

\begin{table}[]
    \centering
    \begin{tabular}{cc|cc|cc|cc|cc}
    \multicolumn{2}{c|}{\includegraphics[width = 0.16\columnwidth]{assets/05-All-BoxPlots/06-G7/Motiv/G7-Feel-In-Control-MOTIV.png}} &
    \multicolumn{2}{c|}{\includegraphics[width = 0.16\columnwidth]{assets/05-All-BoxPlots/06-G7/Motiv/G7-Feel-Secure-MOTIV.png}} &
    \multicolumn{2}{c|}{\includegraphics[width = 0.16\columnwidth]{assets/05-All-BoxPlots/06-G7/Motiv/G7-Feel-Adequate-MOTIV.png}} &
    \multicolumn{2}{c|}{\includegraphics[width = 0.16\columnwidth]{assets/05-All-BoxPlots/06-G7/Motiv/G7-Feel-Certain-MOTIV.png}} &
    \multicolumn{2}{c}{\includegraphics[width = 0.16\columnwidth]{assets/05-All-BoxPlots/06-G7/Motiv/G7-Feel-Productive-MOTIV.png}}
    \\
    \hline
    \hline
    \multicolumn{2}{c|}{\includegraphics[width = 0.16\columnwidth]{assets/05-All-BoxPlots/06-G7/Motiv/G7-Perceived-Useful-MOTIV.png}} &
    \multicolumn{2}{c|}{\includegraphics[width = 0.16\columnwidth]{assets/05-All-BoxPlots/06-G7/Motiv/G7-Not-Suspicious-MOTIV.png}} &
    \multicolumn{2}{c|}{\includegraphics[width = 0.16\columnwidth]{assets/05-All-BoxPlots/06-G7/Motiv/G7-Not-Harmful-MOTIV.png}} &
    \multicolumn{2}{c|}{\includegraphics[width = 0.16\columnwidth]{assets/05-All-BoxPlots/06-G7/Motiv/G7-Product-Reliable-MOTIV.png}} &
    \multicolumn{2}{c}{\includegraphics[width = 0.16\columnwidth]{assets/05-All-BoxPlots/06-G7/Motiv/G7-Trust-Product-MOTIV.png}}
    \end{tabular}
    
    \caption{Guideline 7 participants' ratings for all dependent variables, disaggregated by participants' motivations for using technology.
	%For the disaggregated data, notice how large the distances between the average rating are when the guideline is applied.
	Table~\ref{tab:G7-Motiv-Stats-Appendix} below provides the statistics (where applicable).
}
    \label{fig:Motiv-G7-Appendix}
\end{table}

\begin{table}[h]

%\framebox[\linewidth]{For Measuring!}
\centering
\footnotesize

    \begin{tabular}{p{0.22\columnwidth}|c|c|c|c|c|c}
    
    \rowcolor{LightGray}\multicolumn{7}{c}{\textbf{Violation AI Product}}\\
    \hline
    \textbf{Dependent}  & \textbf{Distance b/w} &  &  & & \textbf{Bonferroni} &  \\
    \textbf{variable} & \textbf{Means} &  \textbf{df} &  \textbf{t-val} &   \textbf{p-value}  & \textbf{correction} & \textbf{Cohen's \textit{d}} \\
    \hline
    
    I would feel in control & - - - & - &  - - - & - - - & - - - & - - - \\
    \hline
    
    I would feel secure & - - - & - &  - - - & - - - & - - - & - - - \\
    \hline
    
    I would feel adequate & - - - & - &  - - - & - - - & - - - & - - - \\
    \hline
    
    I would feel certain & - - - & - &  - - - & - - - & - - - & - - - \\
    \hline
    
    I would feel productive & - - - & - &  - - - & - - - & - - - & - - -  \\
    \hline
    \hline
    
    I perceived it as useful &  - - - & - &  - - - & - - - & - - - & - - -  \\
    \hline
    
    I would not be suspicious & - - - & - &  - - - & - - - & - - - & - - -  \\
    \hline
    
    It would not be harmful & - - - & - &  - - - & - - - & - - - & - - -  \\
    \hline
    
    I find the product reliable & - - - & - &  - - - & - - - & - - - & - - -  \\
    \hline
    
    I would trust the product & 0.8643 & 56 &  2.6214 & \cellcolor{AbiOrangeQuote}.0113 & - - - & 0.6888 \\
    \hline

    \rowcolor{LightGray}\multicolumn{7}{c}{\textbf{Application AI Product}}\\
    \hline
    \textbf{Dependent}  & \textbf{Distance b/w} &  &  & & \textbf{Bonferroni} &  \\
    \textbf{variable} & \textbf{Means} &  \textbf{df} &  \textbf{t-val} &   \textbf{p-value}  & \textbf{correction} & \textbf{Cohen's \textit{d}} \\
    \hline
    
    I would feel in control & - - - & - &  - - - & - - - & - - - & - - -  \\
    \hline
    
    I would feel secure & - - - & - &  - - - & - - - & - - - & - - - \\
    \hline
    
    I would feel adequate & - - -  & - &  - - - & - - - & - - - & - - - \\
    \hline
    
    I would feel certain & - - - & - &  - - - & - - - & - - - & - - - \\
    \hline
    
    I would feel productive & - - - & - &  - - - & - - - & - - - & - - -    \\
    \hline
    \hline
    
    I perceived it as useful &  - - - & - &  - - - & - - - & - - - & - - -   \\
    \hline
    
    I would not be suspicious & - - - & - &  - - - & - - - & - - - & - - -   \\
    \hline
    
    It would not be harmful & - - - & - &  - - - & - - - & - - - & - - -  \\
    \hline
    
    I find the product reliable & - - - & - &  - - - & - - - & - - - & - - - \\
    \hline
    
    I would trust the product & - - - & - &  - - - & - - - & - - - & - - -

    \end{tabular}

    \caption{Guideline 7's t-test results %(\checkmark if Welch's t-test) 
    for task-oriented vs. tech-oriented participants' average ratings of the independent Violation AI product (top) and Application AI product (bottom), for all 10 dependent variables.
    If dashes (- - -) are present, no statistical test was performed.
    If the number of tests exceeded 5 for each product, Bonferroni correction applied by multiplying p-values by the number of tests performed.
    }
    \label{tab:G7-Motiv-Stats-Appendix}
\end{table}

%---------------------------------------------------- End Guideline 7

\clearpage

%Begin Guideline 8----------------------------------------------------

\begin{table}[]
    \centering
    \begin{tabular}{cc|cc|cc|cc|cc}
    \multicolumn{2}{c|}{\includegraphics[width = 0.16\columnwidth]{assets/05-All-BoxPlots/07-G8/Motiv/G8-Feel-In-Control-MOTIV.png}} &
    \multicolumn{2}{c|}{\includegraphics[width = 0.16\columnwidth]{assets/05-All-BoxPlots/07-G8/Motiv/G8-Feel-Secure-MOTIV.png}} &
    \multicolumn{2}{c|}{\includegraphics[width = 0.16\columnwidth]{assets/05-All-BoxPlots/07-G8/Motiv/G8-Feel-Adequate-MOTIV.png}} &
    \multicolumn{2}{c|}{\includegraphics[width = 0.16\columnwidth]{assets/05-All-BoxPlots/07-G8/Motiv/G8-Feel-Certain-MOTIV.png}} &
    \multicolumn{2}{c}{\includegraphics[width = 0.16\columnwidth]{assets/05-All-BoxPlots/07-G8/Motiv/G8-Feel-Productive-MOTIV.png}}
    \\
    \hline
    \hline
    \multicolumn{2}{c|}{\includegraphics[width = 0.16\columnwidth]{assets/05-All-BoxPlots/07-G8/Motiv/G8-Perceived-Useful-MOTIV.png}} &
    \multicolumn{2}{c|}{\includegraphics[width = 0.16\columnwidth]{assets/05-All-BoxPlots/07-G8/Motiv/G8-Not-Suspicious-MOTIV.png}} &
    \multicolumn{2}{c|}{\includegraphics[width = 0.16\columnwidth]{assets/05-All-BoxPlots/07-G8/Motiv/G8-Not-Harmful-MOTIV.png}} &
    \multicolumn{2}{c|}{\includegraphics[width = 0.16\columnwidth]{assets/05-All-BoxPlots/07-G8/Motiv/G8-Product-Reliable-MOTIV.png}} &
    \multicolumn{2}{c}{\includegraphics[width = 0.16\columnwidth]{assets/05-All-BoxPlots/07-G8/Motiv/G8-Trust-Product-MOTIV.png}}
    \end{tabular}
    
    \caption{Guideline 8 participants' ratings for all dependent variables, disaggregated by participants' motivations for using technology.
	%For the disaggregated data, notice how large the distances between the average rating are when the guideline is applied.
	Table~\ref{tab:G8-Motiv-Stats-Appendix} below provides the statistics (where applicable).
}
    \label{fig:Motiv-G8-Appendix}
\end{table}

\begin{table}[h]

%\framebox[\linewidth]{For Measuring!}
\centering
\footnotesize

    \begin{tabular}{p{0.22\columnwidth}|c|c|c|c|c|c}
    
    \rowcolor{LightGray}\multicolumn{7}{c}{\textbf{Violation AI Product}}\\
    \hline
    \textbf{Dependent}  & \textbf{Distance b/w} &  &  & & \textbf{Bonferroni} &  \\
    \textbf{variable} & \textbf{Means} &  \textbf{df} &  \textbf{t-val} &   \textbf{p-value}  & \textbf{correction} & \textbf{Cohen's \textit{d}} \\
    \hline
    
    I would feel in control & - - - & - &  - - - & - - - & - - - & - - - \\
    \hline
    
    I would feel secure &  - - - & - &  - - - & - - - & - - - & - - - \\
    \hline
    
    I would feel adequate & - - - & - &  - - - & - - - & - - - & - - - \\
    \hline
    
    I would feel certain &  - - - & - &  - - - & - - - & - - - & - - - \\
    \hline
    
    I would feel productive & - - - & - &  - - - & - - - & - - - & - - -  \\
    \hline
    \hline
    
    I perceived it as useful &  - - - & - &  - - - & - - - & - - - & - - -  \\
    \hline
    
    I would not be suspicious &  - - - & - &  - - - & - - - & - - - & - - - \\
    \hline
    
    It would not be harmful & - - - & - &  - - - & - - - & - - - & - - -  \\
    \hline
    
    I find the product reliable & - - - & - &  - - - & - - - & - - - & - - -  \\
    \hline
    
    I would trust the product & - - - & - &  - - - & - - - & - - - & - - - \\
    \hline

    \rowcolor{LightGray}\multicolumn{7}{c}{\textbf{Application AI Product}}\\
    \hline
    \textbf{Dependent}  & \textbf{Distance b/w} &  &  & & \textbf{Bonferroni} &  \\
    \textbf{variable} & \textbf{Means} &  \textbf{df} &  \textbf{t-val} &   \textbf{p-value}  & \textbf{correction} & \textbf{Cohen's \textit{d}} \\
    \hline
    
    I would feel in control & - - -& - &  - - - & - - - & - - - & - - -  \\
    \hline
    
    I would feel secure & - - - & - &  - - - & - - - & - - - & - - - \\
    \hline
    
    I would feel adequate & - - -  & - &  - - - & - - - & - - - & - - - \\
    \hline
    
    I would feel certain & - - - & - &  - - - & - - - & - - - & - - - \\
    \hline
    
    I would feel productive & - - - & - &  - - - & - - - & - - - & - - -    \\
    \hline
    \hline
    
    I perceived it as useful &  0.5419 & 59 &  2.2819 & \cellcolor{AbiOrangeQuote}.0261 & - - - & 0.5844 \\
    \hline
    
    I would not be suspicious &  - - - & - &  - - - & - - - & - - - & - - -   \\
    \hline
    
    It would not be harmful & - - - & - &  - - - & - - - & - - - & - - -  \\
    \hline
    
    I find the product reliable & - - - & - &  - - - & - - - & - - - & - - - \\
    \hline
    
    I would trust the product & - - - & - &  - - - & - - - & - - - & - - -

    \end{tabular}

    \caption{Guideline 8's t-test results %(\checkmark if Welch's t-test) 
    for task-oriented vs. tech-oriented participants' average ratings of the independent Violation AI product (top) and Application AI product (bottom), for all 10 dependent variables.
    If dashes (- - -) are present, no statistical test was performed.
    If the number of tests exceeded 5 for each product, Bonferroni correction applied by multiplying p-values by the number of tests performed.
    }
    \label{tab:G8-Motiv-Stats-Appendix}
\end{table}
\clearpage
%---------------------------------------------------- End Guideline 8

%Begin Guideline 9----------------------------------------------------

\begin{table}[]
    \centering
    \begin{tabular}{cc|cc|cc|cc|cc}
    \multicolumn{2}{c|}{\includegraphics[width = 0.16\columnwidth]{assets/05-All-BoxPlots/08-G9/Motiv/G9-Feel-In-Control-MOTIV.png}} &
    \multicolumn{2}{c|}{\includegraphics[width = 0.16\columnwidth]{assets/05-All-BoxPlots/08-G9/Motiv/G9-Feel-Secure-MOTIV.png}} &
    \multicolumn{2}{c|}{\includegraphics[width = 0.16\columnwidth]{assets/05-All-BoxPlots/08-G9/Motiv/G9-Feel-Adequate-MOTIV.png}} &
    \multicolumn{2}{c|}{\includegraphics[width = 0.16\columnwidth]{assets/05-All-BoxPlots/08-G9/Motiv/G9-Feel-Certain-MOTIV.png}} &
    \multicolumn{2}{c}{\includegraphics[width = 0.16\columnwidth]{assets/05-All-BoxPlots/08-G9/Motiv/G9-Feel-Productive-MOTIV.png}}
    \\
    \hline
    \hline
    \multicolumn{2}{c|}{\includegraphics[width = 0.16\columnwidth]{assets/05-All-BoxPlots/08-G9/Motiv/G9-Perceived-Useful-MOTIV.png}} &
    \multicolumn{2}{c|}{\includegraphics[width = 0.16\columnwidth]{assets/05-All-BoxPlots/08-G9/Motiv/G9-Not-Suspicious-MOTIV.png}} &
    \multicolumn{2}{c|}{\includegraphics[width = 0.16\columnwidth]{assets/05-All-BoxPlots/08-G9/Motiv/G9-Not-Harmful-MOTIV.png}} &
    \multicolumn{2}{c|}{\includegraphics[width = 0.16\columnwidth]{assets/05-All-BoxPlots/08-G9/Motiv/G9-Product-Reliable-MOTIV.png}} &
    \multicolumn{2}{c}{\includegraphics[width = 0.16\columnwidth]{assets/05-All-BoxPlots/08-G9/Motiv/G9-Trust-Product-MOTIV.png}}
    \end{tabular}
    
    \caption{Guideline 9 participants' ratings for all dependent variables, disaggregated by participants' motivations for using technology.
	%For the disaggregated data, notice how large the distances between the average rating are when the guideline is applied.
	Table~\ref{tab:G9-Motiv-Stats-Appendix} below provides the statistics (where applicable).
}
    \label{fig:Motiv-G9-Appendix}
\end{table}

\begin{table}[h]

%\framebox[\linewidth]{For Measuring!}
\centering
\footnotesize

    \begin{tabular}{p{0.22\columnwidth}|c|c|c|c|c|c}
    
    \rowcolor{LightGray}\multicolumn{7}{c}{\textbf{Violation AI Product}}\\
    \hline
    \textbf{Dependent}  & \textbf{Distance b/w} &  &  & & \textbf{Bonferroni} &  \\
    \textbf{variable} & \textbf{Means} &  \textbf{df} &  \textbf{t-val} &   \textbf{p-value}  & \textbf{correction} & \textbf{Cohen's \textit{d}} \\
    \hline
    
    I would feel in control & - - - & - &  - - - & - - - & - - - & - - - \\
    \hline
    
    I would feel secure & - - - & - &  - - - & - - - & - - - & - - - \\
    \hline
    
    I would feel adequate & - - - & - &  - - - & - - - & - - - & - - - \\
    \hline
    
    I would feel certain & - - - & - &  - - - & - - - & - - - & - - - \\
    \hline
    
    I would feel productive & - - - & - &  - - - & - - - & - - - & - - -  \\
    \hline
    \hline
    
    I perceived it as useful &  - - - & - &  - - - & - - - & - - - & - - -  \\
    \hline
    
    I would not be suspicious & - - - & - &  - - - & - - - & - - - & - - - \\
    \hline
    
    It would not be harmful & - - - & - &  - - - & - - - & - - - & - - -  \\
    \hline
    
    I find the product reliable & - - - & - &  - - - & - - - & - - - & - - -  \\
    \hline
    
    I would trust the product & - - - & - &  - - - & - - - & - - - & - - - \\
    \hline

    \rowcolor{LightGray}\multicolumn{7}{c}{\textbf{Application AI Product}}\\
    \hline
    \textbf{Dependent}  & \textbf{Distance b/w} &  &  & & \textbf{Bonferroni} &  \\
    \textbf{variable} & \textbf{Means} &  \textbf{df} &  \textbf{t-val} &   \textbf{p-value}  & \textbf{correction} & \textbf{Cohen's \textit{d}} \\
    \hline
    
    I would feel in control & 0.3274 & 55 &  1.1945 & .2374 & - - - & 0.3225  \\
    \hline
    
    I would feel secure & - - - & - &  - - - & - - - & - - - & - - - \\
    \hline
    
    I would feel adequate & - - -  & - &  - - - & - - - & - - - & - - - \\
    \hline
    
    I would feel certain & - - - & - &  - - - & - - - & - - - & - - - \\
    \hline
    
    I would feel productive & 0.5760 & 56 &  1.7537 & .0850 & - - - & 0.4675    \\
    \hline
    \hline
    
    I perceived it as useful &  0.6029 & 56 &  1.9316 & .0585 & - - - & 0.5150   \\
    \hline
    
    I would not be suspicious & - - - & - &  - - - & - - - & - - - & - - -   \\
    \hline
    
    It would not be harmful & - - - & - &  - - - & - - - & - - - & - - -  \\
    \hline
    
    I find the product reliable & - - - & - &  - - - & - - - & - - - & - - - \\
    \hline
    
    I would trust the product & 0.9592 & 53 &  2.7609 & \cellcolor{AbiOrangeQuote}.0079 & - - - & 0.7547
    
    \end{tabular}

    \caption{Guideline 9's t-test results %(\checkmark if Welch's t-test) 
    for task-oriented vs. tech-oriented participants' average ratings of the independent Violation AI product (top) and Application AI product (bottom), for all 10 dependent variables.
    If dashes (- - -) are present, no statistical test was performed.
    If the number of tests exceeded 5 for each product, Bonferroni correction applied by multiplying p-values by the number of tests performed.
    }
    \label{tab:G9-Motiv-Stats-Appendix}
\end{table}
\clearpage
%---------------------------------------------------- End Guideline 9

%Begin Guideline 10----------------------------------------------------

\begin{table}[]
    \centering
    \begin{tabular}{cc|cc|cc|cc|cc}
    \multicolumn{2}{c|}{\includegraphics[width = 0.16\columnwidth]{assets/05-All-BoxPlots/09-G10/Motiv/G10-Feel-In-Control-MOTIV.png}} &
    \multicolumn{2}{c|}{\includegraphics[width = 0.16\columnwidth]{assets/05-All-BoxPlots/09-G10/Motiv/G10-Feel-Secure-MOTIV.png}} &
    \multicolumn{2}{c|}{\includegraphics[width = 0.16\columnwidth]{assets/05-All-BoxPlots/09-G10/Motiv/G10-Feel-Adequate-MOTIV.png}} &
    \multicolumn{2}{c|}{\includegraphics[width = 0.16\columnwidth]{assets/05-All-BoxPlots/09-G10/Motiv/G10-Feel-Certain-MOTIV.png}} &
    \multicolumn{2}{c}{\includegraphics[width = 0.16\columnwidth]{assets/05-All-BoxPlots/09-G10/Motiv/G10-Feel-Productive-MOTIV.png}}
    \\
    \hline
    \hline
    \multicolumn{2}{c|}{\includegraphics[width = 0.16\columnwidth]{assets/05-All-BoxPlots/09-G10/Motiv/G10-Perceived-Useful-MOTIV.png}} &
    \multicolumn{2}{c|}{\includegraphics[width = 0.16\columnwidth]{assets/05-All-BoxPlots/09-G10/Motiv/G10-Not-Suspicious-MOTIV.png}} &
    \multicolumn{2}{c|}{\includegraphics[width = 0.16\columnwidth]{assets/05-All-BoxPlots/09-G10/Motiv/G10-Not-Harmful-MOTIV.png}} &
    \multicolumn{2}{c|}{\includegraphics[width = 0.16\columnwidth]{assets/05-All-BoxPlots/09-G10/Motiv/G10-Product-Reliable-MOTIV.png}} &
    \multicolumn{2}{c}{\includegraphics[width = 0.16\columnwidth]{assets/05-All-BoxPlots/09-G10/Motiv/G10-Trust-Product-MOTIV.png}}
    \end{tabular}
    
    \caption{Guideline 10 participants' ratings for all dependent variables, disaggregated by participants' motivations for using technology.
	%For the disaggregated data, notice how large the distances between the average rating are when the guideline is applied.
	Table~\ref{tab:G10-Motiv-Stats-Appendix} below provides the statistics (where applicable).
}
    \label{fig:Motiv-G10-Appendix}
\end{table}

\begin{table}[h]

%\framebox[\linewidth]{For Measuring!}
\centering
\footnotesize

    \begin{tabular}{p{0.22\columnwidth}|c|c|c|c|c|c}
    
    \rowcolor{LightGray}\multicolumn{7}{c}{\textbf{Violation AI Product}}\\
    \hline
    \textbf{Dependent}  & \textbf{Distance b/w} &  &  & & \textbf{Bonferroni} &  \\
    \textbf{variable} & \textbf{Means} &  \textbf{df} &  \textbf{t-val} &   \textbf{p-value}  & \textbf{correction} & \textbf{Cohen's \textit{d}} \\
    \hline
    
    I would feel in control & - - - & - &  - - - & - - - & - - - & - - - \\
    \hline
    
    I would feel secure & 0.8636 & 63 &  2.0064 & \cellcolor{AbiOrangeQuote}.0491 & - - - & 0.4978 \\
    \hline
    
    I would feel adequate & - - - & - &  - - - & - - - & - - - & - - - \\
    \hline
    
    I would feel certain & - - - & - &  - - - & - - - & - - - & - - - \\
    \hline
    
    I would feel productive & - - - & - &  - - - & - - - & - - - & - - -  \\
    \hline
    \hline
    
    I perceived it as useful &  - - - & - &  - - - & - - - & - - - & - - -  \\
    \hline
    
    I would not be suspicious & 1.0663 & 63 &  2.1911 & \cellcolor{AbiOrangeQuote}.0322 & - - - & 0.5436 \\
    \hline
    
    It would not be harmful & 0.7419 & 61 &  1.7639 & .0828 & - - - & 0.4445 \\
    \hline
    
    I find the product reliable & - - - & - &  - - - & - - - & - - - & - - -  \\
    \hline
    
    I would trust the product & - - - & - &  - - - & - - - & - - - & - - - \\
    \hline

    \rowcolor{LightGray}\multicolumn{7}{c}{\textbf{Application AI Product}}\\
    \hline
    \textbf{Dependent}  & \textbf{Distance b/w} &  &  & & \textbf{Bonferroni} &  \\
    \textbf{variable} & \textbf{Means} &  \textbf{df} &  \textbf{t-val} &   \textbf{p-value}  & \textbf{correction} & \textbf{Cohen's \textit{d}} \\
    \hline
    
    I would feel in control & - - - & - &  - - - & - - - & - - - & - - -  \\
    \hline
    
    I would feel secure &  - - - & - &  - - - & - - - & - - - & - - - \\
    \hline
    
    I would feel adequate & - - -  & - &  - - - & - - - & - - - & - - - \\
    \hline
    
    I would feel certain & - - - & - &  - - - & - - - & - - - & - - - \\
    \hline
    
    I would feel productive & - - - & - &  - - - & - - - & - - - & - - -   \\
    \hline
    \hline
    
    I perceived it as useful &  - - - & - &  - - - & - - - & - - - & - - -   \\
    \hline
    
    I would not be suspicious & 0.6970 & 62 &  1.6587 & .1022 & - - - & 0.4149   \\
    \hline
    
    It would not be harmful & - - - & - &  - - - & - - - & - - - & - - -  \\
    \hline
    
    I find the product reliable & - - - & - &  - - - & - - - & - - - & - - - \\
    \hline
    
    I would trust the product & - - - & - &  - - - & - - - & - - - & - - -

    \end{tabular}

    \caption{Guideline 10's t-test results %(\checkmark if Welch's t-test) 
    for task-oriented vs. tech-oriented participants' average ratings of the independent Violation AI product (top) and Application AI product (bottom), for all 10 dependent variables.
    If dashes (- - -) are present, no statistical test was performed.
    If the number of tests exceeded 5 for each product, Bonferroni correction applied by multiplying p-values by the number of tests performed.
    }
    \label{tab:G10-Motiv-Stats-Appendix}
\end{table}
\clearpage
%---------------------------------------------------- End Guideline 10

%Begin Guideline 11----------------------------------------------------

\begin{table}[]
    \centering
    \begin{tabular}{cc|cc|cc|cc|cc}
    \multicolumn{2}{c|}{\includegraphics[width = 0.16\columnwidth]{assets/05-All-BoxPlots/10-G11/Motiv/G11-Feel-In-Control-MOTIV.png}} &
    \multicolumn{2}{c|}{\includegraphics[width = 0.16\columnwidth]{assets/05-All-BoxPlots/10-G11/Motiv/G11-Feel-Secure-MOTIV.png}} &
    \multicolumn{2}{c|}{\includegraphics[width = 0.16\columnwidth]{assets/05-All-BoxPlots/10-G11/Motiv/G11-Feel-Adequate-MOTIV.png}} &
    \multicolumn{2}{c|}{\includegraphics[width = 0.16\columnwidth]{assets/05-All-BoxPlots/10-G11/Motiv/G11-Feel-Certain-MOTIV.png}} &
    \multicolumn{2}{c}{\includegraphics[width = 0.16\columnwidth]{assets/05-All-BoxPlots/10-G11/Motiv/G11-Feel-Productive-MOTIV.png}}
    \\
    \hline
    \hline
    \multicolumn{2}{c|}{\includegraphics[width = 0.16\columnwidth]{assets/05-All-BoxPlots/10-G11/Motiv/G11-Perceived-Useful-MOTIV.png}} &
    \multicolumn{2}{c|}{\includegraphics[width = 0.16\columnwidth]{assets/05-All-BoxPlots/10-G11/Motiv/G11-Not-Suspicious-MOTIV.png}} &
    \multicolumn{2}{c|}{\includegraphics[width = 0.16\columnwidth]{assets/05-All-BoxPlots/10-G11/Motiv/G11-Not-Harmful-MOTIV.png}} &
    \multicolumn{2}{c|}{\includegraphics[width = 0.16\columnwidth]{assets/05-All-BoxPlots/10-G11/Motiv/G11-Product-Reliable-MOTIV.png}} &
    \multicolumn{2}{c}{\includegraphics[width = 0.16\columnwidth]{assets/05-All-BoxPlots/10-G11/Motiv/G11-Trust-Product-MOTIV.png}}
    \end{tabular}
    
    \caption{Guideline 11 participants' ratings for all dependent variables, disaggregated by participants' motivations for using technology.
	%For the disaggregated data, notice how large the distances between the average rating are when the guideline is applied.
	Table~\ref{tab:G11-Motiv-Stats-Appendix} below provides the statistics (where applicable).
}
    \label{fig:Motiv-G11-Appendix}
\end{table}

\begin{table}[h]

%\framebox[\linewidth]{For Measuring!}
\centering
\footnotesize

    \begin{tabular}{p{0.22\columnwidth}|c|c|c|c|c|c}
    
    \rowcolor{LightGray}\multicolumn{7}{c}{\textbf{Violation AI Product}}\\
    \hline
    \textbf{Dependent}  & \textbf{Distance b/w} &  &  & & \textbf{Bonferroni} &  \\
    \textbf{variable} & \textbf{Means} &  \textbf{df} &  \textbf{t-val} &   \textbf{p-value}  & \textbf{correction} & \textbf{Cohen's \textit{d}} \\
    \hline
    
    I would feel in control & - - - & - &  - - - & - - - & - - - & - - - \\
    \hline
    
    I would feel secure & - - - & - &  - - - & - - - & - - - & - - - \\
    \hline
    
    I would feel adequate & - - - & - &  - - - & - - - & - - - & - - - \\
    \hline
    
    I would feel certain & - - - & - &  - - - & - - - & - - - & - - - \\
    \hline
    
    I would feel productive & - - - & - &  - - - & - - - & - - - & - - -  \\
    \hline
    \hline
    
    I perceived it as useful &  - - - & - &  - - - & - - - & - - - & - - -  \\
    \hline
    
    I would not be suspicious & - - - & - &  - - - & - - - & - - - & - - - \\
    \hline
    
    It would not be harmful & - - - & - &  - - - & - - - & - - - & - - -  \\
    \hline
    
    I find the product reliable & - - - & - &  - - - & - - - & - - - & - - -  \\
    \hline
    
    I would trust the product & - - - & - &  - - - & - - - & - - - & - - - \\
    \hline

    \rowcolor{LightGray}\multicolumn{7}{c}{\textbf{Application AI Product}}\\
    \hline
    \textbf{Dependent}  & \textbf{Distance b/w} &  &  & & \textbf{Bonferroni} &  \\
    \textbf{variable} & \textbf{Means} &  \textbf{df} &  \textbf{t-val} &   \textbf{p-value}  & \textbf{correction} & \textbf{Cohen's \textit{d}} \\
    \hline
    
    I would feel in control & - - - & - &  - - - & - - - & - - - & - - -  \\
    \hline
    
    I would feel secure & - - - & - &  - - - & - - - & - - - & - - - \\
    \hline
    
    I would feel adequate & - - - & - &  - - - & - - - & - - - & - - - \\
    \hline
    
    I would feel certain & - - - & - &  - - - & - - - & - - - & - - - \\
    \hline
    
    I would feel productive & - - - & - &  - - - & - - - & - - - & - - -   \\
    \hline
    \hline
    
    I perceived it as useful &  - - - & - &  - - - & - - - & - - - & - - -   \\
    \hline
    
    I would not be suspicious & - - - & - &  - - - & - - - & - - - & - - -   \\
    \hline
    
    It would not be harmful & - - - & - &  - - - & - - - & - - - & - - -  \\
    \hline
    
    I find the product reliable & - - - & - &  - - - & - - - & - - - & - - - \\
    \hline
    
    I would trust the product & - - - & - &  - - - & - - - & - - - & - - -

    \end{tabular}

    \caption{Guideline 11's t-test results %(\checkmark if Welch's t-test) 
    for task-oriented vs. tech-oriented participants' average ratings of the independent Violation AI product (top) and Application AI product (bottom), for all 10 dependent variables.
    If dashes (- - -) are present, no statistical test was performed.
    If the number of tests exceeded 5 for each product, Bonferroni correction applied by multiplying p-values by the number of tests performed.
    }
    \label{tab:G11-Motiv-Stats-Appendix}
\end{table}
\clearpage
%---------------------------------------------------- End Guideline 11

%Begin Guideline 12----------------------------------------------------

\begin{table}[]
    \centering
    \begin{tabular}{cc|cc|cc|cc|cc}
    \multicolumn{2}{c|}{\includegraphics[width = 0.16\columnwidth]{assets/05-All-BoxPlots/11-G12/Motiv/G12-Feel-In-Control-MOTIV.png}} &
    \multicolumn{2}{c|}{\includegraphics[width = 0.16\columnwidth]{assets/05-All-BoxPlots/11-G12/Motiv/G12-Feel-Secure-MOTIV.png}} &
    \multicolumn{2}{c|}{\includegraphics[width = 0.16\columnwidth]{assets/05-All-BoxPlots/11-G12/Motiv/G12-Feel-Adequate-MOTIV.png}} &
    \multicolumn{2}{c|}{\includegraphics[width = 0.16\columnwidth]{assets/05-All-BoxPlots/11-G12/Motiv/G12-Feel-Certain-MOTIV.png}} &
    \multicolumn{2}{c}{\includegraphics[width = 0.16\columnwidth]{assets/05-All-BoxPlots/11-G12/Motiv/G12-Feel-Productive-MOTIV.png}}
    \\
    \hline
    \hline
    \multicolumn{2}{c|}{\includegraphics[width = 0.16\columnwidth]{assets/05-All-BoxPlots/11-G12/Motiv/G12-Perceived-Useful-MOTIV.png}} &
    \multicolumn{2}{c|}{\includegraphics[width = 0.16\columnwidth]{assets/05-All-BoxPlots/11-G12/Motiv/G12-Not-Suspicious-MOTIV.png}} &
    \multicolumn{2}{c|}{\includegraphics[width = 0.16\columnwidth]{assets/05-All-BoxPlots/11-G12/Motiv/G12-Not-Harmful-MOTIV.png}} &
    \multicolumn{2}{c|}{\includegraphics[width = 0.16\columnwidth]{assets/05-All-BoxPlots/11-G12/Motiv/G12-Product-Reliable-MOTIV.png}} &
    \multicolumn{2}{c}{\includegraphics[width = 0.16\columnwidth]{assets/05-All-BoxPlots/11-G12/Motiv/G12-Trust-Product-MOTIV.png}}
    \end{tabular}
    
    \caption{Guideline 12 participants' ratings for all dependent variables, disaggregated by participants' motivations for using technology.
	%For the disaggregated data, notice how large the distances between the average rating are when the guideline is applied.
	Table~\ref{tab:G12-Motiv-Stats-Appendix} below provides the statistics (where applicable).
}
    \label{fig:Motiv-G12-Appendix}
\end{table}

\begin{table}[h]

%\framebox[\linewidth]{For Measuring!}
\centering
\footnotesize

    \begin{tabular}{p{0.22\columnwidth}|c|c|c|c|c|c}
    
    \rowcolor{LightGray}\multicolumn{7}{c}{\textbf{Violation AI Product}}\\
    \hline
    \textbf{Dependent}  & \textbf{Distance b/w} &  &  & & \textbf{Bonferroni} &  \\
    \textbf{variable} & \textbf{Means} &  \textbf{df} &  \textbf{t-val} &   \textbf{p-value}  & \textbf{correction} & \textbf{Cohen's \textit{d}} \\
    \hline
    
    I would feel in control & - - - & - &  - - - & - - - & - - - & - - -  \\
    \hline
    
    I would feel secure & - - - & - &  - - - & - - - & - - - & - - - \\
    \hline
    
    I would feel adequate & - - -  & - &  - - - & - - - & - - - & - - - \\
    \hline
    
    I would feel certain & - - - & - &  - - - & - - - & - - - & - - - \\
    \hline
    
    I would feel productive & - - - & - &  - - - & - - - & - - - & - - -   \\
    \hline
    \hline
    
    I perceived it as useful &  - - - & - &  - - - & - - - & - - - & - - -   \\
    \hline
    
    I would not be suspicious & - - - & - &  - - - & - - - & - - - & - - -   \\
    \hline
    
    It would not be harmful & - - - & - &  - - - & - - - & - - - & - - -  \\
    \hline
    
    I find the product reliable & - - - & - &  - - - & - - - & - - - & - - - \\
    \hline
    
    I would trust the product & - - - & - &  - - - & - - - & - - - & - - - \\
    \hline

    \rowcolor{LightGray}\multicolumn{7}{c}{\textbf{Application AI Product}}\\
    \hline
    \textbf{Dependent}  & \textbf{Distance b/w} &  &  & & \textbf{Bonferroni} &  \\
    \textbf{variable} & \textbf{Means} &  \textbf{df} &  \textbf{t-val} &   \textbf{p-value}  & \textbf{correction} & \textbf{Cohen's \textit{d}} \\
    \hline
    
    I would feel in control & - - - & - &  - - - & - - - & - - - & - - -  \\
    \hline
    
    I would feel secure & - - - & - &  - - - & - - - & - - - & - - - \\
    \hline
    
    I would feel adequate & - - -  & - &  - - - & - - - & - - - & - - - \\
    \hline
    
    I would feel certain & - - - & - &  - - - & - - - & - - - & - - - \\
    \hline
    
    I would feel productive & - - - & - &  - - - & - - - & - - - & - - -   \\
    \hline
    \hline
    
    I perceived it as useful &  0.8235 & 66 &  2.2379 & \cellcolor{AbiOrangeQuote}.0286 & - - - & 0.5428 \\
    \hline
    
    I would not be suspicious & - - - & - &  - - - & - - - & - - - & - - -   \\
    \hline
    
    It would not be harmful & - - - & - &  - - - & - - - & - - - & - - -  \\
    \hline
    
    I find the product reliable & - - - & - &  - - - & - - - & - - - & - - - \\
    \hline
    
    I would trust the product & - - - & - &  - - - & - - - & - - - & - - -

    \end{tabular}

    \caption{Guideline 12's t-test results %(\checkmark if Welch's t-test) 
    for task-oriented vs. tech-oriented participants' average ratings of the independent Violation AI product (top) and Application AI product (bottom), for all 10 dependent variables.
    If dashes (- - -) are present, no statistical test was performed.
    If the number of tests exceeded 5 for each product, Bonferroni correction applied by multiplying p-values by the number of tests performed.
    }
    \label{tab:G12-Motiv-Stats-Appendix}
\end{table}
\clearpage
%---------------------------------------------------- End Guideline 12

%Begin Guideline 13----------------------------------------------------

\begin{table}[]
    \centering
    \begin{tabular}{cc|cc|cc|cc|cc}
    \multicolumn{2}{c|}{\includegraphics[width = 0.16\columnwidth]{assets/05-All-BoxPlots/12-G13/Motiv/G13-Feel-In-Control-MOTIV.png}} &
    \multicolumn{2}{c|}{\includegraphics[width = 0.16\columnwidth]{assets/05-All-BoxPlots/12-G13/Motiv/G13-Feel-Secure-MOTIV.png}} &
    \multicolumn{2}{c|}{\includegraphics[width = 0.16\columnwidth]{assets/05-All-BoxPlots/12-G13/Motiv/G13-Feel-Adequate-MOTIV.png}} &
    \multicolumn{2}{c|}{\includegraphics[width = 0.16\columnwidth]{assets/05-All-BoxPlots/12-G13/Motiv/G13-Feel-Certain-MOTIV.png}} &
    \multicolumn{2}{c}{\includegraphics[width = 0.16\columnwidth]{assets/05-All-BoxPlots/12-G13/Motiv/G13-Feel-Productive-MOTIV.png}}
    \\
    \hline
    \hline
    \multicolumn{2}{c|}{\includegraphics[width = 0.16\columnwidth]{assets/05-All-BoxPlots/12-G13/Motiv/G13-Perceived-Useful-MOTIV.png}} &
    \multicolumn{2}{c|}{\includegraphics[width = 0.16\columnwidth]{assets/05-All-BoxPlots/12-G13/Motiv/G13-Not-Suspicious-MOTIV.png}} &
    \multicolumn{2}{c|}{\includegraphics[width = 0.16\columnwidth]{assets/05-All-BoxPlots/12-G13/Motiv/G13-Not-Harmful-MOTIV.png}} &
    \multicolumn{2}{c|}{\includegraphics[width = 0.16\columnwidth]{assets/05-All-BoxPlots/12-G13/Motiv/G13-Product-Reliable-MOTIV.png}} &
    \multicolumn{2}{c}{\includegraphics[width = 0.16\columnwidth]{assets/05-All-BoxPlots/12-G13/Motiv/G13-Trust-Product-MOTIV.png}}
    \end{tabular}
    
    \caption{Guideline 13 participants' ratings for all dependent variables, disaggregated by participants' motivations for using technology.
	%For the disaggregated data, notice how large the distances between the average rating are when the guideline is applied.
	Table~\ref{tab:G13-Motiv-Stats-Appendix} below provides the statistics (where applicable).
}
    \label{fig:Motiv-G13-Appendix}
\end{table}

\begin{table}[h]

%\framebox[\linewidth]{For Measuring!}
\centering
\footnotesize

    \begin{tabular}{p{0.22\columnwidth}|c|c|c|c|c|c}
    
    \rowcolor{LightGray}\multicolumn{7}{c}{\textbf{Violation AI Product}}\\
    \hline
    \textbf{Dependent}  & \textbf{Distance b/w} &  &  & & \textbf{Bonferroni} &  \\
    \textbf{variable} & \textbf{Means} &  \textbf{df} &  \textbf{t-val} &   \textbf{p-value}  & \textbf{correction} & \textbf{Cohen's \textit{d}} \\
    \hline
    
    I would feel in control &  - - - & - &  - - - & - - - & - - - & - - -  \\
    \hline
    
    I would feel secure & - - - & - &  - - - & - - - & - - - & - - - \\
    \hline
    
    I would feel adequate & - - -  & - &  - - - & - - - & - - - & - - - \\
    \hline
    
    I would feel certain &  - - - & - &  - - - & - - - & - - - & - - - \\
    \hline
    
    I would feel productive & - - - & - &  - - - & - - - & - - - & - - -   \\
    \hline
    \hline
    
    I perceived it as useful &  - - - & - &  - - - & - - - & - - - & - - -   \\
    \hline
    
    I would not be suspicious &  - - - & - &  - - - & - - - & - - - & - - -   \\
    \hline
    
    It would not be harmful &  - - - & - &  - - - & - - - & - - - & - - -  \\
    \hline
    
    I find the product reliable & - - - & - &  - - - & - - - & - - - & - - - \\
    \hline
    
    I would trust the product & - - - & - &  - - - & - - - & - - - & - - - \\
    \hline

    \rowcolor{LightGray}\multicolumn{7}{c}{\textbf{Application AI Product}}\\
    \hline
    \textbf{Dependent}  & \textbf{Distance b/w} &  &  & & \textbf{Bonferroni} &  \\
    \textbf{variable} & \textbf{Means} &  \textbf{df} &  \textbf{t-val} &   \textbf{p-value}  & \textbf{correction} & \textbf{Cohen's \textit{d}} \\
    \hline
    
    I would feel in control & - - - & - &  - - - & - - - & - - - & - - -  \\
    \hline
    
    I would feel secure & - - - & - &  - - - & - - - & - - - & - - - \\
    \hline
    
    I would feel adequate &  - - - & - &  - - - & - - - & - - - & - - - \\
    \hline
    
    I would feel certain & 0.7007 & 55 &  1.7548 & .0849 & - - - & 0.4649 \\
    \hline
    
    I would feel productive & - - - & - &  - - - & - - - & - - - & - - -   \\
    \hline
    \hline
    
    I perceived it as useful &  - - - & - &  - - - & - - - & - - - & - - -   \\
    \hline
    
    I would not be suspicious & - - - & - &  - - - & - - - & - - - & - - -   \\
    \hline
    
    It would not be harmful & - - - & - &  - - - & - - - & - - - & - - -  \\
    \hline
    
    I find the product reliable & - - - & - &  - - - & - - - & - - - & - - - \\
    \hline
    
    I would trust the product & - - - & - &  - - - & - - - & - - - & - - -

    \end{tabular}

    \caption{Guideline 13's t-test results %(\checkmark if Welch's t-test) 
    for task-oriented vs. tech-oriented participants' average ratings of the independent Violation AI product (top) and Application AI product (bottom), for all 10 dependent variables.
    If dashes (- - -) are present, no statistical test was performed.
    If the number of tests exceeded 5 for each product, Bonferroni correction applied by multiplying p-values by the number of tests performed.
    }
    \label{tab:G13-Motiv-Stats-Appendix}
\end{table}
\clearpage
%---------------------------------------------------- End Guideline 13

%Begin Guideline 14---------------------------------------------------

\begin{table}[]
    \centering
    \begin{tabular}{cc|cc|cc|cc|cc}
    \multicolumn{2}{c|}{\includegraphics[width = 0.16\columnwidth]{assets/05-All-BoxPlots/13-G14/Motiv/G14-Feel-In-Control-MOTIV.png}} &
    \multicolumn{2}{c|}{\includegraphics[width = 0.16\columnwidth]{assets/05-All-BoxPlots/13-G14/Motiv/G14-Feel-Secure-MOTIV.png}} &
    \multicolumn{2}{c|}{\includegraphics[width = 0.16\columnwidth]{assets/05-All-BoxPlots/13-G14/Motiv/G14-Feel-Adequate-MOTIV.png}} &
    \multicolumn{2}{c|}{\includegraphics[width = 0.16\columnwidth]{assets/05-All-BoxPlots/13-G14/Motiv/G14-Feel-Certain-MOTIV.png}} &
    \multicolumn{2}{c}{\includegraphics[width = 0.16\columnwidth]{assets/05-All-BoxPlots/13-G14/Motiv/G14-Feel-Productive-MOTIV.png}}
    \\
    \hline
    \hline
    \multicolumn{2}{c|}{\includegraphics[width = 0.16\columnwidth]{assets/05-All-BoxPlots/13-G14/Motiv/G14-Perceived-Useful-MOTIV.png}} &
    \multicolumn{2}{c|}{\includegraphics[width = 0.16\columnwidth]{assets/05-All-BoxPlots/13-G14/Motiv/G14-Not-Suspicious-MOTIV.png}} &
    \multicolumn{2}{c|}{\includegraphics[width = 0.16\columnwidth]{assets/05-All-BoxPlots/13-G14/Motiv/G14-Not-Harmful-MOTIV.png}} &
    \multicolumn{2}{c|}{\includegraphics[width = 0.16\columnwidth]{assets/05-All-BoxPlots/13-G14/Motiv/G14-Product-Reliable-MOTIV.png}} &
    \multicolumn{2}{c}{\includegraphics[width = 0.16\columnwidth]{assets/05-All-BoxPlots/13-G14/Motiv/G14-Trust-Product-MOTIV.png}}
    \end{tabular}
    
    \caption{Guideline 14 participants' ratings for all dependent variables, disaggregated by participants' motivations for using technology.
	%For the disaggregated data, notice how large the distances between the average rating are when the guideline is applied.
	Table~\ref{tab:G14-Motiv-Stats-Appendix} below provides the statistics (where applicable).
}
    \label{fig:Motiv-G14-Appendix}
\end{table}

\begin{table}[h]

%\framebox[\linewidth]{For Measuring!}
\centering
\footnotesize

    \begin{tabular}{p{0.22\columnwidth}|c|c|c|c|c|c}
    
    \rowcolor{LightGray}\multicolumn{7}{c}{\textbf{Violation AI Product}}\\
    \hline
    \textbf{Dependent}  & \textbf{Distance b/w} &  &  & & \textbf{Bonferroni} &  \\
    \textbf{variable} & \textbf{Means} &  \textbf{df} &  \textbf{t-val} &   \textbf{p-value}  & \textbf{correction} & \textbf{Cohen's \textit{d}} \\
    \hline
    
    I would feel in control & - - - & - &  - - - & - - - & - - - & - - -  \\
    \hline
    
    I would feel secure & - - - & - &  - - - & - - - & - - - & - - - \\
    \hline
    
    I would feel adequate & - - - & - &  - - - & - - - & - - - & - - - \\
    \hline
    
    I would feel certain & - - - & - &  - - - & - - - & - - - & - - - \\
    \hline
    
    I would feel productive & - - - & - &  - - - & - - - & - - - & - - -   \\
    \hline
    \hline
    
    I perceived it as useful &  - - - & - &  - - - & - - - & - - - & - - -   \\
    \hline
    
    I would not be suspicious & - - - & - &  - - - & - - - & - - - & - - -   \\
    \hline
    
    It would not be harmful & - - - & - &  - - - & - - - & - - - & - - - \\
    \hline
    
    I find the product reliable & - - - & - &  - - - & - - - & - - - & - - - \\
    \hline
    
    I would trust the product & - - - & - &  - - - & - - - & - - - & - - - \\
    \hline

    \rowcolor{LightGray}\multicolumn{7}{c}{\textbf{Application AI Product}}\\
    \hline
    \textbf{Dependent}  & \textbf{Distance b/w} &  &  & & \textbf{Bonferroni} &  \\
    \textbf{variable} & \textbf{Means} &  \textbf{df} &  \textbf{t-val} &   \textbf{p-value}  & \textbf{correction} & \textbf{Cohen's \textit{d}} \\
    \hline
    
    I would feel in control & - - - & - &  - - - & - - - & - - - & - - -  \\
    \hline
    
    I would feel secure & - - - & - &  - - - & - - - & - - - & - - - \\
    \hline
    
    I would feel adequate & - - - & - &  - - - & - - - & - - - & - - - \\
    \hline
    
    I would feel certain & - - - & - &  - - - & - - - & - - - & - - - \\
    \hline
    
    I would feel productive & - - - & - &  - - - & - - - & - - - & - - -   \\
    \hline
    \hline
    
    I perceived it as useful &  - - - & - &  - - - & - - - & - - - & - - -   \\
    \hline
    
    I would not be suspicious & - - - & - &  - - - & - - - & - - - & - - -   \\
    \hline
    
    It would not be harmful & - - - & - &  - - - & - - - & - - - & - - - \\
    \hline
    
    I find the product reliable & - - - & - &  - - - & - - - & - - - & - - - \\
    \hline
    
    I would trust the product & - - - & - &  - - - & - - - & - - - & - - - \\

    \end{tabular}

    \caption{Guideline 14's t-test results %(\checkmark if Welch's t-test) 
    for task-oriented vs. tech-oriented participants' average ratings of the independent Violation AI product (top) and Application AI product (bottom), for all 10 dependent variables.
    If dashes (- - -) are present, no statistical test was performed.
    If the number of tests exceeded 5 for each product, Bonferroni correction applied by multiplying p-values by the number of tests performed.
    }
    \label{tab:G14-Motiv-Stats-Appendix}
\end{table}
\clearpage
%---------------------------------------------------- End Guideline 14

%Begin Guideline 15---------------------------------------------------

\begin{table}[]
    \centering
    \begin{tabular}{cc|cc|cc|cc|cc}
    \multicolumn{2}{c|}{\includegraphics[width = 0.16\columnwidth]{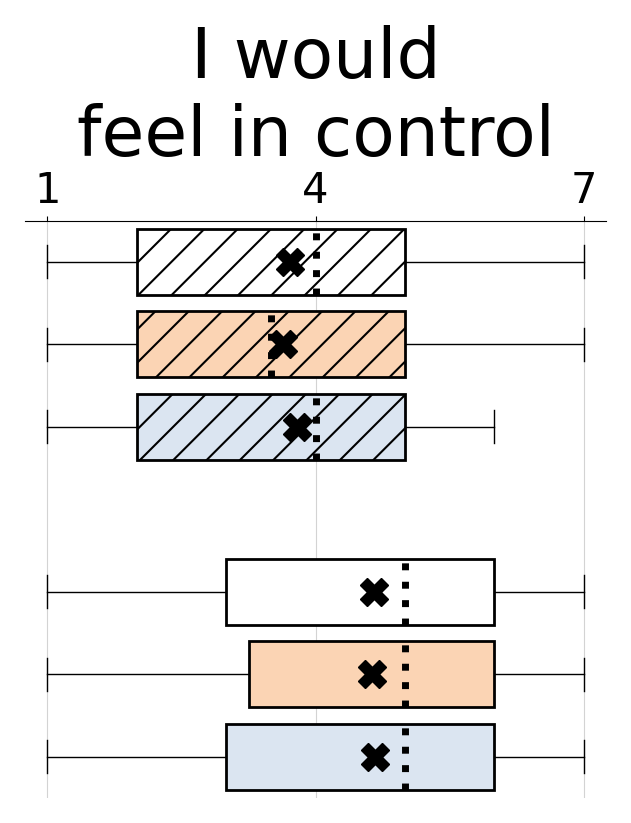}} &
    \multicolumn{2}{c|}{\includegraphics[width = 0.16\columnwidth]{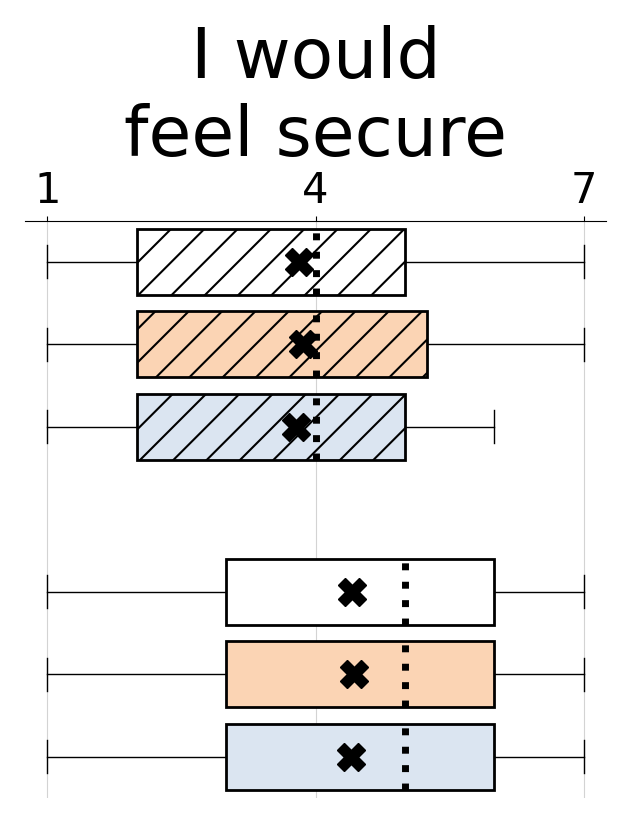}} &
    \multicolumn{2}{c|}{\includegraphics[width = 0.16\columnwidth]{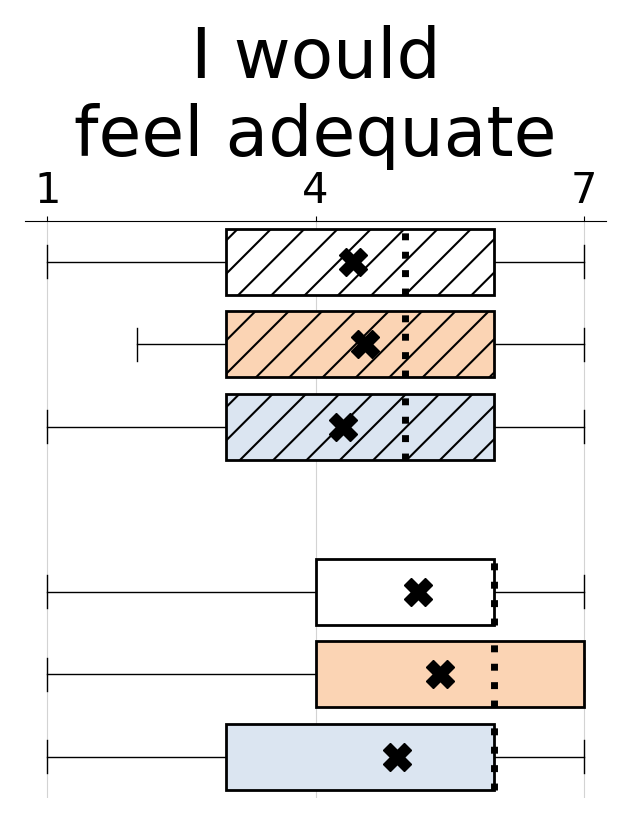}} &
    \multicolumn{2}{c|}{\includegraphics[width = 0.16\columnwidth]{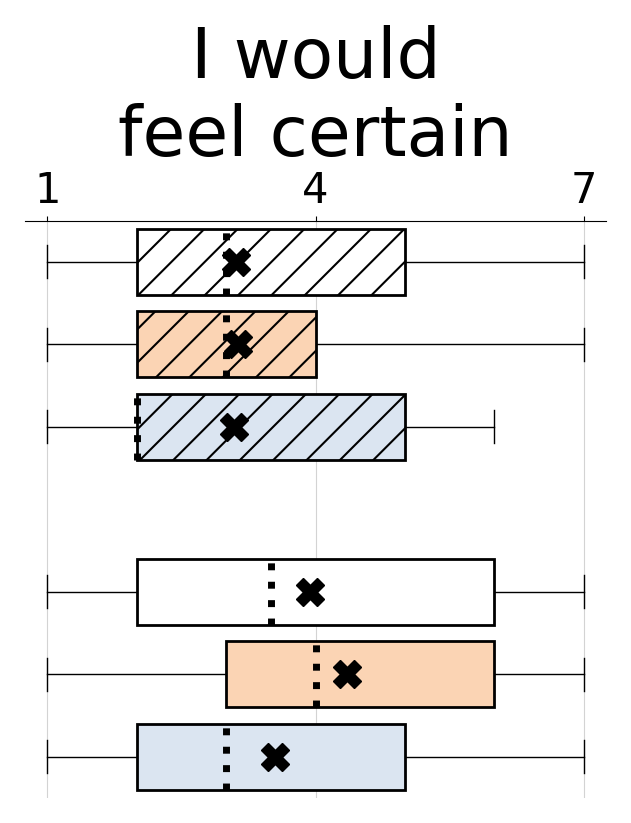}} &
    \multicolumn{2}{c}{\includegraphics[width = 0.16\columnwidth]{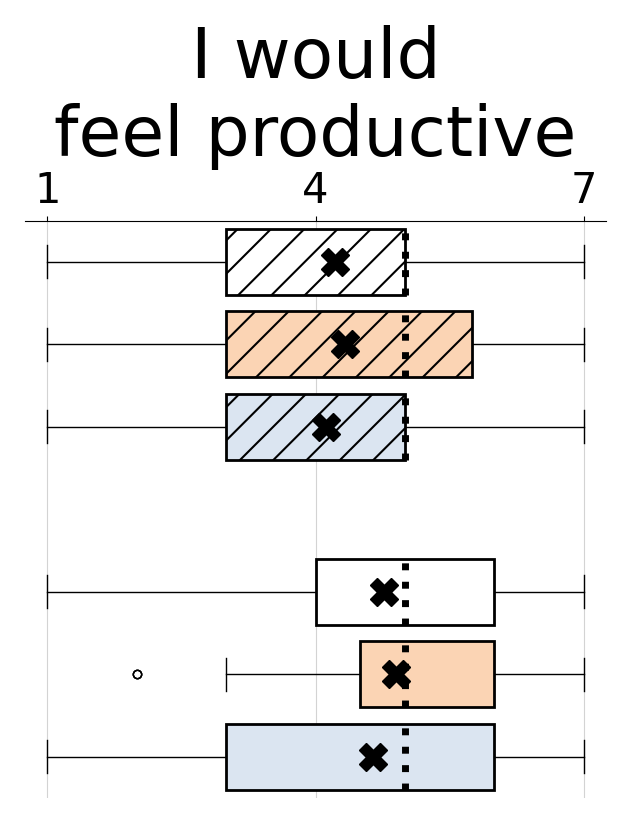}}
    \\
    \hline
    \hline
    \multicolumn{2}{c|}{\includegraphics[width = 0.16\columnwidth]{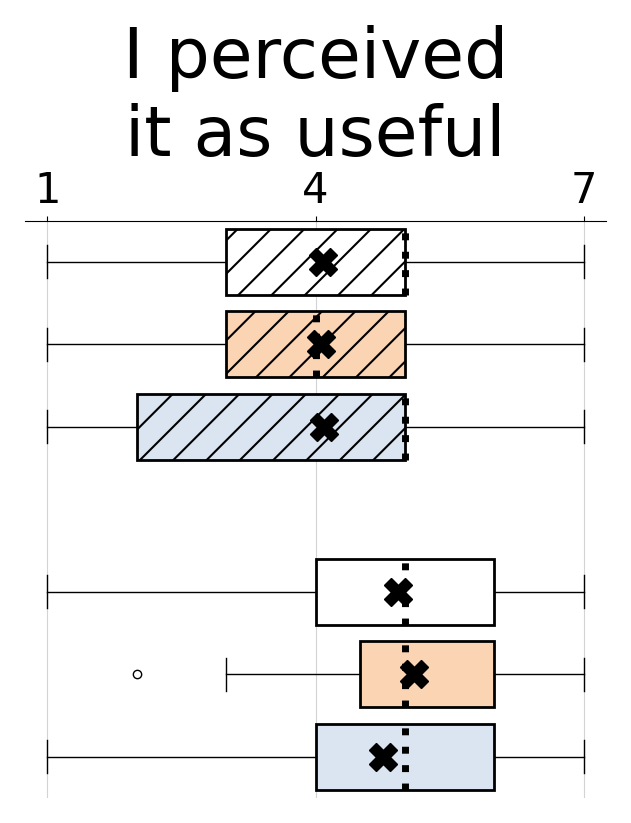}} &
    \multicolumn{2}{c|}{\includegraphics[width = 0.16\columnwidth]{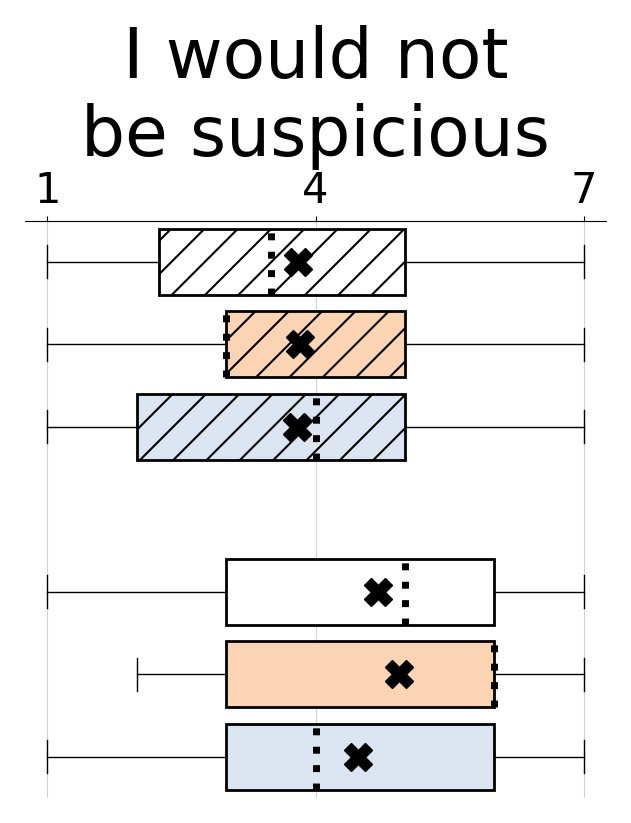}} &
    \multicolumn{2}{c|}{\includegraphics[width = 0.16\columnwidth]{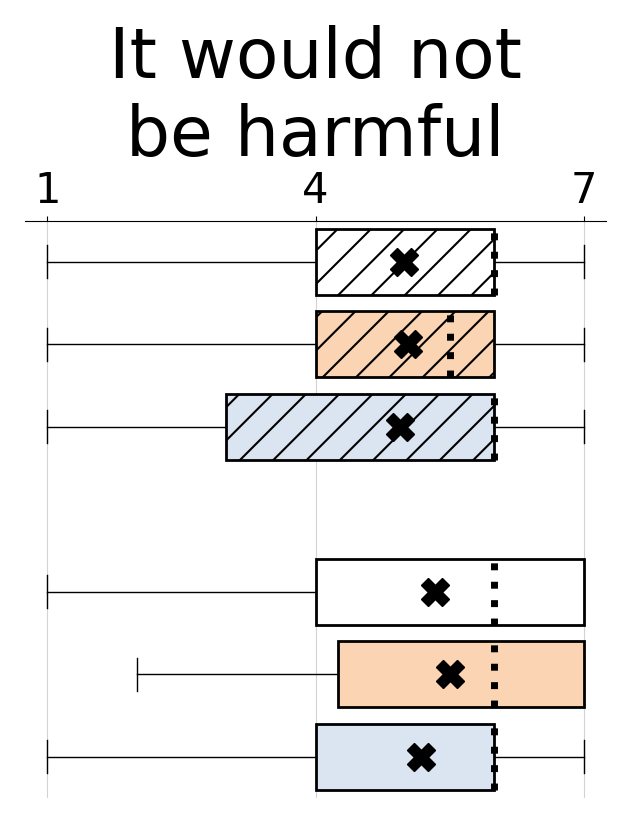}} &
    \multicolumn{2}{c|}{\includegraphics[width = 0.16\columnwidth]{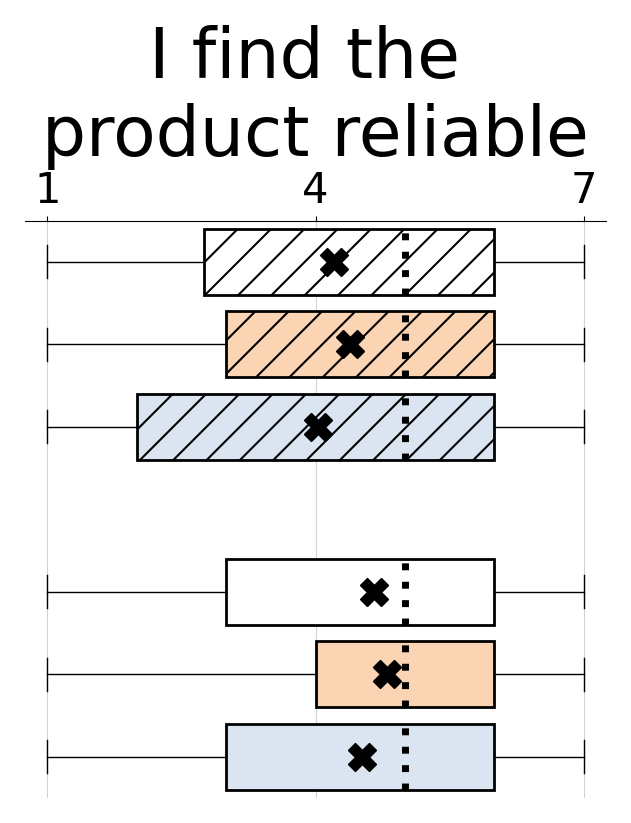}} &
    \multicolumn{2}{c}{\includegraphics[width = 0.16\columnwidth]{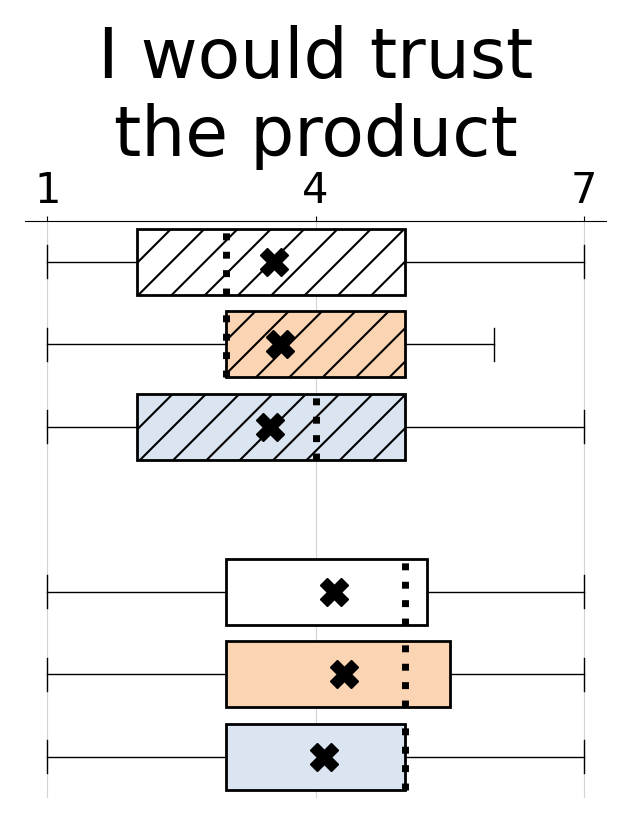}}
    \end{tabular}
    
    \caption{Guideline 15 participants' ratings for all dependent variables, disaggregated by participants' motivations for using technology.
	%For the disaggregated data, notice how large the distances between the average rating are when the guideline is applied.
	Table~\ref{tab:G15-Motiv-Stats-Appendix} below provides the statistics (where applicable).
}
    \label{fig:Motiv-G15-Appendix}
\end{table}

\begin{table}[h]

%\framebox[\linewidth]{For Measuring!}
\centering
\footnotesize

    \begin{tabular}{p{0.22\columnwidth}|c|c|c|c|c|c}
    
    \rowcolor{LightGray}\multicolumn{7}{c}{\textbf{Violation AI Product}}\\
    \hline
    \textbf{Dependent}  & \textbf{Distance b/w} &  &  & & \textbf{Bonferroni} &  \\
    \textbf{variable} & \textbf{Means} &  \textbf{df} &  \textbf{t-val} &   \textbf{p-value}  & \textbf{correction} & \textbf{Cohen's \textit{d}} \\
    \hline
    
    I would feel in control & - - - & - &  - - - & - - - & - - - & - - -  \\
    \hline
    
    I would feel secure &  - - - & - &  - - - & - - - & - - - & - - - \\
    \hline
    
    I would feel adequate &  - - -  & - &  - - - & - - - & - - - & - - - \\
    \hline
    
    I would feel certain &  - - - & - &  - - - & - - - & - - - & - - - \\
    \hline
    
    I would feel productive &  - - - & - &  - - - & - - - & - - - & - - -   \\
    \hline
    \hline
    
    I perceived it as useful &   - - - & - &  - - - & - - - & - - - & - - -   \\
    \hline
    
    I would not be suspicious &  - - - & - &  - - - & - - - & - - - & - - -   \\
    \hline
    
    It would not be harmful &  - - - & - &  - - - & - - - & - - - & - - -  \\
    \hline
    
    I find the product reliable &  - - - & - &  - - - & - - - & - - - & - - - \\
    \hline
    
    I would trust the product &  - - - & - &  - - - & - - - & - - - & - - - \\
    \hline

    \rowcolor{LightGray}\multicolumn{7}{c}{\textbf{Application AI Product}}\\
    \hline
    \textbf{Dependent}  & \textbf{Distance b/w} &  &  & & \textbf{Bonferroni} &  \\
    \textbf{variable} & \textbf{Means} &  \textbf{df} &  \textbf{t-val} &   \textbf{p-value}  & \textbf{correction} & \textbf{Cohen's \textit{d}} \\
    \hline
    
    I would feel in control & - - - & - &  - - - & - - - & - - - & - - -  \\
    \hline
    
    I would feel secure &  - - - & - &  - - - & - - - & - - - & - - - \\
    \hline
    
    I would feel adequate & - - - & - &  - - - & - - - & - - - & - - - \\
    \hline
    
    I would feel certain & - - - & - &  - - - & - - - & - - - & - - - \\
    \hline
    
    I would feel productive & - - - & - &  - - - & - - - & - - - & - - -   \\
    \hline
    \hline
    
    I perceived it as useful &  - - - & - &  - - - & - - - & - - - & - - -   \\
    \hline
    
    I would not be suspicious & - - - & - &  - - - & - - - & - - - & - - -   \\
    \hline
    
    It would not be harmful & - - - & - &  - - - & - - - & - - - & - - -  \\
    \hline
    
    I find the product reliable & - - - & - &  - - - & - - - & - - - & - - - \\
    \hline
    
    I would trust the product & - - - & - &  - - - & - - - & - - - & - - -

    \end{tabular}

    \caption{Guideline 15's t-test results %(\checkmark if Welch's t-test) 
    for task-oriented vs. tech-oriented participants' average ratings of the independent Violation AI product (top) and Application AI product (bottom), for all 10 dependent variables.
    If dashes (- - -) are present, no statistical test was performed.
    If the number of tests exceeded 5 for each product, Bonferroni correction applied by multiplying p-values by the number of tests performed.
    }
    \label{tab:G15-Motiv-Stats-Appendix}
\end{table}
\clearpage
%---------------------------------------------------- End Guideline 15

%Begin Guideline 17---------------------------------------------------

\begin{table}[]
    \centering
    \begin{tabular}{cc|cc|cc|cc|cc}
    \multicolumn{2}{c|}{\includegraphics[width = 0.16\columnwidth]{assets/05-All-BoxPlots/15-G17/Motiv/G17-Feel-In-Control-MOTIV.png}} &
    \multicolumn{2}{c|}{\includegraphics[width = 0.16\columnwidth]{assets/05-All-BoxPlots/15-G17/Motiv/G17-Feel-Secure-MOTIV.png}} &
    \multicolumn{2}{c|}{\includegraphics[width = 0.16\columnwidth]{assets/05-All-BoxPlots/15-G17/Motiv/G17-Feel-Adequate-MOTIV.png}} &
    \multicolumn{2}{c|}{\includegraphics[width = 0.16\columnwidth]{assets/05-All-BoxPlots/15-G17/Motiv/G17-Feel-Certain-MOTIV.png}} &
    \multicolumn{2}{c}{\includegraphics[width = 0.16\columnwidth]{assets/05-All-BoxPlots/15-G17/Motiv/G17-Feel-Productive-MOTIV.png}}
    \\
    \hline
    \hline
    \multicolumn{2}{c|}{\includegraphics[width = 0.16\columnwidth]{assets/05-All-BoxPlots/15-G17/Motiv/G17-Perceived-Useful-MOTIV.png}} &
    \multicolumn{2}{c|}{\includegraphics[width = 0.16\columnwidth]{assets/05-All-BoxPlots/15-G17/Motiv/G17-Not-Suspicious-MOTIV.png}} &
    \multicolumn{2}{c|}{\includegraphics[width = 0.16\columnwidth]{assets/05-All-BoxPlots/15-G17/Motiv/G17-Not-Harmful-MOTIV.png}} &
    \multicolumn{2}{c|}{\includegraphics[width = 0.16\columnwidth]{assets/05-All-BoxPlots/15-G17/Motiv/G17-Product-Reliable-MOTIV.png}} &
    \multicolumn{2}{c}{\includegraphics[width = 0.16\columnwidth]{assets/05-All-BoxPlots/15-G17/Motiv/G17-Trust-Product-MOTIV.png}}
    \end{tabular}
    
    \caption{Guideline 17 participants' ratings for all dependent variables, disaggregated by participants' motivations for using technology.
	%For the disaggregated data, notice how large the distances between the average rating are when the guideline is applied.
	Table~\ref{tab:G17-Motiv-Stats-Appendix} below provides the statistics (where applicable).
}
    \label{fig:Motiv-G17-Appendix}
\end{table}

\begin{table}[h]

%\framebox[\linewidth]{For Measuring!}
\centering
\footnotesize

    \begin{tabular}{p{0.22\columnwidth}|c|c|c|c|c|c}
    
    \rowcolor{LightGray}\multicolumn{7}{c}{\textbf{Violation AI Product}}\\
    \hline
    \textbf{Dependent}  & \textbf{Distance b/w} &  &  & & \textbf{Bonferroni} &  \\
    \textbf{variable} & \textbf{Means} &  \textbf{df} &  \textbf{t-val} &   \textbf{p-value}  & \textbf{correction} & \textbf{Cohen's \textit{d}} \\
    \hline
    
    I would feel in control & - - - & - &  - - - & - - - & - - - & - - -  \\
    \hline
    
    I would feel secure & - - - & - &  - - - & - - - & - - - & - - - \\
    \hline
    
    I would feel adequate & - - -  & - &  - - - & - - - & - - - & - - - \\
    \hline
    
    I would feel certain & - - - & - &  - - - & - - - & - - - & - - - \\
    \hline
    
    I would feel productive & - - - & - &  - - - & - - - & - - - & - - -   \\
    \hline
    \hline
    
    I perceived it as useful &  - - - & - &  - - - & - - - & - - - & - - -   \\
    \hline
    
    I would not be suspicious & - - - & - &  - - - & - - - & - - - & - - -   \\
    \hline
    
    It would not be harmful & - - - & - &  - - - & - - - & - - - & - - -  \\
    \hline
    
    I find the product reliable & - - - & - &  - - - & - - - & - - - & - - - \\
    \hline
    
    I would trust the product & - - - & - &  - - - & - - - & - - - & - - - \\
    \hline

    \rowcolor{LightGray}\multicolumn{7}{c}{\textbf{Application AI Product}}\\
    \hline
    \textbf{Dependent}  & \textbf{Distance b/w} &  &  & & \textbf{Bonferroni} &  \\
    \textbf{variable} & \textbf{Means} &  \textbf{df} &  \textbf{t-val} &   \textbf{p-value}  & \textbf{correction} & \textbf{Cohen's \textit{d}} \\
    \hline
    
    I would feel in control & - - - & - &  - - - & - - - & - - - & - - -  \\
    \hline
    
    I would feel secure & - - - & - &  - - - & - - - & - - - & - - - \\
    \hline
    
    I would feel adequate & - - -  & - &  - - - & - - - & - - - & - - - \\
    \hline
    
    I would feel certain & - - - & - &  - - - & - - - & - - - & - - - \\
    \hline
    
    I would feel productive & - - - & - &  - - - & - - - & - - - & - - -   \\
    \hline
    \hline
    
    I perceived it as useful &  - - - & - &  - - - & - - - & - - - & - - -   \\
    \hline
    
    I would not be suspicious & - - - & - &  - - - & - - - & - - - & - - -   \\
    \hline
    
    It would not be harmful & - - - & - &  - - - & - - - & - - - & - - -  \\
    \hline
    
    I find the product reliable & - - - & - &  - - - & - - - & - - - & - - - \\
    \hline
    
    I would trust the product & - - - & - &  - - - & - - - & - - - & - - -

    \end{tabular}

    \caption{Guideline 17's t-test results %(\checkmark if Welch's t-test) 
    for task-oriented vs. tech-oriented participants' average ratings of the independent Violation AI product (top) and Application AI product (bottom), for all 10 dependent variables.
    If dashes (- - -) are present, no statistical test was performed.
    If the number of tests exceeded 5 for each product, Bonferroni correction applied by multiplying p-values by the number of tests performed.
    }
    \label{tab:G17-Motiv-Stats-Appendix}
\end{table}
\clearpage
%---------------------------------------------------- End Guideline 17

%Begin Guideline 17---------------------------------------------------

\begin{table}[]
    \centering
    \begin{tabular}{cc|cc|cc|cc|cc}
    \multicolumn{2}{c|}{\includegraphics[width = 0.16\columnwidth]{assets/05-All-BoxPlots/16-G18/Motiv/G18-Feel-In-Control-MOTIV.png}} &
    \multicolumn{2}{c|}{\includegraphics[width = 0.16\columnwidth]{assets/05-All-BoxPlots/16-G18/Motiv/G18-Feel-Secure-MOTIV.png}} &
    \multicolumn{2}{c|}{\includegraphics[width = 0.16\columnwidth]{assets/05-All-BoxPlots/16-G18/Motiv/G18-Feel-Adequate-MOTIV.png}} &
    \multicolumn{2}{c|}{\includegraphics[width = 0.16\columnwidth]{assets/05-All-BoxPlots/16-G18/Motiv/G18-Feel-Certain-MOTIV.png}} &
    \multicolumn{2}{c}{\includegraphics[width = 0.16\columnwidth]{assets/05-All-BoxPlots/16-G18/Motiv/G18-Feel-Productive-MOTIV.png}}
    \\
    \hline
    \hline
    \multicolumn{2}{c|}{\includegraphics[width = 0.16\columnwidth]{assets/05-All-BoxPlots/16-G18/Motiv/G18-Perceived-Useful-MOTIV.png}} &
    \multicolumn{2}{c|}{\includegraphics[width = 0.16\columnwidth]{assets/05-All-BoxPlots/16-G18/Motiv/G18-Not-Suspicious-MOTIV.png}} &
    \multicolumn{2}{c|}{\includegraphics[width = 0.16\columnwidth]{assets/05-All-BoxPlots/16-G18/Motiv/G18-Not-Harmful-MOTIV.png}} &
    \multicolumn{2}{c|}{\includegraphics[width = 0.16\columnwidth]{assets/05-All-BoxPlots/16-G18/Motiv/G18-Product-Reliable-MOTIV.png}} &
    \multicolumn{2}{c}{\includegraphics[width = 0.16\columnwidth]{assets/05-All-BoxPlots/16-G18/Motiv/G18-Trust-Product-MOTIV.png}}
    \end{tabular}
    
    \caption{Guideline 18 participants' ratings for all dependent variables, disaggregated by participants' motivations for using technology.
	%For the disaggregated data, notice how large the distances between the average rating are when the guideline is applied.
	Table~\ref{tab:G18-Motiv-Stats-Appendix} below provides the statistics (where applicable).
}
    \label{fig:Motiv-G18-Appendix}
\end{table}

\begin{table}[h]

%\framebox[\linewidth]{For Measuring!}
\centering
\footnotesize

    \begin{tabular}{p{0.22\columnwidth}|c|c|c|c|c|c}
    
    \rowcolor{LightGray}\multicolumn{7}{c}{\textbf{Violation AI Product}}\\
    \hline
    \textbf{Dependent}  & \textbf{Distance b/w} &  &  & & \textbf{Bonferroni} &  \\
    \textbf{variable} & \textbf{Means} &  \textbf{df} &  \textbf{t-val} &   \textbf{p-value}  & \textbf{correction} & \textbf{Cohen's \textit{d}} \\
    \hline
    
    I would feel in control & - - -  & - &  - - - & - - - & - - - & - - -  \\
    \hline
    
    I would feel secure & - - -  & - &  - - - & - - - & - - - & - - - \\
    \hline
    
    I would feel adequate & - - -  & - &  - - - & - - - & - - - & - - - \\
    \hline
    
    I would feel certain & - - -  & - &  - - - & - - - & - - - & - - - \\
    \hline
    
    I would feel productive & - - - & - &  - - - & - - - & - - - & - - -   \\
    \hline
    \hline
    
    I perceived it as useful &  - - - & - &  - - - & - - - & - - - & - - -   \\
    \hline
    
    I would not be suspicious & - - -  & - &  - - - & - - - & - - - & - - -   \\
    \hline
    
    It would not be harmful & - - - & - &  - - - & - - - & - - - & - - -  \\
    \hline
    
    I find the product reliable & - - - & - &  - - - & - - - & - - - & - - - \\
    \hline
    
    I would trust the product & - - - & - &  - - - & - - - & - - - & - - - \\
    \hline

    \rowcolor{LightGray}\multicolumn{7}{c}{\textbf{Application AI Product}}\\
    \hline
    \textbf{Dependent}  & \textbf{Distance b/w} &  &  & & \textbf{Bonferroni} &  \\
    \textbf{variable} & \textbf{Means} &  \textbf{df} &  \textbf{t-val} &   \textbf{p-value}  & \textbf{correction} & \textbf{Cohen's \textit{d}} \\
    \hline
    
    I would feel in control & 0.8788 & 64 &  2.4698 & \cellcolor{AbiOrangeQuote}.0162 & - - - & 0.608  \\
    \hline
    
    I would feel secure & - - - & - &  - - - & - - - & - - - & - - - \\
    \hline
    
    I would feel adequate & - - -  & - &  - - - & - - - & - - - & - - - \\
    \hline
    
    I would feel certain & 0.8476 & 65 &  2.1207 & \cellcolor{AbiOrangeQuote}.0378 & - - - & .0.5182 \\
    \hline
    
    I would feel productive & - - -  & - &  - - - & - - - & - - - & - - -   \\
    \hline
    \hline
    
    I perceived it as useful &  0.5074 & 64 &  1.5892 & .1169 & - - - & 0.3914   \\
    \hline
    
    I would not be suspicious & 0.7279 & 64 &  1.9099 & .0606 & - - - & 0.4704   \\
    \hline
    
    It would not be harmful & - - - & - &  - - - & - - - & - - - & - - - \\
    \hline
    
    I find the product reliable & - - - & - &  - - - & - - - & - - - & - - - \\
    \hline
    
    I would trust the product & - - - & - &  - - - & - - - & - - - & - - -

    \end{tabular}

    \caption{Guideline 18's t-test results %(\checkmark if Welch's t-test) 
    for task-oriented vs. tech-oriented participants' average ratings of the independent Violation AI product (top) and Application AI product (bottom), for all 10 dependent variables.
    If dashes (- - -) are present, no statistical test was performed.
    If the number of tests exceeded 5 for each product, Bonferroni correction applied by multiplying p-values by the number of tests performed.
    }
    \label{tab:G18-Motiv-Stats-Appendix}
\end{table}
\clearpage
%---------------------------------------------------- End Guideline 18
