# Supplementary material for: Measuring User Experience Inclusivity in Human-AI Interaction via Five User Problem-Solving Styles
Source: arXiv:2108.00588 source file (2024-02-17)
Supplement: Supplementary file 10 [file Risk-Appendix.tex]

%Guideline 1 ------------------------------
\begin{table}[]
    \centering
    \begin{tabular}{cc|cc|cc|cc|cc}
    \multicolumn{2}{c|}{\includegraphics[width = 0.16\columnwidth]{assets/05-All-BoxPlots/01-G1/Risk/G1-Feel-In-Control-RISK.png}} &
    \multicolumn{2}{c|}{\includegraphics[width = 0.16\columnwidth]{assets/05-All-BoxPlots/01-G1/Risk/G1-Feel-Secure-RISK.png}} &
    \multicolumn{2}{c|}{\includegraphics[width = 0.16\columnwidth]{assets/05-All-BoxPlots/01-G1/Risk/G1-Feel-Adequate-RISK.png}} &
    \multicolumn{2}{c|}{\includegraphics[width = 0.16\columnwidth]{assets/05-All-BoxPlots/01-G1/Risk/G1-Feel-Certain-RISK.png}} &
    \multicolumn{2}{c}{\includegraphics[width = 0.16\columnwidth]{assets/05-All-BoxPlots/01-G1/Risk/G1-Feel-Productive-RISK.png}}
    \\
    \hline
    \hline
    \multicolumn{2}{c|}{\includegraphics[width = 0.16\columnwidth]{assets/05-All-BoxPlots/01-G1/Risk/G1-Perceived-Useful-RISK.png}} &
    \multicolumn{2}{c|}{\includegraphics[width = 0.16\columnwidth]{assets/05-All-BoxPlots/01-G1/Risk/G1-Not-Suspicious-RISK.png}} &
    \multicolumn{2}{c|}{\includegraphics[width = 0.16\columnwidth]{assets/05-All-BoxPlots/01-G1/Risk/G1-Not-Harmful-RISK.png}} &
    \multicolumn{2}{c|}{\includegraphics[width = 0.16\columnwidth]{assets/05-All-BoxPlots/01-G1/Risk/G1-Product-Reliable-RISK.png}} &
    \multicolumn{2}{c}{\includegraphics[width = 0.16\columnwidth]{assets/05-All-BoxPlots/01-G1/Risk/G1-Trust-Product-RISK.png}}
    \end{tabular}
    
    \caption{Guideline 1 participants' ratings for all dependent variables, disaggregated by participants' attitudes toward risk.
	%For the disaggregated data, notice how large the distances between the average rating are when the guideline is applied.
	Table~\ref{tab:G1-Risk-Stats-Appendix} below provides the statistics (where applicable).
}
    \label{fig:Risk-G1-Appendix}
\end{table}

\begin{table}[h]

%\framebox[\linewidth]{For Measuring!}
\centering
\footnotesize

    \begin{tabular}{p{0.22\columnwidth}|c|c|c|c|c|c}
    
    \rowcolor{LightGray}\multicolumn{7}{c}{\textbf{Violation AI Product}}\\
    \hline
    \textbf{Dependent}  & \textbf{Distance b/w} &  &  & & \textbf{Bonferroni} &  \\
    \textbf{variable} & \textbf{Means} &  \textbf{df} &  \textbf{t-val} &   \textbf{p-value}  & \textbf{correction} & \textbf{Cohen's \textit{d}} \\
    \hline
    
    I would feel in control & - - - & - &  - - - & - - - & - - - & - - -\\
    \hline
    
    I would feel secure & - - - & - &  - - - & - - - & - - - & - - - \\
    \hline
    
    I would feel adequate & - - - & - &  - - - & - - - & - - - & - - - \\
    \hline
    
    I would feel certain & - - - & - &  - - - & - - - & - - - & - - - \\
    \hline
    
    I would feel productive & - - - & - &  - - - & - - - & - - - & - - -  \\
    \hline
    \hline
    
    I perceived it as useful &  - - - & - &  - - - & - - - & - - - & - - -  \\
    \hline
    
    I would not be suspicious & - - - & - &  - - - & - - - & - - - & - - -  \\
    \hline
    
    It would not be harmful & - - - & - &  - - - & - - - & - - - & - - -  \\
    \hline
    
    I find the product reliable & - - - & - &  - - - & - - - & - - - & - - -  \\
    \hline
    
    I would trust the product & - - - & - &  - - - & - - - & - - - & - - - \\
    \hline

    \rowcolor{LightGray}\multicolumn{7}{c}{\textbf{Application AI Product}}\\
    \hline
    \textbf{Dependent}  & \textbf{Distance b/w} &  &  & & \textbf{Bonferroni} &  \\
    \textbf{variable} & \textbf{Means} &  \textbf{df} &  \textbf{t-val} &   \textbf{p-value}  & \textbf{correction} & \textbf{Cohen's \textit{d}} \\
    \hline
    
    I would feel in control & - - - & - &  - - - & - - - & - - - & - - -  \\
    \hline
    
    I would feel secure & - - - & - &  - - - & - - - & - - - & - - - \\
    \hline
    
    I would feel adequate & - - - & - &  - - - & - - - & - - - & - - - \\
    \hline
    
    I would feel certain & - - - & - &  - - - & - - - & - - - & - - - \\
    \hline
    
    I would feel productive & - - - & - &  - - - & - - - & - - - & - - -   \\
    \hline
    \hline
    
    I perceived it as useful &  - - - & - &  - - - & - - - & - - - & - - -  \\
    \hline
    
    I would not be suspicious & - - - & - &  - - - & - - - & - - - & - - -  \\
    \hline
    
    It would not be harmful & - - - & - &  - - - & - - - & - - - & - - -  \\
    \hline
    
    I find the product reliable & - - - & - &  - - - & - - - & - - - & - - - \\
    \hline
    
    I would trust the product & - - - & - &  - - - & - - - & - - - & - - -

    \end{tabular}

    \caption{Guideline 4's t-test results %(\checkmark if Welch's t-test) 
    for risk-averse vs. risk-tolerant participants' average ratings of the independent Violation AI product (top) and Application AI product (bottom), for all 10 dependent variables.
    If dashes (- - -) are present, no statistical test was performed.
    If the number of tests exceeded 5 for each product, Bonferroni correction applied by multiplying p-values by the number of tests performed.
    }
    \label{tab:G1-Risk-Stats-Appendix}
    
    % \FIXME{MMB@AAA: FYI, I took the \checkmark s out and replaced them with plain text, because the \checkmark vs blank visually stood out so much, I kept mis-seeing it as saying only those 4 rows were signif. or important.\\
    % AAA@MMB: Redid it with Y/N. The Welch's t and t were cluttering up the table too much.\\
    % MMB@AAA: I actually prefer the spelled-out way.  Visually, the table layout now screams WELCHES IS GOOD, and draws attention away from all other columns.  Meta-comment: it might help if you forced yourself to look at this paper with a reader hat on.}

\end{table}

\clearpage
%---------------------------------------------------- End Guideline 1

%Guideline 3 ------------------------------
\begin{table}[]
    \centering
    \begin{tabular}{cc|cc|cc|cc|cc}
    \multicolumn{2}{c|}{\includegraphics[width = 0.16\columnwidth]{assets/05-All-BoxPlots/02-G3/Risk/G3-Feel-In-Control-RISK.png}} &
    \multicolumn{2}{c|}{\includegraphics[width = 0.16\columnwidth]{assets/05-All-BoxPlots/02-G3/Risk/G3-Feel-Secure-RISK.png}} &
    \multicolumn{2}{c|}{\includegraphics[width = 0.16\columnwidth]{assets/05-All-BoxPlots/02-G3/Risk/G3-Feel-Adequate-RISK.png}} &
    \multicolumn{2}{c|}{\includegraphics[width = 0.16\columnwidth]{assets/05-All-BoxPlots/02-G3/Risk/G3-Feel-Certain-RISK.png}} &
    \multicolumn{2}{c}{\includegraphics[width = 0.16\columnwidth]{assets/05-All-BoxPlots/02-G3/Risk/G3-Feel-Productive-RISK.png}}
    \\
    \hline
    \hline
    \multicolumn{2}{c|}{\includegraphics[width = 0.16\columnwidth]{assets/05-All-BoxPlots/02-G3/Risk/G3-Perceived-Useful-RISK.png}} &
    \multicolumn{2}{c|}{\includegraphics[width = 0.16\columnwidth]{assets/05-All-BoxPlots/02-G3/Risk/G3-Not-Suspicious-RISK.png}} &
    \multicolumn{2}{c|}{\includegraphics[width = 0.16\columnwidth]{assets/05-All-BoxPlots/02-G3/Risk/G3-Not-Harmful-RISK.png}} &
    \multicolumn{2}{c|}{\includegraphics[width = 0.16\columnwidth]{assets/05-All-BoxPlots/02-G3/Risk/G3-Product-Reliable-RISK.png}} &
    \multicolumn{2}{c}{\includegraphics[width = 0.16\columnwidth]{assets/05-All-BoxPlots/02-G3/Risk/G3-Trust-Product-RISK.png}}
    \end{tabular}
    
    \caption{Guideline 3 participants' ratings for all dependent variables, disaggregated by participants' attitudes toward risk.
	%For the disaggregated data, notice how large the distances between the average rating are when the guideline is applied.
	Table~\ref{tab:G3-Risk-Stats-Appendix} below provides the statistics (where applicable).
}
    \label{fig:Risk-G3-Appendix}
\end{table}

\begin{table}[h]

%\framebox[\linewidth]{For Measuring!}
\centering
\footnotesize

    \begin{tabular}{p{0.22\columnwidth}|c|c|c|c|c|c}
    
    \rowcolor{LightGray}\multicolumn{7}{c}{\textbf{Violation AI Product}}\\
    \hline
    \textbf{Dependent}  & \textbf{Distance b/w} &  &  & & \textbf{Bonferroni} &  \\
    \textbf{variable} & \textbf{Means} &  \textbf{df} &  \textbf{t-val} &   \textbf{p-value}  & \textbf{correction} & \textbf{Cohen's \textit{d}} \\
    \hline
    
    I would feel in control & - - - & - &  - - - & - - - & - - - & - - -\\
    \hline
    
    I would feel secure & - - - & - &  - - - & - - - & - - - & - - - \\
    \hline
    
    I would feel adequate & - - - & - &  - - - & - - - & - - - & - - - \\
    \hline
    
    I would feel certain & - - - & - &  - - - & - - - & - - - & - - - \\
    \hline
    
    I would feel productive & - - - & - &  - - - & - - - & - - - & - - -  \\
    \hline
    \hline
    
    I perceived it as useful &  - - - & - &  - - - & - - - & - - - & - - -  \\
    \hline
    
    I would not be suspicious & - - - & - &  - - - & - - - & - - - & - - -  \\
    \hline
    
    It would not be harmful & - - - & - &  - - - & - - - & - - - & - - -  \\
    \hline
    
    I find the product reliable & - - - & - &  - - - & - - - & - - - & - - -  \\
    \hline
    
    I would trust the product & - - - & - &  - - - & - - - & - - - & - - - \\
    \hline

    \rowcolor{LightGray}\multicolumn{7}{c}{\textbf{Application AI Product}}\\
    \hline
    \textbf{Dependent}  & \textbf{Distance b/w} &  &  & & \textbf{Bonferroni} &  \\
    \textbf{variable} & \textbf{Means} &  \textbf{df} &  \textbf{t-val} &   \textbf{p-value}  & \textbf{correction} & \textbf{Cohen's \textit{d}} \\
    \hline
    
    I would feel in control & - - - & - &  - - - & - - - & - - - & - - -  \\
    \hline
    
    I would feel secure & - - - & - &  - - - & - - - & - - - & - - - \\
    \hline
    
    I would feel adequate & - - - & - &  - - - & - - - & - - - & - - - \\
    \hline
    
    I would feel certain & - - - & - &  - - - & - - - & - - - & - - - \\
    \hline
    
    I would feel productive & - - - & - &  - - - & - - - & - - - & - - -   \\
    \hline
    \hline
    
    I perceived it as useful &  - - - & - &  - - - & - - - & - - - & - - -  \\
    \hline
    
    I would not be suspicious & - - - & - &  - - - & - - - & - - - & - - -  \\
    \hline
    
    It would not be harmful & - - - & - &  - - - & - - - & - - - & - - -  \\
    \hline
    
    I find the product reliable & - - - & - &  - - - & - - - & - - - & - - - \\
    \hline
    
    I would trust the product & - - - & - &  - - - & - - - & - - - & - - -

    \end{tabular}

    \caption{Guideline 3's t-test results %(\checkmark if Welch's t-test) 
    for risk-averse vs. risk-tolerant participants' average ratings of the independent Violation AI product (top) and Application AI product (bottom), for all 10 dependent variables.
    If dashes (- - -) are present, no statistical test was performed.
    If the number of tests exceeded 5 for each product, Bonferroni correction applied by multiplying p-values by the number of tests performed.
    }
    \label{tab:G3-Risk-Stats-Appendix}
    
    % \FIXME{MMB@AAA: FYI, I took the \checkmark s out and replaced them with plain text, because the \checkmark vs blank visually stood out so much, I kept mis-seeing it as saying only those 4 rows were signif. or important.\\
    % AAA@MMB: Redid it with Y/N. The Welch's t and t were cluttering up the table too much.\\
    % MMB@AAA: I actually prefer the spelled-out way.  Visually, the table layout now screams WELCHES IS GOOD, and draws attention away from all other columns.  Meta-comment: it might help if you forced yourself to look at this paper with a reader hat on.}

\end{table}

\clearpage
%---------------------------------------------------- End Guideline 3

%Begin Guideline 4----------------------------------------------------

\begin{table}[]
    \centering
    \begin{tabular}{cc|cc|cc|cc|cc}
    \multicolumn{2}{c|}{\includegraphics[width = 0.16\columnwidth]{assets/05-All-BoxPlots/03-G4/Risk/G4-Feel-In-Control-RISK.png}} &
    \multicolumn{2}{c|}{\includegraphics[width = 0.16\columnwidth]{assets/05-All-BoxPlots/03-G4/Risk/G4-Feel-Secure-RISK.png}} &
    \multicolumn{2}{c|}{\includegraphics[width = 0.16\columnwidth]{assets/05-All-BoxPlots/03-G4/Risk/G4-Feel-Adequate-RISK.png}} &
    \multicolumn{2}{c|}{\includegraphics[width = 0.16\columnwidth]{assets/05-All-BoxPlots/03-G4/Risk/G4-Feel-Certain-RISK.png}} &
    \multicolumn{2}{c}{\includegraphics[width = 0.16\columnwidth]{assets/05-All-BoxPlots/03-G4/Risk/G4-Feel-Productive-RISK.png}}
    \\
    \hline
    \hline
    \multicolumn{2}{c|}{\includegraphics[width = 0.16\columnwidth]{assets/05-All-BoxPlots/03-G4/Risk/G4-Perceived-Useful-RISK.png}} &
    \multicolumn{2}{c|}{\includegraphics[width = 0.16\columnwidth]{assets/05-All-BoxPlots/03-G4/Risk/G4-Not-Suspicious-RISK.png}} &
    \multicolumn{2}{c|}{\includegraphics[width = 0.16\columnwidth]{assets/05-All-BoxPlots/03-G4/Risk/G4-Not-Harmful-RISK.png}} &
    \multicolumn{2}{c|}{\includegraphics[width = 0.16\columnwidth]{assets/05-All-BoxPlots/03-G4/Risk/G4-Product-Reliable-RISK.png}} &
    \multicolumn{2}{c}{\includegraphics[width = 0.16\columnwidth]{assets/05-All-BoxPlots/03-G4/Risk/G4-Trust-Product-RISK.png}}
    \end{tabular}
    
    \caption{Guideline 4 participants' ratings for all dependent variables, disaggregated by participants' attitudes toward risk.
	%For the disaggregated data, notice how large the distances between the average rating are when the guideline is applied.
	Table~\ref{tab:G4-Risk-Stats-Appendix} below provides the statistics (where applicable).
}
    \label{fig:Risk-G4-Appendix}
\end{table}

\begin{table}[h]

%\framebox[\linewidth]{For Measuring!}
\centering
\footnotesize

    \begin{tabular}{p{0.22\columnwidth}|c|c|c|c|c|c}
    
    \rowcolor{LightGray}\multicolumn{7}{c}{\textbf{Violation AI Product}}\\
    \hline
    \textbf{Dependent}  & \textbf{Distance b/w} &  &  & & \textbf{Bonferroni} &  \\
    \textbf{variable} & \textbf{Means} &  \textbf{df} &  \textbf{t-val} &   \textbf{p-value}  & \textbf{correction} & \textbf{Cohen's \textit{d}} \\
    \hline
    
    I would feel in control & 0.4444 & 61 &  1.6268 & .109 & 1 & \\
    \hline
    
    I would feel secure & 0.6667 & 62 & 2.3006 & \cellcolor{AbiOrangeQuote}{.0248} & {.248} & 0.580 \\
    \hline
    
    I would feel adequate & 0.8704 & 61 & 2.9179 & \cellcolor{AbiOrangeQuote}{.0049} &  .049 & 0.743 \\
    \hline
    
    I would feel certain & 1.2798 &  62 & 3.6258 & \cellcolor{AbiOrangeQuote}{.0005} & .005 & 0.910 \\
    \hline
    
    I would feel productive & 0.5397 & 62  & 2.2066 & .0311 & .311 & 0.556  \\
    \hline
    \hline
    
    I perceived it as useful &  0.5119 & 62  & 1.6623 & .102 & 1   &  \\
    \hline
    
    I would not be suspicious & 1.6468 & 34   & 4.8630  & \cellcolor{AbiOrangeQuote}$< .0001$ & $< .001$ & 1.337  \\
    \hline
    
    It would not be harmful & 0.7893 & 39  & 2.8694  & \cellcolor{AbiOrangeQuote}.0066  & .066   & 0.763  \\
    \hline
    
    I find the product reliable & 0.6312 & 49 & 2.0046   & .051  & .510  &  \\
    \hline
    
    I would trust the product & 0.7519 &  63  & 2.6615  & \cellcolor{AbiOrangeQuote}.010 & .100  & 0.664 \\
    \hline

    \rowcolor{LightGray}\multicolumn{7}{c}{\textbf{Application AI Product}}\\
    \hline
    \textbf{Dependent}  & \textbf{Distance b/w} &  &  & & \textbf{Bonferroni} &  \\
    \textbf{variable} & \textbf{Means} &  \textbf{df} &  \textbf{t-val} &   \textbf{p-value}  & \textbf{correction} & \textbf{Cohen's \textit{d}} \\
    \hline
    
    I would feel in control & 0.9643 & 62 &  3.2128  &  .0021  & .021  & 0.810  \\
    \hline
    
    I would feel secure & 1.0093 & 61 & 3.1984 & \cellcolor{AbiOrangeQuote}{.0022} & {.022} & 0.814 \\
    \hline
    
    I would feel adequate & 0.8492 & 62 & 2.4955 & \cellcolor{AbiOrangeQuote}{.0153} &  .153 & 0.629 \\
    \hline
    
    I would feel certain & 1.6916 &   63 & 4.7513 & \cellcolor{AbiOrangeQuote}{$<.0001$} & {$<.001$} & 1.186 \\
    \hline
    
    I would feel productive & 0.4598 & 63  & 1.8462  &  .0696  & .696  &    \\
    \hline
    \hline
    
    I perceived it as useful &  0.7854 & 63  & 2.981  &  .0041  & .041   & 0.744   \\
    \hline
    
    I would not be suspicious & 1.8008 & 42   & 5.1692  & \cellcolor{AbiOrangeQuote}$< .0001$ & {$<.001$} & 1.364   \\
    \hline
    
    It would not be harmful & 0.9607 & 44  & 3.1328  & \cellcolor{AbiOrangeQuote}.0031  & .031   & 0.821  \\
    \hline
    
    I find the product reliable & 0.8170 & 50 & 2.6298  & .0113  & .113  &  0.678 \\
    \hline
    
    I would trust the product & 1.0635 &  62  & 3.7170  & \cellcolor{AbiOrangeQuote}.0004  & .004  & 0.937

    \end{tabular}

    \caption{Guideline 4's t-test results %(\checkmark if Welch's t-test) 
    for risk-averse vs. risk-tolerant participants' average ratings of the independent Violation AI product (top) and Application AI product (bottom), for all 10 dependent variables.
    If dashes (- - -) are present, no statistical test was performed.
    If the number of tests exceeded 5 for each product, Bonferroni correction applied by multiplying p-values by the number of tests performed.
    }
    \label{tab:G4-Risk-Stats-Appendix}
\end{table}

%---------------------------------------------------- End Guideline 4

\clearpage

%Begin Guideline 5----------------------------------------------------

\begin{table}[]
    \centering
    \begin{tabular}{cc|cc|cc|cc|cc}
    \multicolumn{2}{c|}{\includegraphics[width = 0.16\columnwidth]{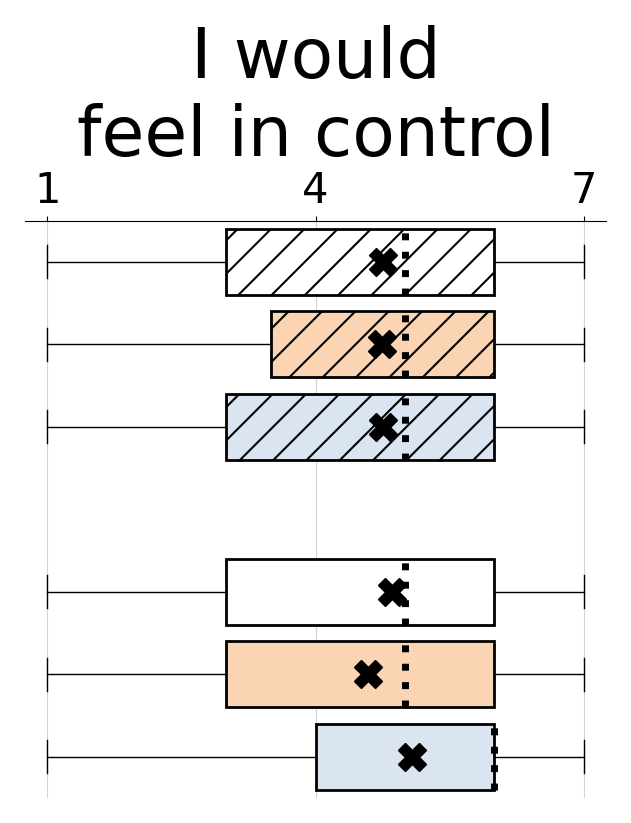}} &
    \multicolumn{2}{c|}{\includegraphics[width = 0.16\columnwidth]{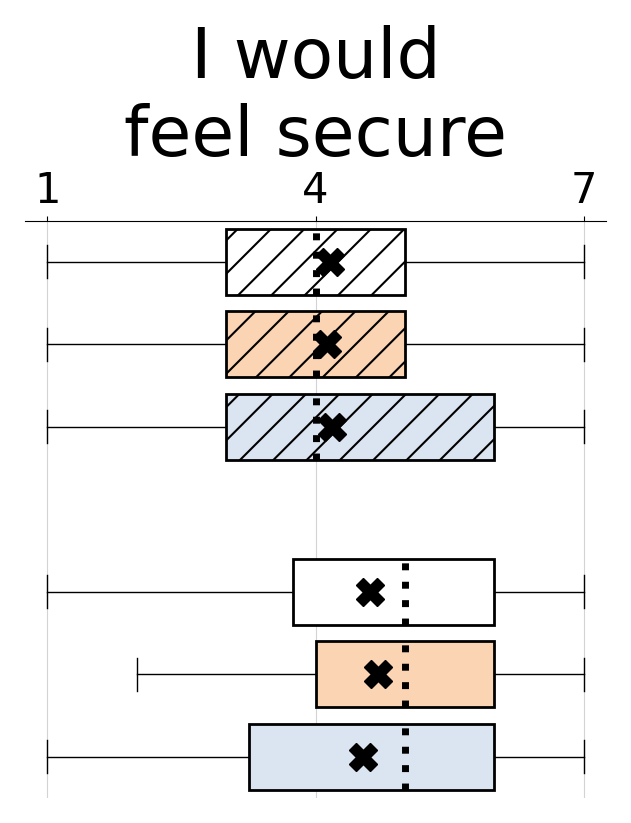}} &
    \multicolumn{2}{c|}{\includegraphics[width = 0.16\columnwidth]{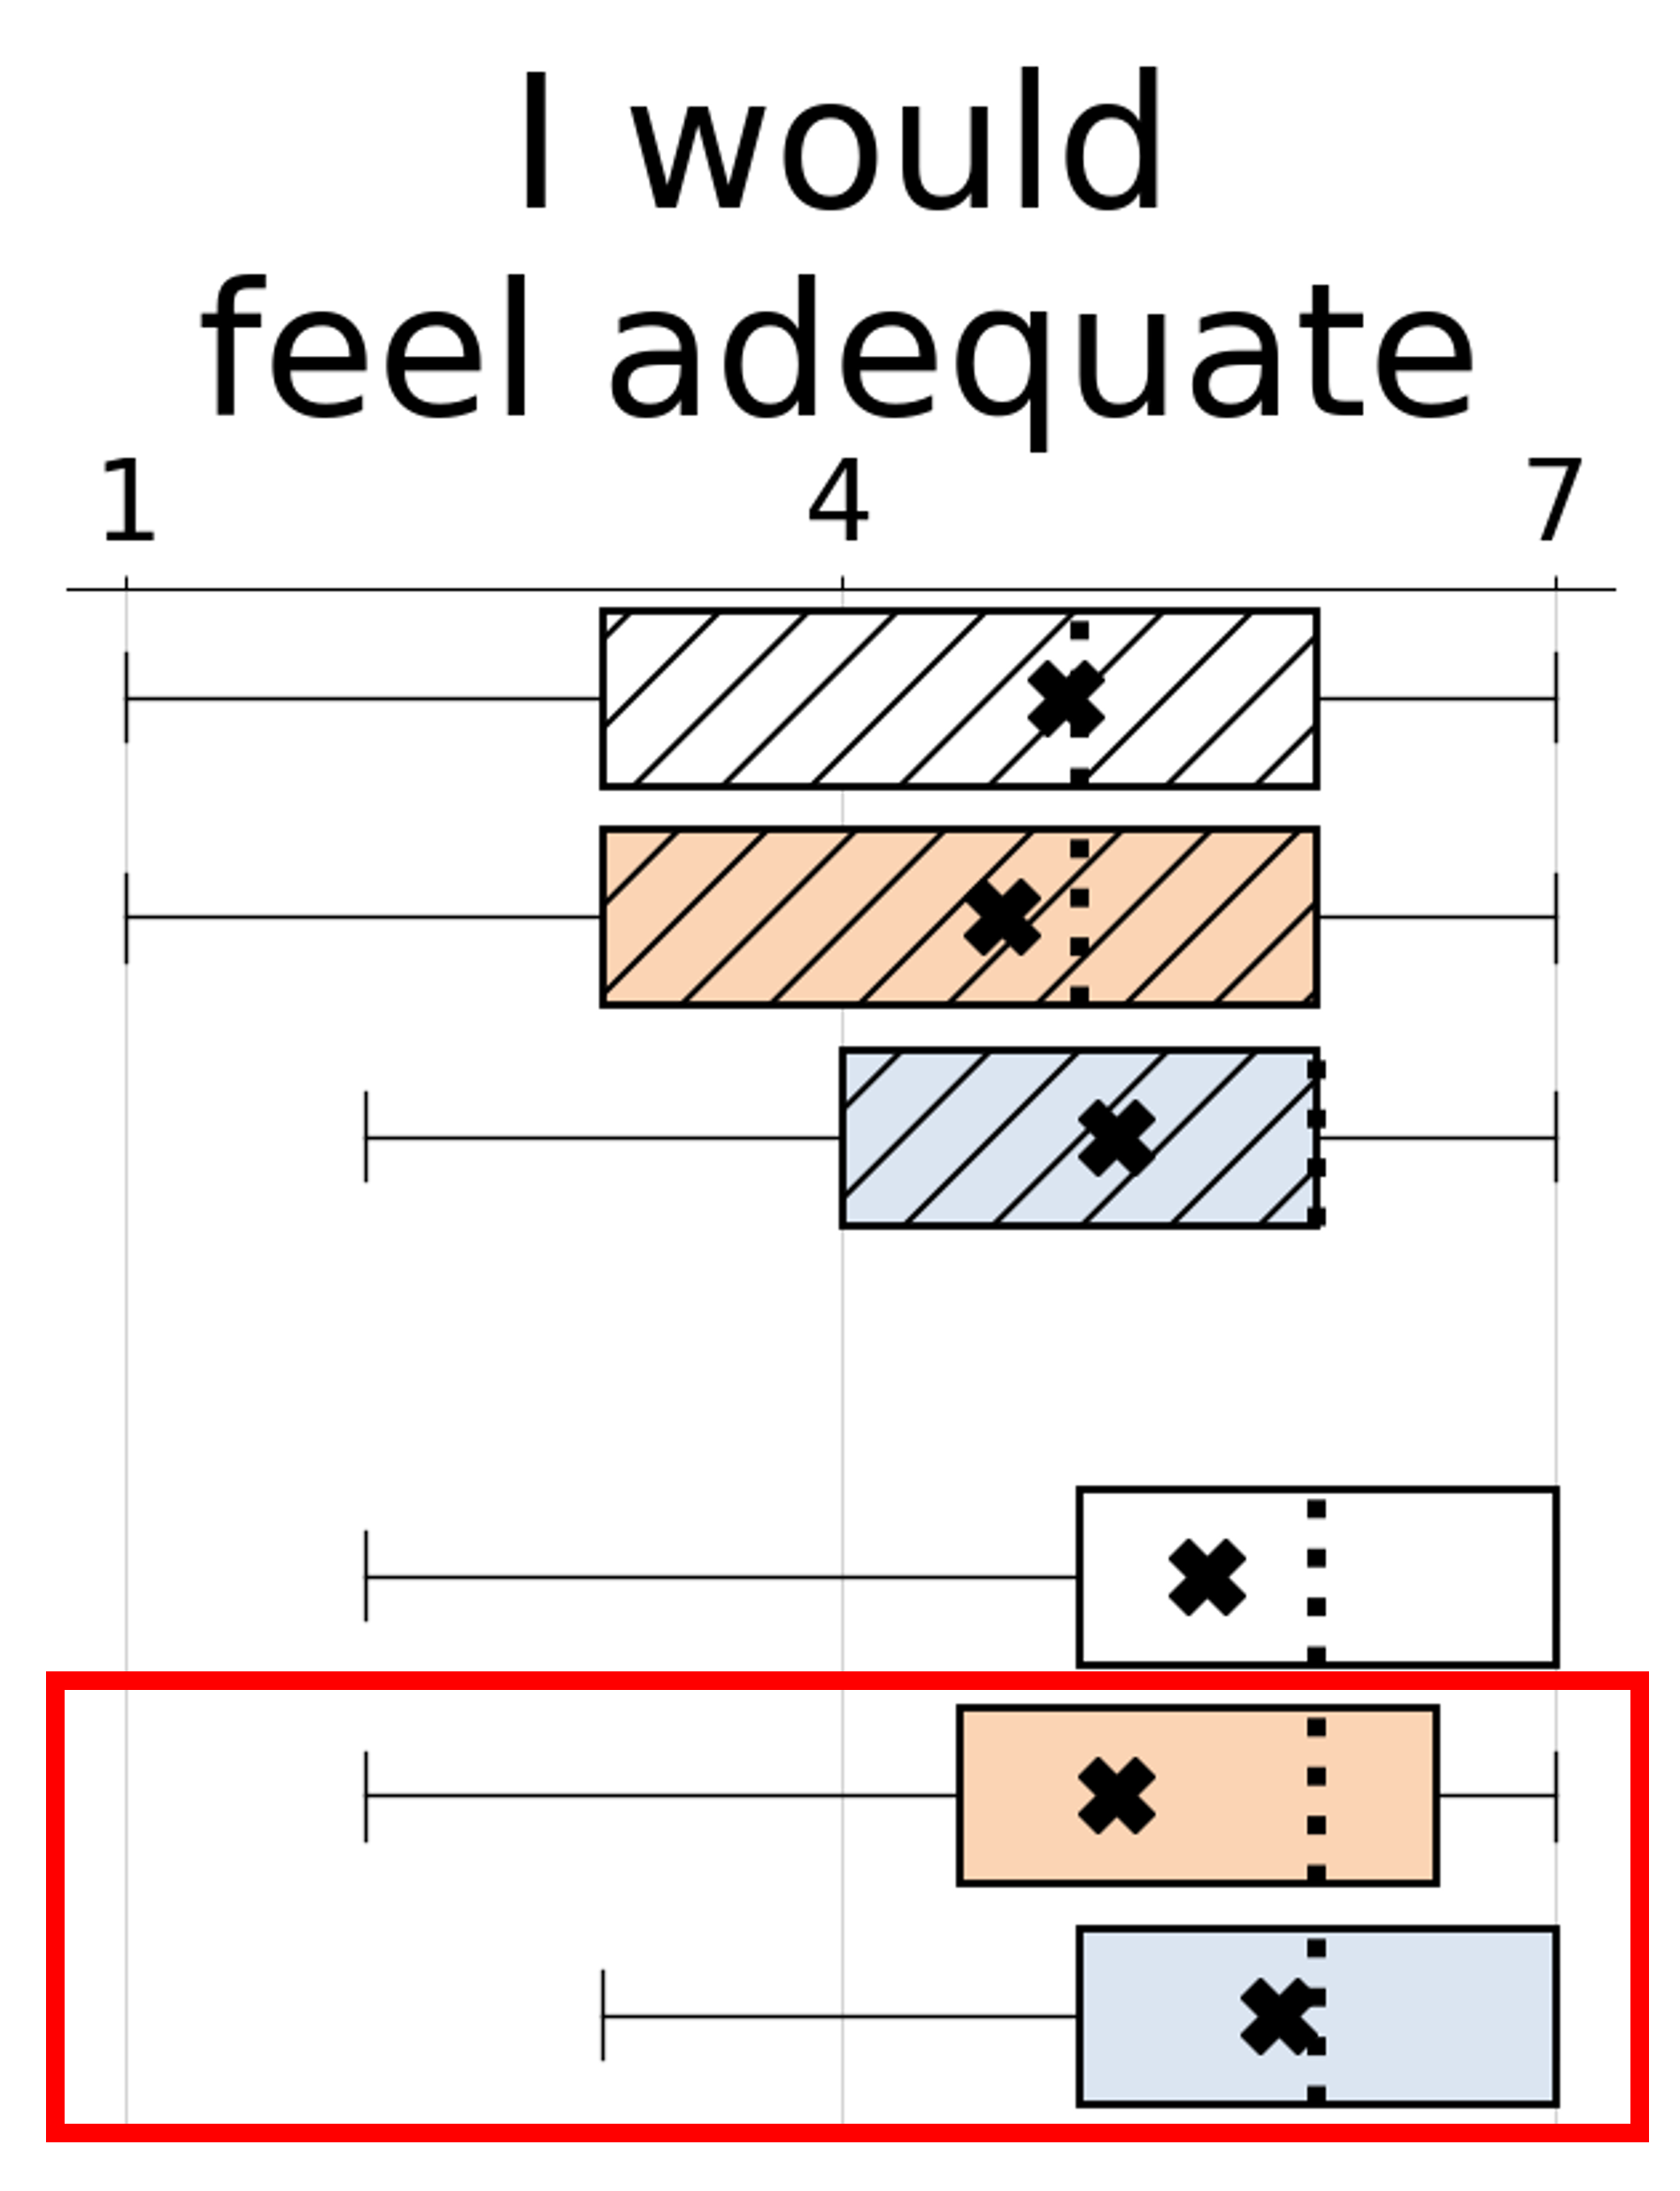}} &
    \multicolumn{2}{c|}{\includegraphics[width = 0.16\columnwidth]{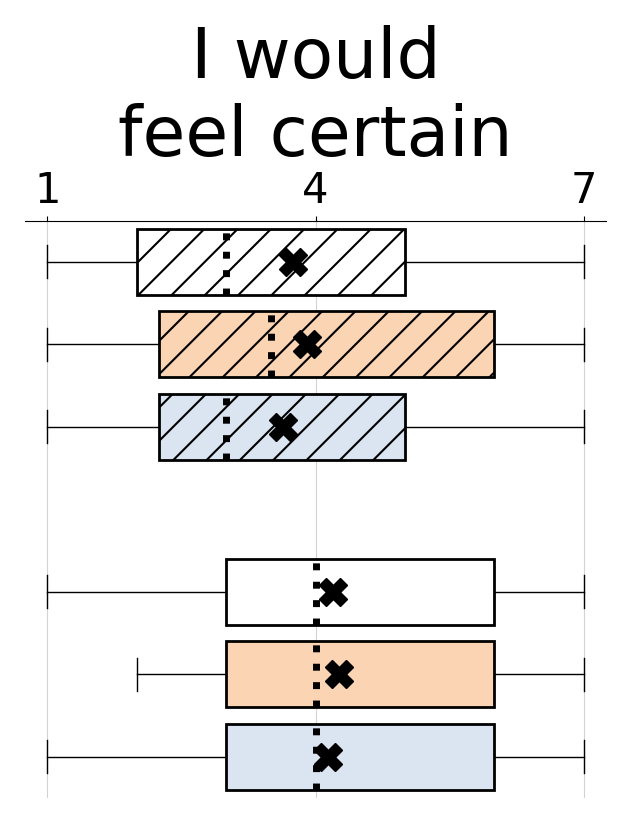}} &
    \multicolumn{2}{c}{\includegraphics[width = 0.16\columnwidth]{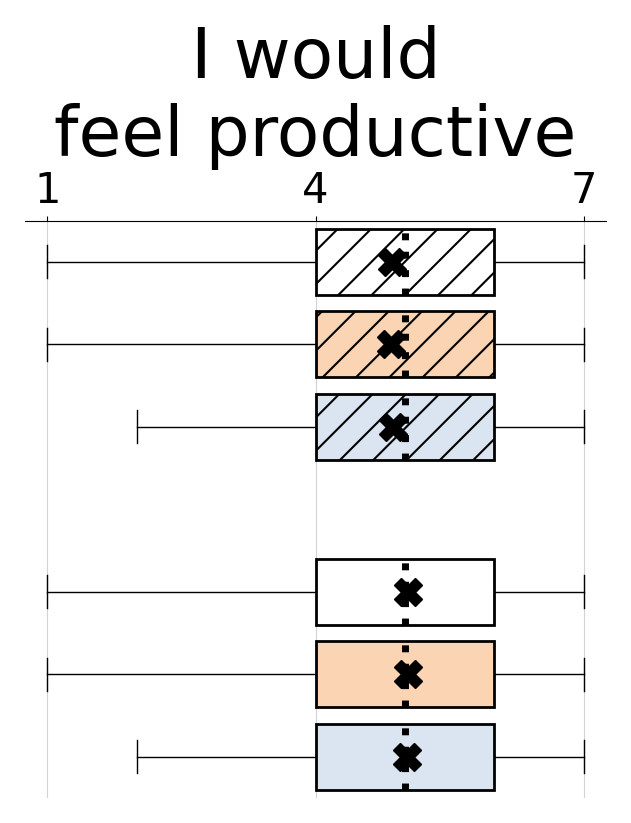}}
    \\
    \hline
    \hline
    \multicolumn{2}{c|}{\includegraphics[width = 0.16\columnwidth]{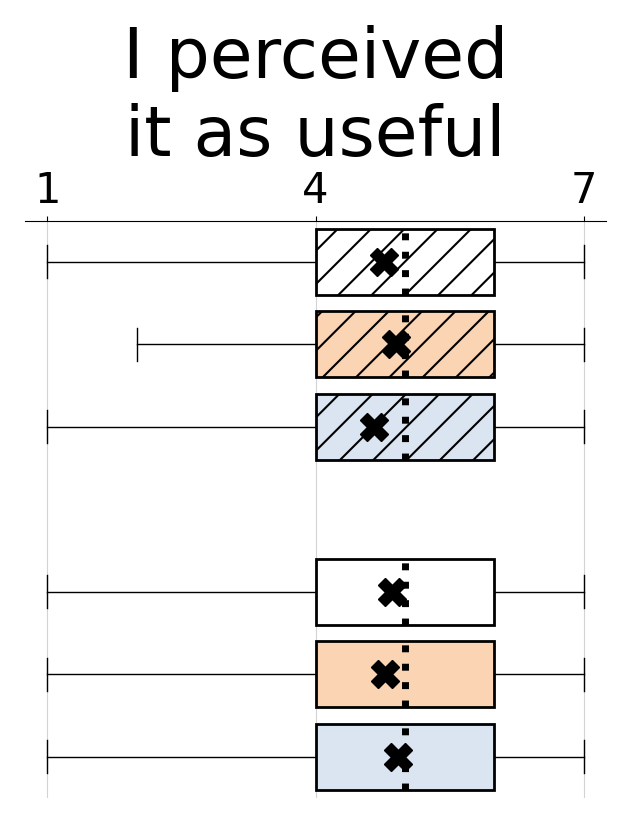}} &
    \multicolumn{2}{c|}{\includegraphics[width = 0.16\columnwidth]{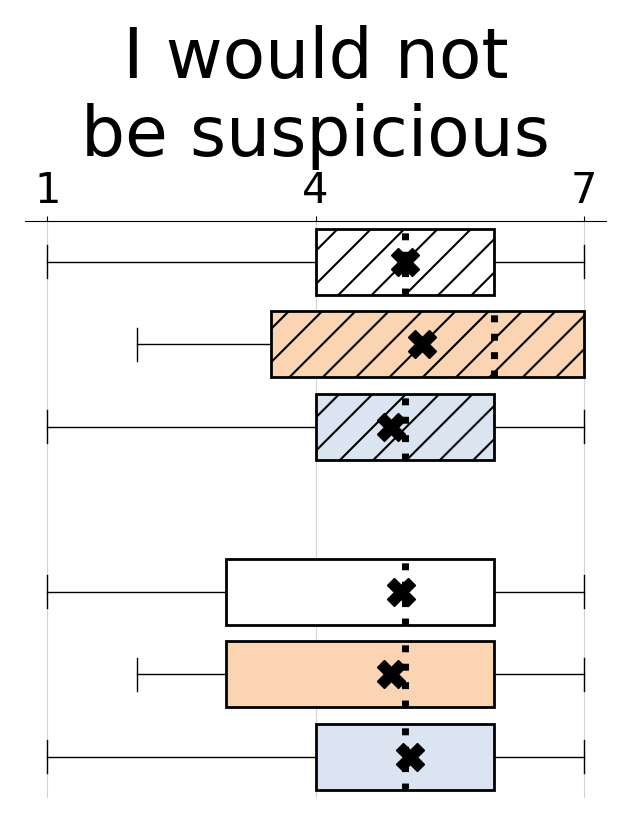}} &
    \multicolumn{2}{c|}{\includegraphics[width = 0.16\columnwidth]{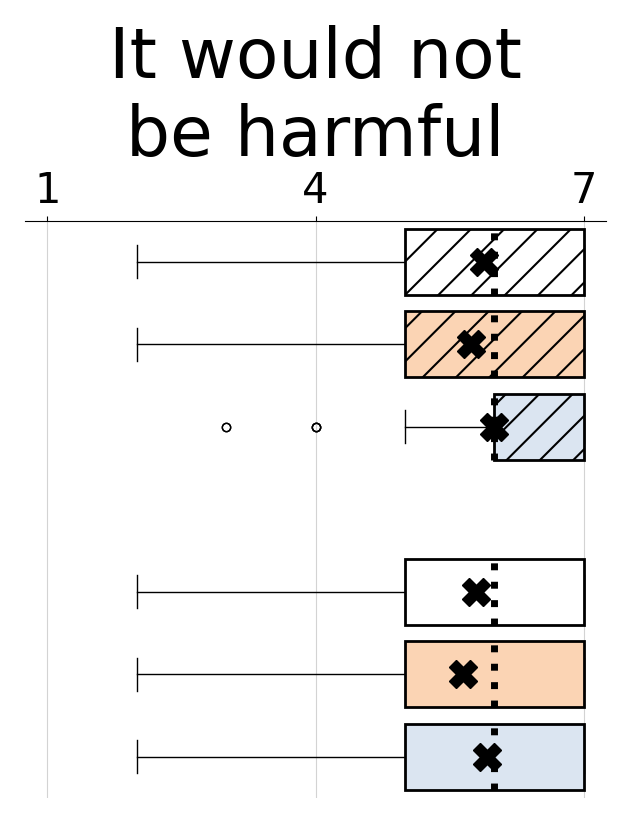}} &
    \multicolumn{2}{c|}{\includegraphics[width = 0.16\columnwidth]{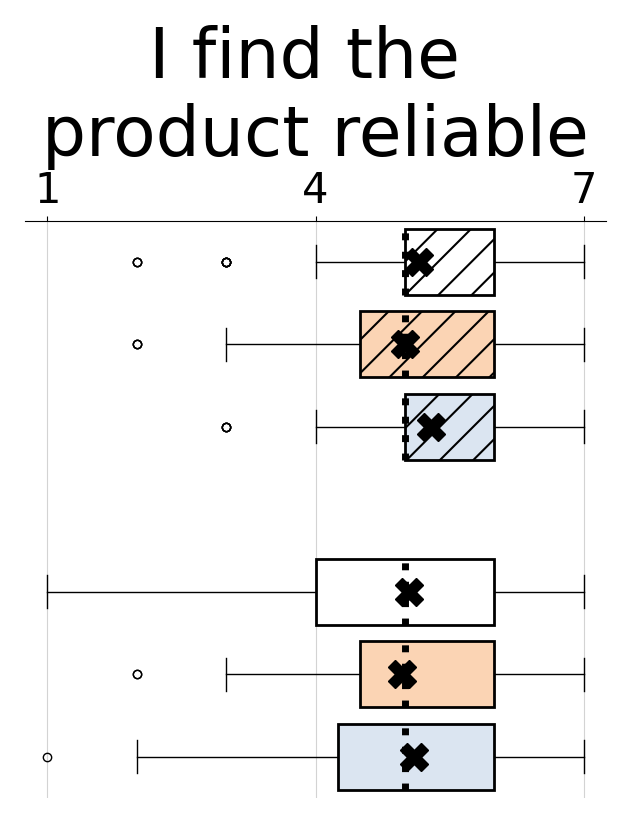}} &
    \multicolumn{2}{c}{\includegraphics[width = 0.16\columnwidth]{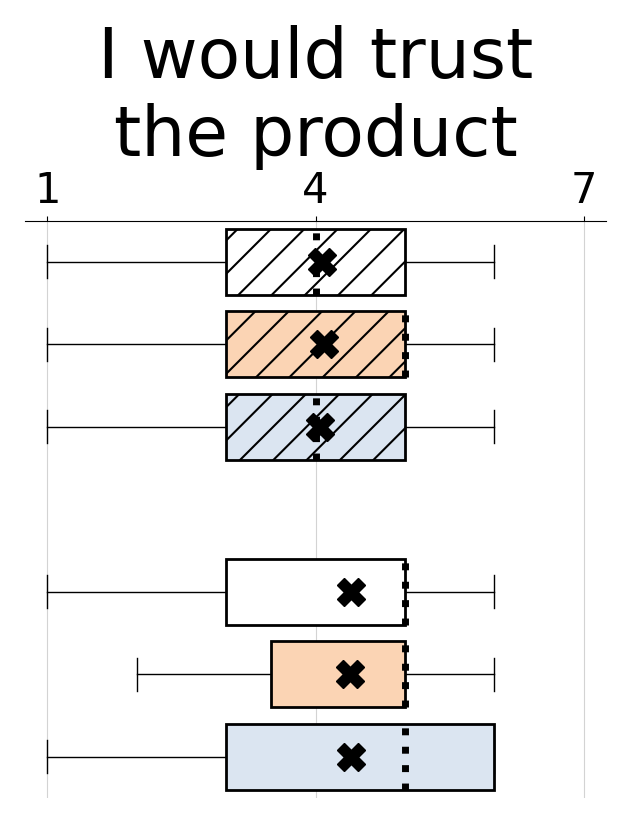}}
    \end{tabular}
    
    \caption{Guideline 5 participants' ratings for all dependent variables, disaggregated by participants' attitudes toward risk.
	%For the disaggregated data, notice how large the distances between the average rating are when the guideline is applied.
	Table~\ref{tab:G5-Risk-Stats-Appendix} below provides the statistics (where applicable).
}
    \label{fig:Risk-G5-Appendix}
\end{table}

\begin{table}[h]

%\framebox[\linewidth]{For Measuring!}
\centering
\footnotesize

    \begin{tabular}{p{0.22\columnwidth}|c|c|c|c|c|c}
    
    \rowcolor{LightGray}\multicolumn{7}{c}{\textbf{Violation AI Product}}\\
    \hline
    \textbf{Dependent}  & \textbf{Distance b/w} &  &  & & \textbf{Bonferroni} &  \\
    \textbf{variable} & \textbf{Means} &  \textbf{df} &  \textbf{t-val} &   \textbf{p-value}  & \textbf{correction} & \textbf{Cohen's \textit{d}} \\
    \hline
    
    I would feel in control & - - - & - &  - - - & - - - & - - - & - - - \\
    \hline
    
    I would feel secure & - - - & - &  - - - & - - - & - - - & - - - \\
    \hline
    
    I would feel adequate & 0.4116 & 67 &  0.9865 & .3274 & - - - & .2377 \\
    \hline
    
    I would feel certain & - - - & - &  - - - & - - - & - - - & - - - \\
    \hline
    
    I would feel productive & - - - & - &  - - - & - - - & - - - & - - -  \\
    \hline
    \hline
    
    I perceived it as useful &  - - - & - &  - - - & - - - & - - - & - - -  \\
    \hline
    
    I would not be suspicious & - - - & - &  - - - & - - - & - - - & - - -  \\
    \hline
    
    It would not be harmful & - - - & - &  - - - & - - - & - - - & - - -  \\
    \hline
    
    I find the product reliable & - - - & - &  - - - & - - - & - - - & - - -  \\
    \hline
    
    I would trust the product & - - - & - &  - - - & - - - & - - - & - - - \\
    \hline

    \rowcolor{LightGray}\multicolumn{7}{c}{\textbf{Application AI Product}}\\
    \hline
    \textbf{Dependent}  & \textbf{Distance b/w} &  &  & & \textbf{Bonferroni} &  \\
    \textbf{variable} & \textbf{Means} &  \textbf{df} &  \textbf{t-val} &   \textbf{p-value}  & \textbf{correction} & \textbf{Cohen's \textit{d}} \\
    \hline
    
    I would feel in control & 0.7152 & 66 &  1.8057 & .0755 & - - - & .4381  \\
    \hline
    
    I would feel secure & - - - & - &  - - - & - - - & - - - & - - - \\
    \hline
    
    I would feel adequate & 0.7374 & 67 & 2.0600 & \cellcolor{AbiOrangeQuote}{.0433} &  & .4965 \\
    \hline
    
    I would feel certain & - - - & - &  - - - & - - - & - - - & - - - \\
    \hline
    
    I would feel productive & - - - & - &  - - - & - - - & - - - & - - -    \\
    \hline
    \hline
    
    I perceived it as useful &  - - - & - &  - - - & - - - & - - - & - - -   \\
    \hline
    
    I would not be suspicious & - - - & - &  - - - & - - - & - - - & - - -   \\
    \hline
    
    It would not be harmful & - - - & - &  - - - & - - - & - - - & - - -  \\
    \hline
    
    I find the product reliable & - - - & - &  - - - & - - - & - - - & - - - \\
    \hline
    
    I would trust the product & - - - & - &  - - - & - - - & - - - & - - -

    \end{tabular}

    \caption{Guideline 5's t-test results %(\checkmark if Welch's t-test) 
    for risk-averse vs. risk-tolerant participants' average ratings of the independent Violation AI product (top) and Application AI product (bottom), for all 10 dependent variables.
    If dashes (- - -) are present, no statistical test was performed.
    If the number of tests exceeded 5 for each product, Bonferroni correction applied by multiplying p-values by the number of tests performed.
    }
    \label{tab:G5-Risk-Stats-Appendix}
\end{table}

%---------------------------------------------------- End Guideline 5

\clearpage

%Begin Guideline 6----------------------------------------------------

\begin{table}[]
    \centering
    \begin{tabular}{cc|cc|cc|cc|cc}
    \multicolumn{2}{c|}{\includegraphics[width = 0.16\columnwidth]{assets/05-All-BoxPlots/05-G6/Risk/G6-Feel-In-Control-RISK.png}} &
    \multicolumn{2}{c|}{\includegraphics[width = 0.16\columnwidth]{assets/05-All-BoxPlots/05-G6/Risk/G6-Feel-Secure-RISK.png}} &
    \multicolumn{2}{c|}{\includegraphics[width = 0.16\columnwidth]{assets/05-All-BoxPlots/05-G6/Risk/G6-Feel-Adequate-RISK.png}} &
    \multicolumn{2}{c|}{\includegraphics[width = 0.16\columnwidth]{assets/05-All-BoxPlots/05-G6/Risk/G6-Feel-Certain-RISK.png}} &
    \multicolumn{2}{c}{\includegraphics[width = 0.16\columnwidth]{assets/05-All-BoxPlots/05-G6/Risk/G6-Feel-Productive-RISK.png}}
    \\
    \hline
    \hline
    \multicolumn{2}{c|}{\includegraphics[width = 0.16\columnwidth]{assets/05-All-BoxPlots/05-G6/Risk/G6-Perceived-Useful-RISK.png}} &
    \multicolumn{2}{c|}{\includegraphics[width = 0.16\columnwidth]{assets/05-All-BoxPlots/05-G6/Risk/G6-Not-Suspicious-RISK.png}} &
    \multicolumn{2}{c|}{\includegraphics[width = 0.16\columnwidth]{assets/05-All-BoxPlots/05-G6/Risk/G6-Not-Harmful-RISK.png}} &
    \multicolumn{2}{c|}{\includegraphics[width = 0.16\columnwidth]{assets/05-All-BoxPlots/05-G6/Risk/G6-Product-Reliable-RISK.png}} &
    \multicolumn{2}{c}{\includegraphics[width = 0.16\columnwidth]{assets/05-All-BoxPlots/05-G6/Risk/G6-Trust-Product-RISK.png}}
    \end{tabular}
    
    \caption{Guideline 6 participants' ratings for all dependent variables, disaggregated by participants' attitudes toward risk.
	%For the disaggregated data, notice how large the distances between the average rating are when the guideline is applied.
	Table~\ref{tab:G6-Risk-Stats-Appendix} below provides the statistics (where applicable).
}
    \label{fig:Risk-G6-Appendix}
\end{table}

\begin{table}[h]

%\framebox[\linewidth]{For Measuring!}
\centering
\footnotesize

    \begin{tabular}{p{0.22\columnwidth}|c|c|c|c|c|c}
    
    \rowcolor{LightGray}\multicolumn{7}{c}{\textbf{Violation AI Product}}\\
    \hline
    \textbf{Dependent}  & \textbf{Distance b/w} &  &  & & \textbf{Bonferroni} &  \\
    \textbf{variable} & \textbf{Means} &  \textbf{df} &  \textbf{t-val} &   \textbf{p-value}  & \textbf{correction} & \textbf{Cohen's \textit{d}} \\
    \hline
    
    I would feel in control & - - - & - &  - - - & - - - & - - - & - - -  \\
    \hline
    
    I would feel secure & - - - & - &  - - - & - - - & - - - & - - - \\
    \hline
    
    I would feel adequate & 0.9683 & 62 &  1.8948 & .0626 & - - - & .4775 \\
    \hline
    
    I would feel certain & - - - & - &  - - - & - - - & - - - & - - - \\
    \hline
    
    I would feel productive & - - - & - &  - - - & - - - & - - - & - - -    \\
    \hline
    \hline
    
    I perceived it as useful &  - - - & - &  - - - & - - - & - - - & - - -   \\
    \hline
    
    I would not be suspicious & - - - & - &  - - - & - - - & - - - & - - -   \\
    \hline
    
    It would not be harmful & - - - & - &  - - - & - - - & - - - & - - -  \\
    \hline
    
    I find the product reliable & - - - & - &  - - - & - - - & - - - & - - - \\
    \hline
    
    I would trust the product & - - - & - &  - - - & - - - & - - - & - - - \\
    \hline

    \rowcolor{LightGray}\multicolumn{7}{c}{\textbf{Application AI Product}}\\
    \hline
    \textbf{Dependent}  & \textbf{Distance b/w} &  &  & & \textbf{Bonferroni} &  \\
    \textbf{variable} & \textbf{Means} &  \textbf{df} &  \textbf{t-val} &   \textbf{p-value}  & \textbf{correction} & \textbf{Cohen's \textit{d}} \\
    \hline
    
    I would feel in control & - - - & - &  - - - & - - - & - - - & - - -  \\
    \hline
    
    I would feel secure & - - - & - &  - - - & - - - & - - - & - - - \\
    \hline
    
    I would feel adequate & - - - & - &  - - - & - - - & - - - & - - - \\
    \hline
    
    I would feel certain & - - - & - &  - - - & - - - & - - - & - - - \\
    \hline
    
    I would feel productive & - - - & - &  - - - & - - - & - - - & - - -    \\
    \hline
    \hline
    
    I perceived it as useful &  - - - & - &  - - - & - - - & - - - & - - -   \\
    \hline
    
    I would not be suspicious & - - - & - &  - - - & - - - & - - - & - - -   \\
    \hline
    
    It would not be harmful & - - - & - &  - - - & - - - & - - - & - - -  \\
    \hline
    
    I find the product reliable & - - - & - &  - - - & - - - & - - - & - - - \\
    \hline
    
    I would trust the product & - - - & - &  - - - & - - - & - - - & - - -

    \end{tabular}

    \caption{Guideline 6's t-test results %(\checkmark if Welch's t-test) 
    for risk-averse vs. risk-tolerant participants' average ratings of the independent Violation AI product (top) and Application AI product (bottom), for all 10 dependent variables.
    If dashes (- - -) are present, no statistical test was performed.
    If the number of tests exceeded 5 for each product, Bonferroni correction applied by multiplying p-values by the number of tests performed.
    }
    \label{tab:G6-Risk-Stats-Appendix}
\end{table}

%---------------------------------------------------- End Guideline 6

\clearpage

%Begin Guideline 7----------------------------------------------------

\begin{table}[]
    \centering
    \begin{tabular}{cc|cc|cc|cc|cc}
    \multicolumn{2}{c|}{\includegraphics[width = 0.16\columnwidth]{assets/05-All-BoxPlots/06-G7/Risk/G7-Feel-In-Control-RISK.png}} &
    \multicolumn{2}{c|}{\includegraphics[width = 0.16\columnwidth]{assets/05-All-BoxPlots/06-G7/Risk/G7-Feel-Secure-RISK.png}} &
    \multicolumn{2}{c|}{\includegraphics[width = 0.16\columnwidth]{assets/05-All-BoxPlots/06-G7/Risk/G7-Feel-Adequate-RISK.png}} &
    \multicolumn{2}{c|}{\includegraphics[width = 0.16\columnwidth]{assets/05-All-BoxPlots/06-G7/Risk/G7-Feel-Certain-RISK.png}} &
    \multicolumn{2}{c}{\includegraphics[width = 0.16\columnwidth]{assets/05-All-BoxPlots/06-G7/Risk/G7-Feel-Productive-RISK.png}}
    \\
    \hline
    \hline
    \multicolumn{2}{c|}{\includegraphics[width = 0.16\columnwidth]{assets/05-All-BoxPlots/06-G7/Risk/G7-Perceived-Useful-RISK.png}} &
    \multicolumn{2}{c|}{\includegraphics[width = 0.16\columnwidth]{assets/05-All-BoxPlots/06-G7/Risk/G7-Not-Suspicious-RISK.png}} &
    \multicolumn{2}{c|}{\includegraphics[width = 0.16\columnwidth]{assets/05-All-BoxPlots/06-G7/Risk/G7-Not-Harmful-RISK.png}} &
    \multicolumn{2}{c|}{\includegraphics[width = 0.16\columnwidth]{assets/05-All-BoxPlots/06-G7/Risk/G7-Product-Reliable-RISK.png}} &
    \multicolumn{2}{c}{\includegraphics[width = 0.16\columnwidth]{assets/05-All-BoxPlots/06-G7/Risk/G7-Trust-Product-RISK.png}}
    \end{tabular}
    
    \caption{Guideline 7 participants' ratings for all dependent variables, disaggregated by participants' attitudes toward risk.
	%For the disaggregated data, notice how large the distances between the average rating are when the guideline is applied.
	Table~\ref{tab:G7-Risk-Stats-Appendix} below provides the statistics (where applicable).
}
    \label{fig:Risk-G7-Appendix}
\end{table}

\begin{table}[h]

%\framebox[\linewidth]{For Measuring!}
\centering
\footnotesize

    \begin{tabular}{p{0.22\columnwidth}|c|c|c|c|c|c}
    
    \rowcolor{LightGray}\multicolumn{7}{c}{\textbf{Violation AI Product}}\\
    \hline
    \textbf{Dependent}  & \textbf{Distance b/w} &  &  & & \textbf{Bonferroni} &  \\
    \textbf{variable} & \textbf{Means} &  \textbf{df} &  \textbf{t-val} &   \textbf{p-value}  & \textbf{correction} & \textbf{Cohen's \textit{d}} \\
    \hline
    
    I would feel in control & 0.9471 & 56 &  2.7112 & \cellcolor{AbiOrangeQuote}.0089 & - - - & .7158 \\
    \hline
    
    I would feel secure & - - - & - &  - - - & - - - & - - - & - - - \\
    \hline
    
    I would feel adequate & - - - & - &  - - - & - - - & - - - & - - - \\
    \hline
    
    I would feel certain & - - - & - &  - - - & - - - & - - - & - - - \\
    \hline
    
    I would feel productive & - - - & - &  - - - & - - - & - - - & - - -  \\
    \hline
    \hline
    
    I perceived it as useful &  - - - & - &  - - - & - - - & - - - & - - -  \\
    \hline
    
    I would not be suspicious & - - - & - &  - - - & - - - & - - - & - - -  \\
    \hline
    
    It would not be harmful & - - - & - &  - - - & - - - & - - - & - - -  \\
    \hline
    
    I find the product reliable & - - - & - &  - - - & - - - & - - - & - - -  \\
    \hline
    
    I would trust the product & - - - & - &  - - - & - - - & - - - & - - - \\
    \hline

    \rowcolor{LightGray}\multicolumn{7}{c}{\textbf{Application AI Product}}\\
    \hline
    \textbf{Dependent}  & \textbf{Distance b/w} &  &  & & \textbf{Bonferroni} &  \\
    \textbf{variable} & \textbf{Means} &  \textbf{df} &  \textbf{t-val} &   \textbf{p-value}  & \textbf{correction} & \textbf{Cohen's \textit{d}} \\
    \hline
    
    I would feel in control & 0.4543 & 56 &  1.3941 & .1688 & - - - & .3681  \\
    \hline
    
    I would feel secure & - - - & - &  - - - & - - - & - - - & - - - \\
    \hline
    
    I would feel adequate & - - -  & - &  - - - & - - - & - - - & - - - \\
    \hline
    
    I would feel certain & - - - & - &  - - - & - - - & - - - & - - - \\
    \hline
    
    I would feel productive & - - - & - &  - - - & - - - & - - - & - - -    \\
    \hline
    \hline
    
    I perceived it as useful &  - - - & - &  - - - & - - - & - - - & - - -   \\
    \hline
    
    I would not be suspicious & - - - & - &  - - - & - - - & - - - & - - -   \\
    \hline
    
    It would not be harmful & - - - & - &  - - - & - - - & - - - & - - -  \\
    \hline
    
    I find the product reliable & - - - & - &  - - - & - - - & - - - & - - - \\
    \hline
    
    I would trust the product & - - - & - &  - - - & - - - & - - - & - - -

    \end{tabular}

    \caption{Guideline 7's t-test results %(\checkmark if Welch's t-test) 
    for risk-averse vs. risk-tolerant participants' average ratings of the independent Violation AI product (top) and Application AI product (bottom), for all 10 dependent variables.
    If dashes (- - -) are present, no statistical test was performed.
    If the number of tests exceeded 5 for each product, Bonferroni correction applied by multiplying p-values by the number of tests performed.
    }
    \label{tab:G7-Risk-Stats-Appendix}
\end{table}

%---------------------------------------------------- End Guideline 7

\clearpage

%Begin Guideline 8----------------------------------------------------

\begin{table}[]
    \centering
    \begin{tabular}{cc|cc|cc|cc|cc}
    \multicolumn{2}{c|}{\includegraphics[width = 0.16\columnwidth]{assets/05-All-BoxPlots/07-G8/Risk/G8-Feel-In-Control-RISK.png}} &
    \multicolumn{2}{c|}{\includegraphics[width = 0.16\columnwidth]{assets/05-All-BoxPlots/07-G8/Risk/G8-Feel-Secure-RISK.png}} &
    \multicolumn{2}{c|}{\includegraphics[width = 0.16\columnwidth]{assets/05-All-BoxPlots/07-G8/Risk/G8-Feel-Adequate-RISK.png}} &
    \multicolumn{2}{c|}{\includegraphics[width = 0.16\columnwidth]{assets/05-All-BoxPlots/07-G8/Risk/G8-Feel-Certain-RISK.png}} &
    \multicolumn{2}{c}{\includegraphics[width = 0.16\columnwidth]{assets/05-All-BoxPlots/07-G8/Risk/G8-Feel-Productive-RISK.png}}
    \\
    \hline
    \hline
    \multicolumn{2}{c|}{\includegraphics[width = 0.16\columnwidth]{assets/05-All-BoxPlots/07-G8/Risk/G8-Perceived-Useful-RISK.png}} &
    \multicolumn{2}{c|}{\includegraphics[width = 0.16\columnwidth]{assets/05-All-BoxPlots/07-G8/Risk/G8-Not-Suspicious-RISK.png}} &
    \multicolumn{2}{c|}{\includegraphics[width = 0.16\columnwidth]{assets/05-All-BoxPlots/07-G8/Risk/G8-Not-Harmful-RISK.png}} &
    \multicolumn{2}{c|}{\includegraphics[width = 0.16\columnwidth]{assets/05-All-BoxPlots/07-G8/Risk/G8-Product-Reliable-RISK.png}} &
    \multicolumn{2}{c}{\includegraphics[width = 0.16\columnwidth]{assets/05-All-BoxPlots/07-G8/Risk/G8-Trust-Product-RISK.png}}
    \end{tabular}
    
    \caption{Guideline 8 participants' ratings for all dependent variables, disaggregated by participants' attitudes toward risk.
	%For the disaggregated data, notice how large the distances between the average rating are when the guideline is applied.
	Table~\ref{tab:G8-Risk-Stats-Appendix} below provides the statistics (where applicable).
}
    \label{fig:Risk-G8-Appendix}
\end{table}

\begin{table}[h]

%\framebox[\linewidth]{For Measuring!}
\centering
\footnotesize

    \begin{tabular}{p{0.22\columnwidth}|c|c|c|c|c|c}
    
    \rowcolor{LightGray}\multicolumn{7}{c}{\textbf{Violation AI Product}}\\
    \hline
    \textbf{Dependent}  & \textbf{Distance b/w} &  &  & & \textbf{Bonferroni} &  \\
    \textbf{variable} & \textbf{Means} &  \textbf{df} &  \textbf{t-val} &   \textbf{p-value}  & \textbf{correction} & \textbf{Cohen's \textit{d}} \\
    \hline
    
    I would feel in control & - - - & - &  - - - & - - - & - - - & - - - \\
    \hline
    
    I would feel secure & 0.5047 & 57 &  1.1824 & .2420 & - - - & .3101 \\
    \hline
    
    I would feel adequate & - - - & - &  - - - & - - - & - - - & - - - \\
    \hline
    
    I would feel certain & 0.7000 & 59 &  1.5830 & .1188 & - - - & .4099  \\
    \hline
    
    I would feel productive & - - - & - &  - - - & - - - & - - - & - - -  \\
    \hline
    \hline
    
    I perceived it as useful &  - - - & - &  - - - & - - - & - - - & - - -  \\
    \hline
    
    I would not be suspicious & 0.9527 &  56 &  2.7112 & \cellcolor{AbiOrangeQuote}.0089 & - - - & .7158 \\
    \hline
    
    It would not be harmful & - - - & - &  - - - & - - - & - - - & - - -  \\
    \hline
    
    I find the product reliable & - - - & - &  - - - & - - - & - - - & - - -  \\
    \hline
    
    I would trust the product & - - - & - &  - - - & - - - & - - - & - - - \\
    \hline

    \rowcolor{LightGray}\multicolumn{7}{c}{\textbf{Application AI Product}}\\
    \hline
    \textbf{Dependent}  & \textbf{Distance b/w} &  &  & & \textbf{Bonferroni} &  \\
    \textbf{variable} & \textbf{Means} &  \textbf{df} &  \textbf{t-val} &   \textbf{p-value}  & \textbf{correction} & \textbf{Cohen's \textit{d}} \\
    \hline
    
    I would feel in control & - - -& - &  - - - & - - - & - - - & - - -  \\
    \hline
    
    I would feel secure & - - - & - &  - - - & - - - & - - - & - - - \\
    \hline
    
    I would feel adequate & - - -  & - &  - - - & - - - & - - - & - - - \\
    \hline
    
    I would feel certain & 0.7429 & 58 &  1.9537 & .0556 & - - - & .5116 \\
    \hline
    
    I would feel productive & - - - & - &  - - - & - - - & - - - & - - -    \\
    \hline
    \hline
    
    I perceived it as useful &  - - - & - &  - - - & - - - & - - - & - - -   \\
    \hline
    
    I would not be suspicious & 0.5429 & 59 &  1.2474 & .2172 & - - - & .3230   \\
    \hline
    
    It would not be harmful & - - - & - &  - - - & - - - & - - - & - - -  \\
    \hline
    
    I find the product reliable & - - - & - &  - - - & - - - & - - - & - - - \\
    \hline
    
    I would trust the product & - - - & - &  - - - & - - - & - - - & - - -

    \end{tabular}

    \caption{Guideline 8's t-test results %(\checkmark if Welch's t-test) 
    for risk-averse vs. risk-tolerant participants' average ratings of the independent Violation AI product (top) and Application AI product (bottom), for all 10 dependent variables.
    If dashes (- - -) are present, no statistical test was performed.
    If the number of tests exceeded 5 for each product, Bonferroni correction applied by multiplying p-values by the number of tests performed.
    }
    \label{tab:G8-Risk-Stats-Appendix}
\end{table}
\clearpage
%---------------------------------------------------- End Guideline 8

%Begin Guideline 9----------------------------------------------------

\begin{table}[]
    \centering
    \begin{tabular}{cc|cc|cc|cc|cc}
    \multicolumn{2}{c|}{\includegraphics[width = 0.16\columnwidth]{assets/05-All-BoxPlots/08-G9/Risk/G9-Feel-In-Control-RISK.png}} &
    \multicolumn{2}{c|}{\includegraphics[width = 0.16\columnwidth]{assets/05-All-BoxPlots/08-G9/Risk/G9-Feel-Secure-RISK.png}} &
    \multicolumn{2}{c|}{\includegraphics[width = 0.16\columnwidth]{assets/05-All-BoxPlots/08-G9/Risk/G9-Feel-Adequate-RISK.png}} &
    \multicolumn{2}{c|}{\includegraphics[width = 0.16\columnwidth]{assets/05-All-BoxPlots/08-G9/Risk/G9-Feel-Certain-RISK.png}} &
    \multicolumn{2}{c}{\includegraphics[width = 0.16\columnwidth]{assets/05-All-BoxPlots/08-G9/Risk/G9-Feel-Productive-RISK.png}}
    \\
    \hline
    \hline
    \multicolumn{2}{c|}{\includegraphics[width = 0.16\columnwidth]{assets/05-All-BoxPlots/08-G9/Risk/G9-Perceived-Useful-RISK.png}} &
    \multicolumn{2}{c|}{\includegraphics[width = 0.16\columnwidth]{assets/05-All-BoxPlots/08-G9/Risk/G9-Not-Suspicious-RISK.png}} &
    \multicolumn{2}{c|}{\includegraphics[width = 0.16\columnwidth]{assets/05-All-BoxPlots/08-G9/Risk/G9-Not-Harmful-RISK.png}} &
    \multicolumn{2}{c|}{\includegraphics[width = 0.16\columnwidth]{assets/05-All-BoxPlots/08-G9/Risk/G9-Product-Reliable-RISK.png}} &
    \multicolumn{2}{c}{\includegraphics[width = 0.16\columnwidth]{assets/05-All-BoxPlots/08-G9/Risk/G9-Trust-Product-RISK.png}}
    \end{tabular}
    
    \caption{Guideline 9 participants' ratings for all dependent variables, disaggregated by participants' attitudes toward risk.
	%For the disaggregated data, notice how large the distances between the average rating are when the guideline is applied.
	Table~\ref{tab:G9-Risk-Stats-Appendix} below provides the statistics (where applicable).
}
    \label{fig:Risk-G9-Appendix}
\end{table}

\begin{table}[h]

%\framebox[\linewidth]{For Measuring!}
\centering
\footnotesize

    \begin{tabular}{p{0.22\columnwidth}|c|c|c|c|c|c}
    
    \rowcolor{LightGray}\multicolumn{7}{c}{\textbf{Violation AI Product}}\\
    \hline
    \textbf{Dependent}  & \textbf{Distance b/w} &  &  & & \textbf{Bonferroni} &  \\
    \textbf{variable} & \textbf{Means} &  \textbf{df} &  \textbf{t-val} &   \textbf{p-value}  & \textbf{correction} & \textbf{Cohen's \textit{d}} \\
    \hline
    
    I would feel in control & - - - & - &  - - - & - - - & - - - & - - - \\
    \hline
    
    I would feel secure & - - - & - &  - - - & - - - & - - - & - - - \\
    \hline
    
    I would feel adequate & - - - & - &  - - - & - - - & - - - & - - - \\
    \hline
    
    I would feel certain & - - - & - &  - - - & - - - & - - - & - - - \\
    \hline
    
    I would feel productive & - - - & - &  - - - & - - - & - - - & - - -  \\
    \hline
    \hline
    
    I perceived it as useful &  - - - & - &  - - - & - - - & - - - & - - -  \\
    \hline
    
    I would not be suspicious & - - - & - &  - - - & - - - & - - - & - - - \\
    \hline
    
    It would not be harmful & - - - & - &  - - - & - - - & - - - & - - -  \\
    \hline
    
    I find the product reliable & - - - & - &  - - - & - - - & - - - & - - -  \\
    \hline
    
    I would trust the product & - - - & - &  - - - & - - - & - - - & - - - \\
    \hline

    \rowcolor{LightGray}\multicolumn{7}{c}{\textbf{Application AI Product}}\\
    \hline
    \textbf{Dependent}  & \textbf{Distance b/w} &  &  & & \textbf{Bonferroni} &  \\
    \textbf{variable} & \textbf{Means} &  \textbf{df} &  \textbf{t-val} &   \textbf{p-value}  & \textbf{correction} & \textbf{Cohen's \textit{d}} \\
    \hline
    
    I would feel in control & - - - & - &  - - - & - - - & - - - & - - -  \\
    \hline
    
    I would feel secure & - - - & - &  - - - & - - - & - - - & - - - \\
    \hline
    
    I would feel adequate & - - -  & - &  - - - & - - - & - - - & - - - \\
    \hline
    
    I would feel certain & - - - & - &  - - - & - - - & - - - & - - - \\
    \hline
    
    I would feel productive & 0.6875 & 56 &  2.1404 & \cellcolor{AbiOrangeQuote}.0367 & - - - & .5651    \\
    \hline
    \hline
    
    I perceived it as useful &  0.6755 & 56 &  2.2058 & \cellcolor{AbiOrangeQuote}.0315 & - - - & .5824   \\
    \hline
    
    I would not be suspicious & - - - & - &  - - - & - - - & - - - & - - -   \\
    \hline
    
    It would not be harmful & - - - & - &  - - - & - - - & - - - & - - -  \\
    \hline
    
    I find the product reliable & - - - & - &  - - - & - - - & - - - & - - - \\
    \hline
    
    I would trust the product & - - - & - &  - - - & - - - & - - - & - - -

    \end{tabular}

    \caption{Guideline 9's t-test results %(\checkmark if Welch's t-test) 
    for risk-averse vs. risk-tolerant participants' average ratings of the independent Violation AI product (top) and Application AI product (bottom), for all 10 dependent variables.
    If dashes (- - -) are present, no statistical test was performed.
    If the number of tests exceeded 5 for each product, Bonferroni correction applied by multiplying p-values by the number of tests performed.
    }
    \label{tab:G9-Risk-Stats-Appendix}
\end{table}
\clearpage
%---------------------------------------------------- End Guideline 9

%Begin Guideline 10----------------------------------------------------

\begin{table}[]
    \centering
    \begin{tabular}{cc|cc|cc|cc|cc}
    \multicolumn{2}{c|}{\includegraphics[width = 0.16\columnwidth]{assets/05-All-BoxPlots/09-G10/Risk/G10-Feel-In-Control-RISK.png}} &
    \multicolumn{2}{c|}{\includegraphics[width = 0.16\columnwidth]{assets/05-All-BoxPlots/09-G10/Risk/G10-Feel-Secure-RISK.png}} &
    \multicolumn{2}{c|}{\includegraphics[width = 0.16\columnwidth]{assets/05-All-BoxPlots/09-G10/Risk/G10-Feel-Adequate-RISK.png}} &
    \multicolumn{2}{c|}{\includegraphics[width = 0.16\columnwidth]{assets/05-All-BoxPlots/09-G10/Risk/G10-Feel-Certain-RISK.png}} &
    \multicolumn{2}{c}{\includegraphics[width = 0.16\columnwidth]{assets/05-All-BoxPlots/09-G10/Risk/G10-Feel-Productive-RISK.png}}
    \\
    \hline
    \hline
    \multicolumn{2}{c|}{\includegraphics[width = 0.16\columnwidth]{assets/05-All-BoxPlots/09-G10/Risk/G10-Perceived-Useful-RISK.png}} &
    \multicolumn{2}{c|}{\includegraphics[width = 0.16\columnwidth]{assets/05-All-BoxPlots/09-G10/Risk/G10-Not-Suspicious-RISK.png}} &
    \multicolumn{2}{c|}{\includegraphics[width = 0.16\columnwidth]{assets/05-All-BoxPlots/09-G10/Risk/G10-Not-Harmful-RISK.png}} &
    \multicolumn{2}{c|}{\includegraphics[width = 0.16\columnwidth]{assets/05-All-BoxPlots/09-G10/Risk/G10-Product-Reliable-RISK.png}} &
    \multicolumn{2}{c}{\includegraphics[width = 0.16\columnwidth]{assets/05-All-BoxPlots/09-G10/Risk/G10-Trust-Product-RISK.png}}
    \end{tabular}
    
    \caption{Guideline 10 participants' ratings for all dependent variables, disaggregated by participants' attitudes toward risk.
	%For the disaggregated data, notice how large the distances between the average rating are when the guideline is applied.
	Table~\ref{tab:G10-Risk-Stats-Appendix} below provides the statistics (where applicable).
}
    \label{fig:Risk-G10-Appendix}
\end{table}

\begin{table}[h]

%\framebox[\linewidth]{For Measuring!}
\centering
\footnotesize

    \begin{tabular}{p{0.22\columnwidth}|c|c|c|c|c|c}
    
    \rowcolor{LightGray}\multicolumn{7}{c}{\textbf{Violation AI Product}}\\
    \hline
    \textbf{Dependent}  & \textbf{Distance b/w} &  &  & & \textbf{Bonferroni} &  \\
    \textbf{variable} & \textbf{Means} &  \textbf{df} &  \textbf{t-val} &   \textbf{p-value}  & \textbf{correction} & \textbf{Cohen's \textit{d}} \\
    \hline
    
    I would feel in control & - - - & - &  - - - & - - - & - - - & - - - \\
    \hline
    
    I would feel secure & - - - & - &  - - - & - - - & - - - & - - - \\
    \hline
    
    I would feel adequate & - - - & - &  - - - & - - - & - - - & - - - \\
    \hline
    
    I would feel certain & - - - & - &  - - - & - - - & - - - & - - - \\
    \hline
    
    I would feel productive & - - - & - &  - - - & - - - & - - - & - - -  \\
    \hline
    \hline
    
    I perceived it as useful &  - - - & - &  - - - & - - - & - - - & - - -  \\
    \hline
    
    I would not be suspicious & - - - & - &  - - - & - - - & - - - & - - - \\
    \hline
    
    It would not be harmful & - - - & - &  - - - & - - - & - - - & - - -  \\
    \hline
    
    I find the product reliable & - - - & - &  - - - & - - - & - - - & - - -  \\
    \hline
    
    I would trust the product & - - - & - &  - - - & - - - & - - - & - - - \\
    \hline

    \rowcolor{LightGray}\multicolumn{7}{c}{\textbf{Application AI Product}}\\
    \hline
    \textbf{Dependent}  & \textbf{Distance b/w} &  &  & & \textbf{Bonferroni} &  \\
    \textbf{variable} & \textbf{Means} &  \textbf{df} &  \textbf{t-val} &   \textbf{p-value}  & \textbf{correction} & \textbf{Cohen's \textit{d}} \\
    \hline
    
    I would feel in control & - - - & - &  - - - & - - - & - - - & - - -  \\
    \hline
    
    I would feel secure & - - - & - &  - - - & - - - & - - - & - - - \\
    \hline
    
    I would feel adequate & - - -  & - &  - - - & - - - & - - - & - - - \\
    \hline
    
    I would feel certain & - - - & - &  - - - & - - - & - - - & - - - \\
    \hline
    
    I would feel productive & - - - & - &  - - - & - - - & - - - & - - -   \\
    \hline
    \hline
    
    I perceived it as useful &  0.7667 & 62 &  2.1542 & \cellcolor{TimBlueQuote}.0351 & - - - & .5392   \\
    \hline
    
    I would not be suspicious & - - - & - &  - - - & - - - & - - - & - - -   \\
    \hline
    
    It would not be harmful & - - - & - &  - - - & - - - & - - - & - - -  \\
    \hline
    
    I find the product reliable & 0.8032 & 61 &  2.4183 & \cellcolor{TimBlueQuote}.0186 & - - - & .6113 \\
    \hline
    
    I would trust the product & - - - & - &  - - - & - - - & - - - & - - -

    \end{tabular}

    \caption{Guideline 10's t-test results %(\checkmark if Welch's t-test) 
    for risk-averse vs. risk-tolerant participants' average ratings of the independent Violation AI product (top) and Application AI product (bottom), for all 10 dependent variables.
    If dashes (- - -) are present, no statistical test was performed.
    If the number of tests exceeded 5 for each product, Bonferroni correction applied by multiplying p-values by the number of tests performed.
    }
    \label{tab:G10-Risk-Stats-Appendix}
\end{table}
\clearpage
%---------------------------------------------------- End Guideline 10

%Begin Guideline 11----------------------------------------------------

\begin{table}[]
    \centering
    \begin{tabular}{cc|cc|cc|cc|cc}
    \multicolumn{2}{c|}{\includegraphics[width = 0.16\columnwidth]{assets/05-All-BoxPlots/10-G11/Risk/G11-Feel-In-Control-RISK.png}} &
    \multicolumn{2}{c|}{\includegraphics[width = 0.16\columnwidth]{assets/05-All-BoxPlots/10-G11/Risk/G11-Feel-Secure-RISK.png}} &
    \multicolumn{2}{c|}{\includegraphics[width = 0.16\columnwidth]{assets/05-All-BoxPlots/10-G11/Risk/G11-Feel-Adequate-RISK.png}} &
    \multicolumn{2}{c|}{\includegraphics[width = 0.16\columnwidth]{assets/05-All-BoxPlots/10-G11/Risk/G11-Feel-Certain-RISK.png}} &
    \multicolumn{2}{c}{\includegraphics[width = 0.16\columnwidth]{assets/05-All-BoxPlots/10-G11/Risk/G11-Feel-Productive-RISK.png}}
    \\
    \hline
    \hline
    \multicolumn{2}{c|}{\includegraphics[width = 0.16\columnwidth]{assets/05-All-BoxPlots/10-G11/Risk/G11-Perceived-Useful-RISK.png}} &
    \multicolumn{2}{c|}{\includegraphics[width = 0.16\columnwidth]{assets/05-All-BoxPlots/10-G11/Risk/G11-Not-Suspicious-RISK.png}} &
    \multicolumn{2}{c|}{\includegraphics[width = 0.16\columnwidth]{assets/05-All-BoxPlots/10-G11/Risk/G11-Not-Harmful-RISK.png}} &
    \multicolumn{2}{c|}{\includegraphics[width = 0.16\columnwidth]{assets/05-All-BoxPlots/10-G11/Risk/G11-Product-Reliable-RISK.png}} &
    \multicolumn{2}{c}{\includegraphics[width = 0.16\columnwidth]{assets/05-All-BoxPlots/10-G11/Risk/G11-Trust-Product-RISK.png}}
    \end{tabular}
    
    \caption{Guideline 11 participants' ratings for all dependent variables, disaggregated by participants' attitudes toward risk.
	%For the disaggregated data, notice how large the distances between the average rating are when the guideline is applied.
	Table~\ref{tab:G11-Risk-Stats-Appendix} below provides the statistics (where applicable).
}
    \label{fig:Risk-G11-Appendix}
\end{table}

\begin{table}[h]

%\framebox[\linewidth]{For Measuring!}
\centering
\footnotesize

    \begin{tabular}{p{0.22\columnwidth}|c|c|c|c|c|c}
    
    \rowcolor{LightGray}\multicolumn{7}{c}{\textbf{Violation AI Product}}\\
    \hline
    \textbf{Dependent}  & \textbf{Distance b/w} &  &  & & \textbf{Bonferroni} &  \\
    \textbf{variable} & \textbf{Means} &  \textbf{df} &  \textbf{t-val} &   \textbf{p-value}  & \textbf{correction} & \textbf{Cohen's \textit{d}} \\
    \hline
    
    I would feel in control & 0.8014 & 61 &  2.1352 & \cellcolor{AbiOrangeQuote}.0368 & - - - & .5381 \\
    \hline
    
    I would feel secure & - - - & - &  - - - & - - - & - - - & - - - \\
    \hline
    
    I would feel adequate & - - - & - &  - - - & - - - & - - - & - - - \\
    \hline
    
    I would feel certain & 0.4647 & 61 &  1.2036 & .2334 & - - - & .3033 \\
    \hline
    
    I would feel productive & - - - & - &  - - - & - - - & - - - & - - -  \\
    \hline
    \hline
    
    I perceived it as useful &  - - - & - &  - - - & - - - & - - - & - - -  \\
    \hline
    
    I would not be suspicious & - - - & - &  - - - & - - - & - - - & - - - \\
    \hline
    
    It would not be harmful & - - - & - &  - - - & - - - & - - - & - - -  \\
    \hline
    
    I find the product reliable & - - - & - &  - - - & - - - & - - - & - - -  \\
    \hline
    
    I would trust the product & - - - & - &  - - - & - - - & - - - & - - - \\
    \hline

    \rowcolor{LightGray}\multicolumn{7}{c}{\textbf{Application AI Product}}\\
    \hline
    \textbf{Dependent}  & \textbf{Distance b/w} &  &  & & \textbf{Bonferroni} &  \\
    \textbf{variable} & \textbf{Means} &  \textbf{df} &  \textbf{t-val} &   \textbf{p-value}  & \textbf{correction} & \textbf{Cohen's \textit{d}} \\
    \hline
    
    I would feel in control & 0.6724 & 61   &  1.8004  & .0767 & - - - & .4537  \\
    \hline
    
    I would feel secure & 0.4839 & 61 &  1.3373 & .1861 & - - - & .337 \\
    \hline
    
    I would feel adequate & 0.7500  & 61 &  2.1964 & \cellcolor{AbiOrangeQuote}.0319 & - - - & .5535 \\
    \hline
    
    I would feel certain & - - - & - &  - - - & - - - & - - - & - - - \\
    \hline
    
    I would feel productive & - - - & - &  - - - & - - - & - - - & - - -   \\
    \hline
    \hline
    
    I perceived it as useful &  - - - & - &  - - - & - - - & - - - & - - -   \\
    \hline
    
    I would not be suspicious & - - - & - &  - - - & - - - & - - - & - - -   \\
    \hline
    
    It would not be harmful & - - - & - &  - - - & - - - & - - - & - - -  \\
    \hline
    
    I find the product reliable & - - - & - &  - - - & - - - & - - - & - - - \\
    \hline
    
    I would trust the product & 0.5192 & 61 &  1.5336 & .1303 & - - - & .3865

    \end{tabular}

    \caption{Guideline 11's t-test results %(\checkmark if Welch's t-test) 
    for risk-averse vs. risk-tolerant participants' average ratings of the independent Violation AI product (top) and Application AI product (bottom), for all 10 dependent variables.
    If dashes (- - -) are present, no statistical test was performed.
    If the number of tests exceeded 5 for each product, Bonferroni correction applied by multiplying p-values by the number of tests performed.
    }
    \label{tab:G11-Risk-Stats-Appendix}
\end{table}
\clearpage
%---------------------------------------------------- End Guideline 11

%Begin Guideline 12----------------------------------------------------

\begin{table}[]
    \centering
    \begin{tabular}{cc|cc|cc|cc|cc}
    \multicolumn{2}{c|}{\includegraphics[width = 0.16\columnwidth]{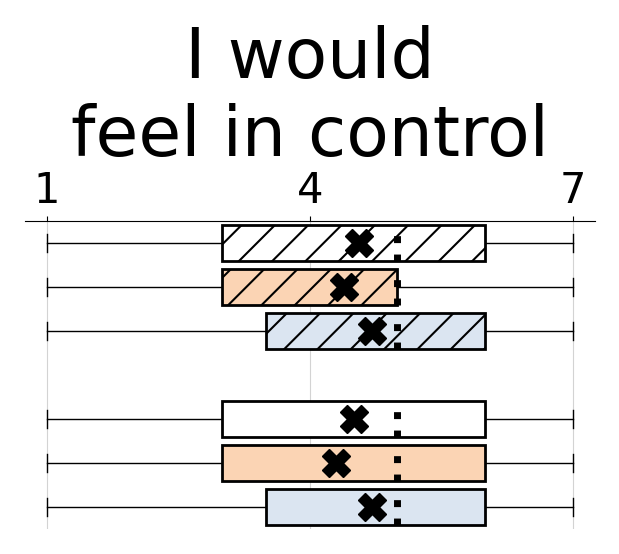}} &
    \multicolumn{2}{c|}{\includegraphics[width = 0.16\columnwidth]{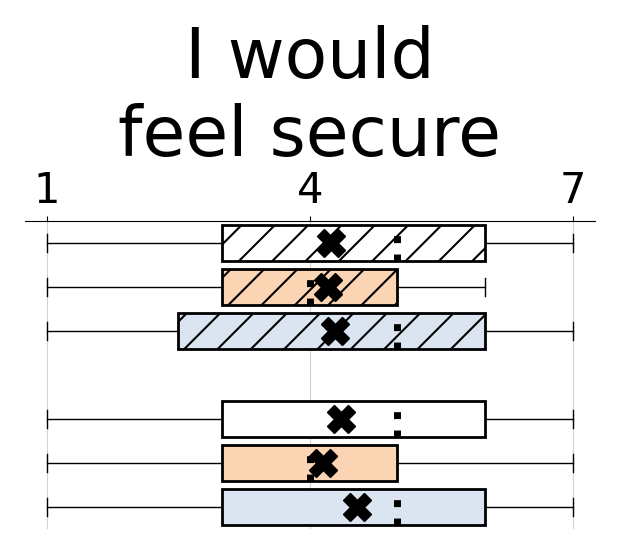}} &
    \multicolumn{2}{c|}{\includegraphics[width = 0.16\columnwidth]{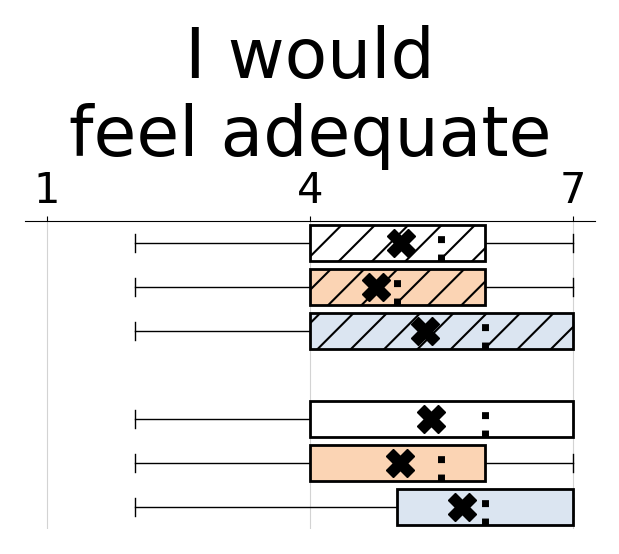}} &
    \multicolumn{2}{c|}{\includegraphics[width = 0.16\columnwidth]{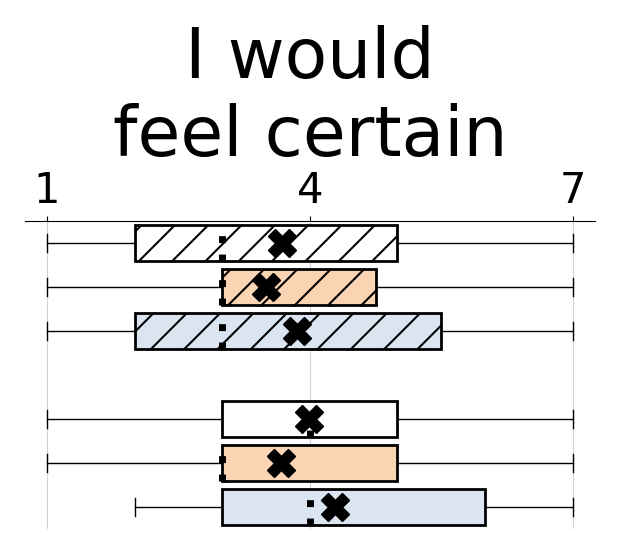}} &
    \multicolumn{2}{c}{\includegraphics[width = 0.16\columnwidth]{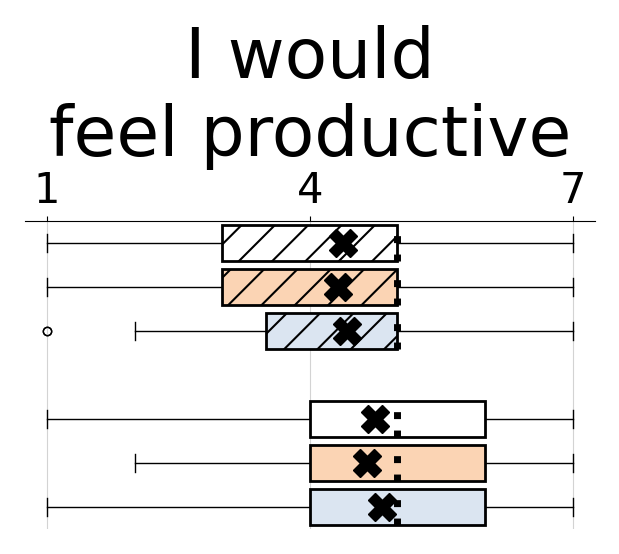}}
    \\
    \hline
    \hline
    \multicolumn{2}{c|}{\includegraphics[width = 0.16\columnwidth]{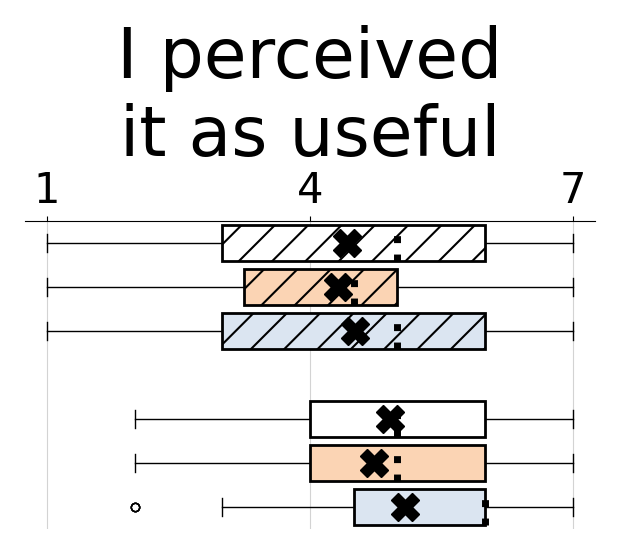}} &
    \multicolumn{2}{c|}{\includegraphics[width = 0.16\columnwidth]{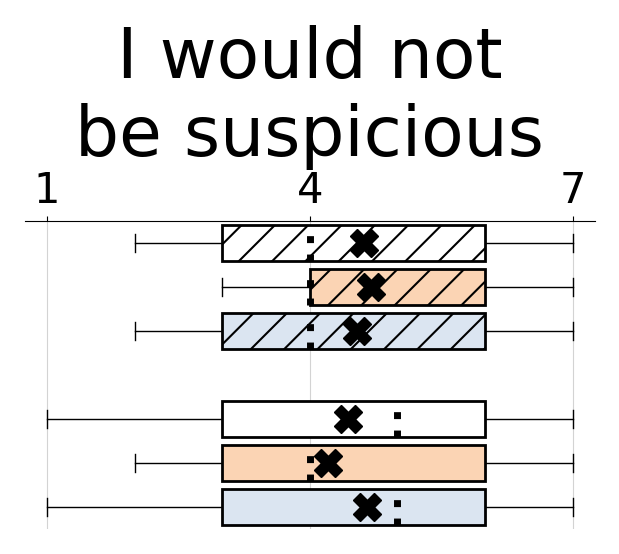}} &
    \multicolumn{2}{c|}{\includegraphics[width = 0.16\columnwidth]{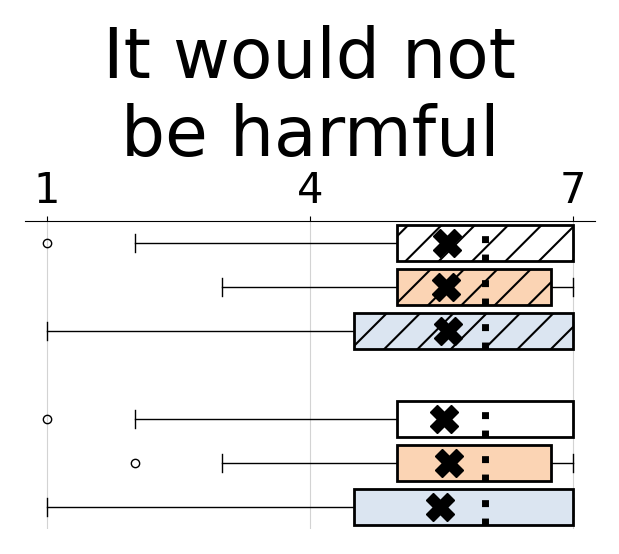}} &
    \multicolumn{2}{c|}{\includegraphics[width = 0.16\columnwidth]{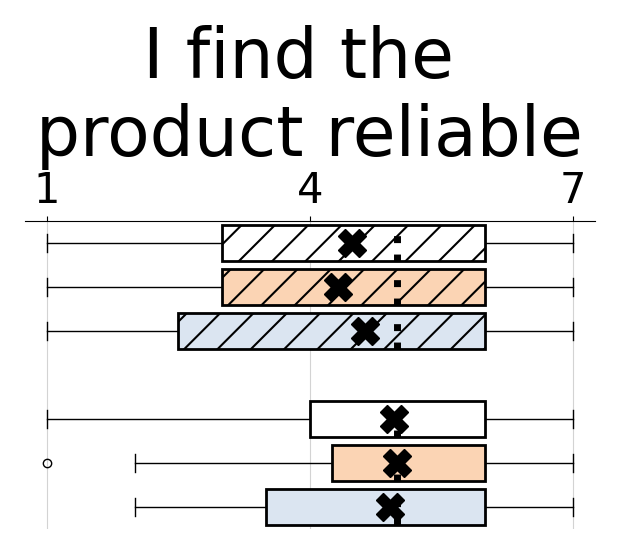}} &
    \multicolumn{2}{c}{\includegraphics[width = 0.16\columnwidth]{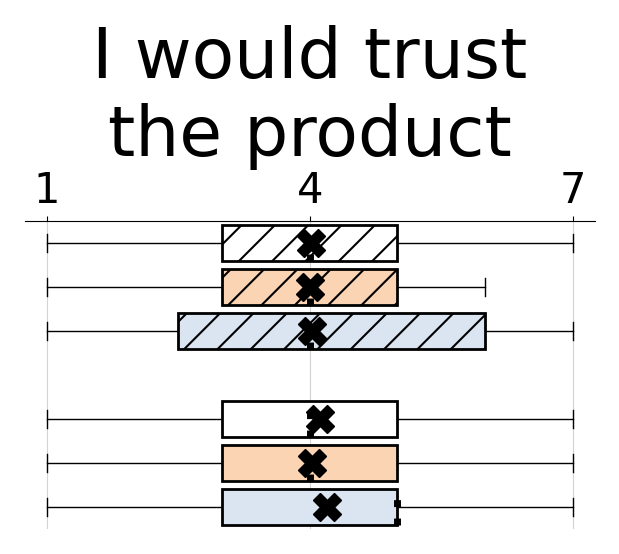}}
    \end{tabular}
    
    \caption{Guideline 12 participants' ratings for all dependent variables, disaggregated by participants' attitudes toward risk.
	%For the disaggregated data, notice how large the distances between the average rating are when the guideline is applied.
	Table~\ref{tab:G12-Risk-Stats-Appendix} below provides the statistics (where applicable).
}
    \label{fig:Risk-G12-Appendix}
\end{table}

\begin{table}[h]

%\framebox[\linewidth]{For Measuring!}
\centering
\footnotesize

    \begin{tabular}{p{0.22\columnwidth}|c|c|c|c|c|c}
    
    \rowcolor{LightGray}\multicolumn{7}{c}{\textbf{Violation AI Product}}\\
    \hline
    \textbf{Dependent}  & \textbf{Distance b/w} &  &  & & \textbf{Bonferroni} &  \\
    \textbf{variable} & \textbf{Means} &  \textbf{df} &  \textbf{t-val} &   \textbf{p-value}  & \textbf{correction} & \textbf{Cohen's \textit{d}} \\
    \hline
    
    I would feel in control & - - - & - &  - - - & - - - & - - - & - - -  \\
    \hline
    
    I would feel secure & - - - & - &  - - - & - - - & - - - & - - - \\
    \hline
    
    I would feel adequate & - - -  & - &  - - - & - - - & - - - & - - - \\
    \hline
    
    I would feel certain & - - - & - &  - - - & - - - & - - - & - - - \\
    \hline
    
    I would feel productive & - - - & - &  - - - & - - - & - - - & - - -   \\
    \hline
    \hline
    
    I perceived it as useful &  - - - & - &  - - - & - - - & - - - & - - -   \\
    \hline
    
    I would not be suspicious & - - - & - &  - - - & - - - & - - - & - - -   \\
    \hline
    
    It would not be harmful & - - - & - &  - - - & - - - & - - - & - - -  \\
    \hline
    
    I find the product reliable & - - - & - &  - - - & - - - & - - - & - - - \\
    \hline
    
    I would trust the product & - - - & - &  - - - & - - - & - - - & - - - \\
    \hline

    \rowcolor{LightGray}\multicolumn{7}{c}{\textbf{Application AI Product}}\\
    \hline
    \textbf{Dependent}  & \textbf{Distance b/w} &  &  & & \textbf{Bonferroni} &  \\
    \textbf{variable} & \textbf{Means} &  \textbf{df} &  \textbf{t-val} &   \textbf{p-value}  & \textbf{correction} & \textbf{Cohen's \textit{d}} \\
    \hline
    
    I would feel in control & - - - & - &  - - - & - - - & - - - & - - -  \\
    \hline
    
    I would feel secure & - - - & - &  - - - & - - - & - - - & - - - \\
    \hline
    
    I would feel adequate & - - -  & - &  - - - & - - - & - - - & - - - \\
    \hline
    
    I would feel certain & - - - & - &  - - - & - - - & - - - & - - - \\
    \hline
    
    I would feel productive & - - - & - &  - - - & - - - & - - - & - - -   \\
    \hline
    \hline
    
    I perceived it as useful &  - - - & - &  - - - & - - - & - - - & - - -   \\
    \hline
    
    I would not be suspicious & - - - & - &  - - - & - - - & - - - & - - -   \\
    \hline
    
    It would not be harmful & - - - & - &  - - - & - - - & - - - & - - -  \\
    \hline
    
    I find the product reliable & - - - & - &  - - - & - - - & - - - & - - - \\
    \hline
    
    I would trust the product & - - - & - &  - - - & - - - & - - - & - - -

    \end{tabular}

    \caption{Guideline 12's t-test results %(\checkmark if Welch's t-test) 
    for risk-averse vs. risk-tolerant participants' average ratings of the independent Violation AI product (top) and Application AI product (bottom), for all 10 dependent variables.
    If dashes (- - -) are present, no statistical test was performed.
    If the number of tests exceeded 5 for each product, Bonferroni correction applied by multiplying p-values by the number of tests performed.
    }
    \label{tab:G12-Risk-Stats-Appendix}
\end{table}
\clearpage
%---------------------------------------------------- End Guideline 12

%Begin Guideline 13----------------------------------------------------

\begin{table}[]
    \centering
    \begin{tabular}{cc|cc|cc|cc|cc}
    \multicolumn{2}{c|}{\includegraphics[width = 0.16\columnwidth]{assets/05-All-BoxPlots/12-G13/Risk/G13-Feel-In-Control-RISK.png}} &
    \multicolumn{2}{c|}{\includegraphics[width = 0.16\columnwidth]{assets/05-All-BoxPlots/12-G13/Risk/G13-Feel-Secure-RISK.png}} &
    \multicolumn{2}{c|}{\includegraphics[width = 0.16\columnwidth]{assets/05-All-BoxPlots/12-G13/Risk/G13-Feel-Adequate-RISK.png}} &
    \multicolumn{2}{c|}{\includegraphics[width = 0.16\columnwidth]{assets/05-All-BoxPlots/12-G13/Risk/G13-Feel-Certain-RISK.png}} &
    \multicolumn{2}{c}{\includegraphics[width = 0.16\columnwidth]{assets/05-All-BoxPlots/12-G13/Risk/G13-Feel-Productive-RISK.png}}
    \\
    \hline
    \hline
    \multicolumn{2}{c|}{\includegraphics[width = 0.16\columnwidth]{assets/05-All-BoxPlots/12-G13/Risk/G13-Perceived-Useful-RISK.png}} &
    \multicolumn{2}{c|}{\includegraphics[width = 0.16\columnwidth]{assets/05-All-BoxPlots/12-G13/Risk/G13-Not-Suspicious-RISK.png}} &
    \multicolumn{2}{c|}{\includegraphics[width = 0.16\columnwidth]{assets/05-All-BoxPlots/12-G13/Risk/G13-Not-Harmful-RISK.png}} &
    \multicolumn{2}{c|}{\includegraphics[width = 0.16\columnwidth]{assets/05-All-BoxPlots/12-G13/Risk/G13-Product-Reliable-RISK.png}} &
    \multicolumn{2}{c}{\includegraphics[width = 0.16\columnwidth]{assets/05-All-BoxPlots/12-G13/Risk/G13-Trust-Product-RISK.png}}
    \end{tabular}
    
    \caption{Guideline 13 participants' ratings for all dependent variables, disaggregated by participants' attitudes toward risk.
	%For the disaggregated data, notice how large the distances between the average rating are when the guideline is applied.
	Table~\ref{tab:G13-Risk-Stats-Appendix} below provides the statistics (where applicable).
}
    \label{fig:Risk-G13-Appendix}
\end{table}

\begin{table}[h]

%\framebox[\linewidth]{For Measuring!}
\centering
\footnotesize

    \begin{tabular}{p{0.22\columnwidth}|c|c|c|c|c|c}
    
    \rowcolor{LightGray}\multicolumn{7}{c}{\textbf{Violation AI Product}}\\
    \hline
    \textbf{Dependent}  & \textbf{Distance b/w} &  &  & & \textbf{Bonferroni} &  \\
    \textbf{variable} & \textbf{Means} &  \textbf{df} &  \textbf{t-val} &   \textbf{p-value}  & \textbf{correction} & \textbf{Cohen's \textit{d}} \\
    \hline
    
    I would feel in control & 0.6444 & 55 &  1.7379 & .0878 & - - - & .4610  \\
    \hline
    
    I would feel secure & - - - & - &  - - - & - - - & - - - & - - - \\
    \hline
    
    I would feel adequate & - - -  & - &  - - - & - - - & - - - & - - - \\
    \hline
    
    I would feel certain & 0.9778 & 55 &  2.3258 & \cellcolor{AbiOrangeQuote}.0237 & - - - & .6170 \\
    \hline
    
    I would feel productive & - - - & - &  - - - & - - - & - - - & - - -   \\
    \hline
    \hline
    
    I perceived it as useful &  - - - & - &  - - - & - - - & - - - & - - -   \\
    \hline
    
    I would not be suspicious & 1.2797 & 54 &  2.9670 & \cellcolor{AbiOrangeQuote}.0045 & - - - & .7935   \\
    \hline
    
    It would not be harmful & 0.8074 & 55 &  2.1230 & \cellcolor{AbiOrangeQuote}.0383 & - - - & .5632  \\
    \hline
    
    I find the product reliable & - - - & - &  - - - & - - - & - - - & - - - \\
    \hline
    
    I would trust the product & - - - & - &  - - - & - - - & - - - & - - - \\
    \hline

    \rowcolor{LightGray}\multicolumn{7}{c}{\textbf{Application AI Product}}\\
    \hline
    \textbf{Dependent}  & \textbf{Distance b/w} &  &  & & \textbf{Bonferroni} &  \\
    \textbf{variable} & \textbf{Means} &  \textbf{df} &  \textbf{t-val} &   \textbf{p-value}  & \textbf{correction} & \textbf{Cohen's \textit{d}} \\
    \hline
    
    I would feel in control & - - - & - &  - - - & - - - & - - - & - - -  \\
    \hline
    
    I would feel secure & - - - & - &  - - - & - - - & - - - & - - - \\
    \hline
    
    I would feel adequate & 1.0926  & 55 &  3.2194 & \cellcolor{AbiOrangeQuote}.0022 & \cellcolor{AbiOrangeQuote}.0132 & .8540 \\
    \hline
    
    I would feel certain & 1.0593 & 55 &  2.7497 & \cellcolor{AbiOrangeQuote}.0081 & \cellcolor{AbiOrangeQuote}.0486 & .7294 \\
    \hline
    
    I would feel productive & - - - & - &  - - - & - - - & - - - & - - -   \\
    \hline
    \hline
    
    I perceived it as useful &  0.6821 & 54 &  2.6993 & \cellcolor{AbiOrangeQuote}.0093 & .0558 & .7233   \\
    \hline
    
    I would not be suspicious & 1.0498 & 54 & 2.6922 & \cellcolor{AbiOrangeQuote}.0094 & .0564 & .7200   \\
    \hline
    
    It would not be harmful & 0.9852 & 55 &  3.0754 & \cellcolor{AbiOrangeQuote}.0033 & \cellcolor{AbiOrangeQuote}.0198 & .8158  \\
    \hline
    
    I find the product reliable & - - - & - &  - - - & - - - & - - - & - - - \\
    \hline
    
    I would trust the product & 0.6066 & 54 &  1.9399 & .0576 & .3456 & .5188

    \end{tabular}

    \caption{Guideline 13's t-test results %(\checkmark if Welch's t-test) 
    for risk-averse vs. risk-tolerant participants' average ratings of the independent Violation AI product (top) and Application AI product (bottom), for all 10 dependent variables.
    If dashes (- - -) are present, no statistical test was performed.
    If the number of tests exceeded 5 for each product, Bonferroni correction applied by multiplying p-values by the number of tests performed.
    }
    \label{tab:G13-Risk-Stats-Appendix}
\end{table}
\clearpage
%---------------------------------------------------- End Guideline 13

%Begin Guideline 14---------------------------------------------------

\begin{table}[]
    \centering
    \begin{tabular}{cc|cc|cc|cc|cc}
    \multicolumn{2}{c|}{\includegraphics[width = 0.16\columnwidth]{assets/05-All-BoxPlots/13-G14/Risk/G14-Feel-In-Control-RISK.png}} &
    \multicolumn{2}{c|}{\includegraphics[width = 0.16\columnwidth]{assets/05-All-BoxPlots/13-G14/Risk/G14-Feel-Secure-RISK.png}} &
    \multicolumn{2}{c|}{\includegraphics[width = 0.16\columnwidth]{assets/05-All-BoxPlots/13-G14/Risk/G14-Feel-Adequate-RISK.png}} &
    \multicolumn{2}{c|}{\includegraphics[width = 0.16\columnwidth]{assets/05-All-BoxPlots/13-G14/Risk/G14-Feel-Certain-RISK.png}} &
    \multicolumn{2}{c}{\includegraphics[width = 0.16\columnwidth]{assets/05-All-BoxPlots/13-G14/Risk/G14-Feel-Productive-RISK.png}}
    \\
    \hline
    \hline
    \multicolumn{2}{c|}{\includegraphics[width = 0.16\columnwidth]{assets/05-All-BoxPlots/13-G14/Risk/G14-Perceived-Useful-RISK.png}} &
    \multicolumn{2}{c|}{\includegraphics[width = 0.16\columnwidth]{assets/05-All-BoxPlots/13-G14/Risk/G14-Not-Suspicious-RISK.png}} &
    \multicolumn{2}{c|}{\includegraphics[width = 0.16\columnwidth]{assets/05-All-BoxPlots/13-G14/Risk/G14-Not-Harmful-RISK.png}} &
    \multicolumn{2}{c|}{\includegraphics[width = 0.16\columnwidth]{assets/05-All-BoxPlots/13-G14/Risk/G14-Product-Reliable-RISK.png}} &
    \multicolumn{2}{c}{\includegraphics[width = 0.16\columnwidth]{assets/05-All-BoxPlots/13-G14/Risk/G14-Trust-Product-RISK.png}}
    \end{tabular}
    
    \caption{Guideline 14 participants' ratings for all dependent variables, disaggregated by participants' attitudes toward risk.
	%For the disaggregated data, notice how large the distances between the average rating are when the guideline is applied.
	Table~\ref{tab:G14-Risk-Stats-Appendix} below provides the statistics (where applicable).
}
    \label{fig:Risk-G14-Appendix}
\end{table}

\begin{table}[h]

%\framebox[\linewidth]{For Measuring!}
\centering
\footnotesize

    \begin{tabular}{p{0.22\columnwidth}|c|c|c|c|c|c}
    
    \rowcolor{LightGray}\multicolumn{7}{c}{\textbf{Violation AI Product}}\\
    \hline
    \textbf{Dependent}  & \textbf{Distance b/w} &  &  & & \textbf{Bonferroni} &  \\
    \textbf{variable} & \textbf{Means} &  \textbf{df} &  \textbf{t-val} &   \textbf{p-value}  & \textbf{correction} & \textbf{Cohen's \textit{d}} \\
    \hline
    
    I would feel in control & - - - & - &  - - - & - - - & - - - & - - -  \\
    \hline
    
    I would feel secure & - - - & - &  - - - & - - - & - - - & - - - \\
    \hline
    
    I would feel adequate & 1.1883  & 65 &  3.0443 & \cellcolor{AbiOrangeQuote}.0034 & - - - & .7479 \\
    \hline
    
    I would feel certain & 0.8477 & 65 &  1.9967 & .05005 & - - - & .4906 \\
    \hline
    
    I would feel productive & 0.7951 & 66 &  2.1935 & \cellcolor{AbiOrangeQuote}.0318 & - - - & .5341   \\
    \hline
    \hline
    
    I perceived it as useful &  - - - & - &  - - - & - - - & - - - & - - -   \\
    \hline
    
    I would not be suspicious & - - - & - &  - - - & - - - & - - - & - - -   \\
    \hline
    
    It would not be harmful & 0.7190 & - &  - - - & - - - & - - - & - - -  \\
    \hline
    
    I find the product reliable & - - - & - &  - - - & - - - & - - - & - - - \\
    \hline
    
    I would trust the product & - - - & - &  - - - & - - - & - - - & - - - \\
    \hline

    \rowcolor{LightGray}\multicolumn{7}{c}{\textbf{Application AI Product}}\\
    \hline
    \textbf{Dependent}  & \textbf{Distance b/w} &  &  & & \textbf{Bonferroni} &  \\
    \textbf{variable} & \textbf{Means} &  \textbf{df} &  \textbf{t-val} &   \textbf{p-value}  & \textbf{correction} & \textbf{Cohen's \textit{d}} \\
    \hline
    
    I would feel in control & 0.6347 & 66 &  1.8472 & .0692 & - - - & .4498  \\
    \hline
    
    I would feel secure & 0.5708 & 65 &  1.7537 & .0842& - - - & .4297 \\
    \hline
    
    I would feel adequate & 0.9077  & 65 &  3.0669 & \cellcolor{AbiOrangeQuote}.0032 & - - - & .7514 \\
    \hline
    
    I would feel certain & - - - & - &  - - - & - - - & - - - & - - - \\
    \hline
    
    I would feel productive & 0.5292 & 66 &  2.1136 & \cellcolor{AbiOrangeQuote}.0383 & - - - & .5146   \\
    \hline
    \hline
    
    I perceived it as useful &  - - - & - &  - - - & - - - & - - - & - - -   \\
    \hline
    
    I would not be suspicious & - - - & - &  - - - & - - - & - - - & - - -   \\
    \hline
    
    It would not be harmful & - - - & - &  - - - & - - - & - - - & - - -  \\
    \hline
    
    I find the product reliable & - - - & - &  - - - & - - - & - - - & - - - \\
    \hline
    
    I would trust the product & - - - & - &  - - - & - - - & - - - & - - -

    \end{tabular}

    \caption{Guideline 14's t-test results %(\checkmark if Welch's t-test) 
    for risk-averse vs. risk-tolerant participants' average ratings of the independent Violation AI product (top) and Application AI product (bottom), for all 10 dependent variables.
    If dashes (- - -) are present, no statistical test was performed.
    If the number of tests exceeded 5 for each product, Bonferroni correction applied by multiplying p-values by the number of tests performed.
    }
    \label{tab:G14-Risk-Stats-Appendix}
\end{table}
\clearpage
%---------------------------------------------------- End Guideline 14

%Begin Guideline 15---------------------------------------------------

\begin{table}[]
    \centering
    \begin{tabular}{cc|cc|cc|cc|cc}
    \multicolumn{2}{c|}{\includegraphics[width = 0.16\columnwidth]{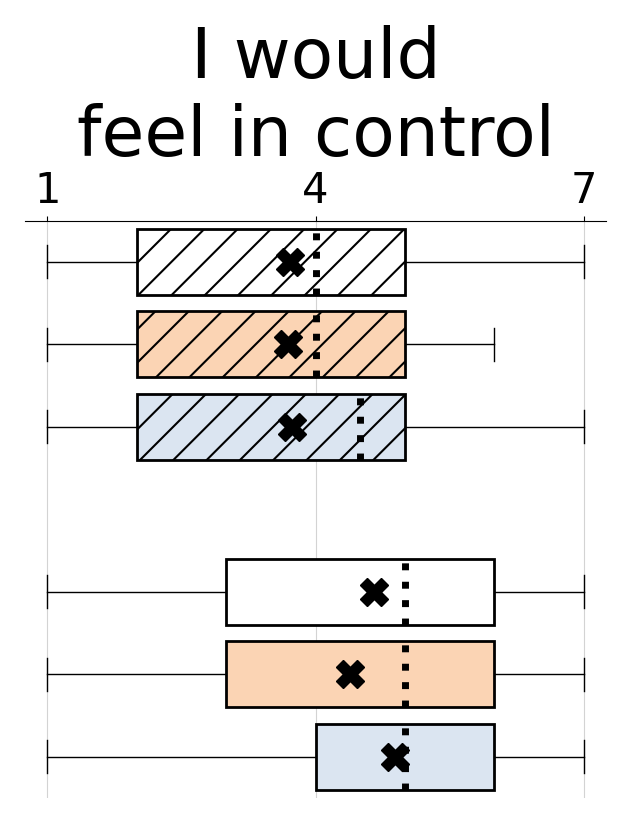}} &
    \multicolumn{2}{c|}{\includegraphics[width = 0.16\columnwidth]{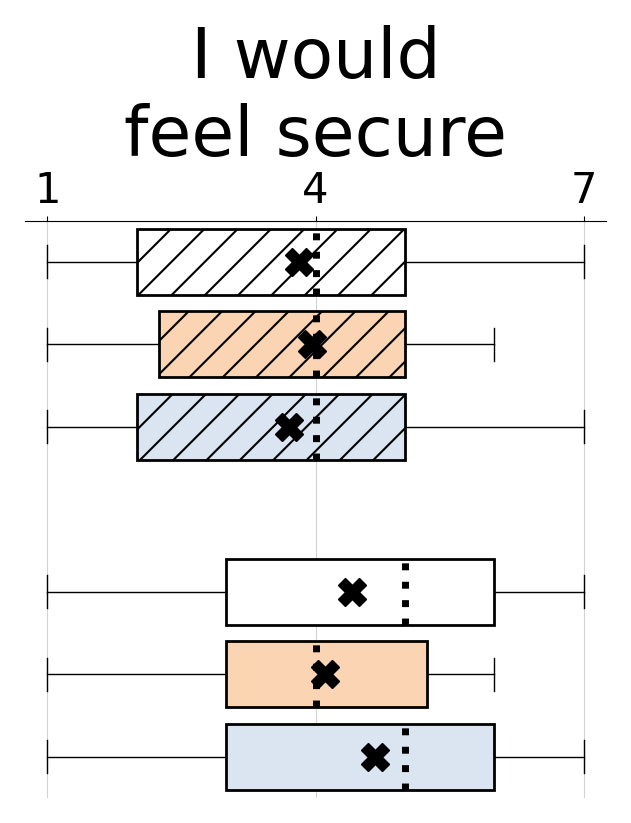}} &
    \multicolumn{2}{c|}{\includegraphics[width = 0.16\columnwidth]{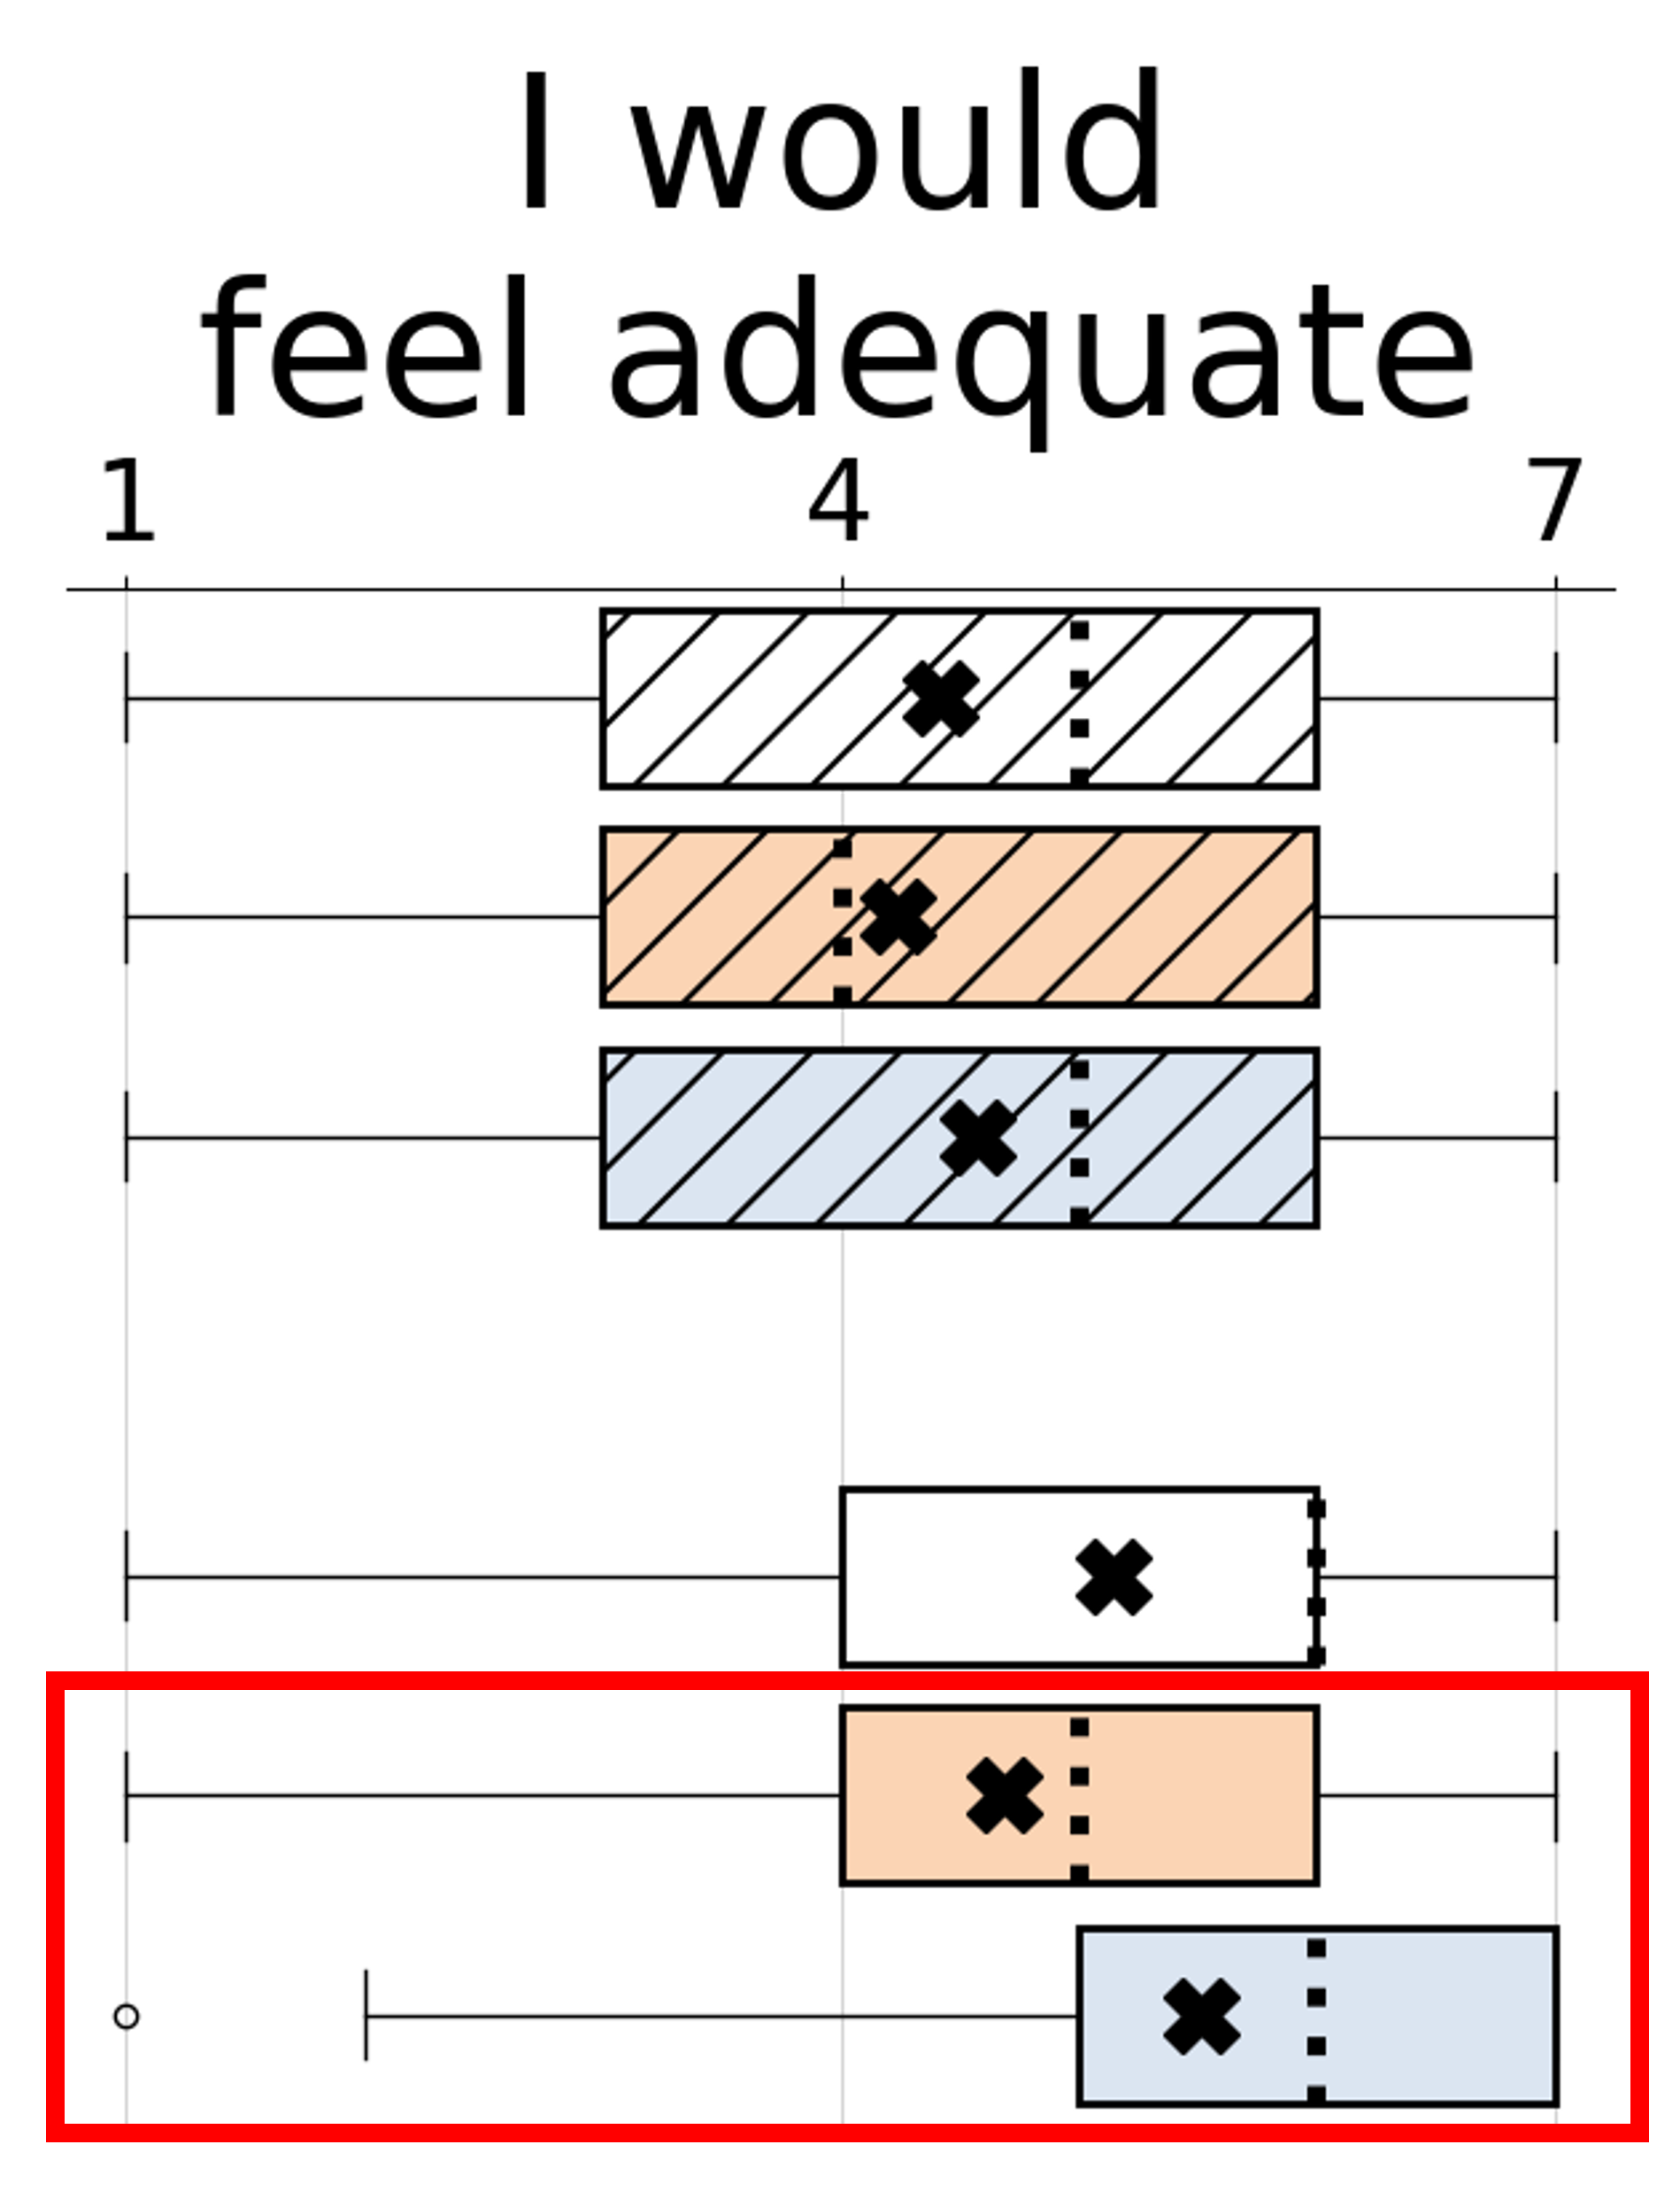}} &
    \multicolumn{2}{c|}{\includegraphics[width = 0.16\columnwidth]{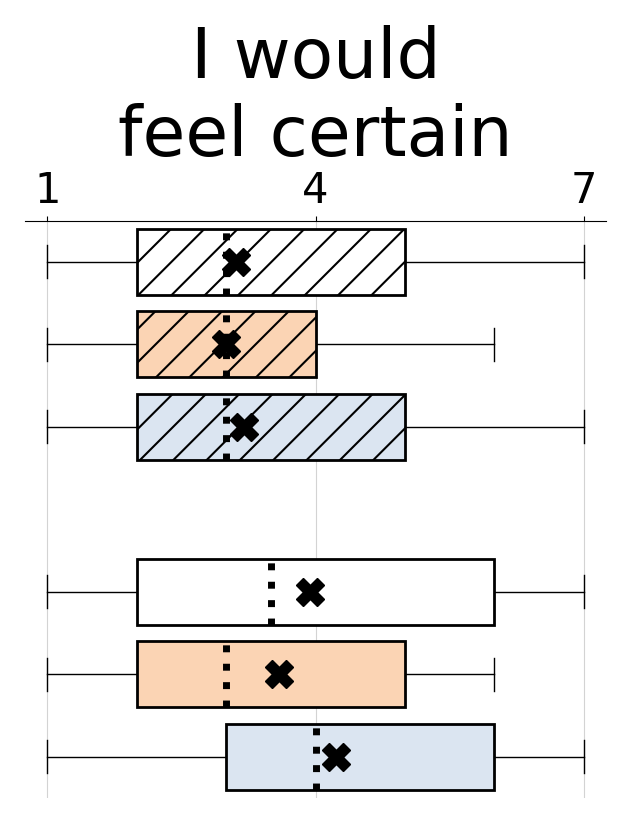}} &
    \multicolumn{2}{c}{\includegraphics[width = 0.16\columnwidth]{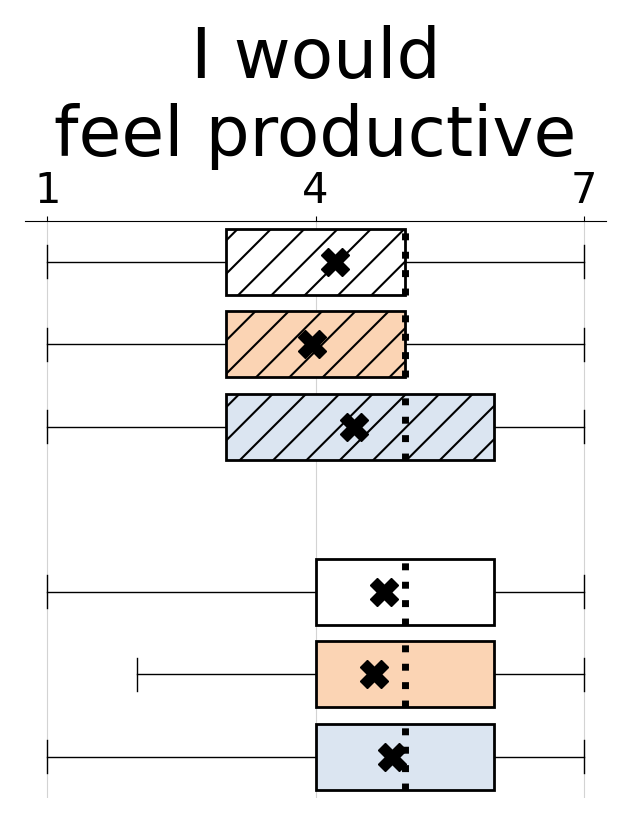}}
    \\
    \hline
    \hline
    \multicolumn{2}{c|}{\includegraphics[width = 0.16\columnwidth]{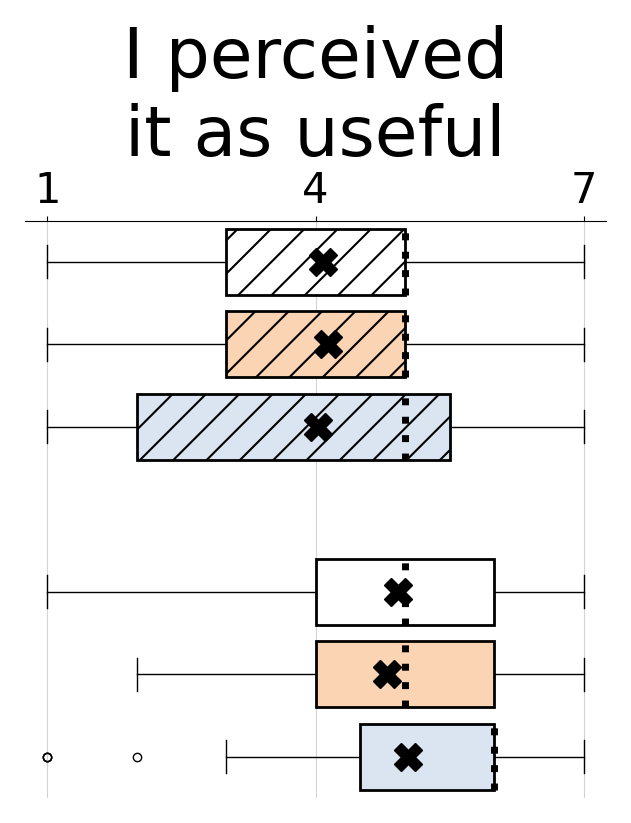}} &
    \multicolumn{2}{c|}{\includegraphics[width = 0.16\columnwidth]{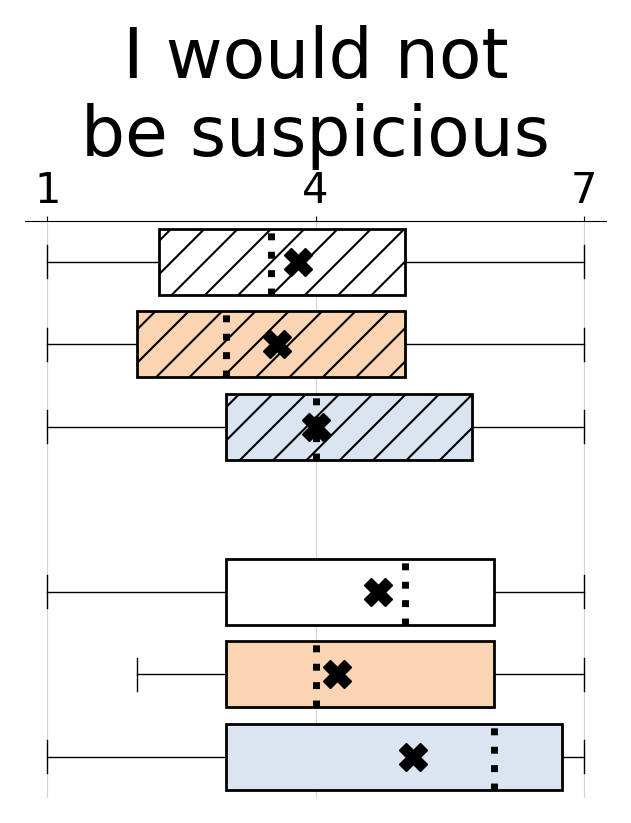}} &
    \multicolumn{2}{c|}{\includegraphics[width = 0.16\columnwidth]{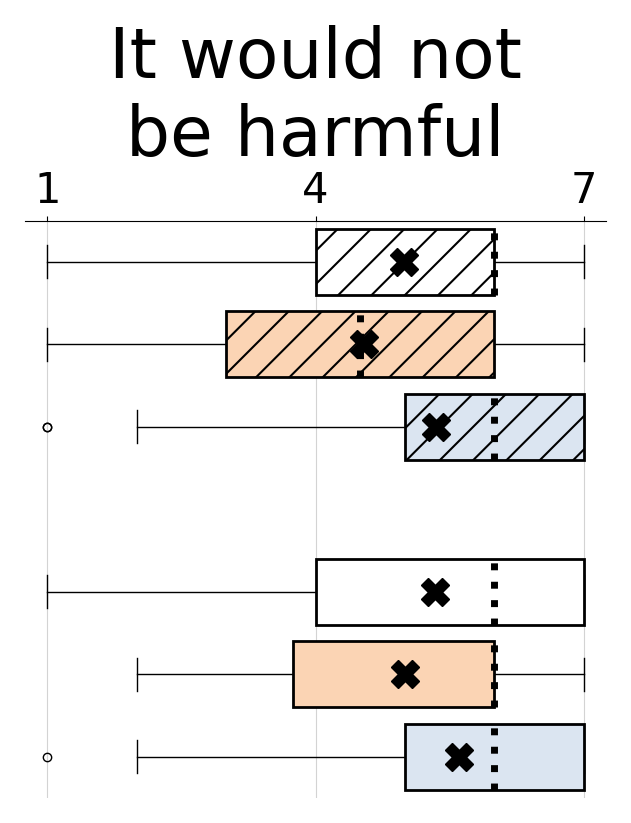}} &
    \multicolumn{2}{c|}{\includegraphics[width = 0.16\columnwidth]{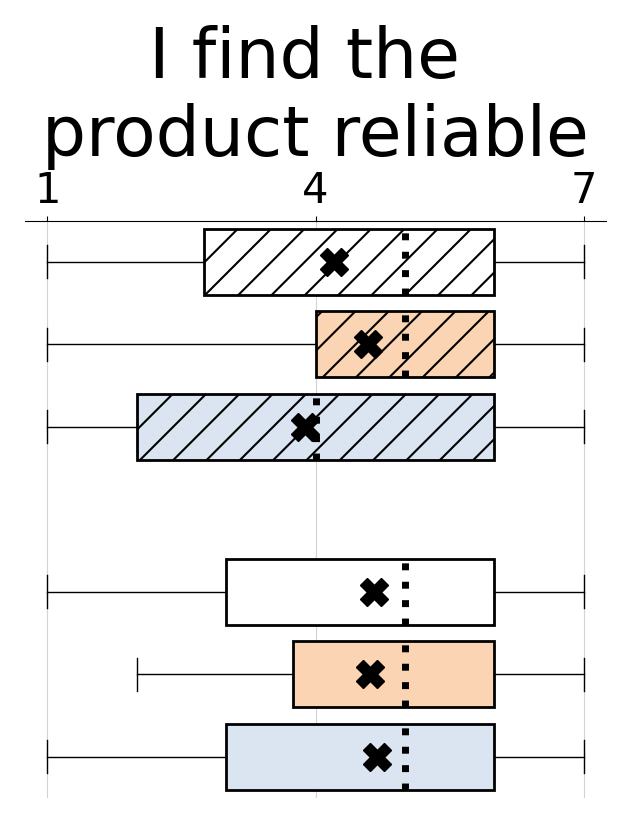}} &
    \multicolumn{2}{c}{\includegraphics[width = 0.16\columnwidth]{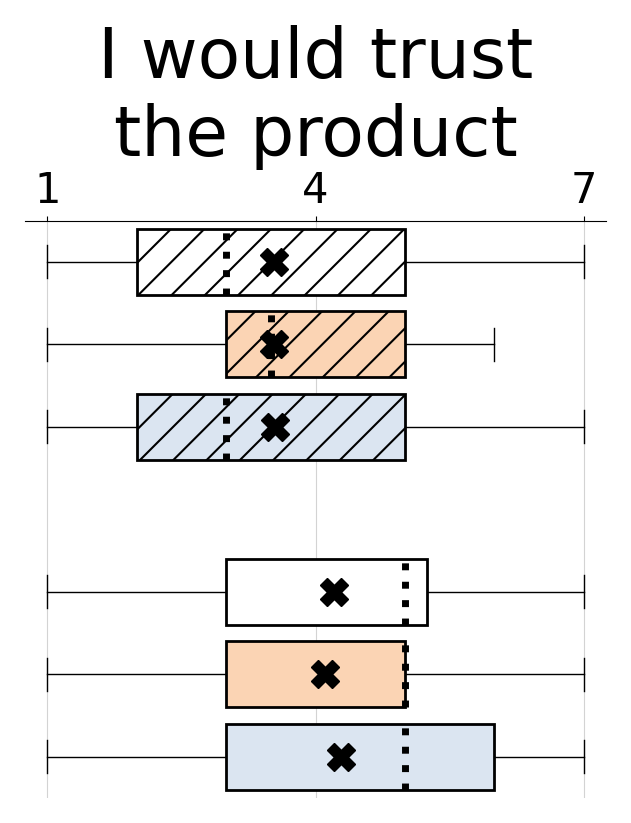}}
    \end{tabular}
    
    \caption{Guideline 15 participants' ratings for all dependent variables, disaggregated by participants' attitudes toward risk.
	%For the disaggregated data, notice how large the distances between the average rating are when the guideline is applied.
	Table~\ref{tab:G15-Risk-Stats-Appendix} below provides the statistics (where applicable).
}
    \label{fig:Risk-G15-Appendix}
\end{table}

\begin{table}[h]

%\framebox[\linewidth]{For Measuring!}
\centering
\footnotesize

    \begin{tabular}{p{0.22\columnwidth}|c|c|c|c|c|c}
    
    \rowcolor{LightGray}\multicolumn{7}{c}{\textbf{Violation AI Product}}\\
    \hline
    \textbf{Dependent}  & \textbf{Distance b/w} &  &  & & \textbf{Bonferroni} &  \\
    \textbf{variable} & \textbf{Means} &  \textbf{df} &  \textbf{t-val} &   \textbf{p-value}  & \textbf{correction} & \textbf{Cohen's \textit{d}} \\
    \hline
    
    I would feel in control & - - - & - &  - - - & - - - & - - - & - - -  \\
    \hline
    
    I would feel secure & - - - & - &  - - - & - - - & - - - & - - - \\
    \hline
    
    I would feel adequate & - - -  & - &  - - - & - - - & - - - & - - - \\
    \hline
    
    I would feel certain & - - - & - &  - - - & - - - & - - - & - - - \\
    \hline
    
    I would feel productive & - - - & - &  - - - & - - - & - - - & - - -   \\
    \hline
    \hline
    
    I perceived it as useful &  - - - & - &  - - - & - - - & - - - & - - -   \\
    \hline
    
    I would not be suspicious & - - - & - &  - - - & - - - & - - - & - - -   \\
    \hline
    
    It would not be harmful & - - - & - &  - - - & - - - & - - - & - - -  \\
    \hline
    
    I find the product reliable & 0.7005 & 62 &  1.5137 & .1352 & - - - & .3801 \\
    \hline
    
    I would trust the product & - - - & - &  - - - & - - - & - - - & - - - \\
    \hline

    \rowcolor{LightGray}\multicolumn{7}{c}{\textbf{Application AI Product}}\\
    \hline
    \textbf{Dependent}  & \textbf{Distance b/w} &  &  & & \textbf{Bonferroni} &  \\
    \textbf{variable} & \textbf{Means} &  \textbf{df} &  \textbf{t-val} &   \textbf{p-value}  & \textbf{correction} & \textbf{Cohen's \textit{d}} \\
    \hline
    
    I would feel in control & - - - & - &  - - - & - - - & - - - & - - -  \\
    \hline
    
    I would feel secure & - - - & - &  - - - & - - - & - - - & - - - \\
    \hline
    
    I would feel adequate & 0.8246  & 62 &  2.0013 & \cellcolor{AbiOrangeQuote}.0497 & - - - & .5025 \\
    \hline
    
    I would feel certain & - - - & - &  - - - & - - - & - - - & - - - \\
    \hline
    
    I would feel productive & - - - & - &  - - - & - - - & - - - & - - -   \\
    \hline
    \hline
    
    I perceived it as useful &  - - - & - &  - - - & - - - & - - - & - - -   \\
    \hline
    
    I would not be suspicious & 0.8469 & 61 &  1.9501 & .0558 & - - - & .4929   \\
    \hline
    
    It would not be harmful & - - - & - &  - - - & - - - & - - - & - - -  \\
    \hline
    
    I find the product reliable & - - - & - &  - - - & - - - & - - - & - - - \\
    \hline
    
    I would trust the product & - - - & - &  - - - & - - - & - - - & - - -

    \end{tabular}

    \caption{Guideline 15's t-test results %(\checkmark if Welch's t-test) 
    for risk-averse vs. risk-tolerant participants' average ratings of the independent Violation AI product (top) and Application AI product (bottom), for all 10 dependent variables.
    If dashes (- - -) are present, no statistical test was performed.
    If the number of tests exceeded 5 for each product, Bonferroni correction applied by multiplying p-values by the number of tests performed.
    }
    \label{tab:G15-Risk-Stats-Appendix}
\end{table}
\clearpage
%---------------------------------------------------- End Guideline 15

%Begin Guideline 17---------------------------------------------------

\begin{table}[]
    \centering
    \begin{tabular}{cc|cc|cc|cc|cc}
    \multicolumn{2}{c|}{\includegraphics[width = 0.16\columnwidth]{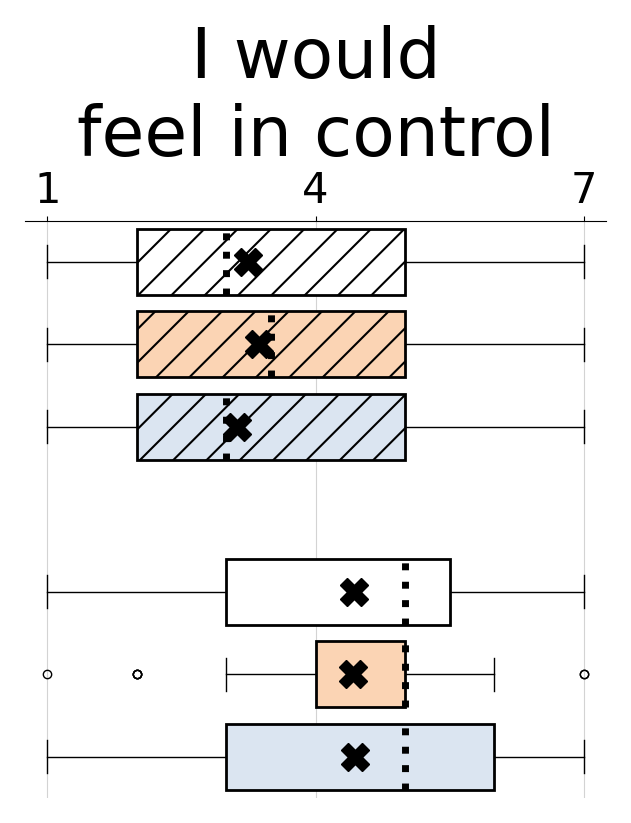}} &
    \multicolumn{2}{c|}{\includegraphics[width = 0.16\columnwidth]{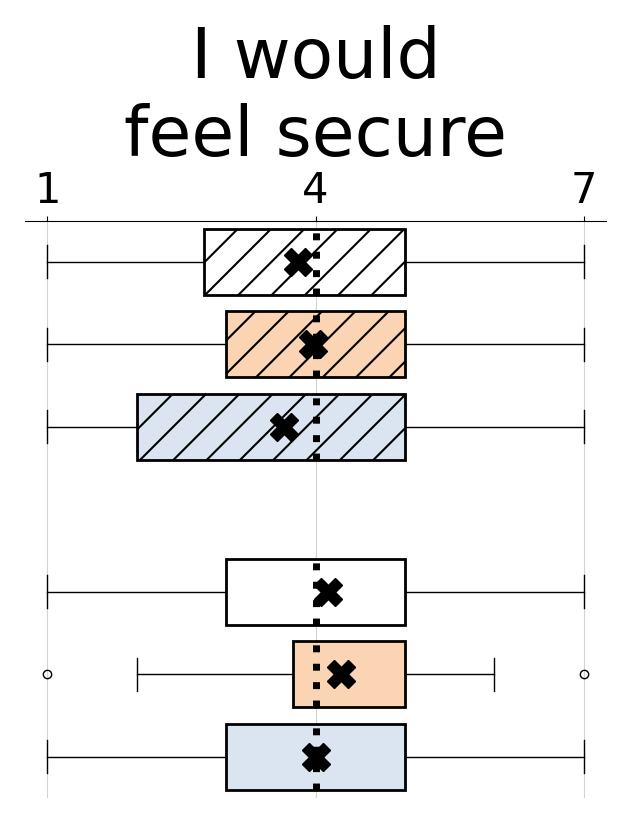}} &
    \multicolumn{2}{c|}{\includegraphics[width = 0.16\columnwidth]{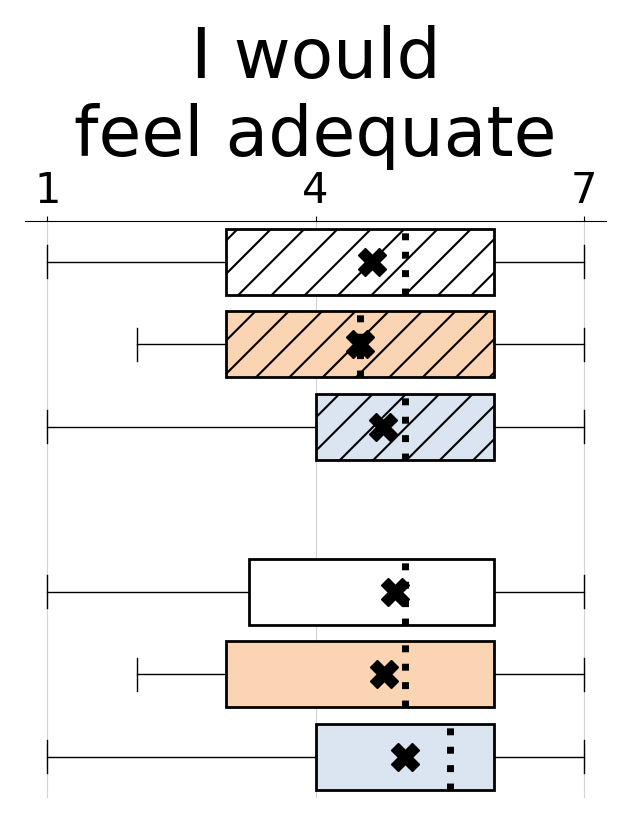}} &
    \multicolumn{2}{c|}{\includegraphics[width = 0.16\columnwidth]{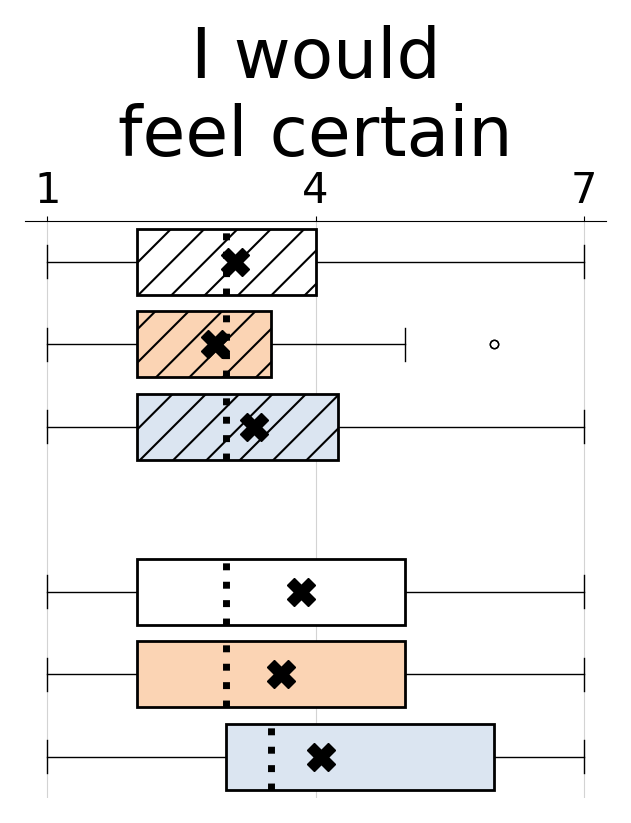}} &
    \multicolumn{2}{c}{\includegraphics[width = 0.16\columnwidth]{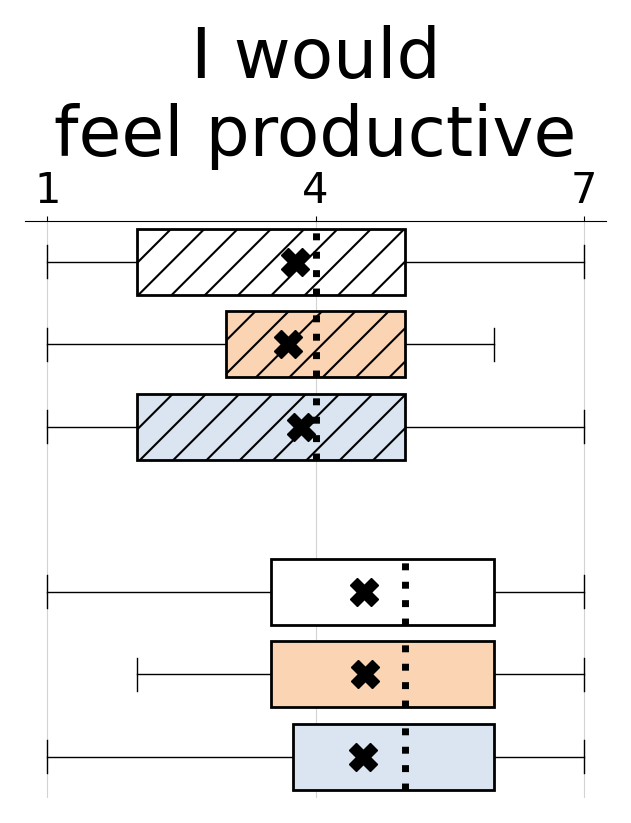}}
    \\
    \hline
    \hline
    \multicolumn{2}{c|}{\includegraphics[width = 0.16\columnwidth]{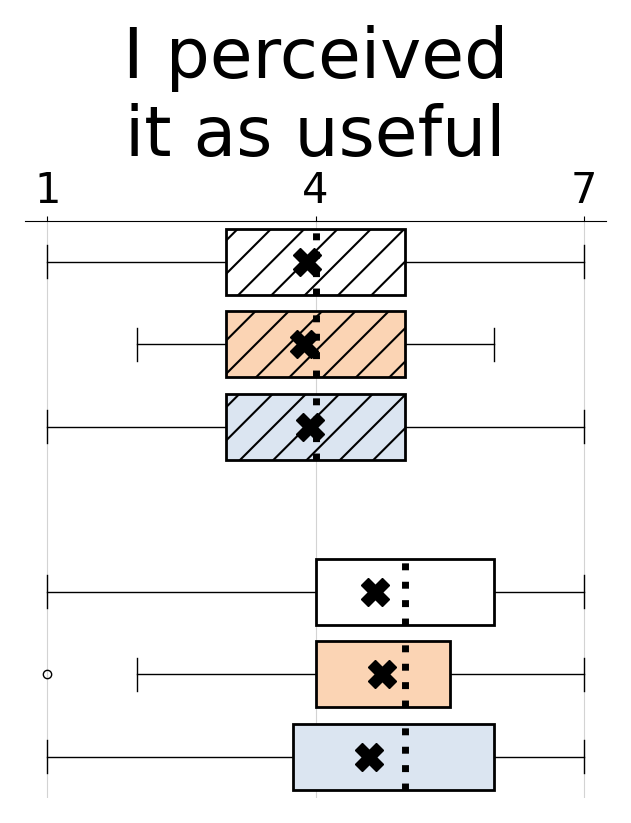}} &
    \multicolumn{2}{c|}{\includegraphics[width = 0.16\columnwidth]{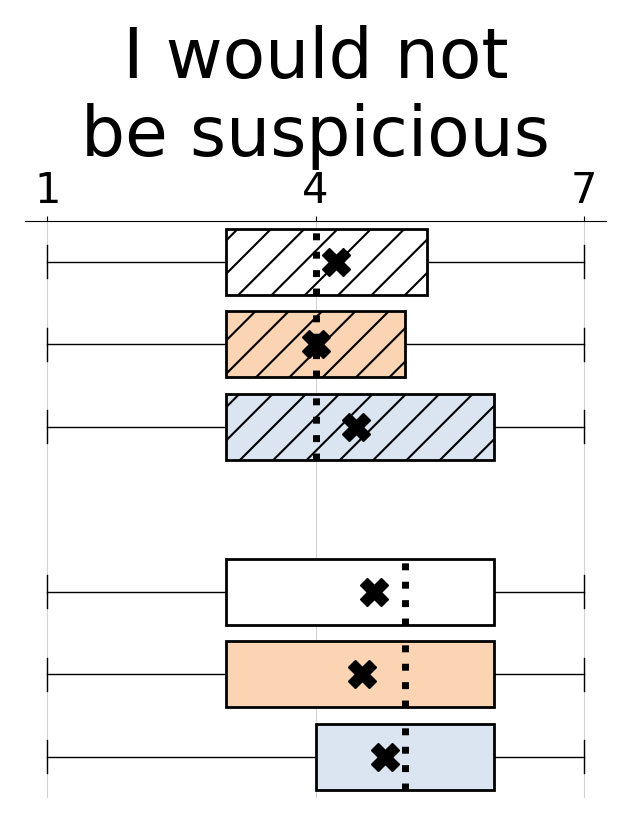}} &
    \multicolumn{2}{c|}{\includegraphics[width = 0.16\columnwidth]{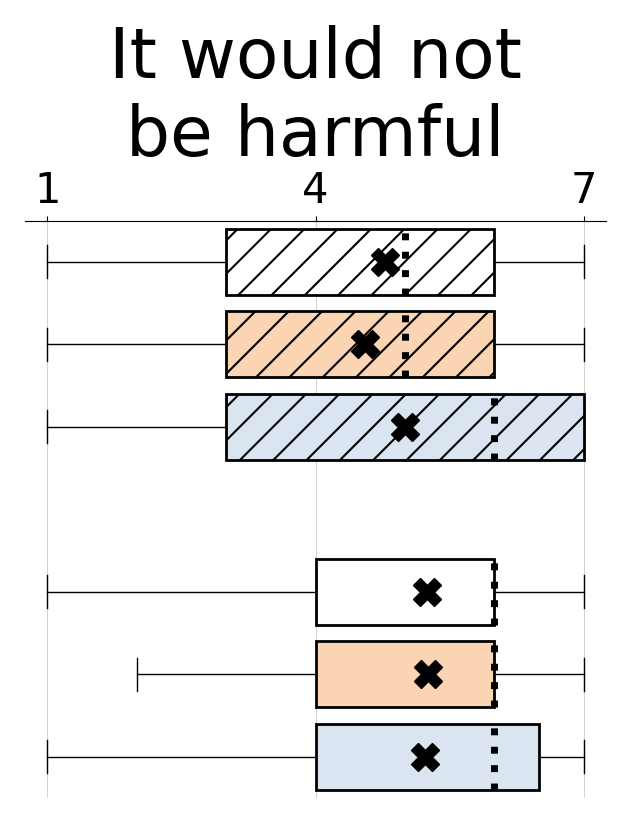}} &
    \multicolumn{2}{c|}{\includegraphics[width = 0.16\columnwidth]{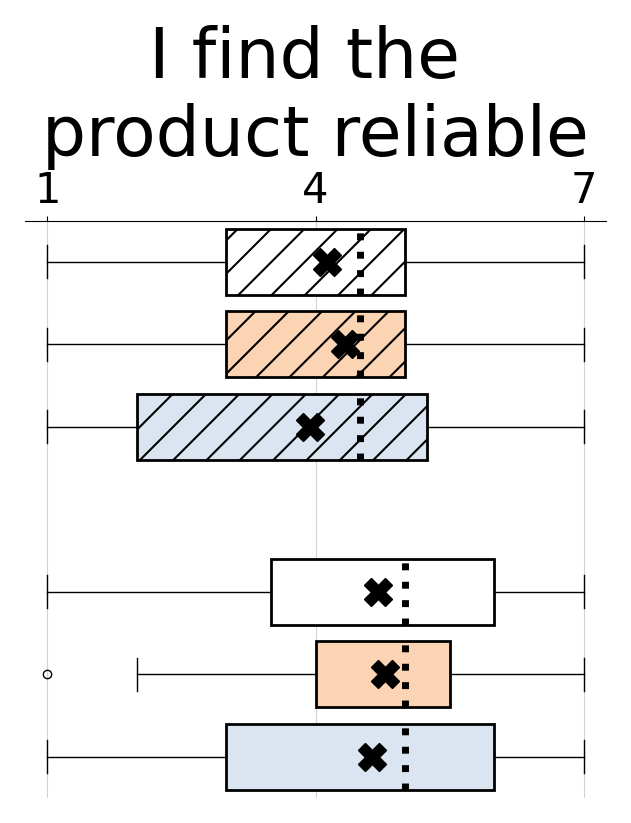}} &
    \multicolumn{2}{c}{\includegraphics[width = 0.16\columnwidth]{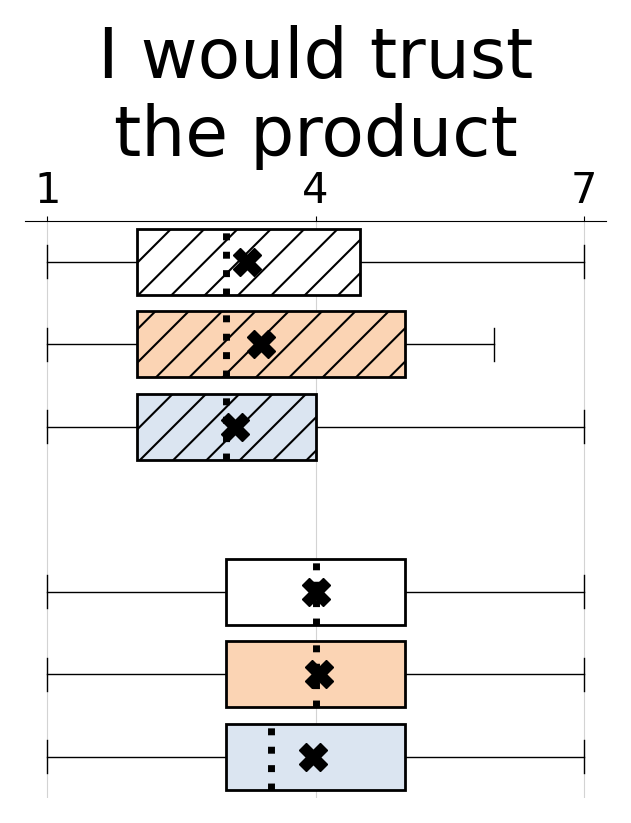}}
    \end{tabular}
    
    \caption{Guideline 17 participants' ratings for all dependent variables, disaggregated by participants' attitudes toward risk.
	%For the disaggregated data, notice how large the distances between the average rating are when the guideline is applied.
	Table~\ref{tab:G17-Risk-Stats-Appendix} below provides the statistics (where applicable).
}
    \label{fig:Risk-G17-Appendix}
\end{table}

\begin{table}[h]

%\framebox[\linewidth]{For Measuring!}
\centering
\footnotesize

    \begin{tabular}{p{0.22\columnwidth}|c|c|c|c|c|c}
    
    \rowcolor{LightGray}\multicolumn{7}{c}{\textbf{Violation AI Product}}\\
    \hline
    \textbf{Dependent}  & \textbf{Distance b/w} &  &  & & \textbf{Bonferroni} &  \\
    \textbf{variable} & \textbf{Means} &  \textbf{df} &  \textbf{t-val} &   \textbf{p-value}  & \textbf{correction} & \textbf{Cohen's \textit{d}} \\
    \hline
    
    I would feel in control & - - - & - &  - - - & - - - & - - - & - - -  \\
    \hline
    
    I would feel secure & - - - & - &  - - - & - - - & - - - & - - - \\
    \hline
    
    I would feel adequate & - - -  & - &  - - - & - - - & - - - & - - - \\
    \hline
    
    I would feel certain & - - - & - &  - - - & - - - & - - - & - - - \\
    \hline
    
    I would feel productive & - - - & - &  - - - & - - - & - - - & - - -   \\
    \hline
    \hline
    
    I perceived it as useful &  - - - & - &  - - - & - - - & - - - & - - -   \\
    \hline
    
    I would not be suspicious & - - - & - &  - - - & - - - & - - - & - - -   \\
    \hline
    
    It would not be harmful & - - - & - &  - - - & - - - & - - - & - - -  \\
    \hline
    
    I find the product reliable & - - - & - &  - - - & - - - & - - - & - - - \\
    \hline
    
    I would trust the product & - - - & - &  - - - & - - - & - - - & - - - \\
    \hline

    \rowcolor{LightGray}\multicolumn{7}{c}{\textbf{Application AI Product}}\\
    \hline
    \textbf{Dependent}  & \textbf{Distance b/w} &  &  & & \textbf{Bonferroni} &  \\
    \textbf{variable} & \textbf{Means} &  \textbf{df} &  \textbf{t-val} &   \textbf{p-value}  & \textbf{correction} & \textbf{Cohen's \textit{d}} \\
    \hline
    
    I would feel in control & - - - & - &  - - - & - - - & - - - & - - -  \\
    \hline
    
    I would feel secure & - - - & - &  - - - & - - - & - - - & - - - \\
    \hline
    
    I would feel adequate & - - -  & - &  - - - & - - - & - - - & - - - \\
    \hline
    
    I would feel certain & - - - & - &  - - - & - - - & - - - & - - - \\
    \hline
    
    I would feel productive & - - - & - &  - - - & - - - & - - - & - - -   \\
    \hline
    \hline
    
    I perceived it as useful &  - - - & - &  - - - & - - - & - - - & - - -   \\
    \hline
    
    I would not be suspicious & - - - & - &  - - - & - - - & - - - & - - -   \\
    \hline
    
    It would not be harmful & - - - & - &  - - - & - - - & - - - & - - -  \\
    \hline
    
    I find the product reliable & - - - & - &  - - - & - - - & - - - & - - - \\
    \hline
    
    I would trust the product & - - - & - &  - - - & - - - & - - - & - - -

    \end{tabular}

    \caption{Guideline 17's t-test results %(\checkmark if Welch's t-test) 
    for risk-averse vs. risk-tolerant participants' average ratings of the independent Violation AI product (top) and Application AI product (bottom), for all 10 dependent variables.
    If dashes (- - -) are present, no statistical test was performed.
    If the number of tests exceeded 5 for each product, Bonferroni correction applied by multiplying p-values by the number of tests performed.
    }
    \label{tab:G17-Risk-Stats-Appendix}
\end{table}
\clearpage
%---------------------------------------------------- End Guideline 17

%Begin Guideline 17---------------------------------------------------

\begin{table}[]
    \centering
    \begin{tabular}{cc|cc|cc|cc|cc}
    \multicolumn{2}{c|}{\includegraphics[width = 0.16\columnwidth]{assets/05-All-BoxPlots/16-G18/Risk/G18-Feel-In-Control-RISK.png}} &
    \multicolumn{2}{c|}{\includegraphics[width = 0.16\columnwidth]{assets/05-All-BoxPlots/16-G18/Risk/G18-Feel-Secure-RISK.png}} &
    \multicolumn{2}{c|}{\includegraphics[width = 0.16\columnwidth]{assets/05-All-BoxPlots/16-G18/Risk/G18-Feel-Adequate-RISK.png}} &
    \multicolumn{2}{c|}{\includegraphics[width = 0.16\columnwidth]{assets/05-All-BoxPlots/16-G18/Risk/G18-Feel-Certain-RISK.png}} &
    \multicolumn{2}{c}{\includegraphics[width = 0.16\columnwidth]{assets/05-All-BoxPlots/16-G18/Risk/G18-Feel-Productive-RISK.png}}
    \\
    \hline
    \hline
    \multicolumn{2}{c|}{\includegraphics[width = 0.16\columnwidth]{assets/05-All-BoxPlots/16-G18/Risk/G18-Perceived-Useful-RISK.png}} &
    \multicolumn{2}{c|}{\includegraphics[width = 0.16\columnwidth]{assets/05-All-BoxPlots/16-G18/Risk/G18-Not-Suspicious-RISK.png}} &
    \multicolumn{2}{c|}{\includegraphics[width = 0.16\columnwidth]{assets/05-All-BoxPlots/16-G18/Risk/G18-Not-Harmful-RISK.png}} &
    \multicolumn{2}{c|}{\includegraphics[width = 0.16\columnwidth]{assets/05-All-BoxPlots/16-G18/Risk/G18-Product-Reliable-RISK.png}} &
    \multicolumn{2}{c}{\includegraphics[width = 0.16\columnwidth]{assets/05-All-BoxPlots/16-G18/Risk/G18-Trust-Product-RISK.png}}
    \end{tabular}
    
    \caption{Guideline 18 participants' ratings for all dependent variables, disaggregated by participants' attitudes toward risk.
	%For the disaggregated data, notice how large the distances between the average rating are when the guideline is applied.
	Table~\ref{tab:G18-Risk-Stats-Appendix} below provides the statistics (where applicable).
}
    \label{fig:Risk-G18-Appendix}
\end{table}

\begin{table}[h]

%\framebox[\linewidth]{For Measuring!}
\centering
\footnotesize

    \begin{tabular}{p{0.22\columnwidth}|c|c|c|c|c|c}
    
    \rowcolor{LightGray}\multicolumn{7}{c}{\textbf{Violation AI Product}}\\
    \hline
    \textbf{Dependent}  & \textbf{Distance b/w} &  &  & & \textbf{Bonferroni} &  \\
    \textbf{variable} & \textbf{Means} &  \textbf{df} &  \textbf{t-val} &   \textbf{p-value}  & \textbf{correction} & \textbf{Cohen's \textit{d}} \\
    \hline
    
    I would feel in control & 1.0680 & 64 &  2.4941 & \cellcolor{AbiOrangeQuote}.0152 & - - - & .6143  \\
    \hline
    
    I would feel secure & - - - & - &  - - - & - - - & - - - & - - - \\
    \hline
    
    I would feel adequate & - - -  & - &  - - - & - - - & - - - & - - - \\
    \hline
    
    I would feel certain & - - - & - &  - - - & - - - & - - - & - - - \\
    \hline
    
    I would feel productive & - - - & - &  - - - & - - - & - - - & - - -   \\
    \hline
    \hline
    
    I perceived it as useful &  - - - & - &  - - - & - - - & - - - & - - -   \\
    \hline
    
    I would not be suspicious & 1.0959 & 64 &  2.6285 & \cellcolor{AbiOrangeQuote}.0107 & - - - & .6483   \\
    \hline
    
    It would not be harmful & - - - & - &  - - - & - - - & - - - & - - -  \\
    \hline
    
    I find the product reliable & - - - & - &  - - - & - - - & - - - & - - - \\
    \hline
    
    I would trust the product & - - - & - &  - - - & - - - & - - - & - - - \\
    \hline

    \rowcolor{LightGray}\multicolumn{7}{c}{\textbf{Application AI Product}}\\
    \hline
    \textbf{Dependent}  & \textbf{Distance b/w} &  &  & & \textbf{Bonferroni} &  \\
    \textbf{variable} & \textbf{Means} &  \textbf{df} &  \textbf{t-val} &   \textbf{p-value}  & \textbf{correction} & \textbf{Cohen's \textit{d}} \\
    \hline
    
    I would feel in control & 1.0074 & 64 &  2.8685 & \cellcolor{AbiOrangeQuote}.0056 & \cellcolor{AbiOrangeQuote}.0336 & .7075  \\
    \hline
    
    I would feel secure & - - - & - &  - - - & - - - & - - - & - - - \\
    \hline
    
    I would feel adequate & - - -  & - &  - - - & - - - & - - - & - - - \\
    \hline
    
    I would feel certain & 0.8125 & 65 &  2.0253 & \cellcolor{AbiOrangeQuote}.0469 & .2814 & .4954 \\
    \hline
    
    I would feel productive & 0.8737 & 64 &  2.6397 & \cellcolor{AbiOrangeQuote}.0104 & .0624 & .6510   \\
    \hline
    \hline
    
    I perceived it as useful &  0.8654 & 64 &  2.8148 & \cellcolor{AbiOrangeQuote}.0065 & .0390 & .6942   \\
    \hline
    
    I would not be suspicious & 1.0341 & 64 &  2.7911 & \cellcolor{AbiOrangeQuote}.0069 & \cellcolor{AbiOrangeQuote}.0414 & .6884   \\
    \hline
    
    It would not be harmful & 0.7917 & 64 &  2.5388 & \cellcolor{AbiOrangeQuote}.0136 & .0816 & .6262  \\
    \hline
    
    I find the product reliable & - - - & - &  - - - & - - - & - - - & - - - \\
    \hline
    
    I would trust the product & - - - & - &  - - - & - - - & - - - & - - -

    \end{tabular}

    \caption{Guideline 18's t-test results %(\checkmark if Welch's t-test) 
    for risk-averse vs. risk-tolerant participants' average ratings of the independent Violation AI product (top) and Application AI product (bottom), for all 10 dependent variables.
    If dashes (- - -) are present, no statistical test was performed.
    If the number of tests exceeded 5 for each product, Bonferroni correction applied by multiplying p-values by the number of tests performed.
    }
    \label{tab:G18-Risk-Stats-Appendix}
\end{table}
\clearpage
%---------------------------------------------------- End Guideline 18
