# Supplementary material for: Measuring User Experience Inclusivity in Human-AI Interaction via Five User Problem-Solving Styles
Source: arXiv:2108.00588 source file (2024-02-17)
Supplement: Supplementary file 11 [file SE-Appendix.tex]

%Guideline 1 ------------------------------
\begin{table}[]
    \centering
    \begin{tabular}{cc|cc|cc|cc|cc}
    \multicolumn{2}{c|}{\includegraphics[width = 0.16\columnwidth]{assets/05-All-BoxPlots/01-G1/SE/G1-Feel-In-Control-SE.png}} &
    \multicolumn{2}{c|}{\includegraphics[width = 0.16\columnwidth]{assets/05-All-BoxPlots/01-G1/SE/G1-Feel-Secure-SE.png}} &
    \multicolumn{2}{c|}{\includegraphics[width = 0.16\columnwidth]{assets/05-All-BoxPlots/01-G1/SE/G1-Feel-Adequate-SE.png}} &
    \multicolumn{2}{c|}{\includegraphics[width = 0.16\columnwidth]{assets/05-All-BoxPlots/01-G1/SE/G1-Feel-Certain-SE.png}} &
    \multicolumn{2}{c}{\includegraphics[width = 0.16\columnwidth]{assets/05-All-BoxPlots/01-G1/SE/G1-Feel-Productive-SE.png}}
    \\
    \hline
    \hline
    \multicolumn{2}{c|}{\includegraphics[width = 0.16\columnwidth]{assets/05-All-BoxPlots/01-G1/SE/G1-Perceived-Useful-SE.png}} &
    \multicolumn{2}{c|}{\includegraphics[width = 0.16\columnwidth]{assets/05-All-BoxPlots/01-G1/SE/G1-Not-Suspicious-SE.png}} &
    \multicolumn{2}{c|}{\includegraphics[width = 0.16\columnwidth]{assets/05-All-BoxPlots/01-G1/SE/G1-Not-Harmful-SE.png}} &
    \multicolumn{2}{c|}{\includegraphics[width = 0.16\columnwidth]{assets/05-All-BoxPlots/01-G1/SE/G1-Product-Reliable-SE.png}} &
    \multicolumn{2}{c}{\includegraphics[width = 0.16\columnwidth]{assets/05-All-BoxPlots/01-G1/SE/G1-Trust-Product-SE.png}}
    \end{tabular}
    
    \caption{Guideline 1 participants' ratings for all dependent variables, disaggregated by participants' computer self-efficacy.
	%For the disaggregated data, notice how large the distances between the average rating are when the guideline is applied.
	Table~\ref{tab:G1-SE-Stats-Appendix} below provides the statistics (where applicable).
}
    \label{fig:SE-G1-Appendix}
\end{table}

\begin{table}[h]

%\framebox[\linewidth]{For Measuring!}
\centering
\footnotesize

    \begin{tabular}{p{0.22\columnwidth}|c|c|c|c|c|c}
    
    \rowcolor{LightGray}\multicolumn{7}{c}{\textbf{Violation AI Product}}\\
    \hline
    \textbf{Dependent}  & \textbf{Distance b/w} &  &  & & \textbf{Bonferroni} &  \\
    \textbf{Variable} & \textbf{Means} &  \textbf{df} &  \textbf{t-val} &   \textbf{p-value}  & \textbf{Correction} & \textbf{Cohen's \textit{d}} \\
    \hline
    
    I would feel in control & - - - & - &  - - - & - - - & - - - & - - -\\
    \hline
    
    I would feel secure & - - - & - &  - - - & - - - & - - - & - - - \\
    \hline
    
    I would feel adequate & 1.3329 & 53 &  3.2383 & \cellcolor{AbiOrangeQuote}.0021 & - - - & 0.8852 \\
    \hline
    
    I would feel certain & - - - & - &  - - - & - - - & - - - & - - - \\
    \hline
    
    I would feel productive & - - - & - &  - - - & - - - & - - - & - - -  \\
    \hline
    \hline
    
    I perceived it as useful &  - - - & - &  - - - & - - - & - - - & - - -  \\
    \hline
    
    I would not be suspicious & - - - & - &  - - - & - - - & - - - & - - -  \\
    \hline
    
    It would not be harmful & - - - & - &  - - - & - - - & - - - & - - -  \\
    \hline
    
    I find the product reliable & - - - & - &  - - - & - - - & - - - & - - -  \\
    \hline
    
    I would trust the product & - - - & - &  - - - & - - - & - - - & - - - \\
    \hline

    \rowcolor{LightGray}\multicolumn{7}{c}{\textbf{Application AI Product}}\\
    \hline
    \textbf{Dependent}  & \textbf{Distance b/w} &  &  & & \textbf{Bonferroni} &  \\
    \textbf{Variable} & \textbf{Means} &  \textbf{df} &  \textbf{t-val} &   \textbf{p-value}  & \textbf{Correction} & \textbf{Cohen's \textit{d}} \\
    \hline
    
    I would feel in control & - - - & - &  - - - & - - - & - - - & - - -  \\
    \hline
    
    I would feel secure & - - - & - &  - - - & - - - & - - - & - - - \\
    \hline
    
    I would feel adequate & 1.2095 & 54 &  3.0073 & \cellcolor{AbiOrangeQuote} .0040 & - - - & 0.8169 \\
    \hline
    
    I would feel certain & - - - & - &  - - - & - - - & - - - & - - - \\
    \hline
    
    I would feel productive & - - - & - &  - - - & - - - & - - - & - - -   \\
    \hline
    \hline
    
    I perceived it as useful &  - - - & - &  - - - & - - - & - - - & - - -  \\
    \hline
    
    I would not be suspicious & - - - & - &  - - - & - - - & - - - & - - -  \\
    \hline
    
    It would not be harmful & 0.8523 & 55 &  2.2688 & \cellcolor{AbiOrangeQuote} .0272 & - - - & 0.6087  \\
    \hline
    
    I find the product reliable & - - - & - &  - - - & - - - & - - - & - - - \\
    \hline
    
    I would trust the product & - - - & - &  - - - & - - - & - - - & - - -

    \end{tabular}

    \caption{Guideline 1's t-test results %(\checkmark if Welch's t-test) 
    for lower self-efficacy vs. higher self-efficacy participants' average ratings of the independent Violation AI product (top) and Application AI product (bottom), for all 10 dependent variables.
    If dashes (- - -) are present, no statistical test was performed.
    If the number of tests exceeded 5 for each product, Bonferroni correction applied by multiplying p-values by the number of tests performed.
    }
    \label{tab:G1-SE-Stats-Appendix}
    
    % \FIXME{MMB@AAA: FYI, I took the \checkmark s out and replaced them with plain text, because the \checkmark vs blank visually stood out so much, I kept mis-seeing it as saying only those 4 rows were signif. or important.\\
    % AAA@MMB: Redid it with Y/N. The Welch's t and t were cluttering up the table too much.\\
    % MMB@AAA: I actually prefer the spelled-out way.  Visually, the table layout now screams WELCHES IS GOOD, and draws attention away from all other columns.  Meta-comment: it might help if you forced yourself to look at this paper with a reader hat on.}

\end{table}

\clearpage
%---------------------------------------------------- End Guideline 1

%Guideline 3 ------------------------------
\begin{table}[]
    \centering
    \begin{tabular}{cc|cc|cc|cc|cc}
    \multicolumn{2}{c|}{\includegraphics[width = 0.16\columnwidth]{assets/05-All-BoxPlots/02-G3/SE/G3-Feel-In-Control-SE.png}} &
    \multicolumn{2}{c|}{\includegraphics[width = 0.16\columnwidth]{assets/05-All-BoxPlots/02-G3/SE/G3-Feel-Secure-SE.png}} &
    \multicolumn{2}{c|}{\includegraphics[width = 0.16\columnwidth]{assets/05-All-BoxPlots/02-G3/SE/G3-Feel-Adequate-SE.png}} &
    \multicolumn{2}{c|}{\includegraphics[width = 0.16\columnwidth]{assets/05-All-BoxPlots/02-G3/SE/G3-Feel-Certain-SE.png}} &
    \multicolumn{2}{c}{\includegraphics[width = 0.16\columnwidth]{assets/05-All-BoxPlots/02-G3/SE/G3-Feel-Productive-SE.png}}
    \\
    \hline
    \hline
    \multicolumn{2}{c|}{\includegraphics[width = 0.16\columnwidth]{assets/05-All-BoxPlots/02-G3/SE/G3-Perceived-Useful-SE.png}} &
    \multicolumn{2}{c|}{\includegraphics[width = 0.16\columnwidth]{assets/05-All-BoxPlots/02-G3/SE/G3-Not-Suspicious-SE.png}} &
    \multicolumn{2}{c|}{\includegraphics[width = 0.16\columnwidth]{assets/05-All-BoxPlots/02-G3/SE/G3-Not-Harmful-SE.png}} &
    \multicolumn{2}{c|}{\includegraphics[width = 0.16\columnwidth]{assets/05-All-BoxPlots/02-G3/SE/G3-Product-Reliable-SE.png}} &
    \multicolumn{2}{c}{\includegraphics[width = 0.16\columnwidth]{assets/05-All-BoxPlots/02-G3/SE/G3-Trust-Product-SE.png}}
    \end{tabular}
    
    \caption{Guideline 3 participants' ratings for all dependent variables, disaggregated by participants' computer self-efficacy.
	%For the disaggregated data, notice how large the distances between the average rating are when the guideline is applied.
	Table~\ref{tab:G3-SE-Stats-Appendix} below provides the statistics (where applicable).
}
    \label{fig:SE-G3-Appendix}
\end{table}

\begin{table}[h]

%\framebox[\linewidth]{For Measuring!}
\centering
\footnotesize

    \begin{tabular}{p{0.22\columnwidth}|c|c|c|c|c|c}
    
    \rowcolor{LightGray}\multicolumn{7}{c}{\textbf{Violation AI Product}}\\
    \hline
    \textbf{Dependent}  & \textbf{Distance b/w} &  &  & & \textbf{Bonferroni} &  \\
    \textbf{Variable} & \textbf{Means} &  \textbf{df} &  \textbf{t-val} &   \textbf{p-value}  & \textbf{Correction} & \textbf{Cohen's \textit{d}} \\
    \hline
    
    I would feel in control & - - - & - &  - - - & - - - & - - - & - - -\\
    \hline
    
    I would feel secure & - - - & - &  - - - & - - - & - - - & - - - \\
    \hline
    
    I would feel adequate & 0.7018 & 66 &  2.1264 & \cellcolor{TimBlueQuote} .0372 & - - - & 0.5193 \\
    \hline
    
    I would feel certain & 0.7789 & 66 &  2.0416 & \cellcolor{TimBlueQuote} .0452 & - - - & 0.4986 \\
    \hline
    
    I would feel productive & - - - & - &  - - - & - - - & - - - & - - -  \\
    \hline
    \hline
    
    I perceived it as useful &  - - - & - &  - - - & - - - & - - - & - - -  \\
    \hline
    
    I would not be suspicious & - - - & - &  - - - & - - - & - - - & - - -  \\
    \hline
    
    It would not be harmful & - - - & - &  - - - & - - - & - - - & - - -  \\
    \hline
    
    I find the product reliable & - - - & - &  - - - & - - - & - - - & - - -  \\
    \hline
    
    I would trust the product & - - - & - &  - - - & - - - & - - - & - - - \\
    \hline

    \rowcolor{LightGray}\multicolumn{7}{c}{\textbf{Application AI Product}}\\
    \hline
    \textbf{Dependent}  & \textbf{Distance b/w} &  &  & & \textbf{Bonferroni} &  \\
    \textbf{Variable} & \textbf{Means} &  \textbf{df} &  \textbf{t-val} &   \textbf{p-value}  & \textbf{Correction} & \textbf{Cohen's \textit{d}} \\
    \hline
    
    I would feel in control & - - - & - &  - - - & - - - & - - - & - - -  \\
    \hline
    
    I would feel secure & - - - & - &  - - - & - - - & - - - & - - - \\
    \hline
    
    I would feel adequate & - - - & - &  - - - & - - - & - - - & - - - \\
    \hline
    
    I would feel certain & - - - & - &  - - - & - - - & - - - & - - - \\
    \hline
    
    I would feel productive & - - - & - &  - - - & - - - & - - - & - - -   \\
    \hline
    \hline
    
    I perceived it as useful &  - - - & - &  - - - & - - - & - - - & - - -  \\
    \hline
    
    I would not be suspicious & - - - & - &  - - - & - - - & - - - & - - -  \\
    \hline
    
    It would not be harmful & 0.5703 & 65 &  1.9770 & .0523 & - - - & 0.4857  \\
    \hline
    
    I find the product reliable & - - - & - &  - - - & - - - & - - - & - - - \\
    \hline
    
    I would trust the product & - - - & - &  - - - & - - - & - - - & - - -

    \end{tabular}

    \caption{Guideline 3's t-test results %(\checkmark if Welch's t-test) 
    for lower self-efficacy vs. higher self-efficacy participants' average ratings of the independent Violation AI product (top) and Application AI product (bottom), for all 10 dependent variables.
    If dashes (- - -) are present, no statistical test was performed.
    If the number of tests exceeded 5 for each product, Bonferroni correction applied by multiplying p-values by the number of tests performed.
    }
    \label{tab:G3-SE-Stats-Appendix}
    
    % \FIXME{MMB@AAA: FYI, I took the \checkmark s out and replaced them with plain text, because the \checkmark vs blank visually stood out so much, I kept mis-seeing it as saying only those 4 rows were signif. or important.\\
    % AAA@MMB: Redid it with Y/N. The Welch's t and t were cluttering up the table too much.\\
    % MMB@AAA: I actually prefer the spelled-out way.  Visually, the table layout now screams WELCHES IS GOOD, and draws attention away from all other columns.  Meta-comment: it might help if you forced yourself to look at this paper with a reader hat on.}

\end{table}

\clearpage
%---------------------------------------------------- End Guideline 3

%Begin Guideline 4----------------------------------------------------

\begin{table}[]
    \centering
    \begin{tabular}{cc|cc|cc|cc|cc}
    \multicolumn{2}{c|}{\includegraphics[width = 0.16\columnwidth]{assets/05-All-BoxPlots/03-G4/SE/G4-Feel-In-Control-SE.png}} &
    \multicolumn{2}{c|}{\includegraphics[width = 0.16\columnwidth]{assets/05-All-BoxPlots/03-G4/SE/G4-Feel-Secure-SE.png}} &
    \multicolumn{2}{c|}{\includegraphics[width = 0.16\columnwidth]{assets/05-All-BoxPlots/03-G4/SE/G4-Feel-Adequate-SE.png}} &
    \multicolumn{2}{c|}{\includegraphics[width = 0.16\columnwidth]{assets/05-All-BoxPlots/03-G4/SE/G4-Feel-Certain-SE.png}} &
    \multicolumn{2}{c}{\includegraphics[width = 0.16\columnwidth]{assets/05-All-BoxPlots/03-G4/SE/G4-Feel-Productive-SE.png}}
    \\
    \hline
    \hline
    \multicolumn{2}{c|}{\includegraphics[width = 0.16\columnwidth]{assets/05-All-BoxPlots/03-G4/SE/G4-Perceived-Useful-SE.png}} &
    \multicolumn{2}{c|}{\includegraphics[width = 0.16\columnwidth]{assets/05-All-BoxPlots/03-G4/SE/G4-Not-Suspicious-SE.png}} &
    \multicolumn{2}{c|}{\includegraphics[width = 0.16\columnwidth]{assets/05-All-BoxPlots/03-G4/SE/G4-Not-Harmful-SE.png}} &
    \multicolumn{2}{c|}{\includegraphics[width = 0.16\columnwidth]{assets/05-All-BoxPlots/03-G4/SE/G4-Product-Reliable-SE.png}} &
    \multicolumn{2}{c}{\includegraphics[width = 0.16\columnwidth]{assets/05-All-BoxPlots/03-G4/SE/G4-Trust-Product-SE.png}}
    \end{tabular}
    
    \caption{Guideline 4 participants' ratings for all dependent variables, disaggregated by participants' computer self-efficacy.
	%For the disaggregated data, notice how large the distances between the average rating are when the guideline is applied.
	Table~\ref{tab:G4-SE-Stats-Appendix} below provides the statistics (where applicable).
}
    \label{fig:SE-G4-Appendix}
\end{table}

\begin{table}[h]

%\framebox[\linewidth]{For Measuring!}
\centering
\footnotesize

    \begin{tabular}{p{0.22\columnwidth}|c|c|c|c|c|c}
    
    \rowcolor{LightGray}\multicolumn{7}{c}{\textbf{Violation AI Product}}\\
    \hline
    \textbf{Dependent}  & \textbf{Distance b/w} &  &  & & \textbf{Bonferroni} &  \\
    \textbf{Variable} & \textbf{Means} &  \textbf{df} &  \textbf{t-val} &   \textbf{p-value}  & \textbf{Correction} & \textbf{Cohen's \textit{d}} \\
    \hline
    
    I would feel in control & - - - & - &  - - - & - - - & - - - & - - -\\
    \hline
    
    I would feel secure & - - - & - &  - - - & - - - & - - - & - - - \\
    \hline
    
    I would feel adequate & 0.6169 & 61 &  2.0218 & \cellcolor{AbiOrangeQuote} .0476 & - - - & 0.5095\\
    \hline
    
    I would feel certain & - - - & - &  - - - & - - - & - - - & - - - \\
    \hline
    
    I would feel productive & - - - & - &  - - - & - - - & - - - & - - - \\
    \hline
    \hline
    
    I perceived it as useful & 0.4882 & 62 &  1.5920 & .1165 & - - - & 0.3988 \\
    \hline
    
    I would not be suspicious & 0.6412 & 62 &  1.7665 & .0822 & - - - & 0.4425  \\
    \hline
    
    It would not be harmful & 0.7932 & 63 &  3.0915 & \cellcolor{AbiOrangeQuote} .0030 & - - - & 0.7677 \\
    \hline
    
    I find the product reliable & - - - & - &  - - - & - - - & - - - & - - -  \\
    \hline
    
    I would trust the product & - - - & - &  - - - & - - - & - - - & - - - \\
    \hline

    \rowcolor{LightGray}\multicolumn{7}{c}{\textbf{Application AI Product}}\\
    \hline
    \textbf{Dependent}  & \textbf{Distance b/w} &  &  & & \textbf{Bonferroni} &  \\
    \textbf{Variable} & \textbf{Means} &  \textbf{df} &  \textbf{t-val} &   \textbf{p-value}  & \textbf{Correction} & \textbf{Cohen's \textit{d}} \\
    \hline
    
    I would feel in control & - - - & - &  - - - & - - - & - - - & - - - \\
    \hline
    
    I would feel secure &- - - & - &  - - - & - - - & - - - & - - - \\
    \hline
    
    I would feel adequate & 0.5220 & 62 &  1.4996 & .1388 & - - - & - - - \\
    \hline
    
    I would feel certain & - - - & - &  - - - & - - - & - - - & - - - \\
    \hline
    
    I would feel productive & - - - & - &  - - - & - - - & - - - & - - - \\
    \hline
    \hline
    
    I perceived it as useful & - - - & - &  - - - & - - - & - - - & - - - \\
    \hline
    
    I would not be suspicious & - - - & - &  - - - & - - - & - - - & - - -  \\
    \hline
    
    It would not be harmful & - - - & - &  - - - & - - - & - - - & - - -  \\
    \hline
    
    I find the product reliable & - - - & - &  - - - & - - - & - - - & - - -\\
    \hline
    
    I would trust the product & - - - & - &  - - - & - - - & - - - & - - -

    \end{tabular}

    \caption{Guideline 4's t-test results %(\checkmark if Welch's t-test) 
    for lower self-efficacy vs. higher self-efficacy participants' average ratings of the independent Violation AI product (top) and Application AI product (bottom), for all 10 dependent variables.
    If dashes (- - -) are present, no statistical test was performed.
    If the number of tests exceeded 5 for each product, Bonferroni correction applied by multiplying p-values by the number of tests performed.
    }
    \label{tab:G4-SE-Stats-Appendix}
\end{table}

%---------------------------------------------------- End Guideline 4

\clearpage

%Begin Guideline 5----------------------------------------------------

\begin{table}[]
    \centering
    \begin{tabular}{cc|cc|cc|cc|cc}
    \multicolumn{2}{c|}{\includegraphics[width = 0.16\columnwidth]{assets/05-All-BoxPlots/04-G5/SE/G5-Feel-In-Control-SE.png}} &
    \multicolumn{2}{c|}{\includegraphics[width = 0.16\columnwidth]{assets/05-All-BoxPlots/04-G5/SE/G5-Feel-Secure-SE.png}} &
    \multicolumn{2}{c|}{\includegraphics[width = 0.16\columnwidth]{assets/05-All-BoxPlots/04-G5/SE/G5-Feel-Adequate-SE.png}} &
    \multicolumn{2}{c|}{\includegraphics[width = 0.16\columnwidth]{assets/05-All-BoxPlots/04-G5/SE/G5-Feel-Certain-SE.png}} &
    \multicolumn{2}{c}{\includegraphics[width = 0.16\columnwidth]{assets/05-All-BoxPlots/04-G5/SE/G5-Feel-Productive-SE.png}}
    \\
    \hline
    \hline
    \multicolumn{2}{c|}{\includegraphics[width = 0.16\columnwidth]{assets/05-All-BoxPlots/04-G5/SE/G5-Perceived-Useful-SE.png}} &
    \multicolumn{2}{c|}{\includegraphics[width = 0.16\columnwidth]{assets/05-All-BoxPlots/04-G5/SE/G5-Not-Suspicious-SE.png}} &
    \multicolumn{2}{c|}{\includegraphics[width = 0.16\columnwidth]{assets/05-All-BoxPlots/04-G5/SE/G5-Not-Harmful-SE.png}} &
    \multicolumn{2}{c|}{\includegraphics[width = 0.16\columnwidth]{assets/05-All-BoxPlots/04-G5/SE/G5-Product-Reliable-SE.png}} &
    \multicolumn{2}{c}{\includegraphics[width = 0.16\columnwidth]{assets/05-All-BoxPlots/04-G5/SE/G5-Trust-Product-SE.png}}
    \end{tabular}
    
    \caption{Guideline 5 participants' ratings for all dependent variables, disaggregated by participants' computer self-efficacy.
	%For the disaggregated data, notice how large the distances between the average rating are when the guideline is applied.
	Table~\ref{tab:G5-SE-Stats-Appendix} below provides the statistics (where applicable).
}
    \label{fig:SE-G5-Appendix}
\end{table}

\begin{table}[h]

%\framebox[\linewidth]{For Measuring!}
\centering
\footnotesize

    \begin{tabular}{p{0.22\columnwidth}|c|c|c|c|c|c}
    
    \rowcolor{LightGray}\multicolumn{7}{c}{\textbf{Violation AI Product}}\\
    \hline
    \textbf{Dependent}  & \textbf{Distance b/w} &  &  & & \textbf{Bonferroni} &  \\
    \textbf{Variable} & \textbf{Means} &  \textbf{df} &  \textbf{t-val} &   \textbf{p-value}  & \textbf{Correction} & \textbf{Cohen's \textit{d}} \\
    \hline
    
    I would feel in control & 0.9273 & 66 &  2.2879 & \cellcolor{AbiOrangeQuote}.0254 & - - - & 0.5551 \\
    \hline
    
    I would feel secure & 0.8918 & 67 &  2.2141 & \cellcolor{AbiOrangeQuote}.0302 & - - - & 0.5336 \\
    \hline
    
    I would feel adequate & - - - & - &  - - - & - - - & - - - & - - - \\
    \hline
    
    I would feel certain & - - - & - &  - - - & - - - & - - - & - - - \\
    \hline
    
    I would feel productive & - - - & - &  - - - & - - - & - - - & - - -  \\
    \hline
    \hline
    
    I perceived it as useful &  - - - & - &  - - - & - - - & - - - & - - -  \\
    \hline
    
    I would not be suspicious & - - - & - &  - - - & - - - & - - - & - - -  \\
    \hline
    
    It would not be harmful & - - - & - &  - - - & - - - & - - - & - - -  \\
    \hline
    
    I find the product reliable & 0.6540 & 67 &  2.1192 & \cellcolor{AbiOrangeQuote}.0378 & - - - & 0.5107  \\
    \hline
    
    I would trust the product & 0.7778 & 67 &  2.1553 & \cellcolor{AbiOrangeQuote}.0347 & - - -  & 0.5194 \\
    \hline

    \rowcolor{LightGray}\multicolumn{7}{c}{\textbf{Application AI Product}}\\
    \hline
    \textbf{Dependent}  & \textbf{Distance b/w} &  &  & & \textbf{Bonferroni} &  \\
    \textbf{Variable} & \textbf{Means} &  \textbf{df} &  \textbf{t-val} &   \textbf{p-value}  & \textbf{Correction} & \textbf{Cohen's \textit{d}} \\
    \hline
    
    I would feel in control & 0.8918 & 66 & 2.2832 & \cellcolor{AbiOrangeQuote}.0256 & - - - & 0.5540  \\
    \hline
    
    I would feel secure & 0.7004 & 66 &  2.0573 & \cellcolor{AbiOrangeQuote}.0436 & - - - & 0.4992- \\
    \hline
    
    I would feel adequate & - - - & - &  - - - & - - - & - - - & - - - \\
    \hline
    
    I would feel certain & - - - & - &  - - - & - - - & - - - & - - - \\
    \hline
    
    I would feel productive & - - - & - &  - - - & - - - & - - - & - - -    \\
    \hline
    \hline
    
    I perceived it as useful &  - - - & - &  - - - & - - - & - - - & - - -   \\
    \hline
    
    I would not be suspicious & - - - & - &  - - - & - - - & - - - & - - -   \\
    \hline
    
    It would not be harmful & - - - & - &  - - - & - - - & - - - & - - -  \\
    \hline
    
    I find the product reliable & 0.7222 & 67 &  2.1691 & \cellcolor{AbiOrangeQuote} .0336 & - - - & 0.5227 \\
    \hline
    
    I would trust the product & 0.6919 & 67 &  2.2593 & \cellcolor{AbiOrangeQuote} .0271 & - - - & 0.5445

    \end{tabular}

    \caption{Guideline 5's t-test results %(\checkmark if Welch's t-test) 
    for lower self-efficacy vs. higher self-efficacy participants' average ratings of the independent Violation AI product (top) and Application AI product (bottom), for all 10 dependent variables.
    If dashes (- - -) are present, no statistical test was performed.
    If the number of tests exceeded 5 for each product, Bonferroni correction applied by multiplying p-values by the number of tests performed.
    }
    \label{tab:G5-SE-Stats-Appendix}
\end{table}

%---------------------------------------------------- End Guideline 5

\clearpage

%Begin Guideline 6----------------------------------------------------

\begin{table}[]
    \centering
    \begin{tabular}{cc|cc|cc|cc|cc}
    \multicolumn{2}{c|}{\includegraphics[width = 0.16\columnwidth]{assets/05-All-BoxPlots/05-G6/SE/G6-Feel-In-Control-SE.png}} &
    \multicolumn{2}{c|}{\includegraphics[width = 0.16\columnwidth]{assets/05-All-BoxPlots/05-G6/SE/G6-Feel-Secure-SE.png}} &
    \multicolumn{2}{c|}{\includegraphics[width = 0.16\columnwidth]{assets/05-All-BoxPlots/05-G6/SE/G6-Feel-Adequate-SE.png}} &
    \multicolumn{2}{c|}{\includegraphics[width = 0.16\columnwidth]{assets/05-All-BoxPlots/05-G6/SE/G6-Feel-Certain-SE.png}} &
    \multicolumn{2}{c}{\includegraphics[width = 0.16\columnwidth]{assets/05-All-BoxPlots/05-G6/SE/G6-Feel-Productive-SE.png}}
    \\
    \hline
    \hline
    \multicolumn{2}{c|}{\includegraphics[width = 0.16\columnwidth]{assets/05-All-BoxPlots/05-G6/SE/G6-Perceived-Useful-SE.png}} &
    \multicolumn{2}{c|}{\includegraphics[width = 0.16\columnwidth]{assets/05-All-BoxPlots/05-G6/SE/G6-Not-Suspicious-SE.png}} &
    \multicolumn{2}{c|}{\includegraphics[width = 0.16\columnwidth]{assets/05-All-BoxPlots/05-G6/SE/G6-Not-Harmful-SE.png}} &
    \multicolumn{2}{c|}{\includegraphics[width = 0.16\columnwidth]{assets/05-All-BoxPlots/05-G6/SE/G6-Product-Reliable-SE.png}} &
    \multicolumn{2}{c}{\includegraphics[width = 0.16\columnwidth]{assets/05-All-BoxPlots/05-G6/SE/G6-Trust-Product-SE.png}}
    \end{tabular}
    
    \caption{Guideline 6 participants' ratings for all dependent variables, disaggregated by participants' computer self-efficacy.
	%For the disaggregated data, notice how large the distances between the average rating are when the guideline is applied.
	Table~\ref{tab:G6-SE-Stats-Appendix} below provides the statistics (where applicable).
}
    \label{fig:SE-G6-Appendix}
\end{table}

\begin{table}[h]

%\framebox[\linewidth]{For Measuring!}
\centering
\footnotesize

    \begin{tabular}{p{0.22\columnwidth}|c|c|c|c|c|c}
    
    \rowcolor{LightGray}\multicolumn{7}{c}{\textbf{Violation AI Product}}\\
    \hline
    \textbf{Dependent}  & \textbf{Distance b/w} &  &  & & \textbf{Bonferroni} &  \\
    \textbf{Variable} & \textbf{Means} &  \textbf{df} &  \textbf{t-val} &   \textbf{p-value}  & \textbf{Correction} & \textbf{Cohen's \textit{d}} \\
    \hline
    
    I would feel in control & - - - & - &  - - - & - - - & - - - & - - -  \\
    \hline
    
    I would feel secure & - - - & - &  - - - & - - - & - - - & - - - \\
    \hline
    
    I would feel adequate & - - - & - &  - - - & - - - & - - - & - - - \\
    \hline
    
    I would feel certain & 0.6588 & 62 &  1.8517 & .0688 & - - - & 0.4638 \\
    \hline
    
    I would feel productive & - - - & - &  - - - & - - - & - - - & - - -    \\
    \hline
    \hline
    
    I perceived it as useful &  - - - & - &  - - - & - - - & - - - & - - -   \\
    \hline
    
    I would not be suspicious & - - - & - &  - - - & - - - & - - - & - - -   \\
    \hline
    
    It would not be harmful & - - - & - &  - - - & - - - & - - - & - - -  \\
    \hline
    
    I find the product reliable & - - - & - &  - - - & - - - & - - - & - - - \\
    \hline
    
    I would trust the product & - - - & - &  - - - & - - - & - - - & - - - \\
    \hline

    \rowcolor{LightGray}\multicolumn{7}{c}{\textbf{Application AI Product}}\\
    \hline
    \textbf{Dependent}  & \textbf{Distance b/w} &  &  & & \textbf{Bonferroni} &  \\
    \textbf{Variable} & \textbf{Means} &  \textbf{df} &  \textbf{t-val} &   \textbf{p-value}  & \textbf{Correction} & \textbf{Cohen's \textit{d}} \\
    \hline
    
    I would feel in control & - - - & - &  - - - & - - - & - - - & - - -  \\
    \hline
    
    I would feel secure & - - - & - &  - - - & - - - & - - - & - - - \\
    \hline
    
    I would feel adequate & - - - & - &  - - - & - - - & - - - & - - - \\
    \hline
    
    I would feel certain & - - - & - &  - - - & - - - & - - - & - - - \\
    \hline
    
    I would feel productive & - - - & - &  - - - & - - - & - - - & - - -    \\
    \hline
    \hline
    
    I perceived it as useful &  - - - & - &  - - - & - - - & - - - & - - -   \\
    \hline
    
    I would not be suspicious & - - - & - &  - - - & - - - & - - - & - - -   \\
    \hline
    
    It would not be harmful & - - - & - &  - - - & - - - & - - - & - - -  \\
    \hline
    
    I find the product reliable & 0.3499 & 61 &  0.9563 & .3427 & - - - & 0.2417\\
    \hline
    
    I would trust the product & 0.4745 & 62 &  1.2821 & .2046 & - - - & 0.3212

    \end{tabular}

    \caption{Guideline 6's t-test results %(\checkmark if Welch's t-test) 
    for lower self-efficacy vs. higher self-efficacy participants' average ratings of the independent Violation AI product (top) and Application AI product (bottom), for all 10 dependent variables.
    If dashes (- - -) are present, no statistical test was performed.
    If the number of tests exceeded 5 for each product, Bonferroni correction applied by multiplying p-values by the number of tests performed.
    }
    \label{tab:G6-SE-Stats-Appendix}
\end{table}

%---------------------------------------------------- End Guideline 6

\clearpage

%Begin Guideline 7----------------------------------------------------

\begin{table}[]
    \centering
    \begin{tabular}{cc|cc|cc|cc|cc}
    \multicolumn{2}{c|}{\includegraphics[width = 0.16\columnwidth]{assets/05-All-BoxPlots/06-G7/SE/G7-Feel-In-Control-SE.png}} &
    \multicolumn{2}{c|}{\includegraphics[width = 0.16\columnwidth]{assets/05-All-BoxPlots/06-G7/SE/G7-Feel-Secure-SE.png}} &
    \multicolumn{2}{c|}{\includegraphics[width = 0.16\columnwidth]{assets/05-All-BoxPlots/06-G7/SE/G7-Feel-Adequate-SE.png}} &
    \multicolumn{2}{c|}{\includegraphics[width = 0.16\columnwidth]{assets/05-All-BoxPlots/06-G7/SE/G7-Feel-Certain-SE.png}} &
    \multicolumn{2}{c}{\includegraphics[width = 0.16\columnwidth]{assets/05-All-BoxPlots/06-G7/SE/G7-Feel-Productive-SE.png}}
    \\
    \hline
    \hline
    \multicolumn{2}{c|}{\includegraphics[width = 0.16\columnwidth]{assets/05-All-BoxPlots/06-G7/SE/G7-Perceived-Useful-SE.png}} &
    \multicolumn{2}{c|}{\includegraphics[width = 0.16\columnwidth]{assets/05-All-BoxPlots/06-G7/SE/G7-Not-Suspicious-SE.png}} &
    \multicolumn{2}{c|}{\includegraphics[width = 0.16\columnwidth]{assets/05-All-BoxPlots/06-G7/SE/G7-Not-Harmful-SE.png}} &
    \multicolumn{2}{c|}{\includegraphics[width = 0.16\columnwidth]{assets/05-All-BoxPlots/06-G7/SE/G7-Product-Reliable-SE.png}} &
    \multicolumn{2}{c}{\includegraphics[width = 0.16\columnwidth]{assets/05-All-BoxPlots/06-G7/SE/G7-Trust-Product-SE.png}}
    \end{tabular}
    
    \caption{Guideline 7 participants' ratings for all dependent variables, disaggregated by participants' computer self-efficacy.
	%For the disaggregated data, notice how large the distances between the average rating are when the guideline is applied.
	Table~\ref{tab:G7-SE-Stats-Appendix} below provides the statistics (where applicable).
}
    \label{fig:SE-G7-Appendix}
\end{table}

\begin{table}[h]

%\framebox[\linewidth]{For Measuring!}
\centering
\footnotesize

    \begin{tabular}{p{0.22\columnwidth}|c|c|c|c|c|c}
    
    \rowcolor{LightGray}\multicolumn{7}{c}{\textbf{Violation AI Product}}\\
    \hline
    \textbf{Dependent}  & \textbf{Distance b/w} &  &  & & \textbf{Bonferroni} &  \\
    \textbf{Variable} & \textbf{Means} &  \textbf{df} &  \textbf{t-val} &   \textbf{p-value}  & \textbf{Correction} & \textbf{Cohen's \textit{d}} \\
    \hline
    
    I would feel in control & - - - & - &  - - - & - - - & - - - & - - - \\
    \hline
    
    I would feel secure & - - - & - &  - - - & - - - & - - - & - - - \\
    \hline
    
    I would feel adequate & - - - & - &  - - - & - - - & - - - & - - - \\
    \hline
    
    I would feel certain & - - - & - &  - - - & - - - & - - - & - - - \\
    \hline
    
    I would feel productive & - - - & - &  - - - & - - - & - - - & - - -  \\
    \hline
    \hline
    
    I perceived it as useful &  - - - & - &  - - - & - - - & - - - & - - -  \\
    \hline
    
    I would not be suspicious & - - - & - &  - - - & - - - & - - - & - - -  \\
    \hline
    
    It would not be harmful & - - - & - &  - - - & - - - & - - - & - - -  \\
    \hline
    
    I find the product reliable & - - - & - &  - - - & - - - & - - - & - - -  \\
    \hline
    
    I would trust the product & - - - & - &  - - - & - - - & - - - & - - - \\
    \hline

    \rowcolor{LightGray}\multicolumn{7}{c}{\textbf{Application AI Product}}\\
    \hline
    \textbf{Dependent}  & \textbf{Distance b/w} &  &  & & \textbf{Bonferroni} &  \\
    \textbf{Variable} & \textbf{Means} &  \textbf{df} &  \textbf{t-val} &   \textbf{p-value}  & \textbf{Correction} & \textbf{Cohen's \textit{d}} \\
    \hline
    
    I would feel in control & 0.4543 & - &  - - - & - - - & - - - & - - -  \\
    \hline
    
    I would feel secure & - - - & - &  - - - & - - - & - - - & - - - \\
    \hline
    
    I would feel adequate & - - -  & - &  - - - & - - - & - - - & - - - \\
    \hline
    
    I would feel certain & - - - & - &  - - - & - - - & - - - & - - - \\
    \hline
    
    I would feel productive & - - - & - &  - - - & - - - & - - - & - - -    \\
    \hline
    \hline
    
    I perceived it as useful &  0.3929 & 56 &  1.2052 & .2332 & - - - & 0.3167   \\
    \hline
    
    I would not be suspicious & - - - & - &  - - - & - - - & - - - & - - -   \\
    \hline
    
    It would not be harmful & 0.5476 & 56 &  2.0238 & \cellcolor{AbiOrangeQuote}.0477 & - - - & 0.5318  \\
    \hline
    
    I find the product reliable & - - - & - &  - - - & - - - & - - - & - - - \\
    \hline
    
    I would trust the product & - - - & - &  - - - & - - - & - - - & - - -

    \end{tabular}

    \caption{Guideline 7's t-test results %(\checkmark if Welch's t-test) 
    for lower self-efficacy vs. higher self-efficacy participants' average ratings of the independent Violation AI product (top) and Application AI product (bottom), for all 10 dependent variables.
    If dashes (- - -) are present, no statistical test was performed.
    If the number of tests exceeded 5 for each product, Bonferroni correction applied by multiplying p-values by the number of tests performed.
    }
    \label{tab:G7-SE-Stats-Appendix}
\end{table}

%---------------------------------------------------- End Guideline 7

\clearpage

%Begin Guideline 8----------------------------------------------------

\begin{table}[]
    \centering
    \begin{tabular}{cc|cc|cc|cc|cc}
    \multicolumn{2}{c|}{\includegraphics[width = 0.16\columnwidth]{assets/05-All-BoxPlots/07-G8/SE/G8-Feel-In-Control-SE.png}} &
    \multicolumn{2}{c|}{\includegraphics[width = 0.16\columnwidth]{assets/05-All-BoxPlots/07-G8/SE/G8-Feel-Secure-SE.png}} &
    \multicolumn{2}{c|}{\includegraphics[width = 0.16\columnwidth]{assets/05-All-BoxPlots/07-G8/SE/G8-Feel-Adequate-SE.png}} &
    \multicolumn{2}{c|}{\includegraphics[width = 0.16\columnwidth]{assets/05-All-BoxPlots/07-G8/SE/G8-Feel-Certain-SE.png}} &
    \multicolumn{2}{c}{\includegraphics[width = 0.16\columnwidth]{assets/05-All-BoxPlots/07-G8/SE/G8-Feel-Productive-SE.png}}
    \\
    \hline
    \hline
    \multicolumn{2}{c|}{\includegraphics[width = 0.16\columnwidth]{assets/05-All-BoxPlots/07-G8/SE/G8-Perceived-Useful-SE.png}} &
    \multicolumn{2}{c|}{\includegraphics[width = 0.16\columnwidth]{assets/05-All-BoxPlots/07-G8/SE/G8-Not-Suspicious-SE.png}} &
    \multicolumn{2}{c|}{\includegraphics[width = 0.16\columnwidth]{assets/05-All-BoxPlots/07-G8/SE/G8-Not-Harmful-SE.png}} &
    \multicolumn{2}{c|}{\includegraphics[width = 0.16\columnwidth]{assets/05-All-BoxPlots/07-G8/SE/G8-Product-Reliable-SE.png}} &
    \multicolumn{2}{c}{\includegraphics[width = 0.16\columnwidth]{assets/05-All-BoxPlots/07-G8/SE/G8-Trust-Product-SE.png}}
    \end{tabular}
    
    \caption{Guideline 8 participants' ratings for all dependent variables, disaggregated by participants' computer self-efficacy.
	%For the disaggregated data, notice how large the distances between the average rating are when the guideline is applied.
	Table~\ref{tab:G8-SE-Stats-Appendix} below provides the statistics (where applicable).
}
    \label{fig:SE-G8-Appendix}
\end{table}

\begin{table}[h]

%\framebox[\linewidth]{For Measuring!}
\centering
\footnotesize

    \begin{tabular}{p{0.22\columnwidth}|c|c|c|c|c|c}
    
    \rowcolor{LightGray}\multicolumn{7}{c}{\textbf{Violation AI Product}}\\
    \hline
    \textbf{Dependent}  & \textbf{Distance b/w} &  &  & & \textbf{Bonferroni} &  \\
    \textbf{Variable} & \textbf{Means} &  \textbf{df} &  \textbf{t-val} &   \textbf{p-value}  & \textbf{Correction} & \textbf{Cohen's \textit{d}} \\
    \hline
    
    I would feel in control & - - - & - &  - - - & - - - & - - - & - - - \\
    \hline
    
    I would feel secure & - - - & - &  - - - & - - - & - - - & - - - \\
    \hline
    
    I would feel adequate & - - - & - &  - - - & - - - & - - - & - - - \\
    \hline
    
    I would feel certain & - - - & - &  - - - & - - - & - - - & - - - \\
    \hline
    
    I would feel productive & - - - & - &  - - - & - - - & - - - & - - -  \\
    \hline
    \hline
    
    I perceived it as useful &  - - - & - &  - - - & - - - & - - - & - - -  \\
    \hline
    
    I would not be suspicious & - - - & - &  - - - & - - - & - - - & - - - \\
    \hline
    
    It would not be harmful & - - - & - &  - - - & - - - & - - - & - - -  \\
    \hline
    
    I find the product reliable & - - - & - &  - - - & - - - & - - - & - - -  \\
    \hline
    
    I would trust the product & - - - & - &  - - - & - - - & - - - & - - - \\
    \hline

    \rowcolor{LightGray}\multicolumn{7}{c}{\textbf{Application AI Product}}\\
    \hline
    \textbf{Dependent}  & \textbf{Distance b/w} &  &  & & \textbf{Bonferroni} &  \\
    \textbf{Variable} & \textbf{Means} &  \textbf{df} &  \textbf{t-val} &   \textbf{p-value}  & \textbf{Correction} & \textbf{Cohen's \textit{d}} \\
    \hline
    
    I would feel in control & - - -& - &  - - - & - - - & - - - & - - -  \\
    \hline
    
    I would feel secure & - - - & - &  - - - & - - - & - - - & - - - \\
    \hline
    
    I would feel adequate & - - -  & - &  - - - & - - - & - - - & - - - \\
    \hline
    
    I would feel certain & - - - & - &  - - - & - - - & - - - & - - - \\
    \hline
    
    I would feel productive & - - - & - &  - - - & - - - & - - - & - - -    \\
    \hline
    \hline
    
    I perceived it as useful &  - - - & - &  - - - & - - - & - - - & - - -   \\
    \hline
    
    I would not be suspicious & - - - & - &  - - - & - - - & - - - & - - -   \\
    \hline
    
    It would not be harmful & - - - & - &  - - - & - - - & - - - & - - -  \\
    \hline
    
    I find the product reliable & - - - & - &  - - - & - - - & - - - & - - - \\
    \hline
    
    I would trust the product & - - - & - &  - - - & - - - & - - - & - - -

    \end{tabular}

    \caption{Guideline 8's t-test results %(\checkmark if Welch's t-test) 
    for lower self-efficacy vs. higher self-efficacy participants' average ratings of the independent Violation AI product (top) and Application AI product (bottom), for all 10 dependent variables.
    If dashes (- - -) are present, no statistical test was performed.
    If the number of tests exceeded 5 for each product, Bonferroni correction applied by multiplying p-values by the number of tests performed.
    }
    \label{tab:G8-SE-Stats-Appendix}
\end{table}
\clearpage
%---------------------------------------------------- End Guideline 8

%Begin Guideline 9----------------------------------------------------

\begin{table}[]
    \centering
    \begin{tabular}{cc|cc|cc|cc|cc}
    \multicolumn{2}{c|}{\includegraphics[width = 0.16\columnwidth]{assets/05-All-BoxPlots/08-G9/SE/G9-Feel-In-Control-SE.png}} &
    \multicolumn{2}{c|}{\includegraphics[width = 0.16\columnwidth]{assets/05-All-BoxPlots/08-G9/SE/G9-Feel-Secure-SE.png}} &
    \multicolumn{2}{c|}{\includegraphics[width = 0.16\columnwidth]{assets/05-All-BoxPlots/08-G9/SE/G9-Feel-Adequate-SE.png}} &
    \multicolumn{2}{c|}{\includegraphics[width = 0.16\columnwidth]{assets/05-All-BoxPlots/08-G9/SE/G9-Feel-Certain-SE.png}} &
    \multicolumn{2}{c}{\includegraphics[width = 0.16\columnwidth]{assets/05-All-BoxPlots/08-G9/SE/G9-Feel-Productive-SE.png}}
    \\
    \hline
    \hline
    \multicolumn{2}{c|}{\includegraphics[width = 0.16\columnwidth]{assets/05-All-BoxPlots/08-G9/SE/G9-Perceived-Useful-SE.png}} &
    \multicolumn{2}{c|}{\includegraphics[width = 0.16\columnwidth]{assets/05-All-BoxPlots/08-G9/SE/G9-Not-Suspicious-SE.png}} &
    \multicolumn{2}{c|}{\includegraphics[width = 0.16\columnwidth]{assets/05-All-BoxPlots/08-G9/SE/G9-Not-Harmful-SE.png}} &
    \multicolumn{2}{c|}{\includegraphics[width = 0.16\columnwidth]{assets/05-All-BoxPlots/08-G9/SE/G9-Product-Reliable-SE.png}} &
    \multicolumn{2}{c}{\includegraphics[width = 0.16\columnwidth]{assets/05-All-BoxPlots/08-G9/SE/G9-Trust-Product-SE.png}}
    \end{tabular}
    
    \caption{Guideline 9 participants' ratings for all dependent variables, disaggregated by participants' computer self-efficacy.
	%For the disaggregated data, notice how large the distances between the average rating are when the guideline is applied.
	Table~\ref{tab:G9-SE-Stats-Appendix} below provides the statistics (where applicable).
}
    \label{fig:SE-G9-Appendix}
\end{table}

\begin{table}[h]

%\framebox[\linewidth]{For Measuring!}
\centering
\footnotesize

    \begin{tabular}{p{0.22\columnwidth}|c|c|c|c|c|c}
    
    \rowcolor{LightGray}\multicolumn{7}{c}{\textbf{Violation AI Product}}\\
    \hline
    \textbf{Dependent}  & \textbf{Distance b/w} &  &  & & \textbf{Bonferroni} &  \\
    \textbf{Variable} & \textbf{Means} &  \textbf{df} &  \textbf{t-val} &   \textbf{p-value}  & \textbf{Correction} & \textbf{Cohen's \textit{d}} \\
    \hline
    
    I would feel in control & - - - & - &  - - - & - - - & - - - & - - - \\
    \hline
    
    I would feel secure & - - - & - &  - - - & - - - & - - - & - - - \\
    \hline
    
    I would feel adequate & - - - & - &  - - - & - - - & - - - & - - - \\
    \hline
    
    I would feel certain & - - - & - &  - - - & - - - & - - - & - - - \\
    \hline
    
    I would feel productive & - - - & - &  - - - & - - - & - - - & - - -  \\
    \hline
    \hline
    
    I perceived it as useful &  - - - & - &  - - - & - - - & - - - & - - -  \\
    \hline
    
    I would not be suspicious & - - - & - &  - - - & - - - & - - - & - - - \\
    \hline
    
    It would not be harmful & - - - & - &  - - - & - - - & - - - & - - -  \\
    \hline
    
    I find the product reliable & - - - & - &  - - - & - - - & - - - & - - -  \\
    \hline
    
    I would trust the product & - - - & - &  - - - & - - - & - - - & - - - \\
    \hline

    \rowcolor{LightGray}\multicolumn{7}{c}{\textbf{Application AI Product}}\\
    \hline
    \textbf{Dependent}  & \textbf{Distance b/w} &  &  & & \textbf{Bonferroni} &  \\
    \textbf{Variable} & \textbf{Means} &  \textbf{df} &  \textbf{t-val} &   \textbf{p-value}  & \textbf{Correction} & \textbf{Cohen's \textit{d}} \\
    \hline
    
    I would feel in control & - - - & - &  - - - & - - - & - - - & - - -  \\
    \hline
    
    I would feel secure & - - - & - &  - - - & - - - & - - - & - - - \\
    \hline
    
    I would feel adequate & - - -  & - &  - - - & - - - & - - - & - - - \\
    \hline
    
    I would feel certain & - - - & - &  - - - & - - - & - - - & - - - \\
    \hline
    
    I would feel productive & 0.8776 & 56 &  2.7919 & \cellcolor{AbiOrangeQuote}.0072 & - - - & 0.7403    \\
    \hline
    \hline
    
    I perceived it as useful &  0.6388 & 56 &  2.0670 & \cellcolor{AbiOrangeQuote}.0434 & - - - & 0.5481   \\
    \hline
    
    I would not be suspicious & - - - & - &  - - - & - - - & - - - & - - -   \\
    \hline
    
    It would not be harmful & - - - & - &  - - - & - - - & - - - & - - -  \\
    \hline
    
    I find the product reliable & - - - & - &  - - - & - - - & - - - & - - - \\
    \hline
    
    I would trust the product & 1.0255 & 53 &  3.0015 & \cellcolor{AbiOrangeQuote}.0041 & - - - & 0.8161

    \end{tabular}

    \caption{Guideline 9's t-test results %(\checkmark if Welch's t-test) 
    for lower self-efficacy vs. higher self-efficacy participants' average ratings of the independent Violation AI product (top) and Application AI product (bottom), for all 10 dependent variables.
    If dashes (- - -) are present, no statistical test was performed.
    If the number of tests exceeded 5 for each product, Bonferroni correction applied by multiplying p-values by the number of tests performed.
    }
    \label{tab:G9-SE-Stats-Appendix}
\end{table}
\clearpage
%---------------------------------------------------- End Guideline 9

%Begin Guideline 10----------------------------------------------------

\begin{table}[]
    \centering
    \begin{tabular}{cc|cc|cc|cc|cc}
    \multicolumn{2}{c|}{\includegraphics[width = 0.16\columnwidth]{assets/05-All-BoxPlots/09-G10/SE/G10-Feel-In-Control-SE.png}} &
    \multicolumn{2}{c|}{\includegraphics[width = 0.16\columnwidth]{assets/05-All-BoxPlots/09-G10/SE/G10-Feel-Secure-SE.png}} &
    \multicolumn{2}{c|}{\includegraphics[width = 0.16\columnwidth]{assets/05-All-BoxPlots/09-G10/SE/G10-Feel-Adequate-SE.png}} &
    \multicolumn{2}{c|}{\includegraphics[width = 0.16\columnwidth]{assets/05-All-BoxPlots/09-G10/SE/G10-Feel-Certain-SE.png}} &
    \multicolumn{2}{c}{\includegraphics[width = 0.16\columnwidth]{assets/05-All-BoxPlots/09-G10/SE/G10-Feel-Productive-SE.png}}
    \\
    \hline
    \hline
    \multicolumn{2}{c|}{\includegraphics[width = 0.16\columnwidth]{assets/05-All-BoxPlots/09-G10/SE/G10-Perceived-Useful-SE.png}} &
    \multicolumn{2}{c|}{\includegraphics[width = 0.16\columnwidth]{assets/05-All-BoxPlots/09-G10/SE/G10-Not-Suspicious-SE.png}} &
    \multicolumn{2}{c|}{\includegraphics[width = 0.16\columnwidth]{assets/05-All-BoxPlots/09-G10/SE/G10-Not-Harmful-SE.png}} &
    \multicolumn{2}{c|}{\includegraphics[width = 0.16\columnwidth]{assets/05-All-BoxPlots/09-G10/SE/G10-Product-Reliable-SE.png}} &
    \multicolumn{2}{c}{\includegraphics[width = 0.16\columnwidth]{assets/05-All-BoxPlots/09-G10/SE/G10-Trust-Product-SE.png}}
    \end{tabular}
    
    \caption{Guideline 10 participants' ratings for all dependent variables, disaggregated by participants' computer self-efficacy.
	%For the disaggregated data, notice how large the distances between the average rating are when the guideline is applied.
	Table~\ref{tab:G10-SE-Stats-Appendix} below provides the statistics (where applicable).
}
    \label{fig:SE-G10-Appendix}
\end{table}

\begin{table}[h]

%\framebox[\linewidth]{For Measuring!}
\centering
\footnotesize

    \begin{tabular}{p{0.22\columnwidth}|c|c|c|c|c|c}
    
    \rowcolor{LightGray}\multicolumn{7}{c}{\textbf{Violation AI Product}}\\
    \hline
    \textbf{Dependent}  & \textbf{Distance b/w} &  &  & & \textbf{Bonferroni} &  \\
    \textbf{Variable} & \textbf{Means} &  \textbf{df} &  \textbf{t-val} &   \textbf{p-value}  & \textbf{Correction} & \textbf{Cohen's \textit{d}} \\
    \hline
    
    I would feel in control & - - - & - &  - - - & - - - & - - - & - - - \\
    \hline
    
    I would feel secure & - - - & - &  - - - & - - - & - - - & - - - \\
    \hline
    
    I would feel adequate & - - - & - &  - - - & - - - & - - - & - - - \\
    \hline
    
    I would feel certain & - - - & - &  - - - & - - - & - - - & - - - \\
    \hline
    
    I would feel productive & - - - & - &  - - - & - - - & - - - & - - -  \\
    \hline
    \hline
    
    I perceived it as useful &  - - - & - &  - - - & - - - & - - - & - - -  \\
    \hline
    
    I would not be suspicious & 1.112 & 63 &  2.2902 & \cellcolor{AbiOrangeQuote}.0254 & - - - & 0.5687 \\
    \hline
    
    It would not be harmful & 0.7606 & 61 &  1.8087 & .0754 & - - - & 0.4563  \\
    \hline
    
    I find the product reliable & - - - & - &  - - - & - - - & - - - & - - -  \\
    \hline
    
    I would trust the product & - - - & - &  - - - & - - - & - - - & - - - \\
    \hline

    \rowcolor{LightGray}\multicolumn{7}{c}{\textbf{Application AI Product}}\\
    \hline
    \textbf{Dependent}  & \textbf{Distance b/w} &  &  & & \textbf{Bonferroni} &  \\
    \textbf{Variable} & \textbf{Means} &  \textbf{df} &  \textbf{t-val} &   \textbf{p-value}  & \textbf{Correction} & \textbf{Cohen's \textit{d}} \\
    \hline
    
    I would feel in control & - - - & - &  - - - & - - - & - - - & - - -  \\
    \hline
    
    I would feel secure & - - - & - &  - - - & - - - & - - - & - - - \\
    \hline
    
    I would feel adequate & - - -  & - &  - - - & - - - & - - - & - - - \\
    \hline
    
    I would feel certain & - - - & - &  - - - & - - - & - - - & - - - \\
    \hline
    
    I would feel productive & - - - & - &  - - - & - - - & - - - & - - -   \\
    \hline
    \hline
    
    I perceived it as useful &  - - - & - &  - - - & - - - & - - - & - - -   \\
    \hline
    
    I would not be suspicious & - - - & - &  - - - & - - - & - - - & - - -   \\
    \hline
    
    It would not be harmful & - - - & - &  - - - & - - - & - - - & - - -  \\
    \hline
    
    I find the product reliable & - - - & - &  - - - & - - - & - - - & - - - \\
    \hline
    
    I would trust the product & - - - & - &  - - - & - - - & - - - & - - -

    \end{tabular}

    \caption{Guideline 10's t-test results %(\checkmark if Welch's t-test) 
    for lower self-efficacy vs. higher self-efficacy participants' average ratings of the independent Violation AI product (top) and Application AI product (bottom), for all 10 dependent variables.
    If dashes (- - -) are present, no statistical test was performed.
    If the number of tests exceeded 5 for each product, Bonferroni correction applied by multiplying p-values by the number of tests performed.
    }
    \label{tab:G10-SE-Stats-Appendix}
\end{table}
\clearpage
%---------------------------------------------------- End Guideline 10

%Begin Guideline 11----------------------------------------------------

\begin{table}[]
    \centering
    \begin{tabular}{cc|cc|cc|cc|cc}
    \multicolumn{2}{c|}{\includegraphics[width = 0.16\columnwidth]{assets/05-All-BoxPlots/10-G11/SE/G11-Feel-In-Control-SE.png}} &
    \multicolumn{2}{c|}{\includegraphics[width = 0.16\columnwidth]{assets/05-All-BoxPlots/10-G11/SE/G11-Feel-Secure-SE.png}} &
    \multicolumn{2}{c|}{\includegraphics[width = 0.16\columnwidth]{assets/05-All-BoxPlots/10-G11/SE/G11-Feel-Adequate-SE.png}} &
    \multicolumn{2}{c|}{\includegraphics[width = 0.16\columnwidth]{assets/05-All-BoxPlots/10-G11/SE/G11-Feel-Certain-SE.png}} &
    \multicolumn{2}{c}{\includegraphics[width = 0.16\columnwidth]{assets/05-All-BoxPlots/10-G11/SE/G11-Feel-Productive-SE.png}}
    \\
    \hline
    \hline
    \multicolumn{2}{c|}{\includegraphics[width = 0.16\columnwidth]{assets/05-All-BoxPlots/10-G11/SE/G11-Perceived-Useful-SE.png}} &
    \multicolumn{2}{c|}{\includegraphics[width = 0.16\columnwidth]{assets/05-All-BoxPlots/10-G11/SE/G11-Not-Suspicious-SE.png}} &
    \multicolumn{2}{c|}{\includegraphics[width = 0.16\columnwidth]{assets/05-All-BoxPlots/10-G11/SE/G11-Not-Harmful-SE.png}} &
    \multicolumn{2}{c|}{\includegraphics[width = 0.16\columnwidth]{assets/05-All-BoxPlots/10-G11/SE/G11-Product-Reliable-SE.png}} &
    \multicolumn{2}{c}{\includegraphics[width = 0.16\columnwidth]{assets/05-All-BoxPlots/10-G11/SE/G11-Trust-Product-SE.png}}
    \end{tabular}
    
    \caption{Guideline 11 participants' ratings for all dependent variables, disaggregated by participants' computer self-efficacy.
	%For the disaggregated data, notice how large the distances between the average rating are when the guideline is applied.
	Table~\ref{tab:G11-SE-Stats-Appendix} below provides the statistics (where applicable).
}
    \label{fig:SE-G11-Appendix}
\end{table}

\begin{table}[h]

%\framebox[\linewidth]{For Measuring!}
\centering
\footnotesize

    \begin{tabular}{p{0.22\columnwidth}|c|c|c|c|c|c}
    
    \rowcolor{LightGray}\multicolumn{7}{c}{\textbf{Violation AI Product}}\\
    \hline
    \textbf{Dependent}  & \textbf{Distance b/w} &  &  & & \textbf{Bonferroni} &  \\
    \textbf{Variable} & \textbf{Means} &  \textbf{df} &  \textbf{t-val} &   \textbf{p-value}  & \textbf{Correction} & \textbf{Cohen's \textit{d}} \\
    \hline
    
    I would feel in control & - - - & - &  - - - & - - - & - - - & - - - \\
    \hline
    
    I would feel secure & - - - & - &  - - - & - - - & - - - & - - - \\
    \hline
    
    I would feel adequate & - - - & - &  - - - & - - - & - - - & - - - \\
    \hline
    
    I would feel certain & - - - & - &  - - - & - - - & - - - & - - - \\
    \hline
    
    I would feel productive & - - - & - &  - - - & - - - & - - - & - - -  \\
    \hline
    \hline
    
    I perceived it as useful &  - - - & - &  - - - & - - - & - - - & - - -  \\
    \hline
    
    I would not be suspicious & - - - & - &  - - - & - - - & - - - & - - - \\
    \hline
    
    It would not be harmful & - - - & - &  - - - & - - - & - - - & - - -  \\
    \hline
    
    I find the product reliable & - - - & - &  - - - & - - - & - - - & - - -  \\
    \hline
    
    I would trust the product & - - - & - &  - - - & - - - & - - - & - - - \\
    \hline

    \rowcolor{LightGray}\multicolumn{7}{c}{\textbf{Application AI Product}}\\
    \hline
    \textbf{Dependent}  & \textbf{Distance b/w} &  &  & & \textbf{Bonferroni} &  \\
    \textbf{Variable} & \textbf{Means} &  \textbf{df} &  \textbf{t-val} &   \textbf{p-value}  & \textbf{Correction} & \textbf{Cohen's \textit{d}} \\
    \hline
    
    I would feel in control & - - - & - &  - - - & - - - & - - - & - - -  \\
    \hline
    
    I would feel secure & - - - & - &  - - - & - - - & - - - & - - - \\
    \hline
    
    I would feel adequate & - - - & - &  - - - & - - - & - - - & - - - \\
    \hline
    
    I would feel certain & - - - & - &  - - - & - - - & - - - & - - - \\
    \hline
    
    I would feel productive & - - - & - &  - - - & - - - & - - - & - - -   \\
    \hline
    \hline
    
    I perceived it as useful &  - - - & - &  - - - & - - - & - - - & - - -   \\
    \hline
    
    I would not be suspicious & - - - & - &  - - - & - - - & - - - & - - -   \\
    \hline
    
    It would not be harmful & - - - & - &  - - - & - - - & - - - & - - -  \\
    \hline
    
    I find the product reliable & - - - & - &  - - - & - - - & - - - & - - - \\
    \hline
    
    I would trust the product & 0.6308 & 61 &  1.8748 & .0656 & - - - & 0.4739

    \end{tabular}

    \caption{Guideline 11's t-test results %(\checkmark if Welch's t-test) 
    for lower self-efficacy vs. higher self-efficacy participants' average ratings of the independent Violation AI product (top) and Application AI product (bottom), for all 10 dependent variables.
    If dashes (- - -) are present, no statistical test was performed.
    If the number of tests exceeded 5 for each product, Bonferroni correction applied by multiplying p-values by the number of tests performed.
    }
    \label{tab:G11-SE-Stats-Appendix}
\end{table}
\clearpage
%---------------------------------------------------- End Guideline 11

%Begin Guideline 12----------------------------------------------------

\begin{table}[]
    \centering
    \begin{tabular}{cc|cc|cc|cc|cc}
    \multicolumn{2}{c|}{\includegraphics[width = 0.16\columnwidth]{assets/05-All-BoxPlots/11-G12/SE/G12-Feel-In-Control-SE.png}} &
    \multicolumn{2}{c|}{\includegraphics[width = 0.16\columnwidth]{assets/05-All-BoxPlots/11-G12/SE/G12-Feel-Secure-SE.png}} &
    \multicolumn{2}{c|}{\includegraphics[width = 0.16\columnwidth]{assets/05-All-BoxPlots/11-G12/SE/G12-Feel-Adequate-SE.png}} &
    \multicolumn{2}{c|}{\includegraphics[width = 0.16\columnwidth]{assets/05-All-BoxPlots/11-G12/SE/G12-Feel-Certain-SE.png}} &
    \multicolumn{2}{c}{\includegraphics[width = 0.16\columnwidth]{assets/05-All-BoxPlots/11-G12/SE/G12-Feel-Productive-SE.png}}
    \\
    \hline
    \hline
    \multicolumn{2}{c|}{\includegraphics[width = 0.16\columnwidth]{assets/05-All-BoxPlots/11-G12/SE/G12-Perceived-Useful-SE.png}} &
    \multicolumn{2}{c|}{\includegraphics[width = 0.16\columnwidth]{assets/05-All-BoxPlots/11-G12/SE/G12-Not-Suspicious-SE.png}} &
    \multicolumn{2}{c|}{\includegraphics[width = 0.16\columnwidth]{assets/05-All-BoxPlots/11-G12/SE/G12-Not-Harmful-SE.png}} &
    \multicolumn{2}{c|}{\includegraphics[width = 0.16\columnwidth]{assets/05-All-BoxPlots/11-G12/SE/G12-Product-Reliable-SE.png}} &
    \multicolumn{2}{c}{\includegraphics[width = 0.16\columnwidth]{assets/05-All-BoxPlots/11-G12/SE/G12-Trust-Product-SE.png}}
    \end{tabular}
    
    \caption{Guideline 12 participants' ratings for all dependent variables, disaggregated by participants' computer self-efficacy.
	%For the disaggregated data, notice how large the distances between the average rating are when the guideline is applied.
	Table~\ref{tab:G12-SE-Stats-Appendix} below provides the statistics (where applicable).
}
    \label{fig:SE-G12-Appendix}
\end{table}

\begin{table}[h]

%\framebox[\linewidth]{For Measuring!}
\centering
\footnotesize

    \begin{tabular}{p{0.22\columnwidth}|c|c|c|c|c|c}
    
    \rowcolor{LightGray}\multicolumn{7}{c}{\textbf{Violation AI Product}}\\
    \hline
    \textbf{Dependent}  & \textbf{Distance b/w} &  &  & & \textbf{Bonferroni} &  \\
    \textbf{Variable} & \textbf{Means} &  \textbf{df} &  \textbf{t-val} &   \textbf{p-value}  & \textbf{Correction} & \textbf{Cohen's \textit{d}} \\
    \hline
    
    I would feel in control & - - - & - &  - - - & - - - & - - - & - - -  \\
    \hline
    
    I would feel secure & - - - & - &  - - - & - - - & - - - & - - - \\
    \hline
    
    I would feel adequate & - - -  & - &  - - - & - - - & - - - & - - - \\
    \hline
    
    I would feel certain & - - - & - &  - - - & - - - & - - - & - - - \\
    \hline
    
    I would feel productive & - - - & - &  - - - & - - - & - - - & - - -   \\
    \hline
    \hline
    
    I perceived it as useful &  - - - & - &  - - - & - - - & - - - & - - -   \\
    \hline
    
    I would not be suspicious & - - - & - &  - - - & - - - & - - - & - - -   \\
    \hline
    
    It would not be harmful & - - - & - &  - - - & - - - & - - - & - - -  \\
    \hline
    
    I find the product reliable & - - - & - &  - - - & - - - & - - - & - - - \\
    \hline
    
    I would trust the product & - - - & - &  - - - & - - - & - - - & - - - \\
    \hline

    \rowcolor{LightGray}\multicolumn{7}{c}{\textbf{Application AI Product}}\\
    \hline
    \textbf{Dependent}  & \textbf{Distance b/w} &  &  & & \textbf{Bonferroni} &  \\
    \textbf{Variable} & \textbf{Means} &  \textbf{df} &  \textbf{t-val} &   \textbf{p-value}  & \textbf{Correction} & \textbf{Cohen's \textit{d}} \\
    \hline
    
    I would feel in control & - - - & - &  - - - & - - - & - - - & - - -  \\
    \hline
    
    I would feel secure & - - - & - &  - - - & - - - & - - - & - - - \\
    \hline
    
    I would feel adequate & - - -  & - &  - - - & - - - & - - - & - - - \\
    \hline
    
    I would feel certain & - - - & - &  - - - & - - - & - - - & - - - \\
    \hline
    
    I would feel productive & - - - & - &  - - - & - - - & - - - & - - -   \\
    \hline
    \hline
    
    I perceived it as useful &  - - - & - &  - - - & - - - & - - - & - - -   \\
    \hline
    
    I would not be suspicious & - - - & - &  - - - & - - - & - - - & - - -   \\
    \hline
    
    It would not be harmful & - - - & - &  - - - & - - - & - - - & - - -  \\
    \hline
    
    I find the product reliable & - - - & - &  - - - & - - - & - - - & - - - \\
    \hline
    
    I would trust the product & - - - & - &  - - - & - - - & - - - & - - -

    \end{tabular}

    \caption{Guideline 12's t-test results %(\checkmark if Welch's t-test) 
    for lower self-efficacy vs. higher self-efficacy participants' average ratings of the independent Violation AI product (top) and Application AI product (bottom), for all 10 dependent variables.
    If dashes (- - -) are present, no statistical test was performed.
    If the number of tests exceeded 5 for each product, Bonferroni correction applied by multiplying p-values by the number of tests performed.
    }
    \label{tab:G12-SE-Stats-Appendix}
\end{table}
\clearpage
%---------------------------------------------------- End Guideline 12

%Begin Guideline 13----------------------------------------------------

\begin{table}[]
    \centering
    \begin{tabular}{cc|cc|cc|cc|cc}
    \multicolumn{2}{c|}{\includegraphics[width = 0.16\columnwidth]{assets/05-All-BoxPlots/12-G13/SE/G13-Feel-In-Control-SE.png}} &
    \multicolumn{2}{c|}{\includegraphics[width = 0.16\columnwidth]{assets/05-All-BoxPlots/12-G13/SE/G13-Feel-Secure-SE.png}} &
    \multicolumn{2}{c|}{\includegraphics[width = 0.16\columnwidth]{assets/05-All-BoxPlots/12-G13/SE/G13-Feel-Adequate-SE.png}} &
    \multicolumn{2}{c|}{\includegraphics[width = 0.16\columnwidth]{assets/05-All-BoxPlots/12-G13/SE/G13-Feel-Certain-SE.png}} &
    \multicolumn{2}{c}{\includegraphics[width = 0.16\columnwidth]{assets/05-All-BoxPlots/12-G13/SE/G13-Feel-Productive-SE.png}}
    \\
    \hline
    \hline
    \multicolumn{2}{c|}{\includegraphics[width = 0.16\columnwidth]{assets/05-All-BoxPlots/12-G13/SE/G13-Perceived-Useful-SE.png}} &
    \multicolumn{2}{c|}{\includegraphics[width = 0.16\columnwidth]{assets/05-All-BoxPlots/12-G13/SE/G13-Not-Suspicious-SE.png}} &
    \multicolumn{2}{c|}{\includegraphics[width = 0.16\columnwidth]{assets/05-All-BoxPlots/12-G13/SE/G13-Not-Harmful-SE.png}} &
    \multicolumn{2}{c|}{\includegraphics[width = 0.16\columnwidth]{assets/05-All-BoxPlots/12-G13/SE/G13-Product-Reliable-SE.png}} &
    \multicolumn{2}{c}{\includegraphics[width = 0.16\columnwidth]{assets/05-All-BoxPlots/12-G13/SE/G13-Trust-Product-SE.png}}
    \end{tabular}
    
    \caption{Guideline 13 participants' ratings for all dependent variables, disaggregated by participants' computer self-efficacy.
	%For the disaggregated data, notice how large the distances between the average rating are when the guideline is applied.
	Table~\ref{tab:G13-SE-Stats-Appendix} below provides the statistics (where applicable).
}
    \label{fig:SE-G13-Appendix}
\end{table}

\begin{table}[h]

%\framebox[\linewidth]{For Measuring!}
\centering
\footnotesize

    \begin{tabular}{p{0.22\columnwidth}|c|c|c|c|c|c}
    
    \rowcolor{LightGray}\multicolumn{7}{c}{\textbf{Violation AI Product}}\\
    \hline
    \textbf{Dependent}  & \textbf{Distance b/w} &  &  & & \textbf{Bonferroni} &  \\
    \textbf{Variable} & \textbf{Means} &  \textbf{df} &  \textbf{t-val} &   \textbf{p-value}  & \textbf{Correction} & \textbf{Cohen's \textit{d}} \\
    \hline
    
    I would feel in control & 1.0794 & 55 &  3.0581 & \cellcolor{AbiOrangeQuote}.0034 & - - - & 0.8132  \\
    \hline
    
    I would feel secure & - - - & - &  - - - & - - - & - - - & - - - \\
    \hline
    
    I would feel adequate & 1.1836  & 55 &  2.8562 & \cellcolor{AbiOrangeQuote}.0060 & - - - & 0.7596 \\
    \hline
    
    I would feel certain & 1.0955 & 55 &  2.6319 & \cellcolor{AbiOrangeQuote}.0110 & - - - & 0.6999 \\
    \hline
    
    I would feel productive & - - - & - &  - - - & - - - & - - - & - - -   \\
    \hline
    \hline
    
    I perceived it as useful &  0.7355 & 54 &  2.0324 & \cellcolor{AbiOrangeQuote}.0470 & - - - & 0.5463   \\
    \hline
    
    I would not be suspicious & 0.9161 & 54 &  2.0331 & \cellcolor{AbiOrangeQuote}.0469 & - - - & 0.5465   \\
    \hline
    
    It would not be harmful & - - - & - &  - - - & - - - & - - - & - - -  \\
    \hline
    
    I find the product reliable & - - - & - &  - - - & - - - & - - - & - - - \\
    \hline
    
    I would trust the product & - - - & - &  - - - & - - - & - - - & - - - \\
    \hline

    \rowcolor{LightGray}\multicolumn{7}{c}{\textbf{Application AI Product}}\\
    \hline
    \textbf{Dependent}  & \textbf{Distance b/w} &  &  & & \textbf{Bonferroni} &  \\
    \textbf{Variable} & \textbf{Means} &  \textbf{df} &  \textbf{t-val} &   \textbf{p-value}  & \textbf{Correction} & \textbf{Cohen's \textit{d}} \\
    \hline
    
    I would feel in control & 0.8542 & 54 &  3.0859 & \cellcolor{AbiOrangeQuote}.0032 & \cellcolor{AbiOrangeQuote}.0192 & 0.8295  \\
    \hline
    
    I would feel secure & 0.5149 & 55 &  1.2853 & .2041 & 1.000 & 0.3418 \\
    \hline
    
    I would feel adequate & 0.7692  & 55 &  2.1602 & \cellcolor{AbiOrangeQuote}.0351 & .2106 & 0.5745 \\
    \hline
    
    I would feel certain & - - - & - &  - - - & - - - & - - - & - - - \\
    \hline
    
    I would feel productive & - - - & - &  - - - & - - - & - - - & - - -   \\
    \hline
    \hline
    
    I perceived it as useful &  0.5600 & 54 &  2.1615 & \cellcolor{AbiOrangeQuote}.0351 & .2106 & 0.5810   \\
    \hline
    
    I would not be suspicious & - - - & - &  - - - & - - - & - - - & - - -   \\
    \hline
    
    It would not be harmful & 1.2022 & 55 &  3.9091 & \cellcolor{AbiOrangeQuote}.0003 & \cellcolor{AbiOrangeQuote}.0018 & 1.0395  \\
    \hline
    
    I find the product reliable & - - - & - &  - - - & - - - & - - - & - - - \\
    \hline
    
    I would trust the product & 0.6103 & 54 &  1.3672 & .1772 & 1.000 & 0.5220

    \end{tabular}

    \caption{Guideline 13's t-test results %(\checkmark if Welch's t-test) 
    for lower self-efficacy vs. higher self-efficacy participants' average ratings of the independent Violation AI product (top) and Application AI product (bottom), for all 10 dependent variables.
    If dashes (- - -) are present, no statistical test was performed.
    If the number of tests exceeded 5 for each product, Bonferroni correction applied by multiplying p-values by the number of tests performed.
    }
    \label{tab:G13-SE-Stats-Appendix}
\end{table}
\clearpage
%---------------------------------------------------- End Guideline 13

%Begin Guideline 14---------------------------------------------------

\begin{table}[]
    \centering
    \begin{tabular}{cc|cc|cc|cc|cc}
    \multicolumn{2}{c|}{\includegraphics[width = 0.16\columnwidth]{assets/05-All-BoxPlots/13-G14/SE/G14-Feel-In-Control-SE.png}} &
    \multicolumn{2}{c|}{\includegraphics[width = 0.16\columnwidth]{assets/05-All-BoxPlots/13-G14/SE/G14-Feel-Secure-SE.png}} &
    \multicolumn{2}{c|}{\includegraphics[width = 0.16\columnwidth]{assets/05-All-BoxPlots/13-G14/SE/G14-Feel-Adequate-SE.png}} &
    \multicolumn{2}{c|}{\includegraphics[width = 0.16\columnwidth]{assets/05-All-BoxPlots/13-G14/SE/G14-Feel-Certain-SE.png}} &
    \multicolumn{2}{c}{\includegraphics[width = 0.16\columnwidth]{assets/05-All-BoxPlots/13-G14/SE/G14-Feel-Productive-SE.png}}
    \\
    \hline
    \hline
    \multicolumn{2}{c|}{\includegraphics[width = 0.16\columnwidth]{assets/05-All-BoxPlots/13-G14/SE/G14-Perceived-Useful-SE.png}} &
    \multicolumn{2}{c|}{\includegraphics[width = 0.16\columnwidth]{assets/05-All-BoxPlots/13-G14/SE/G14-Not-Suspicious-SE.png}} &
    \multicolumn{2}{c|}{\includegraphics[width = 0.16\columnwidth]{assets/05-All-BoxPlots/13-G14/SE/G14-Not-Harmful-SE.png}} &
    \multicolumn{2}{c|}{\includegraphics[width = 0.16\columnwidth]{assets/05-All-BoxPlots/13-G14/SE/G14-Product-Reliable-SE.png}} &
    \multicolumn{2}{c}{\includegraphics[width = 0.16\columnwidth]{assets/05-All-BoxPlots/13-G14/SE/G14-Trust-Product-SE.png}}
    \end{tabular}
    
    \caption{Guideline 14 participants' ratings for all dependent variables, disaggregated by participants' computer self-efficacy.
	%For the disaggregated data, notice how large the distances between the average rating are when the guideline is applied.
	Table~\ref{tab:G14-SE-Stats-Appendix} below provides the statistics (where applicable).
}
    \label{fig:SE-G14-Appendix}
\end{table}

\begin{table}[h]

%\framebox[\linewidth]{For Measuring!}
\centering
\footnotesize

    \begin{tabular}{p{0.22\columnwidth}|c|c|c|c|c|c}
    
    \rowcolor{LightGray}\multicolumn{7}{c}{\textbf{Violation AI Product}}\\
    \hline
    \textbf{Dependent}  & \textbf{Distance b/w} &  &  & & \textbf{Bonferroni} &  \\
    \textbf{Variable} & \textbf{Means} &  \textbf{df} &  \textbf{t-val} &   \textbf{p-value}  & \textbf{Correction} & \textbf{Cohen's \textit{d}} \\
    \hline
    
    I would feel in control & - - - & - &  - - - & - - - & - - - & - - -  \\
    \hline
    
    I would feel secure & - - - & - &  - - - & - - - & - - - & - - - \\
    \hline
    
    I would feel adequate & - - - & - &  - - - & - - - & - - - & - - - \\
    \hline
    
    I would feel certain & - - - & - &  - - - & - - - & - - - & - - - \\
    \hline
    
    I would feel productive & - - - & - &  - - - & - - - & - - - & - - -   \\
    \hline
    \hline
    
    I perceived it as useful &  - - - & - &  - - - & - - - & - - - & - - -  \\
    \hline
    
    I would not be suspicious & - - - & - &  - - - & - - - & - - - & - - -  \\
    \hline
    
    It would not be harmful & 0.6600 & 63 &  1.7784 & .0802 & - - - & 0.4412  \\
    \hline
    
    I find the product reliable & - - - & - &  - - - & - - - & - - - & - - - \\
    \hline
    
    I would trust the product & - - - & - &  - - - & - - - & - - - & - - - \\
    \hline

    \rowcolor{LightGray}\multicolumn{7}{c}{\textbf{Application AI Product}}\\
    \hline
    \textbf{Dependent}  & \textbf{Distance b/w} &  &  & & \textbf{Bonferroni} &  \\
    \textbf{Variable} & \textbf{Means} &  \textbf{df} &  \textbf{t-val} &   \textbf{p-value}  & \textbf{Correction} & \textbf{Cohen's \textit{d}} \\
    \hline
    
    I would feel in control & - - - & - &  - - - & - - - & - - - & - - -  \\
    \hline
    
    I would feel secure & - - - & - &  - - - & - - - & - - - & - - - \\
    \hline
    
    I would feel adequate & - - - & - &  - - - & - - - & - - - & - - - \\
    \hline
    
    I would feel certain & - - - & - &  - - - & - - - & - - - & - - - \\
    \hline
    
    I would feel productive & - - - & - &  - - - & - - - & - - - & - - - \\
    \hline
    \hline
    
    I perceived it as useful &  - - - & - &  - - - & - - - & - - - & - - -   \\
    \hline
    
    I would not be suspicious & - - - & - &  - - - & - - - & - - - & - - -  \\
    \hline
    
    It would not be harmful & 0.5927 & 65 &  2.3268 & \cellcolor{AbiOrangeQuote}.0231 & - - - & 0.5686  \\
    \hline
    
    I find the product reliable & 0.7398 & 65 &  2.3433 & \cellcolor{AbiOrangeQuote}.0222 & - - - & 0.5726 \\
    \hline
    
    I would trust the product & 0.5187 & 65 &  1.8766 & 0.0651 & - - - & 0.4586

    \end{tabular}

    \caption{Guideline 14's t-test results %(\checkmark if Welch's t-test) 
    for lower self-efficacy vs. higher self-efficacy participants' average ratings of the independent Violation AI product (top) and Application AI product (bottom), for all 10 dependent variables.
    If dashes (- - -) are present, no statistical test was performed.
    If the number of tests exceeded 5 for each product, Bonferroni correction applied by multiplying p-values by the number of tests performed.
    }
    \label{tab:G14-SE-Stats-Appendix}
\end{table}
\clearpage
%---------------------------------------------------- End Guideline 14

%Begin Guideline 15---------------------------------------------------

\begin{table}[]
    \centering
    \begin{tabular}{cc|cc|cc|cc|cc}
    \multicolumn{2}{c|}{\includegraphics[width = 0.16\columnwidth]{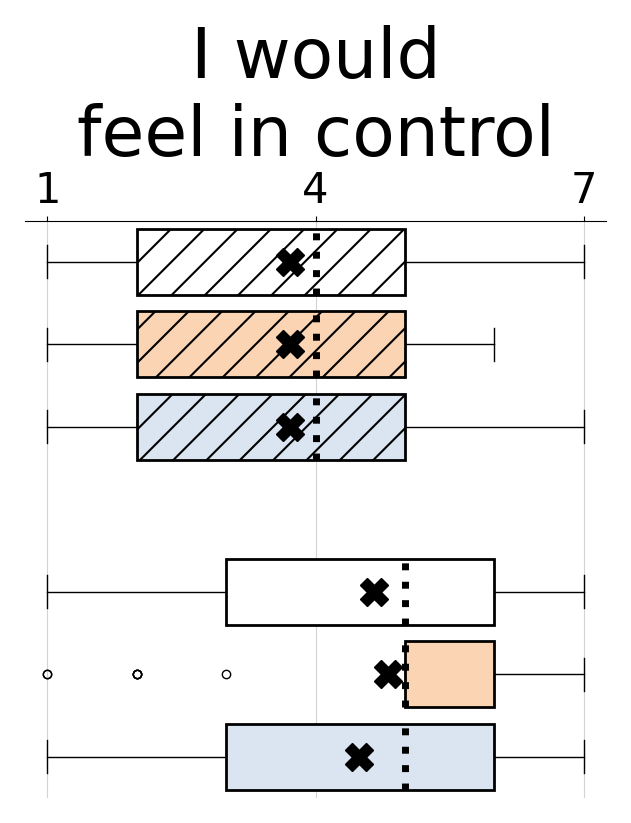}} &
    \multicolumn{2}{c|}{\includegraphics[width = 0.16\columnwidth]{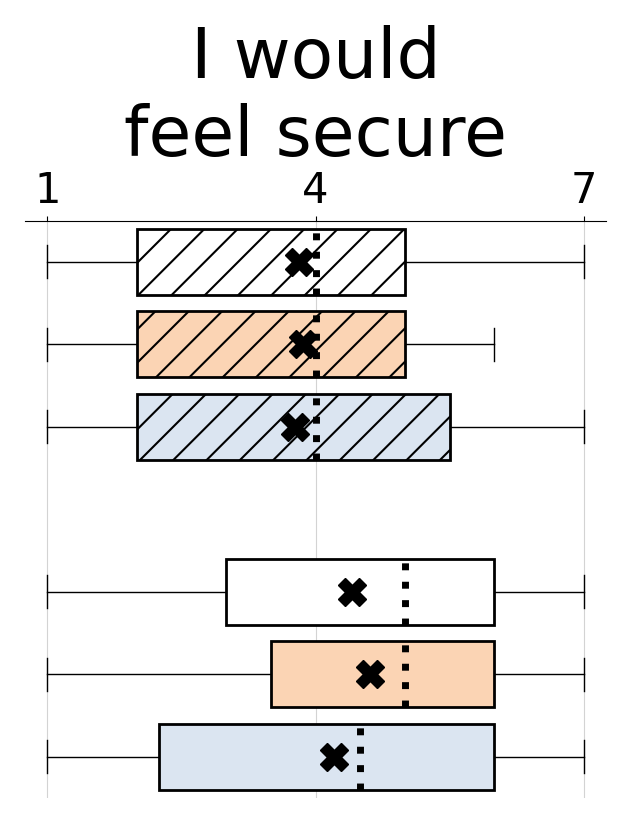}} &
    \multicolumn{2}{c|}{\includegraphics[width = 0.16\columnwidth]{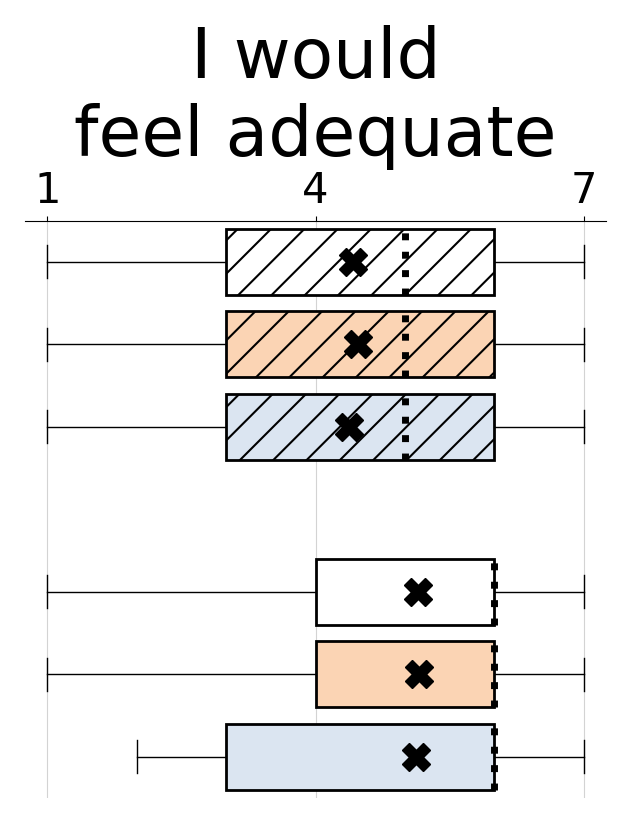}} &
    \multicolumn{2}{c|}{\includegraphics[width = 0.16\columnwidth]{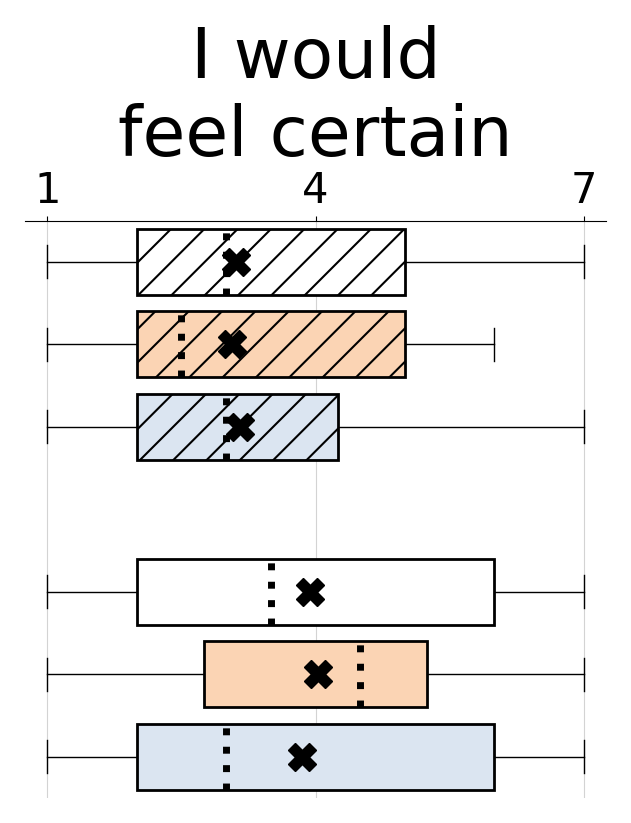}} &
    \multicolumn{2}{c}{\includegraphics[width = 0.16\columnwidth]{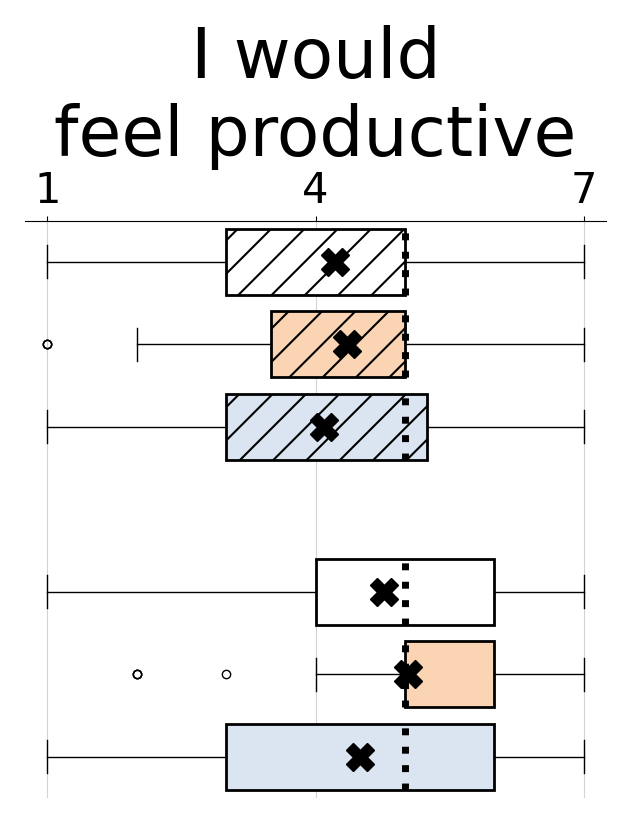}}
    \\
    \hline
    \hline
    \multicolumn{2}{c|}{\includegraphics[width = 0.16\columnwidth]{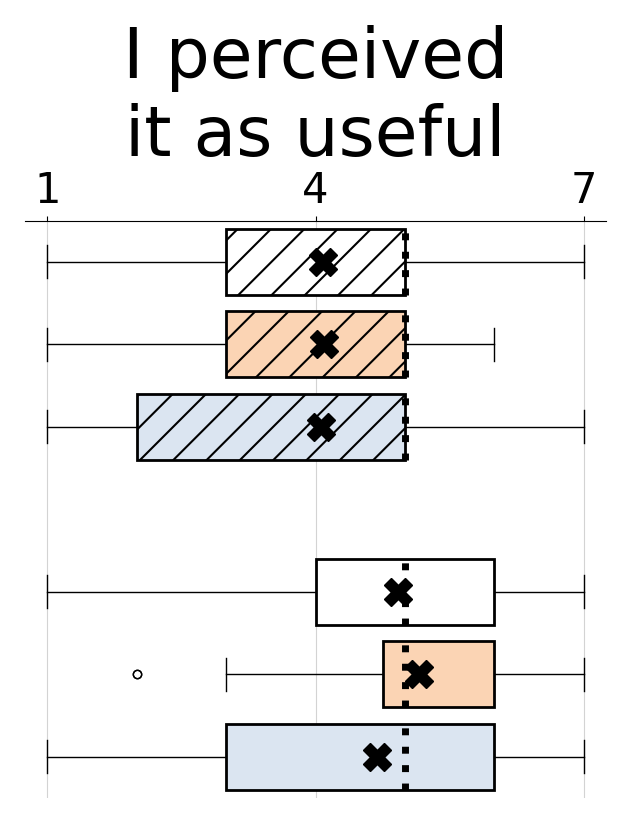}} &
    \multicolumn{2}{c|}{\includegraphics[width = 0.16\columnwidth]{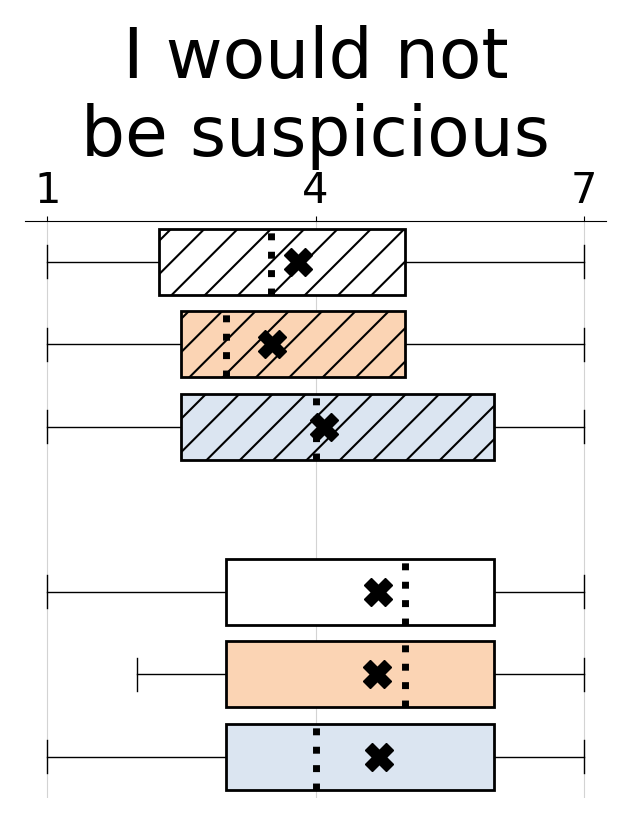}} &
    \multicolumn{2}{c|}{\includegraphics[width = 0.16\columnwidth]{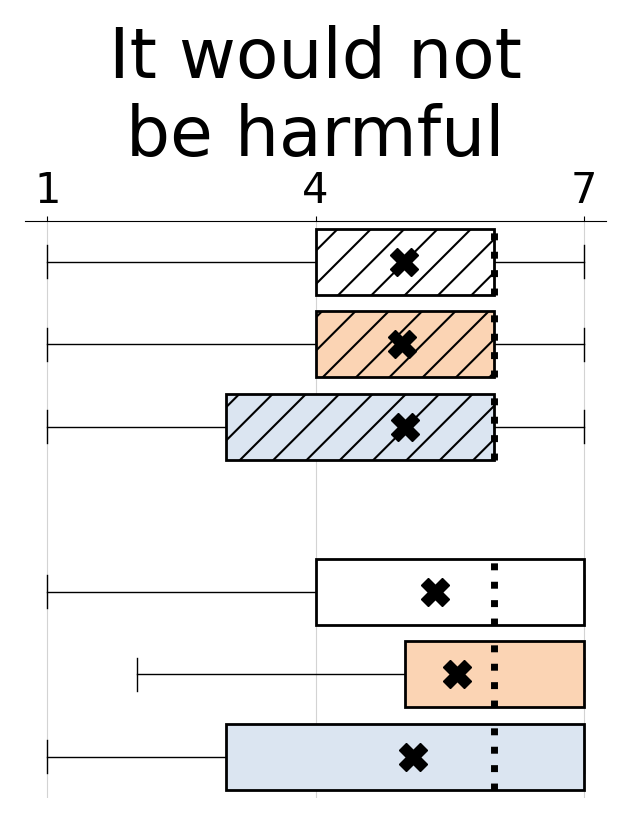}} &
    \multicolumn{2}{c|}{\includegraphics[width = 0.16\columnwidth]{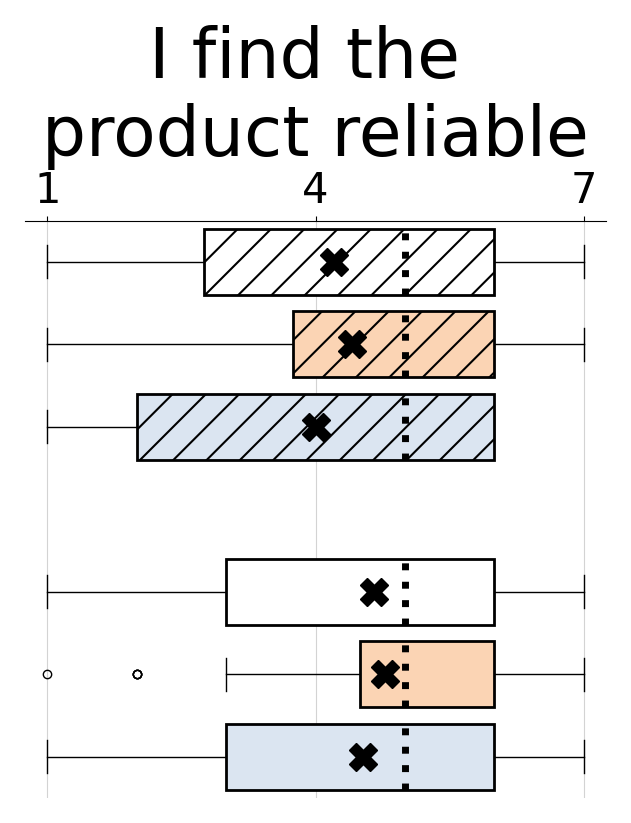}} &
    \multicolumn{2}{c}{\includegraphics[width = 0.16\columnwidth]{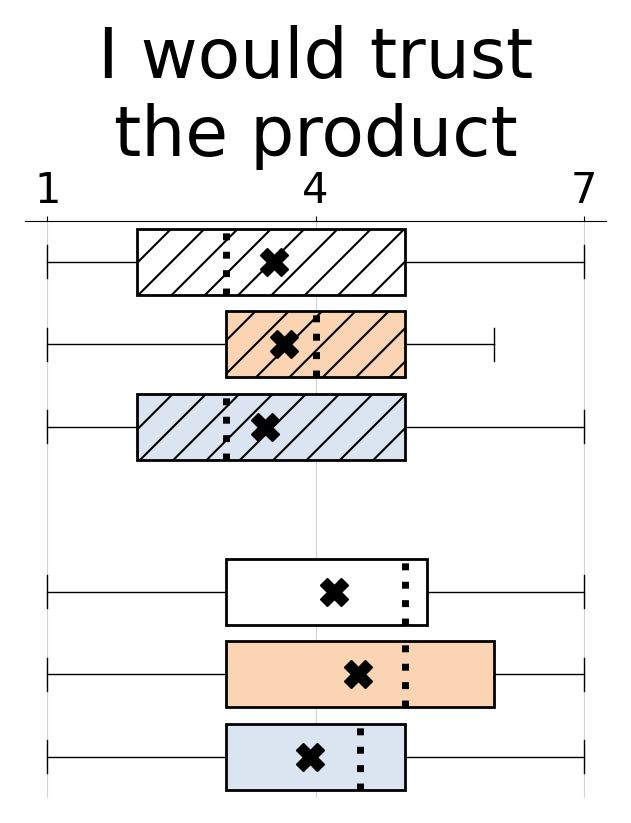}}
    \end{tabular}
    
    \caption{Guideline 15 participants' ratings for all dependent variables, disaggregated by participants' computer self-efficacy.
	%For the disaggregated data, notice how large the distances between the average rating are when the guideline is applied.
	Table~\ref{tab:G15-SE-Stats-Appendix} below provides the statistics (where applicable).
}
    \label{fig:SE-G15-Appendix}
\end{table}

\begin{table}[h]

%\framebox[\linewidth]{For Measuring!}
\centering
\footnotesize

    \begin{tabular}{p{0.22\columnwidth}|c|c|c|c|c|c}
    
    \rowcolor{LightGray}\multicolumn{7}{c}{\textbf{Violation AI Product}}\\
    \hline
    \textbf{Dependent}  & \textbf{Distance b/w} &  &  & & \textbf{Bonferroni} &  \\
    \textbf{Variable} & \textbf{Means} &  \textbf{df} &  \textbf{t-val} &   \textbf{p-value}  & \textbf{Correction} & \textbf{Cohen's \textit{d}} \\
    \hline
    
    I would feel in control & - - - & - &  - - - & - - - & - - - & - - -  \\
    \hline
    
    I would feel secure &  - - - & - &  - - - & - - - & - - - & - - - \\
    \hline
    
    I would feel adequate &  - - - & - &  - - - & - - - & - - - & - - - \\
    \hline
    
    I would feel certain &  - - - & - &  - - - & - - - & - - - & - - - \\
    \hline
    
    I would feel productive & - - - & - &  - - - & - - - & - - - & - - -  \\
    \hline
    \hline
    
    I perceived it as useful &   - - - & - &  - - - & - - - & - - - & - - -  \\
    \hline
    
    I would not be suspicious &  0.8381 & 60 &  1.8059 & .0760 & - - - & 0.4626   \\
    \hline
    
    It would not be harmful &  - - - & - &  - - - & - - - & - - - & - - -  \\
    \hline
    
    I find the product reliable &  - - - & - &  - - - & - - - & - - - & - - - \\
    \hline
    
    I would trust the product &  - - - & - &  - - - & - - - & - - - & - - - \\
    \hline

    \rowcolor{LightGray}\multicolumn{7}{c}{\textbf{Application AI Product}}\\
    \hline
    \textbf{Dependent}  & \textbf{Distance b/w} &  &  & & \textbf{Bonferroni} &  \\
    \textbf{Variable} & \textbf{Means} &  \textbf{df} &  \textbf{t-val} &   \textbf{p-value}  & \textbf{Correction} & \textbf{Cohen's \textit{d}} \\
    \hline
    
    I would feel in control &  - - - & - &  - - - & - - - & - - - & - - -  \\
    \hline
    
    I would feel secure &  - - - & - &  - - - & - - - & - - - & - - - \\
    \hline
    
    I would feel adequate & - - - & - &  - - - & - - - & - - - & - - - \\
    \hline
    
    I would feel certain &  - - - & - &  - - - & - - - & - - - & - - -\\
    \hline
    
    I would feel productive &  0.2262 & 62 &  0.5410 & .5904 & - - - & 0.1363  \\
    \hline
    \hline
    
    I perceived it as useful &   - - - & - &  - - - & - - - & - - - & - - -  \\
    \hline
    
    I would not be suspicious &  - - - & - &  - - - & - - - & - - - & - - -   \\
    \hline
    
    It would not be harmful &  - - - & - &  - - - & - - - & - - - & - - -  \\
    \hline
    
    I find the product reliable &  - - - & - &  - - - & - - - & - - - & - - - \\
    \hline
    
    I would trust the product & - - - & - &  - - - & - - - & - - - & - - -

    \end{tabular}

    \caption{Guideline 15's t-test results %(\checkmark if Welch's t-test) 
    for lower self-efficacy vs. higher self-efficacy participants' average ratings of the independent Violation AI product (top) and Application AI product (bottom), for all 10 dependent variables.
    If dashes (- - -) are present, no statistical test was performed.
    If the number of tests exceeded 5 for each product, Bonferroni correction applied by multiplying p-values by the number of tests performed.
    }
    \label{tab:G15-SE-Stats-Appendix}
\end{table}
\clearpage
%---------------------------------------------------- End Guideline 15

%Begin Guideline 17---------------------------------------------------

\begin{table}[]
    \centering
    \begin{tabular}{cc|cc|cc|cc|cc}
    \multicolumn{2}{c|}{\includegraphics[width = 0.16\columnwidth]{assets/05-All-BoxPlots/15-G17/SE/G17-Feel-In-Control-SE.png}} &
    \multicolumn{2}{c|}{\includegraphics[width = 0.16\columnwidth]{assets/05-All-BoxPlots/15-G17/SE/G17-Feel-Secure-SE.png}} &
    \multicolumn{2}{c|}{\includegraphics[width = 0.16\columnwidth]{assets/05-All-BoxPlots/15-G17/SE/G17-Feel-Adequate-SE.png}} &
    \multicolumn{2}{c|}{\includegraphics[width = 0.16\columnwidth]{assets/05-All-BoxPlots/15-G17/SE/G17-Feel-Certain-SE.png}} &
    \multicolumn{2}{c}{\includegraphics[width = 0.16\columnwidth]{assets/05-All-BoxPlots/15-G17/SE/G17-Feel-Productive-SE.png}}
    \\
    \hline
    \hline
    \multicolumn{2}{c|}{\includegraphics[width = 0.16\columnwidth]{assets/05-All-BoxPlots/15-G17/SE/G17-Perceived-Useful-SE.png}} &
    \multicolumn{2}{c|}{\includegraphics[width = 0.16\columnwidth]{assets/05-All-BoxPlots/15-G17/SE/G17-Not-Suspicious-SE.png}} &
    \multicolumn{2}{c|}{\includegraphics[width = 0.16\columnwidth]{assets/05-All-BoxPlots/15-G17/SE/G17-Not-Harmful-SE.png}} &
    \multicolumn{2}{c|}{\includegraphics[width = 0.16\columnwidth]{assets/05-All-BoxPlots/15-G17/SE/G17-Product-Reliable-SE.png}} &
    \multicolumn{2}{c}{\includegraphics[width = 0.16\columnwidth]{assets/05-All-BoxPlots/15-G17/SE/G17-Trust-Product-SE.png}}
    \end{tabular}
    
    \caption{Guideline 17 participants' ratings for all dependent variables, disaggregated by participants' computer self-efficacy.
	%For the disaggregated data, notice how large the distances between the average rating are when the guideline is applied.
	Table~\ref{tab:G17-SE-Stats-Appendix} below provides the statistics (where applicable).
}
    \label{fig:SE-G17-Appendix}
\end{table}

\begin{table}[h]

%\framebox[\linewidth]{For Measuring!}
\centering
\footnotesize

    \begin{tabular}{p{0.22\columnwidth}|c|c|c|c|c|c}
    
    \rowcolor{LightGray}\multicolumn{7}{c}{\textbf{Violation AI Product}}\\
    \hline
    \textbf{Dependent}  & \textbf{Distance b/w} &  &  & & \textbf{Bonferroni} &  \\
    \textbf{Variable} & \textbf{Means} &  \textbf{df} &  \textbf{t-val} &   \textbf{p-value}  & \textbf{Correction} & \textbf{Cohen's \textit{d}} \\
    \hline
    
    I would feel in control & - - - & - &  - - - & - - - & - - - & - - -  \\
    \hline
    
    I would feel secure & - - - & - &  - - - & - - - & - - - & - - - \\
    \hline
    
    I would feel adequate & - - -  & - &  - - - & - - - & - - - & - - - \\
    \hline
    
    I would feel certain & - - - & - &  - - - & - - - & - - - & - - - \\
    \hline
    
    I would feel productive & - - - & - &  - - - & - - - & - - - & - - -   \\
    \hline
    \hline
    
    I perceived it as useful &  - - - & - &  - - - & - - - & - - - & - - -   \\
    \hline
    
    I would not be suspicious & - - - & - &  - - - & - - - & - - - & - - -   \\
    \hline
    
    It would not be harmful & - - - & - &  - - - & - - - & - - - & - - -  \\
    \hline
    
    I find the product reliable & - - - & - &  - - - & - - - & - - - & - - - \\
    \hline
    
    I would trust the product & - - - & - &  - - - & - - - & - - - & - - - \\
    \hline

    \rowcolor{LightGray}\multicolumn{7}{c}{\textbf{Application AI Product}}\\
    \hline
    \textbf{Dependent}  & \textbf{Distance b/w} &  &  & & \textbf{Bonferroni} &  \\
    \textbf{Variable} & \textbf{Means} &  \textbf{df} &  \textbf{t-val} &   \textbf{p-value}  & \textbf{Correction} & \textbf{Cohen's \textit{d}} \\
    \hline
    
    I would feel in control & - - - & - &  - - - & - - - & - - - & - - -  \\
    \hline
    
    I would feel secure & - - - & - &  - - - & - - - & - - - & - - - \\
    \hline
    
    I would feel adequate & - - -  & - &  - - - & - - - & - - - & - - - \\
    \hline
    
    I would feel certain & - - - & - &  - - - & - - - & - - - & - - - \\
    \hline
    
    I would feel productive & - - - & - &  - - - & - - - & - - - & - - -   \\
    \hline
    \hline
    
    I perceived it as useful &  - - - & - &  - - - & - - - & - - - & - - -   \\
    \hline
    
    I would not be suspicious & - - - & - &  - - - & - - - & - - - & - - -   \\
    \hline
    
    It would not be harmful & - - - & - &  - - - & - - - & - - - & - - -  \\
    \hline
    
    I find the product reliable & - - - & - &  - - - & - - - & - - - & - - - \\
    \hline
    
    I would trust the product & - - - & - &  - - - & - - - & - - - & - - -

    \end{tabular}

    \caption{Guideline 17's t-test results %(\checkmark if Welch's t-test) 
    for lower self-efficacy vs. higher self-efficacy participants' average ratings of the independent Violation AI product (top) and Application AI product (bottom), for all 10 dependent variables.
    If dashes (- - -) are present, no statistical test was performed.
    If the number of tests exceeded 5 for each product, Bonferroni correction applied by multiplying p-values by the number of tests performed.
    }
    \label{tab:G17-SE-Stats-Appendix}
\end{table}
\clearpage
%---------------------------------------------------- End Guideline 17

%Begin Guideline 17---------------------------------------------------

\begin{table}[]
    \centering
    \begin{tabular}{cc|cc|cc|cc|cc}
    \multicolumn{2}{c|}{\includegraphics[width = 0.16\columnwidth]{assets/05-All-BoxPlots/16-G18/SE/G18-Feel-In-Control-SE.png}} &
    \multicolumn{2}{c|}{\includegraphics[width = 0.16\columnwidth]{assets/05-All-BoxPlots/16-G18/SE/G18-Feel-Secure-SE.png}} &
    \multicolumn{2}{c|}{\includegraphics[width = 0.16\columnwidth]{assets/05-All-BoxPlots/16-G18/SE/G18-Feel-Adequate-SE.png}} &
    \multicolumn{2}{c|}{\includegraphics[width = 0.16\columnwidth]{assets/05-All-BoxPlots/16-G18/SE/G18-Feel-Certain-SE.png}} &
    \multicolumn{2}{c}{\includegraphics[width = 0.16\columnwidth]{assets/05-All-BoxPlots/16-G18/SE/G18-Feel-Productive-SE.png}}
    \\
    \hline
    \hline
    \multicolumn{2}{c|}{\includegraphics[width = 0.16\columnwidth]{assets/05-All-BoxPlots/16-G18/SE/G18-Perceived-Useful-SE.png}} &
    \multicolumn{2}{c|}{\includegraphics[width = 0.16\columnwidth]{assets/05-All-BoxPlots/16-G18/SE/G18-Not-Suspicious-SE.png}} &
    \multicolumn{2}{c|}{\includegraphics[width = 0.16\columnwidth]{assets/05-All-BoxPlots/16-G18/SE/G18-Not-Harmful-SE.png}} &
    \multicolumn{2}{c|}{\includegraphics[width = 0.16\columnwidth]{assets/05-All-BoxPlots/16-G18/SE/G18-Product-Reliable-SE.png}} &
    \multicolumn{2}{c}{\includegraphics[width = 0.16\columnwidth]{assets/05-All-BoxPlots/16-G18/SE/G18-Trust-Product-SE.png}}
    \end{tabular}
    
    \caption{Guideline 18 participants' ratings for all dependent variables, disaggregated by participants' computer self-efficacy.
	%For the disaggregated data, notice how large the distances between the average rating are when the guideline is applied.
	Table~\ref{tab:G18-SE-Stats-Appendix} below provides the statistics (where applicable).
}
    \label{fig:SE-G18-Appendix}
\end{table}

\begin{table}[h]

%\framebox[\linewidth]{For Measuring!}
\centering
\footnotesize

    \begin{tabular}{p{0.22\columnwidth}|c|c|c|c|c|c}
    
    \rowcolor{LightGray}\multicolumn{7}{c}{\textbf{Violation AI Product}}\\
    \hline
    \textbf{Dependent}  & \textbf{Distance b/w} &  &  & & \textbf{Bonferroni} &  \\
    \textbf{Variable} & \textbf{Means} &  \textbf{df} &  \textbf{t-val} &   \textbf{p-value}  & \textbf{Correction} & \textbf{Cohen's \textit{d}} \\
    \hline
    
    I would feel in control & 0.7647 & 64 &  1.7450 & .0858 & - - - & 0.4298  \\
    \hline
    
    I would feel secure & 0.6627 & 62 &  1.7014 & .0939 & - - - & 0.4262 \\
    \hline
    
    I would feel adequate & - - -  & - &  - - - & - - - & - - - & - - - \\
    \hline
    
    I would feel certain & 1.0143 & 65 &  2.3253 & \cellcolor{AbiOrangeQuote}.0232 & - - - & 0.5687 \\
    \hline
    
    I would feel productive & - - - & - &  - - - & - - - & - - - & - - -   \\
    \hline
    \hline
    
    I perceived it as useful &  - - - & - &  - - - & - - - & - - - & - - -   \\
    \hline
    
    I would not be suspicious & 0.9134 & 64 &  2.1555 & \cellcolor{AbiOrangeQuote}.0349 & - - - & .0.5316   \\
    \hline
    
    It would not be harmful & 0.9669 & 64 &  2.6848 & \cellcolor{AbiOrangeQuote}.0092 & - - - & 0.6612  \\
    \hline
    
    I find the product reliable & - - - & - &  - - - & - - - & - - - & - - - \\
    \hline
    
    I would trust the product & - - -  & - &  - - - & - - - & - - - & - - - \\
    \hline

    \rowcolor{LightGray}\multicolumn{7}{c}{\textbf{Application AI Product}}\\
    \hline
    \textbf{Dependent}  & \textbf{Distance b/w} &  &  & & \textbf{Bonferroni} &  \\
    \textbf{Variable} & \textbf{Means} &  \textbf{df} &  \textbf{t-val} &   \textbf{p-value}  & \textbf{Correction} & \textbf{Cohen's \textit{d}} \\
    \hline
    
    I would feel in control & 0.7298 & 64 &  2.1509 & \cellcolor{AbiOrangeQuote}.0353 & .2118 & 0.4976  \\
    \hline
    
    I would feel secure & - - - & - &  - - - & - - - & - - - & - - - \\
    \hline
    
    I would feel adequate & - - -  & - &  - - - & - - - & - - - & - - - \\
    \hline
    
    I would feel certain & 0.8723 & 65 &  2.1850 & \cellcolor{AbiOrangeQuote}.0325 & .195 & 0.5344 \\
    \hline
    
    I would feel productive & - - -  & - &  - - - & - - - & - - - & - - -   \\
    \hline
    \hline
    
    I perceived it as useful &  0.7438 & 64 &  2.3809 & \cellcolor{AbiOrangeQuote}.0203 & .1218 & 0.5872   \\
    \hline
    
    I would not be suspicious & 0.9706 & 64 &  2.6049 & \cellcolor{AbiOrangeQuote}.0114 & .0684 & 0.6416   \\
    \hline
    
    It would not be harmful & 1.0959 & 64 &  3.6883 & \cellcolor{AbiOrangeQuote}.0005 & \cellcolor{AbiOrangeQuote}.003 & 0.9097  \\
    \hline
    
    I find the product reliable & - - - & - &  - - - & - - - & - - - & - - - \\
    \hline
    
    I would trust the product & 0.6305 & 64 &  1.9598 & .0544 & .3264 & 0.4827

    \end{tabular}

    \caption{Guideline 18's t-test results %(\checkmark if Welch's t-test) 
    for lower self-efficacy vs. higher self-efficacy participants' average ratings of the independent Violation AI product (top) and Application AI product (bottom), for all 10 dependent variables.
    If dashes (- - -) are present, no statistical test was performed.
    If the number of tests exceeded 5 for each product, Bonferroni correction applied by multiplying p-values by the number of tests performed.
    }
    \label{tab:G18-SE-Stats-Appendix}
\end{table}
\clearpage
%---------------------------------------------------- End Guideline 18
