# Supplementary material for: Measuring User Experience Inclusivity in Human-AI Interaction via Five User Problem-Solving Styles
Source: arXiv:2108.00588 source file (2024-02-17)
Supplement: Supplementary file 12 [file Appendix-AnalysisChange.tex]

\section{Analysis change in Section~\ref{sec:gender}}
\label{appendix:analysis-change}

\subsection{Why we combine participants from all 16 experiments in this section.}

\boldify{Here's the problem: people were classified differently, depending on their experimental assignment. For example, take participant G1-205-risk-averse in Guideline 1's experiment. They had a risk-score of 26, and the median for Guideline 1's experiment was 25 (thus risk-averse because they were above it).}

In Section~\ref{sec:Results-Insights}, participants (the experimental units) generated 2 data points (measurement units) for each of the 10 dependent variables discussed.
We interpreted those measurements by looking through one of their 5 problem solving styles, like their attitudes toward risk.
However, these were dependent on their experimental assignment.
For example, take participant 205 in Guideline 1's experiment (G1-205), who had a risk score of 26.
The median score for all 64 participants in in Guideline 1's experiment was 25, so G1-205 was risk-averse relative to their 63 peers (see Table~\ref{tab:style_rules} for the rules).


\boldify{However, had they been randomly placed in any other experiment (assuming they would have answered the exact same questions the exact same way), their score of 26 might have placed them in the risk-tolerant category, like for Guideline 6 ( its independent median was 27). Turns out that for 8 experiments, this participant would be risk-averse, and the other 8 risk-tolerant }

What would have happened if G1-205 had been placed in any other experiment, since experimental assignment was equally likely?
Since their answers to the survey were independent of their experimental assignment, they would have answered the exact same questions in the survey (Appendix~\ref{sec:appendix-facets}) the exact same way, so they would have still scored a 26 for risk.
However, in Guideline 6's experiment, the median was 27, so G1-205 would have been risk-tolerant relative to those 68 participants.
Further, G1-205 would be classified as risk-averse in 8 of the experiments, but they would be classified risk-\textit{tolerant} in the other 8.
These variations happened for all five of the problem solving styles (Table~\ref{table:personas}).

\boldify{So if this happens enough times across the 5 facets, it can change the outcome variable for our statistical analysis. In Table~\ref{tab:Fisher-1}, the threshold of $\geq 3$ and $< 3$ exist, but if we used their relative facets, then people like participant G1-743 could have between 2 (if they were in G6) and 5 (for G1, G7, G11, G15, \& G18) ``Abi'' styles. }

Since we count up the number of ``Abi''-like and ``Tim''-like problem solving styles each participant had in  Section~\ref{sec:gender}, we had to ensure that our outcome variable (i.e., these number of ``Abi-'' and ``Tim''-like styles) could not change.
Thus, to avoid the variation discussed above, we had to re-compute their problem solving styles because of the dependency of their styles on their experimental assignment.
Thus, we re-computed their problem solving styles (Section~\ref{sec:GenderMag}) relative to grand medians of all 1,016 participants to analyze the data in Section~\ref{sec:gender}.
